# Supplementary material for: Involutive scroll structures on solutions of 4D dispersionless integrable hierarchies
Source: arXiv:2503.10897 ancillary file (2025-03-13)
Supplement: Supplementary file 1 [file EFBK25-Scroll-Suppl-1.pdf]

Computation of Lax distributions, characteristic varieties and point symmetry algebras for the integrable hierarchies of EFBK-2025-Scroll paper

>

```
> with(DifferentialGeometry) : with(JetCalculus) : with(Tensor) : with(Tools) :
    with(LieAlgebras) : with(PDETools) :
  Preferences("ShowFramePrompt",'false') : interface(warnlevel = 0) : interface(rtablesize
    = 14) :
```

>

S2 constructions

```
> var := x1, x2, x3, x4 : DGsetup([var], R4) :
```

Construction 1

```
> g := evalDG(dx2 &s dx3 − dx1 &s dx4 + u1 dx3 &s dx3 + (v1 − u2) dx3 &s dx4 + v2 dx4
    &s dx4) :
  V1 := evalDG(D_x3 + (v1 − q) D_x1 + u1 D_x2) : V2 := evalDG(D_x4 + v2 D_x1 + (u2
    − q) D_x2) :
  InverseMetric(g); ContractIndices(g, V1 &t V1, [[1, 1], [2, 2]]), ContractIndices(g, V1 &t V2,
    [[1, 1], [2, 2]]), ContractIndices(g, V2 &t V2, [[1, 1], [2, 2]])
```

−4 v2 D_x1 D_x1 − (−2 v1 + 2 u2) D_x1 D_x2 − 2 D_x1 D_x4 − (−2 v1 + 2 u2) D_x2 D_x1 − 4 u1 D_x2 D_x2 + 2 D_x2 D_x3 + 2 D_x3 D_x2 − 2 D_x4 D_x1

2 u1, 0, 0 **(1)**

```
> g := evalDG(dx2 &s dx3 − dx1 &s dx4 − u1 dx3 &s dx3 + (v1 − u2) dx3 &s dx4 + v2 dx4
    &s dx4) :
  V1 := evalDG(D_x3 + (v1 − q) D_x1 + u1 D_x2) : V2 := evalDG(D_x4 + v2 D_x1 + (u2
    − q) D_x2) :
  InverseMetric(g); ContractIndices(g, V1 &t V1, [[1, 1], [2, 2]]), ContractIndices(g, V1 &t V2,
    [[1, 1], [2, 2]]), ContractIndices(g, V2 &t V2, [[1, 1], [2, 2]])
```

−4 v2 D_x1 D_x1 − (−2 v1 + 2 u2) D_x1 D_x2 − 2 D_x1 D_x4 − (−2 v1 + 2 u2) D_x2 D_x1 + 4 u1 D_x2 D_x2 + 2 D_x2 D_x3 + 2 D_x3 D_x2 − 2 D_x4 D_x1

0, 0, 0 **(2)**

```
> DGsetup([var, q], M5) :
> V1 := evalDG(D_x3 + (diff(v(var), x1)−q) D_x1 + diff(u(var), x1) D_x2 + diff(w(var),
    x1) D_q) : V2 := evalDG(D_x4 + diff(v(var), x2) D_x1 + (diff(u(var), x2)−q) D_x2
    + diff(w(var), x2) D_q) :
> ToJet(DGinfo(LieDerivative(V1, V2), "CoefficientSet"), {u(var), v(var), w(var)}, notation
    =jetnumbers)
```

$\{u_1 w_{2,2} - u_2 w_{1,2} + v_1 w_{1,2} - v_2 w_{1,1} - w_{1,4} + w_{2,3}, u_1 u_{2,2} - u_2 u_{1,2} - u_{1,1} v_2 + u_{1,2} v_1 - u_{1,4} + u_{2,3} - w_1, u_1 v_{2,2} - u_2 v_{1,2} + v_1 v_{1,2} - v_2 v_{1,1} - v_{1,4} + v_{2,3} + w_2\}$ **(3)**

```
> DGsetup([var], [u, v, w], J4, 2) :
```

> $Q1 := f \to TotalDiff(f, [2,3]) - TotalDiff(f, [1,4]) + u_1\, TotalDiff(f, [2,2]) + v_1\, TotalDiff(f, [1,2]) - u_2\, TotalDiff(f, [1,2]) - v_2\, TotalDiff(f, [1,1])$ :

> $simplify(\{Q1(u_{[\,]}) - w_1, Q1(v_{[\,]}) + w_2, Q1(w_{[\,]})\})$

$\{(-u_2 + v_1) w_{1,2} + u_1 w_{2,2} - v_2 w_{1,1} - w_{1,4} + w_{2,3}, (-u_2 + v_1) u_{1,2} + u_1 u_{2,2} - v_2 u_{1,1} + u_{2,3}$ **(4)**

$$- w_1 - u_{1,4}, \left(-u_2 + v_1\right) v_{1,2} + u_1 v_{2,2} - v_2 v_{1,1} + v_{2,3} + w_2 - v_{1,4}\}$$

Construction 2

```
> ChangeFrame(R4) :
> g := evalDG((u1 dx1 + u2 dx2) &s dx4 − (v1 dx1 + v2 dx2) &s dx3) :
  V1 := evalDG(q D_x1 − u1 D_x3 − v1 D_x4) : V2 := evalDG(q D_x2 − u2 D_x3
      − v2 D_x4) :
   evalDG((−u1 v2 + u2 v1)·InverseMetric(g)); ContractIndices(g, V1 &t V1, [[1, 1], [2,
      2]]), ContractIndices(g, V1 &t V2, [[1, 1], [2, 2]]), ContractIndices(g, V2 &t V2, [[1, 1],
      [2, 2]])
```

$$-2\, u2\, D\_x1\, D\_x3 - 2\, v2\, D\_x1\, D\_x4 + 2\, u1\, D\_x2\, D\_x3 + 2\, v1\, D\_x2\, D\_x4 - 2\, u2\, D\_x3\, D\_x1 + 2\, u1\, D\_x3\, D\_x2 - 2\, v2\, D\_x4\, D\_x1 + 2\, v1\, D\_x4\, D\_x2$$

$$0, 0, 0 \qquad (5)$$

```
> W1 := evalDG(D_x1 + q D_x2) : W2 := evalDG((u2 q + u1) D_x3 + (v2 q + v1) D_x4) :
      ContractIndices(g, W1 &t W1, [[1, 1], [2, 2]]), simplify(ContractIndices(g, W1 &t W2,
      [[1, 1], [2, 2]])), ContractIndices(g, W2 &t W2, [[1, 1], [2, 2]])
```

$$0, 0, 0 \qquad (6)$$

```
> ChangeFrame(M5) :
> V1 := evalDG(q D_x1 − diff(u(var), x1) D_x3 − diff(v(var), x1) D_x4 + q diff(w(var),
      x1) D_q) : V2 := evalDG(q D_x2 − diff(u(var), x2) D_x3 − diff(v(var), x2) D_x4
      + q diff(w(var), x2) D_q) :
> ToJet(DGinfo(evalDG(LieDerivative(V1, V2) + diff(w(var), x2) V1 − diff(w(var), x1) V2),
      "CoefficientSet"), {u(var), v(var), w(var)}, notation = jetnumbers)
```

$$\{q\left(-u_1 w_{2,3} + u_2 w_{1,3} - v_1 w_{2,4} + v_2 w_{1,4}\right), u_1 u_{2,3} - u_1 w_2 - u_2 u_{1,3} + u_2 w_1 - u_{1,4} v_2 + u_{2,4} v_1, u_1 v_{2,3} - u_2 v_{1,3} + v_1 v_{2,4} - v_1 w_2 - v_2 v_{1,4} + v_2 w_1\} \qquad (7)$$

```
> V1 := evalDG(q D_x1 − u1(var) D_x3 − v1(var) D_x4 + q w1(var) D_q) : V2 :=
      evalDG(q D_x2 − u2(var) D_x3 − v2(var) D_x4 + q w2(var) D_q) :
> map(coeffs, expand(ToJet(DGinfo(evalDG(LieDerivative(V1, V2) + w2(var) V1
      − w1(var) V2), "CoefficientSet"), {u1(var), u2(var), v1(var), v2(var), w1(var),
      w2(var)}, notation = jetnumbers)), q)
```

$$\{u1_2 - u2_1, v1_2 - v2_1, -w1_2 + w2_1, -u1[\,]\, w2_3 + u2[\,]\, w1_3 - v1[\,]\, w2_4 + v2[\,]\, w1_4, u1[\,]\, u2_3 - w2[\,]\, u1[\,] - u1_3\, u2[\,] - u1_4\, v2[\,] + w1[\,]\, u2[\,] + u2_4\, v1[\,], u1[\,]\, v2_3 - u2[\,]\, v1_3 + v1[\,]\, v2_4 - w2[\,]\, v1[\,] - v1_4\, v2[\,] + w1[\,]\, v2[\,]\} \qquad (8)$$

```
> ChangeFrame(J4) :
> R1 := f→u₁ TotalDiff(f, [2, 3]) + v₁ TotalDiff(f, [2, 4]) − u₂ TotalDiff(f, [1, 3])
      − v₂ TotalDiff(f, [1, 4]) :
> simplify({R1(u[ ]) − u₁ w₂ + u₂ w₁, R1(v[ ]) − v₁ w₂ + v₂ w₁, R1(w[ ])})
```

$$\{\left(v_{2,4} - w_2\right) v_1 + \left(w_1 - v_{1,4}\right) v_2 + u_1 v_{2,3} - u_2 v_{1,3}, \left(-w_2 + u_{2,3}\right) u_1 + \left(w_1 - u_{1,3}\right) u_2 + v_1 u_{2,4} - v_2 u_{1,4}, u_1 w_{2,3} - u_2 w_{1,3} + v_1 w_{2,4} - v_2 w_{1,4}\} \qquad (9)$$

```
>
> ChangeFrame(R4) : g0 := evalDG(dx1 &s dx4 − dx2 &s dx3) :
```

> $HodgeStar(g0, dx1 \&w\ dx2), HodgeStar(g0, dx3 \&w\ dx4), HodgeStar(g0, dx1 \&w\ dx4 - dx2 \&w\ dx3)$

$$dx1 \wedge dx2, dx3 \wedge dx4, dx1 \wedge dx4 - dx2 \wedge dx3 \quad (10)$$

> $HodgeStar(g0, dx1 \&w\ dx3), HodgeStar(g0, dx2 \&w\ dx4), HodgeStar(g0, dx1 \&w\ dx4 + dx2 \&w\ dx3)$

$$-dx1 \wedge dx3, -dx2 \wedge dx4, -dx1 \wedge dx4 - dx2 \wedge dx3 \quad (11)$$

>

S2.1

> $DGsetup([seq(x \| i, i = 1..5)], [u], J5, 5):$

> $Eq2 := \{u_{1,5} - u_{1,3}\, u_{4,4} + u_{1,4}\, u_{3,4}, u_{2,5} - u_{2,3}\, u_{4,4} + u_{2,4}\, u_{3,4}, u_{1,4}\, u_{2,3} - u_{1,3}\, u_{2,4} - 1\}:$
$el2 := eliminate(Eq2, \{u_{1,4}, u_{1,5}, u_{2,5}\}) : sl2 := el2[1] : el2[2]$

$$\varnothing \quad (12)$$

> $Eq3 := \{seq(op(map(TotalDiff, Eq2, i)), i = 1..5)\} : el3 := eliminate(Eq3, \{seq(u_{1,i,4}, i = 1..4), seq(u_{1,i,5}, i = 1..5), seq(u_{2,i,5}, i = 2..5)\}) : sl3 := el3[1] : el3[2]$

$$\varnothing \quad (13)$$

> $Eq4 := \{seq(seq(op(map(TotalDiff, Eq2, [i, j])), j = i..5), i = 1..5)\} : el4 := eliminate(Eq4, \{seq(seq(u_{1,i,j,4}, j = i..4), i = 1..4), seq(seq(u_{1,i,j,5}, j = i..5), i = 1..5), seq(seq(u_{2,i,j,5}, j = i..5), i = 2..5)\}) : sl4 := el4[1] : simplify(eval(el4[2], sl3))$

$$\{0\} \quad (14)$$

> $Char := \{p1\, p5 - u_{1,3}\, p4^2 - u_{4,4}\, p1\, p3 + u_{1,4}\, p3\, p4 + u_{3,4}\, p1\, p4, p2\, p5 - u_{2,3}\, p4^2 - u_{4,4}\, p2\, p3 + u_{2,4}\, p3\, p4 + u_{3,4}\, p2\, p4, u_{1,4}\, p2\, p3 + u_{2,3}\, p1\, p4 - u_{1,3}\, p2\, p4 - u_{2,4}\, p1\, p3\}$
$:$

> $simplify(eval(Char, \{p1 = -a\, u_{1,4} + b\, u_{1,3}, p2 = -a\, u_{2,4} + b\, u_{2,3}, p3 = a\, q, p4 = b\, q, p5 = a\, q\, u_{4,4} - b\, q\, u_{3,4} + b\, q^2\}))$

$$\{0\} \quad (15)$$

>

S2.2.1: construction 1

> $var5 := seq(x \| i, i = 1..5) : DGsetup([var5, q], M6):$

> $V1 := evalDG(D\_x3 + (diff(v(var5), x1) - q)\, D\_x1 + diff(u(var5), x1)\, D\_x2 + diff(w(var5), x1)\, D\_q):$
$V2 := evalDG(D\_x4 + diff(v(var5), x2)\, D\_x1 + (diff(u(var5), x2) - q)\, D\_x2 + diff(w(var5), x2)\, D\_q):$
$V3 := evalDG(D\_x5 + (diff(v(var5), x3) - w(var5))\, D\_x1 + diff(u(var5), x3)\, D\_x2 - q\, D\_x3 + diff(w(var5), x3)\, D\_q):$

> $Eq12 := ToJet(DGinfo(LieDerivative(V1, V2), \text{"CoefficientSet"}), \{u(var5), v(var5), w(var5)\}, notation = jetnumbers);$
$Eq13 := ToJet(DGinfo(evalDG(LieDerivative(V1, V3) + diff(w(var5), x1)\, V1), \text{"CoefficientSet"}), \{u(var5), v(var5), w(var5)\}, notation = jetnumbers);$
$Eq23 := ToJet(DGinfo(evalDG(LieDerivative(V2, V3) + diff(w(var5), x2)\, V1), \text{"CoefficientSet"}), \{u(var5), v(var5), w(var5)\}, notation = jetnumbers)$

$Eq12 := \{u_1\, w_{2,2} - u_2\, w_{1,2} + v_1\, w_{1,2} - v_2\, w_{1,1} - w_{1,4} + w_{2,3}, u_1\, u_{2,2} - u_2\, u_{1,2} - u_{1,1}\, v_2$

$$+ u_{1,2} v_1 - u_{1,4} + u_{2,3} - w_1, u_1 v_{2,2} - u_2 v_{1,2} + v_1 v_{1,2} - v_2 v_{1,1} - v_{1,4} + v_{2,3} + w_2\}$$

$$Eq13 := \{u_1 u_{2,3} + u_1 w_1 - u_3 u_{1,2} - u_{1,1} v_3 + u_{1,1} w[\,] + v_1 u_{1,3} - u_{1,5} + u_{3,3}, u_1 v_{2,3} - u_1 w_2 - u_3 v_{1,2} + v_1 v_{1,3} - v_{1,1} v_3 + v_{1,1} w[\,] - v_{1,5} + v_{3,3}, u_1 w_{2,3} - u_3 w_{1,2} + v_1 w_{1,3} - v_3 w_{1,1} + w[\,] w_{1,1} + w_1^2 - w_{1,5} + w_{3,3}\}$$

$$Eq23 := \{w_2 (v_1 - q) - (v_3 - w[\,]) v_{1,2} - u_3 v_{2,2} + q v_{2,3} - v_{2,5} + v_2 (v_{1,3} - w_1) + (u_2 - q) (v_{2,3} - w_2) + v_{3,4} - w_4, u_2 w_{2,3} - u_3 w_{2,2} + v_2 w_{1,3} - v_3 w_{1,2} + w[\,] w_{1,2} + w_1 w_2 - w_{2,5} + w_{3,4}, u_1 w_2 + u_2 u_{2,3} - u_3 u_{2,2} - u_{1,2} v_3 + u_{1,2} w[\,] + u_{1,3} v_2 - u_{2,5} + u_{3,4} + w_3\} \quad (16)$$

$> DGsetup([var5], [u, v, w], J5, 2):$

$$> Q1 := f \to TotalDiff(f, [2,3]) - TotalDiff(f, [1,4]) + u_1\, TotalDiff(f, [2,2]) + (v_1 - u_2)\, TotalDiff(f, [1,2]) - v_2\, TotalDiff(f, [1,1]):$$

$$Q2 := f \to TotalDiff(f, [3,3]) - TotalDiff(f, [1,5]) + u_1\, TotalDiff(f, [2,3]) + v_1\, TotalDiff(f, [1,3]) - u_3\, TotalDiff(f, [1,2]) + (w_{[\,]} - v_3)\, TotalDiff(f, [1,1]):$$

$$Q3 := f \to TotalDiff(f, [3,4]) - TotalDiff(f, [2,5]) + u_2\, TotalDiff(f, [2,3]) + v_2\, TotalDiff(f, [1,3]) - u_3\, TotalDiff(f, [2,2]) + (w_{[\,]} - v_3)\, TotalDiff(f, [1,2]):$$

$$> simplify(eval(Eq12 \textbf{ union } Eq13 \textbf{ union } Eq23, solve(\{Q1(u_{[\,]}) - w_1, Q1(v_{[\,]}) + w_2, Q1(w_{[\,]}), Q2(u_{[\,]}) + u_1 w_1, Q2(v_{[\,]}) - u_1 w_2, Q2(w_{[\,]}) + w_1^2, Q3(u_{[\,]}) + w_3 + u_1 w_2, Q3(v_{[\,]}) - w_4 - v_2 w_1 + (v_1 - u_2) w_2, Q3(w_{[\,]}) + w_1 w_2\}, \{u_{1,4}, u_{1,5}, u_{2,5}, v_{1,4}, v_{1,5}, v_{2,5}, w_{1,4}, w_{1,5}, w_{2,5}\})))$$

$$\{0\} \quad (17)$$

$$> Char := \{p2\, p3 - p1\, p4 + u_1\, p2^2 + v_1\, p1\, p2 - u_2\, p1\, p2 - v_2\, p1^2, p3^2 - p1\, p5 + u_1\, p2\, p3 + v_1\, p1\, p3 - u_3\, p1\, p2 + (w_{[\,]} - v_3)\, p1^2, p3\, p4 - p2\, p5 + u_2\, p2\, p3 + v_2\, p1\, p3 - u_3\, p2^2 + (w_{[\,]} - v_3)\, p1\, p2\}:$$

$$> simplify(eval(Char, \{p1 = b, p2 = a, p3 = -a\, u_1 + b \cdot (q - v_1), p4 = a \cdot (q - u_2) - b\, v_2, p5 = -a \cdot (u_3 + q\, u_1) - b \cdot (v_3 + q\, v_1 - q^2 - w_{[\,]})\}))$$

$$\{0\} \quad (18)$$

$$> Eq2 := Eq12 \textbf{ union } Eq13 \textbf{ union } Eq23 : el2 := eliminate(Eq2, \{u_{1,4}, u_{1,5}, u_{2,5}, v_{1,4}, v_{1,5}, v_{2,5}, w_{1,4}, w_{1,5}, w_{2,5}\}) : sl2 := el2[1] : el2[2]$$

$$\varnothing \quad (19)$$

$$> Eq3 := \{seq(op(map(TotalDiff, Eq2, i)), i = 1..5)\} : el3 := eliminate(Eq3, \{seq(u_{1,i,4}, i = 1..4), seq(u_{1,i,5}, i = 1..5), seq(u_{2,i,5}, i = 2..5), seq(v_{1,i,4}, i = 1..4), seq(v_{1,i,5}, i = 1..5), seq(v_{2,i,5}, i = 2..5), seq(w_{1,i,4}, i = 1..4), seq(w_{1,i,5}, i = 1..5), seq(w_{2,i,5}, i = 2..5)\}) : sl3 := el3[1] : simplify(eval(el3[2], sl2))$$

$$\{0\} \quad (20)$$

$$> Eq4 := \{seq(seq(op(map(TotalDiff, Eq2, [i,j])), j = i..5), i = 1..5)\} : el4 := eliminate(Eq4, \{seq(seq(u_{1,i,j,4}, j = i..4), i = 1..4), seq(seq(u_{1,i,j,5}, j = i..5), i = 1..5), seq(seq(u_{2,i,j,5}, j = i..5), i = 2..5), seq(seq(v_{1,i,j,4}, j = i..4), i = 1..4), seq(seq(v_{1,i,j,5}, j = i..5), i = 1..5),$$

$seq\left(seq\left(v_{2,i,j,5}, j=i..5\right), i=2..5\right), seq\left(seq\left(w_{1,i,j,4}, j=i..4\right), i=1..4\right), seq\left(seq\left(w_{1,i,j,5}, j=i..5\right), i=1..5\right), seq\left(seq\left(w_{2,i,j,5}, j=i..5\right), i=2..5\right)\}\right) : sl4 := el4[1] :$
$simplify(eval(eval(el4[2], sl3), sl2))$

$$\{0\} \quad \textbf{(21)}$$

> $V := evalDG\left(b1\left(var5, u_{[\,]}, v_{[\,]}, w_{[\,]}\right) D\_u[\,] + b2\left(var5, u_{[\,]}, v_{[\,]}, w_{[\,]}\right) D\_v[\,] + b3\left(var5, u_{[\,]}, v_{[\,]}, w_{[\,]}\right) D\_w[\,]\right) : V2 := Prolong(V, 2) :$

> $psl2 := pdsolve\left(\{seq\left(coeffs\left(expand(eval(LieDerivative(V2, Eq2[i]), sl2)), \{seq\left(u_i, i=1..5\right), seq\left(v_i, i=1..5\right), seq\left(w_i, i=1..5\right), seq\left(seq\left(u_{i,j}, j=i..5\right), i=1..5\right), seq\left(seq\left(v_{i,j}, j=i..5\right), i=1..5\right), seq\left(seq\left(w_{i,j}, j=i..5\right), i=1..5\right)\}\right), i=1..nops(Eq2)\right)\}\right)$

$$psl2 := \{b1(x1, x2, x3, x4, x5, u[\,], v[\,], w[\,]) = f_2(x4, x5), b2(x1, x2, x3, x4, x5, u[\,], v[\,], w[\,]) = f_1(x4, x5)\, x3 + f_3(x4, x5), b3(x1, x2, x3, x4, x5, u[\,], v[\,], w[\,]) = f_1(x4, x5)\} \quad \textbf{(22)}$$

> $V := evalDG\left(a1\left(var5, u_{[\,]}, v_{[\,]}, w_{[\,]}\right) D\_x1 + a2\left(var5, u_{[\,]}, v_{[\,]}, w_{[\,]}\right) D\_x2 + a3\left(var5, u_{[\,]}, v_{[\,]}, w_{[\,]}\right) D\_x3 + a4\left(var5, u_{[\,]}, v_{[\,]}, w_{[\,]}\right) D\_x4 + a5\left(var5, u_{[\,]}, v_{[\,]}, w_{[\,]}\right) D\_x5 + b1\left(var5, u_{[\,]}, v_{[\,]}, w_{[\,]}\right) D\_u[\,] + b2\left(var5, u_{[\,]}, v_{[\,]}, w_{[\,]}\right) D\_v[\,] + b3\left(var5, u_{[\,]}, v_{[\,]}, w_{[\,]}\right) D\_w[\,]\right) :$
$V2 := Prolong(V, 2) :$

> $pdsys := \{seq\left(coeffs\left(expand(eval(LieDerivative(V2, Eq2[i]), sl2)), \{seq\left(u_i, i=1..5\right), seq\left(v_i, i=1..5\right), seq\left(w_i, i=1..5\right), seq\left(seq\left(u_{i,j}, j=i..5\right), i=1..5\right), seq\left(seq\left(v_{i,j}, j=i..5\right), i=1..5\right), seq\left(seq\left(w_{i,j}, j=i..5\right), i=1..5\right)\}\right), i=1..nops(Eq2)\right)\} : psl2 := pdsolve(pdsys)$

$$psl2 := \left\{ a1(x1, x2, x3, x4, x5, u[\,], v[\,], w[\,]) = \left(-\frac{d}{dx5} f_2(x5) + 2 f_3(x4, x5)\right) x1 + \left(\left(\frac{\partial}{\partial x4} f_3(x4, x5)\right) x3 + \frac{\partial}{\partial x4} f_4(x4, x5)\right) x2 + \frac{\left(-\frac{d^2}{dx5^2} f_2(x5) + 2 \frac{\partial}{\partial x5} f_3(x4, x5)\right) x3^2}{2} + \left(f_8(x4, x5) + \frac{\partial}{\partial x5} f_4(x4, x5) + f_{11}(x5) + c_1\right) x3 + f_{13}(x4, x5), a2(x1, x2, x3, x4, x5, u[\,], v[\,], w[\,]) = \left(\frac{\partial}{\partial x5} f_1(x4, x5)\right) x3 + \left(-\frac{d}{dx5} f_2(x5) + \frac{\partial}{\partial x4} f_1(x4, x5) + f_3(x4, x5)\right) x2 + f_5(x4, x5), a3(x1, x2, x3, x4, x5, u[\,], v[\,], w[\,]) = f_3(x4, x5)\, x3 + f_4(x4, x5), a4(x1, x2, x3, x4, x5, u[\,], v[\,], w[\,]) = f_1(x4, x5), a5(x1, x2, x3, x4, x5, u[\,], v[\,], w[\,]) \right. \quad \textbf{(23)}$$

$$=f_{2}(x5),\ b1(x1, x2, x3, x4, x5, u[\ ], v[\ ], w[\ ]) = \left(\frac{\partial}{\partial x5}\ f_{1}(x4, x5)\right) x1 + \Big(-2\ \frac{d}{dx5}\ f_{2}(x5)$$

$$+\ 2\, f_{3}(x4, x5) + \frac{\partial}{\partial x4}\ f_{1}(x4, x5)\Big)\ u[\ ] + \frac{\left(\frac{\partial^{2}}{\partial x5^{2}}\ f_{1}(x4, x5)\right) x3^{2}}{2} + \Big(-x2\ \Big(\frac{d^{2}}{dx5^{2}}$$

$$f_{2}(x5)\Big) + x2\left(\frac{\partial}{\partial x5}\ f_{3}(x4, x5)\right) + x2\left(\frac{\partial^{2}}{\partial x4 \partial x5}\ f_{1}(x4, x5)\right) + \frac{\partial}{\partial x5}\ f_{5}(x4, x5)\Big)\ x3$$

$$+\ \frac{x2^{2}\left(\frac{\partial^{2}}{\partial x4^{2}}\ f_{1}(x4, x5) + 2\ \frac{\partial}{\partial x4}\ f_{3}(x4, x5)\right)}{2} + \Big(\frac{\partial}{\partial x4}\ f_{5}(x4, x5) + f_{11}(x5) + f_{8}(x4, x5)$$

$$+\ c_{1}\Big)\ x2 + f_{14}(x4, x5),\ b2(x1, x2, x3, x4, x5, u[\ ], v[\ ], w[\ ]) = \Big(-2\ \frac{d}{dx5}\ f_{2}(x5) + 3\, f_{3}(x4,$$

$$x5)\Big)\ v[\ ] + \Big(\left(\frac{\partial}{\partial x4}\ f_{3}(x4, x5)\right) x3 + \frac{\partial}{\partial x4}\ f_{4}(x4, x5)\Big)\ u[\ ] + \Big(-2\left(\frac{d^{2}}{dx5^{2}}\ f_{2}(x5)\right) x3$$

$$+\ 3\left(\frac{\partial}{\partial x5}\ f_{3}(x4, x5)\right) x3 + 2\left(\frac{\partial}{\partial x4}\ f_{3}(x4, x5)\right) x2 + 2\, f_{11}(x5) + 2\, f_{8}(x4, x5) + \frac{\partial}{\partial x5}$$

$$f_{4}(x4, x5) + 2\ c_{1}\Big)\ x1 + \frac{\left(\left(\frac{\partial^{2}}{\partial x4^{2}}\ f_{3}(x4, x5)\right) x3 + \frac{\partial^{2}}{\partial x4^{2}}\ f_{4}(x4, x5)\right) x2^{2}}{2} + \Big(\Big(\frac{\partial^{2}}{\partial x4 \partial x5}$$

$$f_{3}(x4, x5)\Big)\ x3^{2} + x3\left(\frac{\partial^{2}}{\partial x4 \partial x5}\ f_{4}(x4, x5)\right) + x3\left(\frac{\partial}{\partial x4}\ f_{8}(x4, x5)\right) + \frac{\partial}{\partial x4}\ f_{13}(x4, x5)\Big)\ x2$$

$$+\ \frac{\left(-2\ \frac{d^{3}}{dx5^{3}}\ f_{2}(x5) + 3\ \frac{\partial^{2}}{\partial x5^{2}}\ f_{3}(x4, x5)\right) x3^{3}}{6}$$

$$+\ \frac{\left(2\ \frac{\partial}{\partial x5}\ f_{8}(x4, x5) + \frac{\partial^{2}}{\partial x5^{2}}\ f_{4}(x4, x5) + 2\ \frac{d}{dx5}\ f_{11}(x5)\right) x3^{2}}{2} + \Big(\frac{\partial}{\partial x5}\ f_{13}(x4, x5)$$

$$+\ f_{10}(x4, x5)\Big)\ x3 + f_{15}(x4, x5),\ b3(x1, x2, x3, x4, x5, u[\ ], v[\ ], w[\ ]) = \Big(\frac{\partial}{\partial x4}\ f_{3}(x4,$$

$$x5)\Big) u[\,] + 2\left(-\frac{d}{dx5} f_2(x5) + f_3(x4, x5)\right) w[\,] + \left(-\frac{d^2}{dx5^2} f_2(x5) + \frac{\partial}{\partial x5} f_3(x4, x5)\right) x1$$
$$+ \frac{x2^2 \left(\frac{\partial^2}{\partial x4^2} f_3(x4, x5)\right)}{2} + \left(\left(\frac{\partial^2}{\partial x4 \partial x5} f_3(x4, x5)\right) x3 + \frac{\partial}{\partial x4} f_8(x4, x5)\right) x2$$
$$+ \frac{\left(-\frac{d^3}{dx5^3} f_2(x5) + \frac{\partial^2}{\partial x5^2} f_3(x4, x5)\right) x3^2}{2} + \left(\frac{\partial}{\partial x5} f_8(x4, x5) + \frac{d}{dx5} f_{11}(x5)\right) x3$$
$$+ f_{10}(x4, x5)\Big\}$$

# 1 arg:2, 11; 2 *arg* : 1, 3, 4, 5, 8, 10 , 13, 14, 15
thus the symmetry of the corresponding PDE system contains only (9) functions of 2 arguments, and so cannot change count of functions of 3 arguments in the solution space

> *pdetest*( *psl2*, *pdsys*)

$$\{0\} \quad (24)$$

>

S2.2.1a: reduction to Dunajski hierarchy

> $suvrho := \{u_{[\,]} = -z_1, u_1 = -z_{1,1}, u_2 = -z_{1,2}, u_3 = -z_{1,3}, u_{1,1} = -z_{1,1,1}, u_{1,2} = -z_{1,1,2}, u_{1,3} = -z_{1,1,3}, u_{2,2} = -z_{1,2,2}, u_{2,3} = -z_{1,2,3}, u_{1,4} = -z_{1,1,4}, u_{1,5} = -z_{1,1,5}, u_{2,5} = -z_{1,2,5}, u_{3,3} = -z_{1,3,3}, u_{3,4} = -z_{1,3,4}, v_{[\,]} = z_2, v_1 = z_{1,2}, v_2 = z_{2,2}, v_3 = z_{2,3}, v_{1,1} = z_{1,1,2}, v_{1,2} = z_{1,2,2}, v_{1,3} = z_{1,2,3}, v_{2,2} = z_{2,2,2}, v_{2,3} = z_{2,2,3}, v_{2,5} = z_{2,2,5}, v_{1,4} = z_{1,2,4}, v_{1,5} = z_{1,2,5}, v_{3,3} = z_{2,3,3}, v_{3,4} = z_{2,3,4}\}$ :

> $simplify(subs(suvrho, Q1(u_{[\,]}) - w_1)); simplify(subs(suvrho, -Q1(v_{[\,]}) - w_2)); simplify(subs(suvrho, -Q1(w_{[\,]})))$

$$z_{1,1} z_{1,2,2} - 2 z_{1,2} z_{1,1,2} + z_{1,1,1} z_{2,2} - w_1 + z_{1,1,4} - z_{1,2,3}$$
$$z_{1,1} z_{2,2,2} - 2 z_{1,2} z_{1,2,2} + z_{2,2} z_{1,1,2} - w_2 + z_{1,2,4} - z_{2,2,3}$$
$$z_{2,2} w_{1,1} - 2 z_{1,2} w_{1,2} + z_{1,1} w_{2,2} + w_{1,4} - w_{2,3} \quad (25)$$

> $expand(subs(suvrho, Q2(u_{[\,]}) + u_1 w_1)); expand(subs(suvrho, -Q2(v_{[\,]}) + u_1 w_2)); expand(subs(suvrho, -Q2(w_{[\,]}) - w_1^2))$

$$-z_{1,1,1} w[\,] - z_{1,1} w_1 + z_{1,1} z_{1,2,3} - z_{1,2} z_{1,1,3} - z_{1,3} z_{1,1,2} + z_{1,1,1} z_{2,3} + z_{1,1,5} - z_{1,3,3}$$
$$-z_{1,1,2} w[\,] - z_{1,1} w_2 + z_{1,1} z_{2,2,3} - z_{1,2} z_{1,2,3} - z_{1,3} z_{1,2,2} + z_{1,1,2} z_{2,3} + z_{1,2,5} - z_{2,3,3}$$
$$-w[\,] w_{1,1} - w_1^2 + w_{1,1} z_{2,3} - z_{1,3} w_{1,2} - z_{1,2} w_{1,3} + z_{1,1} w_{2,3} + w_{1,5} - w_{3,3} \quad (26)$$

> $expand(subs(suvrho, Q3(u_{[\,]}) + w_3 + u_1 w_2)); expand(subs(suvrho, -(Q3(v_{[\,]}) - w_4 - v_2 w_1 + (v_1 - u_2) w_2))); expand(subs(suvrho, -Q3(w_{[\,]}) - w_1 w_2))$

$$-w[\,] z_{1,1,2} - z_{1,1} w_2 + z_{1,2} z_{1,2,3} - z_{1,3} z_{1,2,2} - z_{2,2} z_{1,1,3} + z_{2,3} z_{1,1,2} + w_3 + z_{1,2,5} - z_{1,3,4}$$

$$-z_{1,2,2}\, w[\,] + z_{2,2}\, w_1 - 2\, z_{1,2}\, w_2 + z_{1,2}\, z_{2,2,3} - z_{1,3}\, z_{2,2,2} - z_{2,2}\, z_{1,2,3} + z_{1,2,2}\, z_{2,3} + w_4 + z_{2,2,5} - z_{2,3,4}$$

$$-w[\,]\, w_{1,2} - w_1\, w_2 + w_{1,2}\, z_{2,3} - z_{2,2}\, w_{1,3} - z_{1,3}\, w_{2,2} + z_{1,2}\, w_{2,3} + w_{2,5} - w_{3,4} \quad \textbf{(27)}$$

>

> $Eq2a := \{z_{1,4} - z_{2,3} + z_{1,1}\, z_{2,2} - z_{1,2}^2 - w_{[\,]},\ w_{1,4} - w_{2,3} + z_{2,2}\, w_{1,1} - 2\, z_{1,2}\, w_{1,2} + z_{1,1}\, w_{2,2}\}$ :
$Eq2b := \{z_{1,5} - z_{3,3} + z_{1,1}\, z_{2,3} - z_{1,2}\, z_{1,3} - z_{1,1}\, w_{[\,]},\ w_{1,5} - w_{3,3} + z_{1,1}\, w_{2,3} + z_{2,3}\, w_{1,1} - z_{1,2}\, w_{1,3} - z_{1,3}\, w_{1,2} - w_{[\,]}\, w_{1,1} - w_1^2\}$ :
$Eq2c := \{z_{2,5} - z_{3,4} + z_{1,2}\, z_{2,3} - z_{1,3}\, z_{2,2} - z_{1,2}\, w_{[\,]} + r_{[\,]},\ w_{2,5} - w_{3,4} + z_{1,2}\, w_{2,3} + z_{2,3}\, w_{1,2} - z_{1,3}\, w_{2,2} - z_{2,2}\, w_{1,3} - w_{[\,]}\, w_{1,2} - w_1\, w_2\}$ :
$Eq2d := \{r_1 - (w_3 + z_{1,2}\, w_1 - z_{1,1}\, w_2),\ r_2 - (w_4 + z_{2,2}\, w_1 - z_{1,2}\, w_2)\}$ :

> *Eq2* := *Eq2a* **union** *Eq2b* **union** *Eq2c* **union** *Eq2d* : *sl2* := $solve(Eq2, \{z_{1,4}, z_{1,5}, z_{2,5}, w_{1,4}, w_{1,5}, w_{2,5}, r_1, r_2\})$ :

> $eval(TotalDiff(Eq2a[1], 3) - TotalDiff(Eq2b[1], 2) + TotalDiff(Eq2c[1], 1), sl2)$

$$0 \quad \textbf{(28)}$$

> $eval(TotalDiff(eval(r_1, sl2), 2) - TotalDiff(eval(r_2, sl2), 1), sl2)$

$$0 \quad \textbf{(29)}$$

> $DGsetup([var5], [z, w, r], J5, 3)$ :

> $V := evalDG(a(var5, z_{[\,]}, w_{[\,]}, r_{[\,]})\, D\_z[\,] + b(var5, z_{[\,]}, w_{[\,]}, r_{[\,]})\, D\_w[\,] + c(var5, z_{[\,]}, w_{[\,]}, r_{[\,]})\, D\_r[\,])$ : $V2 := Prolong(V, 2)$ :

> $psl2 := pdsolve(\{seq(coeffs(expand(eval(LieDerivative(V2, Eq2[i]), sl2)), \{seq(z_i, i=1..5), seq(w_i, i=1..5), seq(r_i, i=1..5), seq(seq(z_{i,j}, j=i..5), i=1..5), seq(seq(w_{i,j}, j=i..5), i=1..5), seq(seq(r_{i,j}, j=i..5), i=1..5)\}), i=1..nops(Eq2))\})$

$$psl2 := \left\{ a(x1, x2, x3, x4, x5, z[\,], w[\,], r[\,]) = f_3(x4, x5)\, x1 + \frac{\left(\frac{\partial}{\partial x5} f_3(x4, x5)\right) x3^2}{2} + \frac{x2 \left(\frac{\partial}{\partial x4} f_3(x4, x5)\right) x3}{2} + x2\, f_6(x4, x5) + f_7(x4, x5)\, x3 + f_8(x4, x5),\ b(x1, x2, x3, x4, x5, z[\,], w[\,], r[\,]) = \frac{\frac{\partial}{\partial x4} f_3(x4, x5)}{2},\ c(x1, x2, x3, x4, x5, z[\,], w[\,], r[\,]) = \frac{\left(\frac{\partial^2}{\partial x4 \partial x5} f_3(x4, x5)\right) x3}{2} - \frac{\partial}{\partial x5} f_6(x4, x5) + \frac{x2 \left(\frac{\partial^2}{\partial x4^2} f_3(x4, x5)\right)}{2} + \frac{\partial}{\partial x4} f_7(x4, x5) \right\} \quad \textbf{(30)}$$

> $Eq3 := \{seq(op(map(TotalDiff, Eq2, i)), i=1..5)\} : el3 := eliminate\left(Eq3, \left\{seq\left(z_{1,i,4}, i=1..4\right), seq\left(z_{1,i,5}, i=1..5\right), seq\left(z_{2,i,5}, i=2..5\right), seq\left(w_{1,i,4}, i=1..4\right), seq\left(w_{1,i,5}, i=1..5\right), seq\left(w_{2,i,5}, i=2..5\right), seq\left(r_{1,i}, i=1..5\right), seq\left(r_{2,i}, i=2..5\right)\right\}\right) : sl3 := el3[1] : simplify(eval(el3[2], sl2))$

$$\{0, \left(w_2 z_{1,3} + \left(w[\,] - z_{2,3}\right) w_1 + r_3 - w_5\right) w_{2,2}, \left(-w[\,] + z_{2,3}\right) w_1 - w_2 z_{1,3} - r_3 + w_5\} \quad \textbf{(31)}$$

> $Eq2a := \left\{z_{1,4} - z_{2,3} + z_{1,1} z_{2,2} - z_{1,2}^2 - w_{[\,]}, w_{1,4} - w_{2,3} + z_{2,2} w_{1,1} - 2 z_{1,2} w_{1,2} + z_{1,1} w_{2,2}\right\} :$
$Eq2b := \left\{z_{1,5} - z_{3,3} + z_{1,1} z_{2,3} - z_{1,2} z_{1,3} - z_{1,1} w_{[\,]}, w_{1,5} - w_{3,3} + z_{1,1} w_{2,3} + z_{2,3} w_{1,1} - z_{1,2} w_{1,3} - z_{1,3} w_{1,2} - w_{[\,]} w_{1,1} - w_1^2\right\} :$
$Eq2c := \left\{z_{2,5} - z_{3,4} + z_{1,2} z_{2,3} - z_{1,3} z_{2,2} - z_{1,2} w_{[\,]} + r_{[\,]}, w_{2,5} - w_{3,4} + z_{1,2} w_{2,3} + z_{2,3} w_{1,2} - z_{1,3} w_{2,2} - z_{2,2} w_{1,3} - w_{[\,]} w_{1,2} - w_1 w_2\right\} :$
$Eq2d := \left\{r_1 - \left(w_3 + z_{1,2} w_1 - z_{1,1} w_2\right), r_2 - \left(w_4 + z_{2,2} w_1 - z_{1,2} w_2\right), r_3 - \left(w_5 + \left(z_{2,3} - w[\,]\right) w_1 - z_{1,3} w_2\right)\right\} :$

> $Eq2 := Eq2a$ **union** $Eq2b$ **union** $Eq2c$ **union** $Eq2d : sl2 := solve\left(Eq2, \left\{z_{1,4}, z_{1,5}, z_{2,5}, w_{1,4}, w_{1,5}, w_{2,5}, r_1, r_2, r_3\right\}\right) :$

> $Eq3 := \{seq(op(map(TotalDiff, Eq2, i)), i=1..5)\} : el3 := eliminate\left(eval(Eq3, sl2), \left\{seq\left(z_{1,i,4}, i=1..4\right), seq\left(z_{1,i,5}, i=1..5\right), seq\left(z_{2,i,5}, i=2..5\right), seq\left(w_{1,i,4}, i=1..4\right), seq\left(w_{1,i,5}, i=1..5\right), seq\left(w_{2,i,5}, i=2..5\right), seq\left(r_{1,i}, i=1..5\right), seq\left(r_{2,i}, i=2..5\right), seq\left(r_{3,i}, i=3..5\right)\right\}\right) : sl3 := el3[1] : el3[2]$

$$\emptyset \quad \textbf{(32)}$$

> $Eq4 := \{seq(seq(op(map(TotalDiff, Eq2, [i,j])), j=i..5), i=1..5)\} : el4 := eliminate\left(eval(eval(Eq4, sl3), sl2), \left\{seq\left(seq\left(z_{1,i,j,4}, j=i..4\right), i=1..4\right), seq\left(seq\left(z_{1,i,j,5}, j=i..5\right), i=1..5\right), seq\left(seq\left(z_{2,i,j,5}, j=i..5\right), i=2..5\right), seq\left(seq\left(w_{1,i,j,4}, j=i..4\right), i=1..4\right), seq\left(seq\left(w_{1,i,j,5}, j=i..5\right), i=1..5\right), seq\left(seq\left(w_{2,i,j,5}, j=i..5\right), i=2..5\right), seq\left(seq\left(r_{1,i,j}, j=i..5\right), i=1..5\right), seq\left(seq\left(r_{2,i,j}, j=i..5\right), i=2..5\right), seq\left(seq\left(r_{3,i,j}, j=i..5\right), i=3..5\right)\right\}\right) : sl4 := el4[1] : el4[2]$

$$\emptyset \quad \textbf{(33)}$$

>

> $DGsetup([var5], [z, w, r, s, t], J5, 3) :$

> $Eq2a := \left\{z_{1,4} - z_{2,3} + z_{1,1} z_{2,2} - z_{1,2}^2 - w_{[\,]} + s[\,], w_{1,4} - w_{2,3} + z_{2,2} w_{1,1} - 2 z_{1,2} w_{1,2} + z_{1,1} w_{2,2}\right\} :$
$Eq2b := \left\{z_{1,5} - z_{3,3} + z_{1,1} z_{2,3} - z_{1,2} z_{1,3} - z_{1,1} w_{[\,]} + t[\,], w_{1,5} - w_{3,3} + z_{1,1} w_{2,3} + z_{2,3} w_{1,1} - z_{1,2} w_{1,3} - z_{1,3} w_{1,2} - w_{[\,]} w_{1,1} - w_1^2\right\} :$
$Eq2c := \left\{z_{2,5} - z_{3,4} + z_{1,2} z_{2,3} - z_{1,3} z_{2,2} - z_{1,2} w_{[\,]} + r_{[\,]}, w_{2,5} - w_{3,4} + z_{1,2} w_{2,3} + z_{2,3} w_{1,2} - z_{1,3} w_{2,2} - z_{2,2} w_{1,3} - w_{[\,]} w_{1,2} - w_1 w_2\right\} :$
$Eq2d := \left\{r_1 - \left(w_3 + z_{1,2} w_1 - z_{1,1} w_2\right), r_2 - \left(w_4 + z_{2,2} w_1 - z_{1,2} w_2\right), s_1, s_2, t_1, t_2\right\} :$

> $Eq2 := Eq2a$ **union** $Eq2b$ **union** $Eq2c$ **union** $Eq2d : sl2 := solve\left(Eq2, \left\{z_{1,4}, z_{1,5}, w_{1,4}, w_{1,5}, z_{2,5}, w_{2,5}, r_1, r_2, s_1, s_2, t_1, t_2\right\}\right) :$

> $V := evalDG\left(b1\left(var5, z_{[\,]}, w_{[\,]}, r_{[\,]}, s_{[\,]}, t_{[\,]}\right) D\_z[\,] + b2\left(var5, z_{[\,]}, w_{[\,]}, r_{[\,]}, s_{[\,]}, t_{[\,]}\right) D\_w[\,] + b3\left(var5, z_{[\,]}, w_{[\,]}, r_{[\,]}, s_{[\,]}, t_{[\,]}\right) D\_r[\,] + b4\left(var5, z_{[\,]}, w_{[\,]}, r_{[\,]}, s_{[\,]}, t_{[\,]}\right) D\_s[\,]\right.$

$+ b5(var5, z_{[\,]}, w_{[\,]}, r_{[\,]}, s_{[\,]}, t_{[\,]})\, D\_t[\,]) : V2 := Prolong(V, 2) :$

$> psl2 := pdsolve(\{seq(coeffs(expand(eval(LieDerivative(V2, Eq2[i]), sl2)), \{seq(z_i, i=1..5), seq(w_i, i=1..5), seq(r_i, i=1..5), seq(s_i, i=1..5), seq(t_i, i=1..5), seq(seq(z_{i,j}, j=i..5), i=1..5), seq(seq(w_{i,j}, j=i..5), i=1..5), seq(seq(r_{i,j}, j=i..5), i=1..5), seq(seq(s_{i,j}, j=i..5), i=1..5), seq(seq(t_{i,j}, j=i..5), i=1..5)\}), i=1..nops(Eq2))\})$

$$psl2 := \Big\{b1(x1, x2, x3, x4, x5, z[\,], w[\,], r[\,], s[\,], t[\,]) = f_3(x4, x5)\, x1 + f_6(x4, x5)\, x2\, x3 + f_7(x4, x5)\, x2 + f_5(x3, x4, x5),\ b2(x1, x2, x3, x4, x5, z[\,], w[\,], r[\,], s[\,], t[\,]) = f_6(x4, x5),\ b3(x1, x2, x3, x4, x5, z[\,], w[\,], r[\,], s[\,], t[\,]) = -\left(\frac{\partial}{\partial x5} f_6(x4, x5)\right) x3 - \frac{\partial}{\partial x5} f_7(x4, x5) + x2\left(\frac{\partial}{\partial x4} f_6(x4, x5)\right) + \frac{\partial^2}{\partial x3 \partial x4} f_5(x3, x4, x5),\ b4(x1, x2, x3, x4, x5, z[\,], w[\,], r[\,], s[\,], t[\,]) = -\frac{\partial}{\partial x4} f_3(x4, x5) + 2 f_6(x4, x5),\ b5(x1, x2, x3, x4, x5, z[\,], w[\,], r[\,], s[\,], t[\,]) = -\frac{\partial}{\partial x5} f_3(x4, x5) + \frac{\partial^2}{\partial x3^2} f_5(x3, x4, x5)\Big\} \quad (34)$$

>

S2.2.1b : reduction to the hierartchy of the second heavenly equation

$> DGsetup([var5], [z], J5, 3) :$

$> Eq2a := \{z_{1,4} - z_{2,3} + z_{1,1} z_{2,2} - z_{1,2}^2\} :$

$Eq2b := \{z_{1,5} - z_{3,3} + z_{1,1} z_{2,3} - z_{1,2} z_{1,3}\} :$

$Eq2c := \{z_{2,5} - z_{3,4} + z_{1,2} z_{2,3} - z_{1,3} z_{2,2}\} :$

$> Eq2 := Eq2a$ **union** $Eq2b$ **union** $Eq2c : sl2 := solve(Eq2, \{z_{1,4}, z_{1,5}, z_{2,5}\}) :$

$> Eq3 := \{seq(op(map(TotalDiff, Eq2, i)), i=1..5)\} : el3 := eliminate(eval(Eq3, sl2), \{seq(z_{1,i,4}, i=1..4), seq(z_{1,i,5}, i=1..5), seq(z_{2,i,5}, i=2..5)\}) : sl3 := el3[1] : el3[2]$

$$\emptyset \quad (35)$$

$> Eq4 := \{seq(seq(op(map(TotalDiff, Eq2, [i,j])), j=i..5), i=1..5)\} : el4 := eliminate(eval(eval(Eq4, sl3), sl2), \{seq(seq(z_{1,i,j,4}, j=i..4), i=1..4), seq(seq(z_{1,i,j,5}, j=i..5), i=1..5), seq(seq(z_{2,i,j,5}, j=i..5), i=2..5)\}) : sl4 := el4[1] : el4[2]$

$$\emptyset \quad (36)$$

>

S2.2.2: Construction 2

$> DGsetup([var5, q], M6) :$

$> V1 := evalDG(q\, D\_x1 - diff(u(var5), x1)\, D\_x3 - diff(v(var5), x1)\, D\_x4 + q\, diff(w(var5), x1)\, D\_q) :$

$V2 := evalDG(q\, D\_x2 - diff(u(var5), x2)\, D\_x3 - diff(v(var5), x2)\, D\_x4 + q\, diff(w(var5), x2)\, D\_q) :$

$V3 := evalDG(D\_x5 + diff(u(var5), x4)\, D\_x3 + (diff(v(var5), x4) + w(var5) - q)\, D\_x4 - q\, diff(w(var5), x4)\, D\_q) :$

> $Eq12 := map(coeffs, expand(ToJet(DGinfo(evalDG(LieDerivative(V1, V2) + diff(w(var5), x2)\ V1 - diff(w(var5), x1)\ V2), \text{"CoefficientSet"}), \{u(var5), v(var5), w(var5)\}, notation = jetnumbers)), \{q\});$
> $Eq13 := map(coeffs, expand(ToJet(DGinfo(evalDG(LieDerivative(V1, V3) - diff(w(var5), x4)\ V1), \text{"CoefficientSet"}), \{u(var5), v(var5), w(var5)\}, notation = jetnumbers)), \{q\});$
> $Eq23 := map(coeffs, expand(ToJet(DGinfo(evalDG(LieDerivative(V2, V3) - diff(w(var5), x4)\ V2), \text{"CoefficientSet"}), \{u(var5), v(var5), w(var5)\}, notation = jetnumbers)), \{q\})$

$$Eq12 := \{-u_1 w_{2,3} + u_2 w_{1,3} - w_{2,4} v_1 + v_2 w_{1,4}, u_1 u_{2,3} - u_1 w_2 - u_2 u_{1,3} + u_2 w_1 - v_2 u_{1,4} + v_1 u_{2,4}, u_1 v_{2,3} - u_2 v_{1,3} + v_1 v_{2,4} - v_1 w_2 - v_2 v_{1,4} + v_2 w_1\}$$

$$Eq13 := \{-u_1 u_{3,4} + u_1 w_4 + u_4 u_{1,3} + u_{1,4} v_4 + u_{1,4} w[\,] - u_{4,4} v_1 + u_{1,5}, -u_1 v_{3,4} - u_1 w_3 + u_4 v_{1,3} - v_1 v_{4,4} + v_4 v_{1,4} + v_{1,4} w[\,] + v_{1,5}, u_1 w_{3,4} - u_4 w_{1,3} + v_1 w_{4,4} - v_4 w_{1,4} - w_{1,4} w[\,] - w_1 w_4 - w_{1,5}\}$$

$$Eq23 := \{-u_2 u_{3,4} + u_2 w_4 + u_4 u_{2,3} + u_{2,4} v_4 + u_{2,4} w[\,] - u_{4,4} v_2 + u_{2,5}, -u_2 v_{3,4} - u_2 w_3 + u_4 v_{2,3} - v_2 v_{4,4} + v_4 v_{2,4} + v_{2,4} w[\,] + v_{2,5}, u_2 w_{3,4} - u_4 w_{2,3} + v_2 w_{4,4} - v_4 w_{2,4} - w_{2,4} w[\,] - w_2 w_4 - w_{2,5}\} \quad \textbf{(37)}$$

> $R1 := f \to u_1\, TotalDiff(f, [2, 3]) + v_1\, TotalDiff(f, [2, 4]) - u_2\, TotalDiff(f, [1, 3]) - v_2\, TotalDiff(f, [1, 4]) :$
> $R2 := f \to u_1\, TotalDiff(f, [3, 4]) + v_1\, TotalDiff(f, [4, 4]) - TotalDiff(f, [1, 5]) - u_4\, TotalDiff(f, [1, 3]) - (v_4 + w_{[\,]})\, TotalDiff(f, [1, 4]) :$
> $R3 := f \to u_2\, TotalDiff(f, [3, 4]) + v_2\, TotalDiff(f, [4, 4]) - TotalDiff(f, [2, 5]) - u_4\, TotalDiff(f, [2, 3]) - (v_4 + w_{[\,]})\, TotalDiff(f, [2, 4]) :$

> $DGsetup([var5], [u, v, w], J5, 4) :$

> $expand(R1(u_{[\,]}) - u_1 w_2 + u_2 w_1 - Eq12[2]), expand(R1(v_{[\,]}) - v_1 w_2 + v_2 w_1 - Eq12[3]), expand(R1(w_{[\,]}) + Eq12[1]);$
> $expand(R2(u_{[\,]}) - u_1 w_4 + Eq13[1]), expand(R2(v_{[\,]}) + u_1 w_3 + Eq13[2]), expand(R2(w_{[\,]}) - w_1 w_4 - Eq13[3]);$
> $expand(R3(u_{[\,]}) - u_2 w_4 + Eq23[1]), expand(R3(v_{[\,]}) + u_2 w_3 + Eq23[2]), expand(R3(w_{[\,]}) - w_2 w_4 - Eq23[3]);$

$$0, 0, 0$$
$$0, 0, 0$$
$$0, 0, 0 \quad \textbf{(38)}$$

> $Eq2 := Eq12\ \textbf{union}\ Eq13\ \textbf{union}\ Eq23 : el2 := eliminate(Eq2, \{u_{1,4}, u_{1,5}, u_{2,5}, v_{1,4}, v_{1,5}, v_{2,5}, w_{1,4}, w_{1,5}, w_{2,5}\}) : sl2 := el2[1] : el2[2]$

$$\varnothing \quad \textbf{(39)}$$

> $Eq3 := \{seq(op(map(TotalDiff, Eq2, i)), i = 1..5)\} : el3 := eliminate(Eq3, \{seq(u_{1,i,4}, i = 1..4), seq(u_{1,i,5}, i = 1..5), seq(u_{2,i,5}, i = 2..5), seq(v_{1,i,4}, i = 1..4), seq(v_{1,i,5}, i = 1..5), seq(v_{2,i,5}, i = 2..5), seq(w_{1,i,4}, i = 1..4), seq(w_{1,i,5}, i = 1..5), seq(w_{2,i,5}, i = 2..5)\}) :$
> $sl3 := el3[1] : simplify(eval(el3[2], sl2))$

$$\{0\} \quad \textbf{(40)}$$

> $Eq4 := \{seq(seq(op(map(TotalDiff, Eq2, [i,j])), j=i..5), i=1..5)\} : el4 := eliminate\big(Eq4, \{seq(seq(u_{1,i,j,4}, j=i..4), i=1..4), seq(seq(u_{1,i,j,5}, j=i..5), i=1..5), seq(seq(u_{2,i,j,5}, j=i..5), i=2..5), seq(seq(v_{1,i,j,4}, j=i..4), i=1..4), seq(seq(v_{1,i,j,5}, j=i..5), i=1..5), seq(seq(v_{2,i,j,5}, j=i..5), i=2..5), seq(seq(w_{1,i,j,4}, j=i..4), i=1..4), seq(seq(w_{1,i,j,5}, j=i..5), i=1..5), seq(seq(w_{2,i,j,5}, j=i..5), i=2..5)\}\big) : sl4 := el4[1] :$
$simplify(eval(eval(el4[2], sl3), sl2))$

$$\{0\} \tag{41}$$

> $Char := \{u_1\, p2\, p3 + v_1\, p2\, p4 - u_2\, p1\, p3 - v_2\, p1\, p4, u_1\, p3\, p4 + v_1\, p4^2 - p1\, p5 - u_4\, p1\, p3 - (v_4 + w_{[\,]})\, p1\, p4, u_2\, p3\, p4 + v_2\, p4^2 - p2\, p5 - u_4\, p2\, p3 - (v_4 + w_{[\,]})\, p2\, p4\} :$
$simplify\big(eval\big(Char, \{p1 = a\, u_1 + b\, v_1, p2 = a\, u_2 + b\, v_2, p3 = a\, q, p4 = b\, q, p5 = -a\, q\, u_4 - b\, q\, (v_4 + w_{[\,]}) + b\, q^2\}\big)\big)$

$$\{0\} \tag{42}$$

> $V := evalDG\big(b1(var5, u_{[\,]}, v_{[\,]}, w_{[\,]})\, D\_u[\,] + b2(var5, u_{[\,]}, v_{[\,]}, w_{[\,]})\, D\_v[\,] + b3(var5, u_{[\,]}, v_{[\,]}, w_{[\,]})\, D\_w[\,]\big) : V2 := Prolong(V, 2) :$

> $psl2 := pdsolve\big(\{seq\big(coeffs\big(expand(eval(LieDerivative(V2, Eq2[i]), sl2)), \{seq(u_i, i=1..5), seq(v_i, i=1..5), seq(w_i, i=1..5), seq(seq(u_{i,j}, j=i..5), i=1..5), seq(seq(v_{i,j}, j=i..5), i=1..5), seq(seq(w_{i,j}, j=i..5), i=1..5)\}\big), i=1..nops(Eq2)\big)\}\big)$

$$psl2 := \{b1(x1, x2, x3, x4, x5, u[\,], v[\,], w[\,]) = f_3(x3, x5), b2(x1, x2, x3, x4, x5, u[\,], v[\,], w[\,]) = f_1(x3, x5)\, x4 + f_2(x3, x5), b3(x1, x2, x3, x4, x5, u[\,], v[\,], w[\,]) = -f_1(x3, x5)\} \tag{43}$$

> $V := evalDG\big(a1(var5, u_{[\,]}, v_{[\,]}, w_{[\,]})\, D\_x1 + a2(var5, u_{[\,]}, v_{[\,]}, w_{[\,]})\, D\_x2 + a3(var5, u_{[\,]}, v_{[\,]}, w_{[\,]})\, D\_x3 + a4(var5, u_{[\,]}, v_{[\,]}, w_{[\,]})\, D\_x4 + a5(var5, u_{[\,]}, v_{[\,]}, w_{[\,]})\, D\_x5 + b1(var5, u_{[\,]}, v_{[\,]}, w_{[\,]})\, D\_u[\,] + b2(var5, u_{[\,]}, v_{[\,]}, w_{[\,]})\, D\_v[\,] + b3(var5, u_{[\,]}, v_{[\,]}, w_{[\,]})\, D\_w[\,]\big) :$
$V2 := Prolong(V, 2) :$

> $pdsys := \{seq\big(coeffs\big(expand(eval(LieDerivative(V2, Eq2[i]), sl2)), \{seq(u_i, i=1..5), seq(v_i, i=1..5), seq(w_i, i=1..5), seq(seq(u_{i,j}, j=i..5), i=1..5), seq(seq(v_{i,j}, j=i..5), i=1..5), seq(seq(w_{i,j}, j=i..5), i=1..5)\}\big), i=1..nops(Eq2)\big)\} : psl2 := pdsolve(pdsys)$

$$psl2 := \Big\{a1(x1, x2, x3, x4, x5, u[\,], v[\,], w[\,]) = f_1(x1, x2), a2(x1, x2, x3, x4, x5, u[\,], v[\,], w[\,]) = f_3(x1, x2), a3(x1, x2, x3, x4, x5, u[\,], v[\,], w[\,]) = f_4(x3, x5), a4(x1, x2, x3, x4, x5, u[\,], v[\,], w[\,]) = f_5(x3, x5)\, x4 + f_6(x3, x5), a5(x1, x2, x3, x4, x5, u[\,], v[\,], w[\,]) = f_2(x5), b1(x1, x2, x3, x4, x5, u[\,], v[\,], w[\,]) = \left(\frac{\partial}{\partial x5} f_4(x3, x5)\right) x4 + \left(-\frac{d}{dx5} f_2(x5) + f_5(x3, x5)\right. \tag{44}$$

$$+\frac{\partial}{\partial x3} f_4(x3,x5)\Big) u[\,] + f_7(x3,x5), b2(x1,x2,x3,x4,x5,u[\,],v[\,],w[\,]) = \Big(-\frac{d}{dx5}$$

$$f_2(x5) + 2 f_5(x3,x5)\Big) v[\,] + \Big(\Big(\frac{\partial}{\partial x3} f_5(x3,x5)\Big) x4 + \frac{\partial}{\partial x3} f_6(x3,x5)\Big) u[\,]$$

$$+ \frac{x4^2 \Big(2 \frac{\partial}{\partial x5} f_5(x3,x5) - \frac{d^2}{dx5^2} f_2(x5)\Big)}{2} + \Big(\frac{\partial}{\partial x5} f_6(x3,x5) - f_8(x3,x5)\Big) x4 + f_9(x3,$$

$$x5), b3(x1,x2,x3,x4,x5,u[\,],v[\,],w[\,]) = -\Big(\frac{\partial}{\partial x3} f_5(x3,x5)\Big) u[\,] + \Big(f_5(x3,x5) - \frac{d}{dx5}$$

$$f_2(x5)\Big) w[\,] + \Big(-\frac{\partial}{\partial x5} f_5(x3,x5) + \frac{d^2}{dx5^2} f_2(x5)\Big) x4 + f_8(x3,x5)\Big\}$$

# 1 arg:2, 11; 2 *arg* : 1, 3, 4, 5, 6, 7, 8, 9
thus the symmetry of the corresponding PDE system contains only (8) functions of 2 arguments, and so cannot change count of functions of 3 arguments in the solution space

```
> pdetest(psl2, pdsys)
```

$$\{0\} \quad (45)$$

```
>
```

S2.3.1

```
> var6 := seq(x||i, i=1..6) : DGsetup([var6, q], M7) :
> V1 := evalDG(D_x3 + (diff(v(var6), x1) - q) D_x1 + diff(u(var6), x1) D_x2
        + diff(w(var6), x1) D_q) :
  V2 := evalDG(D_x4 + diff(v(var6), x2) D_x1 + (diff(u(var6), x2) - q) D_x2
        + diff(w(var6), x2) D_q) :
  V3 := evalDG(D_x5 + (diff(v(var6), x3) - w(var6)) D_x1 + diff(u(var6), x3) D_x2
        - q D_x3 + diff(w(var6), x3) D_q) :
  V4 := evalDG(D_x6 + diff(v(var6), x4) D_x1 + (diff(u(var6), x4) - w(var6)) D_x2
        - q D_x4 + diff(w(var6), x4) D_q) :
> Eq12 := ToJet(DGinfo(LieDerivative(V1, V2), "CoefficientSet"), {u(var6), v(var6),
       w(var6)}, notation = jetnumbers);
  Eq13 := ToJet(DGinfo(evalDG(LieDerivative(V1, V3) + diff(w(var6), x1) V1),
       "CoefficientSet"), {u(var6), v(var6), w(var6)}, notation = jetnumbers);
  Eq23 := ToJet(DGinfo(evalDG(LieDerivative(V2, V3) + diff(w(var6), x2) V1),
       "CoefficientSet"), {u(var6), v(var6), w(var6)}, notation = jetnumbers);
  Eq14 := ToJet(DGinfo(evalDG(LieDerivative(V1, V4) + diff(w(var6), x1) V2),
       "CoefficientSet"), {u(var6), v(var6), w(var6)}, notation = jetnumbers);
  Eq24 := ToJet(DGinfo(evalDG(LieDerivative(V2, V4) + diff(w(var6), x2) V2),
       "CoefficientSet"), {u(var6), v(var6), w(var6)}, notation = jetnumbers);
  Eq34 := ToJet(DGinfo(evalDG(LieDerivative(V3, V4) - diff(w(var6), x4) V1
```

$+ diff(w(var6), x3)\ V2), \text{"CoefficientSet"}), \{u(var6), v(var6), w(var6)\}, notation = jetnumbers);$

$$Eq12 := \{u_1 w_{2,2} - u_2 w_{1,2} + v_1 w_{1,2} - v_2 w_{1,1} - w_{1,4} + w_{2,3}, u_1 u_{2,2} - u_2 u_{1,2} - v_2 u_{1,1} + u_{1,2} v_1 - u_{1,4} + u_{2,3} - w_1, u_1 v_{2,2} - u_2 v_{1,2} + v_1 v_{1,2} - v_2 v_{1,1} - v_{1,4} + v_{2,3} + w_2\}$$

$$Eq13 := \{u_1 u_{2,3} + u_1 w_1 - u_3 u_{1,2} - u_{1,1} v_3 + u_{1,1} w[\,] + u_{1,3} v_1 - u_{1,5} + u_{3,3}, u_1 v_{2,3} - u_1 w_2 - u_3 v_{1,2} + v_1 v_{1,3} - v_3 v_{1,1} + v_{1,1} w[\,] - v_{1,5} + v_{3,3}, u_1 w_{2,3} - u_3 w_{1,2} + v_1 w_{1,3} - v_3 w_{1,1} + w[\,] w_{1,1} + w_1^2 - w_{1,5} + w_{3,3}\}$$

$$Eq23 := \{w_2 (v_1 - q) - (v_3 - w[\,]) v_{1,2} - u_3 v_{2,2} + q v_{2,3} - v_{2,5} + v_2 (v_{1,3} - w_1) + (u_2 - q) (v_{2,3} - w_2) + v_{3,4} - w_4, u_2 w_{2,3} - u_3 w_{2,2} + v_2 w_{1,3} - v_3 w_{1,2} + w[\,] w_{1,2} + w_1 w_2 - w_{2,5} + w_{3,4}, u_1 w_2 + u_2 u_{2,3} - u_3 u_{2,2} - u_{1,2} v_3 + u_{1,2} w[\,] + u_{1,3} v_2 - u_{2,5} + u_{3,4} + w_3\}$$

$$Eq14 := \{w_1 (u_2 - q) - v_4 u_{1,1} - (u_4 - w[\,]) u_{1,2} + q u_{1,4} - u_{1,6} + (v_1 - q) (u_{1,4} - w_1) + u_1 (u_{2,4} - w_2) + u_{3,4} - w_3, u_1 w_{2,4} - u_4 w_{1,2} + v_1 w_{1,4} - v_4 w_{1,1} + w[\,] w_{1,2} + w_1 w_2 - w_{1,6} + w_{3,4}, u_1 v_{2,4} - u_4 v_{1,2} + v_1 v_{1,4} + v_2 w_1 - v_4 v_{1,1} + v_{1,2} w[\,] - v_{1,6} + v_{3,4} + w_4\}$$

$$Eq24 := \{u_2 u_{2,4} - u_4 u_{2,2} - u_{1,2} v_4 + u_{1,4} v_2 + u_{2,2} w[\,] - v_2 w_1 - u_{2,6} + u_{4,4}, u_2 v_{2,4} - u_4 v_{2,2} + v_2 v_{1,4} + v_2 w_2 - v_4 v_{1,2} + v_{2,2} w[\,] - v_{2,6} + v_{4,4}, u_2 w_{2,4} - u_4 w_{2,2} + v_2 w_{1,4} - v_4 w_{1,2} + w[\,] w_{2,2} + w_2^2 - w_{2,6} + w_{4,4}\}$$

$$Eq34 := \{w_3 w_2 - w_4 w_1 - v_4 w_{1,3} - (u_4 - w[\,]) w_{2,3} - w_{3,6} + (v_3 - w[\,]) w_{1,4} + u_3 w_{2,4} + w_{4,5}, -u_1 w_4 + u_2 w_3 + u_3 u_{2,4} - u_3 w_2 - u_4 u_{2,3} - u_{1,3} v_4 + u_{1,4} v_3 - u_{1,4} w[\,] + u_{2,3} w[\,] - v_3 w_1 + w[\,] w_1 - u_{3,6} + u_{4,5} - w_5, u_3 v_{2,4} - u_4 v_{2,3} + u_4 w_2 - v_1 w_4 + v_2 w_3 + v_3 v_{1,4} - v_4 v_{1,3} + v_4 w_1 - v_{1,4} w[\,] + v_{2,3} w[\,] - w[\,] w_2 - v_{3,6} + v_{4,5} + w_6\} \quad (46)$$

> $DGsetup([var6], [u, v, w], J6, 4):$

> $Q1 := f \to TotalDiff(f, [2, 3]) - TotalDiff(f, [1, 4]) + u_1\, TotalDiff(f, [2, 2]) + (v_1 - u_2)\, TotalDiff(f, [1, 2]) - v_2\, TotalDiff(f, [1, 1]):$

$Q2 := f \to TotalDiff(f, [3, 3]) - TotalDiff(f, [1, 5]) + u_1\, TotalDiff(f, [2, 3]) + v_1\, TotalDiff(f, [1, 3]) - u_3\, TotalDiff(f, [1, 2]) + (w_{[\,]} - v_3)\, TotalDiff(f, [1, 1]):$

$Q3 := f \to TotalDiff(f, [3, 4]) - TotalDiff(f, [2, 5]) + u_2\, TotalDiff(f, [2, 3]) + v_2\, TotalDiff(f, [1, 3]) - u_3\, TotalDiff(f, [2, 2]) + (w_{[\,]} - v_3)\, TotalDiff(f, [1, 2]):$

$Q4 := f \to TotalDiff(f, [3, 4]) - TotalDiff(f, [1, 6]) + u_1\, TotalDiff(f, [2, 4]) + v_1\, TotalDiff(f, [1, 4]) + (w_{[\,]} - u_4)\, TotalDiff(f, [1, 2]) - v_4\, TotalDiff(f, [1, 1]):$

$Q5 := f \to TotalDiff(f, [4, 4]) - TotalDiff(f, [2, 6]) + u_2\, TotalDiff(f, [2, 4]) + v_2\, TotalDiff(f, [1, 4]) + (w_{[\,]} - u_4)\, TotalDiff(f, [2, 2]) - v_4\, TotalDiff(f, [1, 2]):$

$Q6 := f \to TotalDiff(f, [4, 5]) - TotalDiff(f, [3, 6]) - (w_{[\,]} - v_3)\, TotalDiff(f, [1, 4]) + (w_{[\,]} - u_4)\, TotalDiff(f, [2, 3]) + u_3\, TotalDiff(f, [2, 4]) - v_4\, TotalDiff(f, [1, 3]):$

> $Eq2 := Eq12$ **union** $Eq13$ **union** $Eq23$ **union** $Eq14$ **union** $Eq24$ **union** $Eq34 : sl2 := solve(Eq2,$

$\{u_{1,4}, u_{1,5}, u_{1,6}, u_{2,5}, u_{2,6}, u_{3,6}, v_{1,4}, v_{1,5}, v_{1,6}, v_{2,5}, v_{2,6}, v_{3,6}, w_{1,4}, w_{1,5}, w_{1,6}, w_{2,5}, w_{2,6}, w_{3,6}\})$ :

> $EQ2 := \{Q1(u_{[\,]}) - w_1, Q1(v_{[\,]}) + w_2, Q1(w_{[\,]}), Q2(u_{[\,]}) + u_1 w_1, Q2(v_{[\,]}) - u_1 w_2, Q2(w_{[\,]}) + w_1^2, Q3(u_{[\,]}) + w_3 + u_1 w_2, Q3(v_{[\,]}) - w_4 - v_2 w_1 + (v_1 - u_2) w_2, Q3(w_{[\,]}) + w_1 w_2, Q4(u_{[\,]}) - w_3 - (v_1 - u_2) w_1 - u_1 w_2, Q4(v_{[\,]}) + w_4 + v_2 w_1, Q4(w_{[\,]}) + w_1 w_2, Q5(u_{[\,]}) - v_2 w_1, Q5(v_{[\,]}) + v_2 w_2, Q5(w_{[\,]}) + w_2^2, Q6(u_{[\,]}) - w_5 - (v_3 - w_{[\,]}) w_1 - u_1 w_4 + u_2 w_3 - u_3 w_2, Q6(v_{[\,]}) + w_6 - v_1 w_4 + v_2 w_3 - (w_{[\,]} - u_4) w_2 + v_4 w_1, Q6(w_{[\,]}) - w_1 w_4 + w_2 w_3\}$ : $sL2 := solve(EQ2, \{u_{1,4}, u_{1,5}, u_{1,6}, u_{2,5}, u_{2,6}, u_{3,6}, v_{1,4}, v_{1,5}, v_{1,6}, v_{2,5}, v_{2,6}, v_{3,6}, w_{1,4}, w_{1,5}, w_{1,6}, w_{2,5}, w_{2,6}, w_{3,6}\})$ :

> $simplify(eval(EQ2, sl2)), simplify(eval(Eq2, sL2))$

$$\{0\}, \{0\} \quad \textbf{(47)}$$

> $Char := [p2\,p3 - p1\,p4 + u_1\,p2^2 + v_1\,p1\,p2 - u_2\,p1\,p2 - v_2\,p1^2, p3^2 - p1\,p5 + u_1\,p2\,p3 + v_1\,p1\,p3 - u_3\,p1\,p2 + (w_{[\,]} - v_3)\,p1^2, p3\,p4 - p2\,p5 + u_2\,p2\,p3 + v_2\,p1\,p3 - u_3\,p2^2 + (w_{[\,]} - v_3)\,p1\,p2, p3\,p4 - p1\,p6 + u_1\,p2\,p4 + v_1\,p1\,p4 + (w_{[\,]} - u_4)\,p1\,p2 - v_4\,p1^2, p4^2 - p2\,p6 + u_2\,p2\,p4 + v_2\,p1\,p4 + (w_{[\,]} - u_4)\,p2^2 - v_4\,p1\,p2, p4\,p5 - p3\,p6 - (w_{[\,]} - v_3)\,p1\,p4 + (w_{[\,]} - u_4)\,p2\,p3 + u_3\,p2\,p4 - v_4\,p1\,p3]$ :

> $simplify(eval(Char, \{p1 = a, p2 = b, p3 = a\,q - b\,u_1, p4 = -a\,v_2 + b\cdot(v_1 - u_2 + q), p5 = a\cdot(w_{[\,]} - v_3 + q\,v_1 + 2\,q^2) - b\cdot(u_1\,v_1 + u_3 + q\,u_1), p6 = -a\,(v_1\,v_2 + v_4 + q\,v_2) + b\cdot(v_1^2 - u_2\,v_1 - u_4 + w_{[\,]} + q\cdot(2\,v_1 - u_2) + 2\,q^2)\}))$

$$[0, -a^2 q^2, -a\,b\,q^2, -a\,b\,q^2, -b^2 q^2, -q^2 (a^2 v_2 + b\,(u_2 - v_1)\,a - b^2 u_1)] \quad \textbf{(48)}$$

> $simplify(eval(Char, \{p1 = b, p2 = a, p3 = -a\,u_1 + b\cdot(q - v_1), p4 = a\cdot(q - u_2) - b\,v_2, p5 = -a\cdot(u_3 + q\,u_1) - b\cdot(v_3 + q\,v_1 - q^2 - w_{[\,]}), p6 = a\,(q^2 - q\,u_2 - u_4 + w[\,]) - b\,(q\,v_2 + v_4)\,\}))$

$$[0, 0, 0, 0, 0, 0] \quad \textbf{(49)}$$

> $Eq3 := \{seq(op(map(TotalDiff, Eq2, i)), i = 1..6)\}$ : $el3 := eliminate(eval(Eq3, sl2), \{seq(u_{1,i,4}, i = 1..4), seq(u_{1,i,5}, i = 1..5), seq(u_{1,i,6}, i = 1..6), seq(u_{2,i,5}, i = 2..5), seq(u_{2,i,6}, i = 2..6), seq(u_{3,i,6}, i = 3..6), seq(v_{1,i,4}, i = 1..4), seq(v_{1,i,5}, i = 1..5), seq(v_{1,i,6}, i = 1..6), seq(v_{2,i,5}, i = 2..5), seq(v_{2,i,6}, i = 2..6), seq(v_{3,i,6}, i = 3..6), seq(w_{1,i,4}, i = 1..4), seq(w_{1,i,5}, i = 1..5), seq(w_{1,i,6}, i = 1..6), seq(w_{2,i,5}, i = 2..5), seq(w_{2,i,6}, i = 2..6), seq(w_{3,i,6}, i = 3..6)\})$ : $sl3 := el3[1]$ : $el3[2]$

$$\varnothing \quad \textbf{(50)}$$

> $Eq4 := \{seq(seq(op(map(TotalDiff, Eq2, [i,j])), j = i..6), i = 1..6)\}$ : $el4 := eliminate(eval(eval(Eq4, sl3), sl2), \{seq(seq(u_{1,i,j,4}, j = i..4), i = 1..4), seq(seq(u_{1,i,j,5}, j = i..5), i = 1..5), seq(seq(u_{1,i,j,6}, j = i..6), i = 1..6), seq(seq(u_{2,i,j,5}, j = i..5), i = 2..5), seq(seq(u_{2,i,j,6}, j = i..6), i = 2..6), seq(seq(u_{3,i,j,6}, j = i..6), i = 3..6), seq(seq(v_{1,i,j,4}, j = i..4), i = 1..4), seq(seq(v_{1,i,j,5}, j = i..5), i = 1..5), seq(seq(v_{1,i,j,6}, j = i..6), i = 1..6), seq(seq(v_{2,i,j,5}, j = i..5), i = 2..5), seq(seq(v_{2,i,j,6}, j = i..6), i = 2..6), seq(seq(v_{3,i,j,6}, j = i$

$..6), i=3..6), seq(seq(w_{1,i,j,4}, j=i..4), i=1..4), seq(seq(w_{1,i,j,5}, j=i..5), i=1..5), seq(seq(w_{1,i,j,6}, j=i..6), i=1..6), seq(seq(w_{2,i,j,5}, j=i..5), i=2..5), seq(seq(w_{2,i,j,6}, j=i..6), i=2..6), seq(seq(w_{3,i,j,6}, j=i..6), i=3..6)\}) : sl4 := el4[1] : el4[2]$

$$\varnothing \quad \textbf{(51)}$$

> $V := evalDG(b1(var6, u_{[\,]}, v_{[\,]}, w_{[\,]})\, D\_u[\,] + b2(var6, u_{[\,]}, v_{[\,]}, w_{[\,]})\, D\_v[\,] + b3(var6, u_{[\,]}, v_{[\,]}, w_{[\,]})\, D\_w[\,]) : V2 := Prolong(V, 2) :$

> $psl2 := pdsolve(\{seq(coeffs(expand(eval(LieDerivative(V2, Eq2[i]), sl2)), \{seq(u_i, i=1..6), seq(v_i, i=1..6), seq(w_i, i=1..6), seq(seq(u_{i,j}, j=i..6), i=1..6), seq(seq(v_{i,j}, j=i..6), i=1..6), seq(seq(w_{i,j}, j=i..6), i=1..6)\}), i=1..nops(Eq2))\})$

$$psl2 := \{b1(x1, x2, x3, x4, x5, x6, u[\,], v[\,], w[\,]) = f_1(x5, x6)\, x4 + f_2(x5, x6), b2(x1, x2, x3, x4, x5, x6, u[\,], v[\,], w[\,]) = f_1(x5, x6)\, x3 + f_3(x5, x6), b3(x1, x2, x3, x4, x5, x6, u[\,], v[\,], w[\,]) = f_1(x5, x6)\} \quad \textbf{(52)}$$

> $V := evalDG(a1(var6, u_{[\,]}, v_{[\,]}, w_{[\,]})\, D\_x1 + a2(var6, u_{[\,]}, v_{[\,]}, w_{[\,]})\, D\_x2 + a3(var6, u_{[\,]}, v_{[\,]}, w_{[\,]})\, D\_x3 + a4(var6, u_{[\,]}, v_{[\,]}, w_{[\,]})\, D\_x4 + a5(var6, u_{[\,]}, v_{[\,]}, w_{[\,]})\, D\_x5 + a6(var6, u_{[\,]}, v_{[\,]}, w_{[\,]})\, D\_x6 + b1(var6, u_{[\,]}, v_{[\,]}, w_{[\,]})\, D\_u[\,] + b2(var6, u_{[\,]}, v_{[\,]}, w_{[\,]})\, D\_v[\,] + b3(var6, u_{[\,]}, v_{[\,]}, w_{[\,]})\, D\_w[\,]) : V2 := Prolong(V, 2) :$

> $pdsys := \{seq(coeffs(expand(eval(LieDerivative(V2, Eq2[i]), sl2)), \{seq(u_i, i=1..6), seq(v_i, i=1..6), seq(w_i, i=1..6), seq(seq(u_{i,j}, j=i..6), i=1..6), seq(seq(v_{i,j}, j=i..6), i=1..6), seq(seq(w_{i,j}, j=i..6), i=1..6)\}), i=1..nops(Eq2))\} : psl2 := pdsolve(pdsys)$

$$psl2 := \Big\{ a1(x1, x2, x3, x4, x5, x6, u[\,], v[\,], w[\,]) = \left(\frac{\partial}{\partial x6} f_2(x5, x6)\right) x2 + \left(2 f_3(x5, x6) + \frac{\partial}{\partial x5} f_2(x5, x6) - 2 \frac{\partial}{\partial x6} f_1(x5, x6)\right) x1 + \frac{\left(\frac{\partial^2}{\partial x6^2} f_2(x5, x6)\right) x4^2}{2} + \left(x3 \left(\frac{\partial}{\partial x6} f_3(x5, x6)\right) + x3 \left(\frac{\partial^2}{\partial x5 \partial x6} f_2(x5, x6)\right) - x3 \left(\frac{\partial^2}{\partial x6^2} f_1(x5, x6)\right) + \frac{\partial}{\partial x6} f_5(x5, x6)\right) x4 + \frac{\left(2 \frac{\partial}{\partial x5} f_3(x5, x6) + \frac{\partial^2}{\partial x5^2} f_2(x5, x6) - 2 \frac{\partial^2}{\partial x5 \partial x6} f_1(x5, x6)\right) x3^2}{2} + f_6(x5, x6)\, x3 + f_7(x5, x6), a2(x1, x2, x3, x4, x5, x6, u[\,], v[\,], w[\,]) = \left(\frac{\partial}{\partial x5} f_1(x5, x6)\right) x1 + \left(-\frac{\partial}{\partial x6} f_1(x5, x6) + 2 f_3(x5, x6)\right) x2 + \frac{\left(\frac{\partial^2}{\partial x5^2} f_1(x5, x6)\right) x3^2}{2} + \left(\left(\frac{\partial}{\partial x5} f_3(x5, x6)\right) x4 + \frac{\partial}{\partial x5} \quad \textbf{(53)}$$

$$f_4(x5, x6)\Big) x3 + \frac{x4^2 \left(2 \frac{\partial}{\partial x6} f_3(x5, x6) - \frac{\partial^2}{\partial x6^2} f_1(x5, x6)\right)}{2} + \Big(f_6(x5, x6) - \frac{\partial}{\partial x5} f_5(x5,$$

$$x6) + \frac{\partial}{\partial x6} f_4(x5, x6)\Big) x4 + f_9(x5, x6), a3(x1, x2, x3, x4, x5, x6, u[\,], v[\,], w[\,]) = \Big(\frac{\partial}{\partial x6}$$

$$f_2(x5, x6)\Big) x4 + \left(f_3(x5, x6) + \frac{\partial}{\partial x5} f_2(x5, x6) - \frac{\partial}{\partial x6} f_1(x5, x6)\right) x3 + f_5(x5, x6), a4(x1,$$

$$x2, x3, x4, x5, x6, u[\,], v[\,], w[\,]) = \left(\frac{\partial}{\partial x5} f_1(x5, x6)\right) x3 + f_3(x5, x6)\, x4 + f_4(x5, x6),$$

$$a5(x1, x2, x3, x4, x5, x6, u[\,], v[\,], w[\,]) = f_2(x5, x6), a6(x1, x2, x3, x4, x5, x6, u[\,], v[\,], w[\,])$$

$$= f_1(x5, x6), b1(x1, x2, x3, x4, x5, x6, u[\,], v[\,], w[\,]) = \left(\frac{\partial}{\partial x5} f_1(x5, x6)\right) v[\,] + \Big(-2 \frac{\partial}{\partial x6}$$

$$f_1(x5, x6) + 3 f_3(x5, x6)\Big) u[\,] + \Big(\Big(\left(\frac{\partial^2}{\partial x5^2} f_1(x5, x6)\right) x3 + \left(\frac{\partial}{\partial x5} f_3(x5, x6)\right) x4 + \frac{\partial}{\partial x5}$$

$$f_4(x5, x6)\Big) x1 + \Big(2\, x3 \left(\frac{\partial}{\partial x5} f_3(x5, x6)\right) - \left(\frac{\partial^2}{\partial x5 \partial x6} f_1(x5, x6)\right) x3 + 3 \Big(\frac{\partial}{\partial x6} f_3(x5,$$

$$x6)\Big) x4 - 2 \left(\frac{\partial^2}{\partial x6^2} f_1(x5, x6)\right) x4 + 2 f_6(x5, x6) - 2 \frac{\partial}{\partial x5} f_5(x5, x6) + \frac{\partial}{\partial x6} f_4(x5, x6)\Big)$$

$$x2 + \frac{\left(\frac{\partial^3}{\partial x5^3} f_1(x5, x6)\right) x3^3}{6} + \frac{\left(\left(\frac{\partial^2}{\partial x5^2} f_3(x5, x6)\right) x4 + \frac{\partial^2}{\partial x5^2} f_4(x5, x6)\right) x3^2}{2}$$

$$+ \Bigg(x4^2 \left(\frac{\partial^2}{\partial x5 \partial x6} f_3(x5, x6)\right) - \frac{x4^2 \left(\frac{\partial^3}{\partial x5 \partial x6^2} f_1(x5, x6)\right)}{2} + x4 \left(\frac{\partial^2}{\partial x5 \partial x6} f_4(x5, x6)\right)$$

$$- x4 \left(\frac{\partial^2}{\partial x5^2} f_5(x5, x6)\right) + x4 \left(\frac{\partial}{\partial x5} f_6(x5, x6)\right) + \frac{\partial}{\partial x5} f_9(x5, x6)\Bigg) x3$$

$$+ \frac{\left(3 \frac{\partial^2}{\partial x6^2} f_{3}(x5, x6) - 2 \frac{\partial^3}{\partial x6^3} f_{1}(x5, x6)\right) x4^3}{6}$$

$$+ \frac{\left(-2 \frac{\partial^2}{\partial x5 \partial x6} f_{5}(x5, x6) + 2 \frac{\partial}{\partial x6} f_{6}(x5, x6) + \frac{\partial^2}{\partial x6^2} f_{4}(x5, x6)\right) x4^2}{2} + \left(\frac{\partial}{\partial x6} f_{9}(x5,\right.$$

$$\left. x6) + f_{8}(x5, x6)\right) x4 + f_{11}(x5, x6), b2(x1, x2, x3, x4, x5, x6, u[\ ], v[\ ], w[\ ]) = \left(\frac{\partial}{\partial x6} f_{2}(x5,\right.$$

$$\left. x6)\right) u[\ ] + \left(3 f_{3}(x5, x6) + \frac{\partial}{\partial x5} f_{2}(x5, x6) - 3 \frac{\partial}{\partial x6} f_{1}(x5, x6)\right) v[\ ] + \left(\left(\frac{\partial^2}{\partial x6^2} f_{2}(x5,\right.\right.$$

$$\left. x6)\right) x4 + x3 \left(\frac{\partial}{\partial x6} f_{3}(x5, x6)\right) + x3 \left(\frac{\partial^2}{\partial x5 \partial x6} f_{2}(x5, x6)\right) - x3 \left(\frac{\partial^2}{\partial x6^2} f_{1}(x5, x6)\right)$$

$$\left. + \frac{\partial}{\partial x6} f_{5}(x5, x6)\right) x2 + \left(3\, x3 \left(\frac{\partial}{\partial x5} f_{3}(x5, x6)\right) + x3 \left(\frac{\partial^2}{\partial x5^2} f_{2}(x5, x6)\right) - 3 \left(\frac{\partial^2}{\partial x5 \partial x6}\right.\right.$$

$$\left. f_{1}(x5, x6)\right) x3 + 2 \left(\frac{\partial}{\partial x6} f_{3}(x5, x6)\right) x4 + \left(\frac{\partial^2}{\partial x5 \partial x6} f_{2}(x5, x6)\right) x4 - 2 \left(\frac{\partial^2}{\partial x6^2} f_{1}(x5,\right.$$

$$\left.\left. x6)\right) x4 + 2 f_{6}(x5, x6) - \frac{\partial}{\partial x5} f_{5}(x5, x6)\right) x1 + \frac{\left(\frac{\partial^3}{\partial x6^3} f_{2}(x5, x6)\right) x4^3}{6}$$

$$+ \frac{1}{2} \left(\left(x3 \left(\frac{\partial^2}{\partial x6^2} f_{3}(x5, x6)\right) + x3 \left(\frac{\partial^3}{\partial x5 \partial x6^2} f_{2}(x5, x6)\right) - x3 \left(\frac{\partial^3}{\partial x6^3} f_{1}(x5, x6)\right)\right.\right.$$

$$\left.\left. + \frac{\partial^2}{\partial x6^2} f_{5}(x5, x6)\right) x4^2\right) + \left( x3^2 \left(\frac{\partial^2}{\partial x5 \partial x6} f_{3}(x5, x6)\right) - x3^2 \left(\frac{\partial^3}{\partial x5 \partial x6^2} f_{1}(x5, x6)\right)\right.$$

$$\left. + \frac{x3^2 \left(\frac{\partial^3}{\partial x5^2 \partial x6} f_{2}(x5, x6)\right)}{2} + \left(\frac{\partial}{\partial x6} f_{6}(x5, x6)\right) x3 + \frac{\partial}{\partial x6} f_{7}(x5, x6)\right) x4$$

$$+ \frac{\left(3 \frac{\partial^2}{\partial x5^2} f_{3}(x5, x6) - 3 \frac{\partial^3}{\partial x5^2 \partial x6} f_{1}(x5, x6) + \frac{\partial^3}{\partial x5^3} f_{2}(x5, x6)\right) x3^3}{6}$$

$$+\frac{\left(-2\frac{\partial^2}{\partial x5^2}f_5(x5,x6)+4\frac{\partial}{\partial x5}f_6(x5,x6)\right)x3^2}{4}+\left(f_8(x5,x6)+\frac{\partial}{\partial x5}f_7(x5,x6)\right)x3$$

$$+f_{10}(x5,x6),\ b3(x1,x2,x3,x4,x5,x6,u[\,],v[\,],w[\,])=2\left(f_3(x5,x6)-\frac{\partial}{\partial x6}f_1(x5,\right.$$

$$\left.x6)\right)w[\,]+\left(\frac{\partial}{\partial x5}f_3(x5,x6)-\frac{\partial^2}{\partial x5\partial x6}f_1(x5,x6)\right)x1+\left(\frac{\partial}{\partial x6}f_3(x5,x6)-\frac{\partial^2}{\partial x6^2}f_1(x5,\right.$$

$$\left.x6)\right)x2+\frac{x3^2\left(\frac{\partial^2}{\partial x5^2}f_3(x5,x6)-\frac{\partial^3}{\partial x5^2\partial x6}f_1(x5,x6)\right)}{2}+\left(x4\left(\frac{\partial^2}{\partial x5\partial x6}f_3(x5,x6)\right)\right.$$

$$\left.-x4\left(\frac{\partial^3}{\partial x5\partial x6^2}f_1(x5,x6)\right)-\frac{\partial^2}{\partial x5^2}f_5(x5,x6)+\frac{\partial}{\partial x5}f_6(x5,x6)\right)x3$$

$$+\frac{x4^2\left(\frac{\partial^2}{\partial x6^2}f_3(x5,x6)-\frac{\partial^3}{\partial x6^3}f_1(x5,x6)\right)}{2}+\left(-\frac{\partial^2}{\partial x5\partial x6}f_5(x5,x6)+\frac{\partial}{\partial x6}f_6(x5,\right.$$

$$\left.x6)\right)x4+f_8(x5,x6)\Big\}$$

# 2 *arg* : 1, 2, 3, 4, 5, 6, 7, 8, 9, 10, 11
thus the symmetry of the corresponding PDE system contains only (11) functions of 2 arguments, and so cannot change count of functions of 3 arguments in the solution space

```
> pdetest(psl2, pdsys)
```

$$\{0\} \quad (54)$$

```
>
```

S2.3.2

```
> var6 := seq(x||i, i=1..6) : DGsetup([var6, q], M7) :
> V1 := evalDG(q D_x1 - diff(u(var6), x1) D_x3 - diff(v(var6), x1) D_x4 + q diff(w(var6),
     x1) D_q) :
  V2 := evalDG(q D_x2 - diff(u(var6), x2) D_x3 - diff(v(var6), x2) D_x4 + q diff(w(var6),
     x2) D_q) :
  V3 := evalDG(D_x5 + diff(u(var6), x4) D_x3 + (diff(v(var6), x4) + w(var6) - q) D_x4
      - q diff(w(var6), x4) D_q) :
  V4 := evalDG(D_x6 + (diff(u(var6), x3) + w(var6) - q) D_x3 + diff(v(var6), x3) D_x4
      - q diff(w(var6), x3) D_q) :
> Eq12 := map(coeffs, expand(ToJet(DGinfo(evalDG(LieDerivative(V1, V2) + diff(w(var6),
     x2) V1 - diff(w(var6), x1) V2), "CoefficientSet"), {u(var6), v(var6), w(var6)}, notation
      =jetnumbers)), {q});
  Eq13 := map(coeffs, expand(ToJet(DGinfo(evalDG(LieDerivative(V1, V3) - diff(w(var6),
     x4) V1), "CoefficientSet"), {u(var6), v(var6), w(var6)}, notation =jetnumbers)), {q});
```

$Eq23 := map(coeffs, expand(ToJet(DGinfo(evalDG(LieDerivative(V2, V3) - diff(w(var6), x4)\ V2), "CoefficientSet"), \{u(var6), v(var6), w(var6)\}, notation = jetnumbers)), \{q\});$
$Eq14 := map(coeffs, expand(ToJet(DGinfo(evalDG(LieDerivative(V1, V4) - diff(w(var6), x3)\ V1), "CoefficientSet"), \{u(var6), v(var6), w(var6)\}, notation = jetnumbers)), \{q\});$
$Eq24 := map(coeffs, expand(ToJet(DGinfo(evalDG(LieDerivative(V2, V4) - diff(w(var6), x3)\ V2), "CoefficientSet"), \{u(var6), v(var6), w(var6)\}, notation = jetnumbers)), \{q\});$
$Eq34 := map(coeffs, expand(ToJet(DGinfo(evalDG(LieDerivative(V3, V4)), "CoefficientSet"), \{u(var6), v(var6), w(var6)\}, notation = jetnumbers)), \{q\});$

$$Eq12 := \{-u_1 w_{2,3} + u_2 w_{1,3} - w_{2,4} v_1 + v_2 w_{1,4}, u_1 u_{2,3} - u_1 w_2 - u_2 u_{1,3} + u_2 w_1 - v_2 u_{1,4} + u_{2,4} v_1, u_1 v_{2,3} - u_2 v_{1,3} + v_1 v_{2,4} - v_1 w_2 - v_2 v_{1,4} + v_2 w_1\}$$

$$Eq13 := \{-u_1 u_{3,4} + u_1 w_4 + u_4 u_{1,3} + u_{1,4} v_4 + u_{1,4} w[\,] - u_{4,4} v_1 + u_{1,5}, -u_1 v_{3,4} - u_1 w_3 + u_4 v_{1,3} - v_1 v_{4,4} + v_4 v_{1,4} + v_{1,4} w[\,] + v_{1,5}, u_1 w_{3,4} - u_4 w_{1,3} + v_1 w_{4,4} - v_4 w_{1,4} - w_{1,4} w[\,] - w_1 w_4 - w_{1,5}\}$$

$$Eq23 := \{-u_2 u_{3,4} + u_2 w_4 + u_4 u_{2,3} + u_{2,4} v_4 + u_{2,4} w[\,] - v_2 u_{4,4} + u_{2,5}, -u_2 v_{3,4} - u_2 w_3 + u_4 v_{2,3} - v_2 v_{4,4} + v_4 v_{2,4} + v_{2,4} w[\,] + v_{2,5}, u_2 w_{3,4} - u_4 w_{2,3} + v_2 w_{4,4} - v_4 w_{2,4} - w_{2,4} w[\,] - w_2 w_4 - w_{2,5}\}$$

$$Eq14 := \{-u_1 u_{3,3} + u_3 u_{1,3} + u_{1,3} w[\,] + u_{1,4} v_3 - u_{3,4} v_1 - v_1 w_4 + u_{1,6}, -u_1 v_{3,3} + u_3 v_{1,3} - v_1 v_{3,4} + v_1 w_3 + v_3 v_{1,4} + v_{1,3} w[\,] + v_{1,6}, u_1 w_{3,3} - u_3 w_{1,3} + v_1 w_{3,4} - v_3 w_{1,4} - w[\,] w_{1,3} - w_1 w_3 - w_{1,6}\}$$

$$Eq24 := \{-u_2 u_{3,3} + u_3 u_{2,3} + u_{2,3} w[\,] + u_{2,4} v_3 - u_{3,4} v_2 - v_2 w_4 + u_{2,6}, -u_2 v_{3,3} + u_3 v_{2,3} - v_2 v_{3,4} + v_2 w_3 + v_3 v_{2,4} + v_{2,3} w[\,] + v_{2,6}, u_2 w_{3,3} - u_3 w_{2,3} + v_2 w_{3,4} - v_3 w_{2,4} - w[\,] w_{2,3} - w_2 w_3 - w_{2,6}\}$$

$$Eq34 := \{u_3 w_{3,4} - u_4 w_{3,3} + v_3 w_{4,4} - v_4 w_{3,4} - w_{3,5} + w_{4,6}, -u_3 u_{3,4} + u_4 u_{3,3} + u_4 w_3 + u_{3,4} v_4 - u_{4,4} v_3 + v_4 w_4 + w[\,] w_4 + u_{3,5} - u_{4,6} + w_5, -u_3 v_{3,4} - u_3 w_3 + u_4 v_{3,3} - v_3 v_{4,4} - v_3 w_4 + v_4 v_{3,4} - w[\,] w_3 + v_{3,5} - v_{4,6} - w_6\} \quad (55)$$

> $R1 := f \to u_1\, TotalDiff(f, [2, 3]) + v_1\, TotalDiff(f, [2, 4]) - u_2\, TotalDiff(f, [1, 3]) - v_2\, TotalDiff(f, [1, 4]):$

$R2 := f \to u_1\, TotalDiff(f, [3, 4]) + v_1\, TotalDiff(f, [4, 4]) - TotalDiff(f, [1, 5]) - u_4\, TotalDiff(f, [1, 3]) - (v_4 + w_{[\,]})\, TotalDiff(f, [1, 4]):$

$R3 := f \to u_2\, TotalDiff(f, [3, 4]) + v_2\, TotalDiff(f, [4, 4]) - TotalDiff(f, [2, 5]) - u_4\, TotalDiff(f, [2, 3]) - (v_4 + w_{[\,]})\, TotalDiff(f, [2, 4]):$

$R4 := f \to v_1\, TotalDiff(f, [3, 4]) + u_1\, TotalDiff(f, [3, 3]) - TotalDiff(f, [1, 6]) - v_3\, TotalDiff(f, [1, 4]) - (u_3 + w_{[\,]})\, TotalDiff(f, [1, 3]):$

$R5 := f \to v_2\, TotalDiff(f, [3, 4]) + u_2\, TotalDiff(f, [3, 3]) - TotalDiff(f, [2, 6]) - v_3\, TotalDiff(f, [2, 4]) - (u_3 + w_{[\,]})\, TotalDiff(f, [2, 3]):$

$R6 := f \to TotalDiff(f, [3, 5]) - TotalDiff(f, [4, 6]) + u_4\, TotalDiff(f, [3, 3])$

$- v_3\ TotalDiff(f, [4, 4]) + (v_4 - u_3)\ TotalDiff(f, [3, 4])$ :

> $DGsetup([var6], [u, v, w], J6, 4)$ :

> $expand(R1(u_{[\,]}) - u_1 w_2 + u_2 w_1 - Eq12[2]), expand(R1(v_{[\,]}) - v_1 w_2 + v_2 w_1 - Eq12[3]), expand(R1(w_{[\,]}) + Eq12[1]),$
$expand(R2(u_{[\,]}) - u_1 w_4 + Eq13[1]), expand(R2(v_{[\,]}) + u_1 w_3 + Eq13[2]), expand(R2(w_{[\,]}) - w_1 w_4 - Eq13[3]),$
$expand(R3(u_{[\,]}) - u_2 w_4 + Eq23[1]), expand(R3(v_{[\,]}) + u_2 w_3 + Eq23[2]), expand(R3(w_{[\,]}) - w_2 w_4 - Eq23[3]),$
$expand(R4(u_{[\,]}) + v_1 w_4 + Eq14[1]), expand(R4(v_{[\,]}) - v_1 w_3 + Eq14[2]), expand(R4(w_{[\,]}) - w_1 w_3 - Eq14[3]),$
$expand(R5(u_{[\,]}) + v_2 w_4 + Eq24[1]), expand(R5(v_{[\,]}) - v_2 w_3 + Eq24[2]), expand(R5(w_{[\,]}) - w_2 w_3 - Eq24[3]),$
$expand(R6(u_{[\,]}) + w_5 + (v_4 + w_{[\,]}) w_4 + u_4 w_3 - Eq34[2]), expand(R6(v_{[\,]}) - w_6 - (u_3 + w_{[\,]}) w_3 - v_3 w_4 - Eq34[3]), expand(R6(w_{[\,]}) + Eq34[1])$

$$0, 0, 0, 0, 0, 0, 0, 0, 0, 0, 0, 0, 0, 0, 0, 0, 0, 0 \quad (56)$$

> $Eq2 := Eq12$ **union** $Eq13$ **union** $Eq23$ **union** $Eq14$ **union** $Eq24$ **union** $Eq34$ : $el2 := eliminate(Eq2, \{u_{1,4}, u_{1,5}, u_{1,6}, u_{2,5}, u_{2,6}, u_{3,5}, v_{1,4}, v_{1,5}, v_{1,6}, v_{2,5}, v_{2,6}, v_{3,5}, w_{1,4}, w_{1,5}, w_{1,6}, w_{2,5}, w_{2,6}, w_{3,5}\})$ : $sl2 := el2[1] : el2[2]$

$$\varnothing \quad (57)$$

> $Char := \{u_1\, p2\, p3 + v_1\, p2\, p4 - u_2\, p1\, p3 - v_2\, p1\, p4, u_1\, p3\, p4 + v_1\, p4^2 - p1\, p5 - u_4\, p1\, p3 - (v_4 + w_{[\,]})\, p1\, p4, u_2\, p3\, p4 + v_2\, p4^2 - p2\, p5 - u_4\, p2\, p3 - (v_4 + w_{[\,]})\, p2\, p4, v_1\, p3\, p4 + u_1\, p3^2 - p1\, p6 - v_3\, p1\, p4 - (u_3 + w_{[\,]})\, p1\, p3, v_2\, p3\, p4 + u_2\, p3^2 - p2\, p6 - v_3\, p2\, p4 - (u_3 + w_{[\,]})\, p2\, p3, p3\, p5 - p4\, p6 + u_4\, p3^2 - v_3\, p4^2 + (v_4 - u_3)\, p3\, p4\}$ :
$simplify(eval(Char, \{p1 = a\, u_1 + b\, v_1, p2 = a\, u_2 + b\, v_2, p3 = a\, q, p4 = b\, q, p5 = -a\, q\, u_4 - b\, q\, (v_4 + w_{[\,]}) + b\, q^2, p6 = -a\, q\, (u_3 + w_{[\,]}) + a\, q^2 - b\, q\, v_3\}))$

$$\{0\} \quad (58)$$

> $Eq3 := \{seq(op(map(TotalDiff, Eq2, i)), i = 1..6)\}$ : $el3 := eliminate(eval(Eq3, sl2), \{seq(u_{1,i,4}, i = 1..4), seq(u_{1,i,5}, i = 1..5), seq(u_{1,i,6}, i = 1..6), seq(u_{2,i,5}, i = 2..5), seq(u_{2,i,6}, i = 2..6), seq(u_{3,i,5}, i = 3..5), u_{3,5,6}, seq(v_{1,i,4}, i = 1..4), seq(v_{1,i,5}, i = 1..5), seq(v_{1,i,6}, i = 1..6), seq(v_{2,i,5}, i = 2..5), seq(v_{2,i,6}, i = 2..6), seq(v_{3,i,5}, i = 3..5), v_{3,5,6}, seq(w_{1,i,4}, i = 1..4), seq(w_{1,i,5}, i = 1..5), seq(w_{1,i,6}, i = 1..6), seq(w_{2,i,5}, i = 2..5), seq(w_{2,i,6}, i = 2..6), seq(w_{3,i,5}, i = 3..5), w_{3,5,6}\})$ : $sl3 := el3[1] : el3[2]$

$$\varnothing \quad (59)$$

> $Eq4 := \{seq(seq(op(map(TotalDiff, Eq2, [i, j])), j = i..6), i = 1..6)\}$ : $el4 := eliminate(eval(eval(Eq4, sl3), sl2), \{seq(seq(u_{1,i,j,4}, j = i..4), i = 1..4), seq(seq(u_{1,i,j,5}, j = i..5), i = 1..5), seq(seq(u_{1,i,j,6}, j = i..6), i = 1..6), seq(seq(u_{2,i,j,5}, j = i..5), i = 2..5), seq(seq(u_{2,i,j,6}, j = i..6), i = 2..6), seq(seq(u_{3,i,j,5}, j = i..5), i = 3..5), seq(u_{3,i,5,6}, i = 3..5), u_{3,5,6,6}, seq(seq(v_{1,i,j,4}, j = i..4), i = 1..4), seq(seq(v_{1,i,j,5}, j = i..5), i = 1..5), seq(seq(v_{1,i,j,6}, j = i..6), i = 1..6), seq(seq(v_{2,i,j,5}, j = i..5), i = 2..5), seq(seq(v_{2,i,j,6}, j = i$

$..6), i=2..6), seq(seq(v_{3,i,j,5}, j=i..5), i=3..5), seq(v_{3,i,5,6}, i=3..5), v_{3,5,6,6}, seq(seq(w_{1,i,j,4}, j=i..4), i=1..4), seq(seq(w_{1,i,j,5}, j=i..5), i=1..5), seq(seq(w_{1,i,j,6}, j=i..6), i=1..6), seq(seq(w_{2,i,j,5}, j=i..5), i=2..5), seq(seq(w_{2,i,j,6}, j=i..6), i=2..6), seq(seq(w_{3,i,j,5}, j=i..5), i=3..5), seq(w_{3,i,5,6}, i=3..5), w_{3,5,6,6}\}) : sl4 := el4[1] : el4[2]$

$$\varnothing \tag{60}$$

> $V := evalDG(b1(var6, u_{[\,]}, v_{[\,]}, w_{[\,]})\ D\_u[\,] + b2(var6, u_{[\,]}, v_{[\,]}, w_{[\,]})\ D\_v[\,] + b3(var6, u_{[\,]}, v_{[\,]}, w_{[\,]})\ D\_w[\,]) : V2 := Prolong(V, 2) :$

> $psl2 := pdsolve(\{seq(coeffs(expand(eval(LieDerivative(V2, Eq2[i]), sl2)), \{seq(u_i, i=1..6), seq(v_i, i=1..6), seq(w_i, i=1..6), seq(seq(u_{i,j}, j=i..6), i=1..6), seq(seq(v_{i,j}, j=i..6), i=1..6), seq(seq(w_{i,j}, j=i..6), i=1..6)\}), i=1..nops(Eq2))\})$

$$psl2 := \{b1(x1, x2, x3, x4, x5, x6, u[\,], v[\,], w[\,]) = -f_1(x5, x6)\ x3 + f_3(x5, x6), b2(x1, x2, x3, x4, x5, x6, u[\,], v[\,], w[\,]) = -f_1(x5, x6)\ x4 + f_2(x5, x6), b3(x1, x2, x3, x4, x5, x6, u[\,], v[\,], w[\,]) = f_1(x5, x6)\} \tag{61}$$

> $V := evalDG(a1(var6, u_{[\,]}, v_{[\,]}, w_{[\,]})\ D\_x1 + a2(var6, u_{[\,]}, v_{[\,]}, w_{[\,]})\ D\_x2 + a3(var6, u_{[\,]}, v_{[\,]}, w_{[\,]})\ D\_x3 + a4(var6, u_{[\,]}, v_{[\,]}, w_{[\,]})\ D\_x4 + a5(var6, u_{[\,]}, v_{[\,]}, w_{[\,]})\ D\_x5 + a6(var6, u_{[\,]}, v_{[\,]}, w_{[\,]})\ D\_x6 + b1(var6, u_{[\,]}, v_{[\,]}, w_{[\,]})\ D\_u[\,] + b2(var6, u_{[\,]}, v_{[\,]}, w_{[\,]})\ D\_v[\,] + b3(var6, u_{[\,]}, v_{[\,]}, w_{[\,]})\ D\_w[\,]) : V2 := Prolong(V, 2) :$

> $pdsys := \{seq(coeffs(expand(eval(LieDerivative(V2, Eq2[i]), sl2)), \{seq(u_i, i=1..6), seq(v_i, i=1..6), seq(w_i, i=1..6), seq(seq(u_{i,j}, j=i..6), i=1..6), seq(seq(v_{i,j}, j=i..6), i=1..6), seq(seq(w_{i,j}, j=i..6), i=1..6)\}), i=1..nops(Eq2))\} : psl2 := pdsolve(pdsys)$

$$psl2 := \Big\{a1(x1, x2, x3, x4, x5, x6, u[\,], v[\,], w[\,]) = f_2(x1, x2), a2(x1, x2, x3, x4, x5, x6, u[\,], v[\,], w[\,]) = f_4(x1, x2), a3(x1, x2, x3, x4, x5, x6, u[\,], v[\,], w[\,]) = \left(\frac{\partial}{\partial x5} f_3(x5, x6)\right) x4 + f_5(x5, x6)\ x3 + f_6(x5, x6), a4(x1, x2, x3, x4, x5, x6, u[\,], v[\,], w[\,]) = \left(\frac{\partial}{\partial x6} f_1(x5, x6)\right) x3 + \left(f_5(x5, x6) + \frac{\partial}{\partial x5} f_1(x5, x6) - \frac{\partial}{\partial x6} f_3(x5, x6)\right) x4 + f_7(x5, x6), a5(x1, x2, x3, x4, x5, x6, u[\,], v[\,], w[\,]) = f_1(x5, x6), a6(x1, x2, x3, x4, x5, x6, u[\,], v[\,], w[\,]) = f_3(x5, x6), b1(x1, x2, x3, x4, x5, x6, u[\,], v[\,], w[\,]) = \left(\frac{\partial}{\partial x5} f_3(x5, x6)\right) v[\,] + \left(2 f_5(x5, x6) - \frac{\partial}{\partial x6}\right. \tag{62}$$

$$f_3(x5,x6)\Big) u[\,] + \frac{\left(\frac{\partial^2}{\partial x5^2} f_3(x5,x6)\right) x4^2}{2} + \Bigg(\left(\left(\frac{\partial}{\partial x5} f_5(x5,x6)\right) x3 + \frac{\partial}{\partial x5} f_6(x5,$$

$$x6)\Big) x4 + \frac{x3^2 \left(2 \frac{\partial}{\partial x6} f_5(x5,x6) - \frac{\partial^2}{\partial x6^2} f_3(x5,x6)\right)}{2} + \left(\frac{\partial}{\partial x6} f_6(x5,x6) - f_8(x5,\right.$$

$$x6)\Big) x3 + f_9(x5,x6), b2(x1,x2,x3,x4,x5,x6,u[\,],v[\,],w[\,]) = \left(\frac{\partial}{\partial x6} f_1(x5,x6)\right) u[\,]$$

$$+ \left(2 f_5(x5,x6) + \frac{\partial}{\partial x5} f_1(x5,x6) - 2 \frac{\partial}{\partial x6} f_3(x5,x6)\right) v[\,] + \frac{x3^2 \left(\frac{\partial^2}{\partial x6^2} f_1(x5,x6)\right)}{2}$$

$$+ \left(x4 \left(\frac{\partial^2}{\partial x5 \partial x6} f_1(x5,x6)\right) + x4 \left(\frac{\partial}{\partial x6} f_5(x5,x6)\right) - x4 \left(\frac{\partial^2}{\partial x6^2} f_3(x5,x6)\right) + \frac{\partial}{\partial x6}\right.$$

$$f_7(x5,x6)\Big) x3 + \frac{x4^2 \left(\frac{\partial^2}{\partial x5^2} f_1(x5,x6) + 2 \frac{\partial}{\partial x5} f_5(x5,x6) - 2 \frac{\partial^2}{\partial x5 \partial x6} f_3(x5,x6)\right)}{2}$$

$$+ \left(\frac{\partial}{\partial x5} f_7(x5,x6) - f_8(x5,x6)\right) x4 + f_{10}(x5,x6), b3(x1,x2,x3,x4,x5,x6,u[\,],v[\,],w[\,])$$

$$= \left(f_5(x5,x6) - \frac{\partial}{\partial x6} f_3(x5,x6)\right) w[\,] + \left(-\frac{\partial}{\partial x6} f_5(x5,x6) + \frac{\partial^2}{\partial x6^2} f_3(x5,x6)\right) x3 + \Bigg($$

$$- \frac{\partial}{\partial x5} f_5(x5,x6) + \frac{\partial^2}{\partial x5 \partial x6} f_3(x5,x6)\Bigg) x4 + f_8(x5,x6)\Big\}$$

# 2 *arg* : 1, 2, 3, 4, 5, 6, 7, 8, 9, 10
thus the symmetry of the corresponding PDE system contains only (10) functions of 2 arguments, and so cannot change count of functions of 3 arguments in the solution space

> *pdetest*(*psl2*, *pdsys*)

$$\{0\} \quad \textbf{(63)}$$

>

S3.1

> *DGsetup*([*var5*, *q*], *M6*) :

> $\omega := evalDG(a(var5)\, dx1 + b(var5)\, dx2 + q \cdot (dx3 + m(var5)\, dx5)) : \phi := evalDG(c(var5)\, dx1 + d(var5)\, dx2 + q \cdot (dx4 + (n(var5) + q)\, dx5)) :$

> # *unassign*('*S1*','*S2*','*S3*')

> $V1 := evalDG(q\, D\_x1 - a(var5)\, D\_x3 - c(var5)\, D\_x4 + S1\, D\_q) :$
$V2 := evalDG(q\, D\_x2 - b(var5)\, D\_x3 - d(var5)\, D\_x4 + S2\, D\_q) :$
$V3 := evalDG(D\_x5 - m(var5)\, D\_x3 - (n(var5) + q)\, D\_x4 + S3\, D\_q) :$

> $seq(Hook(V \| i, \omega), i = 1..3), seq(Hook(V \| i, \phi), i = 1..3)$

**(64)**

$$0, 0, 0, 0, 0, 0 \quad \textbf{(64)}$$

```
> V12 := evalDG(LieDerivative(V1, V2) + S2/q V1 - S1/q V2) : V13 :=
      evalDG(LieDerivative(V1, V3) + S3/q V1 - (S1·S3)/q D_q) : V23 :=
      evalDG(LieDerivative(V2, V3) + S3/q V2 - (S2·S3)/q D_q) :
```

```
> LieDerivative(V12, x1), LieDerivative(V12, x2), LieDerivative(V12, x5), LieDerivative(V12,
      q), LieDerivative(V13, x1), LieDerivative(V13, x2), LieDerivative(V13, x5),
      LieDerivative(V13, q), LieDerivative(V23, x1), LieDerivative(V23, x2), LieDerivative(V23,
      x5), LieDerivative(V23, q)
```

$$0, 0, 0, 0, 0, 0, 0, 0, 0, 0, 0, 0 \quad \textbf{(65)}$$

```
> tmp1 := DGinfo(V12, "CoefficientSet") : tmp2 := DGinfo(V13, "CoefficientSet") : tmp3 :=
      DGinfo(V23, "CoefficientSet") :
  tmp := tmp1 union tmp2 union tmp3 : sltm := eliminate(tmp, {S1, S2, S3}) : sltm2 :=
      eliminate(tmp1, {S1, S2}) :
```

```
> eval(S1, sltm[1]) - eval(S1, sltm2[1]), eval(S2, sltm[1]) - eval(S2, sltm2[1])
```

$$0, 0 \quad \textbf{(66)}$$

```
> factor(ToJet({coeffs(sltm[2][1], {q}), coeffs(sltm[2][2], {q}), coeffs(sltm[2][3], {q})},
      {a(var5), b(var5), c(var5), d(var5), m(var5), n(var5)}))
```

$$\{b\,(a\,c_{x2} - a\,d_{x1} - c\,a_{x2} + c\,b_{x1}),\ (a\,d - b\,c)\,(a\,b\,n_{x3} - b\,c\,m_{x3} + b\,c\,n_{x4} - b\,m\,c_{x3} - b\,n\,c_{x4} - c\,d\,m_{x4} + c\,m\,b_{x3} + c\,n\,b_{x4} + b\,c_{x5} - c\,b_{x5}),\ -b\,(b\,c_{x2} - b\,d_{x1} - d\,a_{x2} + d\,b_{x1}),\ -(b^2\,n_{x3} - b\,d\,m_{x3} + b\,d\,n_{x4} - b\,m\,d_{x3} - b\,n\,d_{x4} - d^2\,m_{x4} + d\,m\,b_{x3} + d\,n\,b_{x4} + b\,d_{x5} - d\,b_{x5})\,(a\,d - b\,c),\ -a\,b_{x4} - a\,m_{x2} + b\,a_{x4} + b\,m_{x1},\ a\,d\,m_{x4} - a\,m\,b_{x3} - a\,n\,b_{x4} - b\,c\,m_{x4} + b\,m\,a_{x3} + b\,n\,a_{x4} + a\,b_{x5} - b\,a_{x5},\ a^2\,b\,d_{x3} - a\,b^2\,c_{x3} - a\,b\,c\,b_{x3} + a\,b\,c\,d_{x4} - 2\,a\,b\,d\,c_{x4} - a\,b\,d\,n_{x1} + a\,c\,d\,b_{x4} + a\,c\,d\,m_{x2} + b^2\,c\,a_{x3} + b^2\,c\,c_{x4} + b^2\,c\,n_{x1} - 2\,b\,c^2\,b_{x4} - b\,c^2\,m_{x2} + b\,c\,d\,a_{x4},\ -a\,b^2\,d_{x3} + a\,b\,d\,b_{x3} + a\,b\,d\,d_{x4} + a\,b\,d\,n_{x2} - a\,d^2\,b_{x4} - a\,d^2\,m_{x2} + b^3\,c_{x3} - 2\,b^2\,c\,d_{x4} - b^2\,c\,n_{x2} - b^2\,d\,a_{x3} + b^2\,d\,c_{x4} + 2\,b\,c\,d\,b_{x4} + b\,c\,d\,m_{x2} - b\,d^2\,a_{x4}\} \quad \textbf{(67)}$$

the first two equations rewrite as $a\cdot(c_2 - d_1) = c\cdot(a_2 - b_1)$, $b\cdot(c_2 - d_1) = d\cdot(a_2 - b_1)$ and hence we get $a = u_1$, $b = u_2$, $c = v_1$, $d = v_2$;
then the last short equation becomes $u_1\cdot(m + u_4)_2 = u_2\cdot(m + u_4)_1$ whence $m = -u_4 + f(u, x3, x4, x5)$ and we also have:

$$> S1 = \frac{-q}{u_1 - v_1}\cdot\left(u_1^2\,v_{2,3} + u_1\,v_1\,v_{2,4} - u_1\,v_1\,u_{2,3} - u_1\,u_2\,v_{1,3} - u_1\,v_2\,v_{1,4} + u_2\,v_1\,u_{1,3} + v_1\,v_2\,u_{1,4} - v_1^2\,u_{2,4} - v_1\,u_{1,2}\,q + v_1\,u_{1,2}\,q + u_1\,v_{1,2}\,q - u_1\,v_{1,2}\,q\right)$$

```
> # collect(expand(numer(eval(S1, sltm[1]))), {q}); collect(expand(numer(eval(S2,
      sltm[1]))), {q}); collect(expand(numer(eval(S3, sltm[1]))), {q})
```

```
> collect(expand(numer(eval(S3, sltm[1]))), {q})
```

**(68)**

$$\left(-\frac{\partial}{\partial x2}\, m(x1,x2,x3,x4,x5) - \frac{\partial}{\partial x4}\, b(x1,x2,x3,x4,x5)\right) q^2 + \left(d(x1,x2,x3,x4,x5)\left(\frac{\partial}{\partial x4}\, m(x1,x2,x3,x4,x5)\right) + b(x1,x2,x3,x4,x5)\left(\frac{\partial}{\partial x3}\, m(x1,x2,x3,x4,x5)\right) - m(x1,x2,x3,x4,x5)\left(\frac{\partial}{\partial x3}\, b(x1,x2,x3,x4,x5)\right) - n(x1,x2,x3,x4,x5)\left(\frac{\partial}{\partial x4}\, b(x1,x2,x3,x4,x5)\right) + \frac{\partial}{\partial x5}\, b(x1,x2,x3,x4,x5)\right) q \tag{68}$$

this and similar computation show that S1 and S2 are q*function(var5) while S3 is the same plus possibly and expression q^2*function(var5) so we restart

```
> V1 := evalDG(q D_x1 - diff(u(var5), x1) D_x3 - diff(v(var5), x1) D_x4
      + q w1(var5) D_q) :
  V2 := evalDG(q D_x2 - diff(u(var5), x2) D_x3 - diff(v(var5), x2) D_x4
      + q w2(var5) D_q) :
  V3 := evalDG(D_x5 + (diff(u(var5), x4) + f(u(var5), x3, x4, x5)) D_x3 - (n(var5)
      + q) D_x4 + (q w4(var5) + q^2 h(var5)) D_q) :
> V12 := evalDG(LieDerivative(V1, V2) + w2(var5) V1 - w1(var5) V2) :
  V13 := evalDG(LieDerivative(V1, V3) + (w4(var5) + q h(var5)) V1) : V23 :=
      evalDG(LieDerivative(V2, V3) + (w4(var5) + q h(var5)) V2) :
> tmp1 := DGinfo(V12, "CoefficientSet") : tmp2 := DGinfo(V13, "CoefficientSet") : tmp3 :=
      DGinfo(V23, "CoefficientSet") : tmp := tmp1 union tmp2 union tmp3 :
> factor(map(coeffs, expand(ToJet(tmp, {u(var5), v(var5), w1(var5), w2(var5), w4(var5),
      n(var5), h(var5)})), {q}))[1..8]
```

$$\left\{h_{x1}, h_{x2}, u_{x1}\left(\frac{\partial}{\partial u}\, f(u,x3,x4,x5) - h\right), u_{x2}\left(\frac{\partial}{\partial u}\, f(u,x3,x4,x5) - h\right), -w1_{x2} + w2_{x1}, -w4\, v_{x1} + v_{x1,x3}\, u_{x4} + v_{x1,x3} f(u,x3,x4,x5) - v_{x1,x4}\, n + v_{x1,x5} + u_{x1}\, n_{x3} + v_{x1}\, n_{x4}, -w4\, v_{x2} + v_{x2,x3}\, u_{x4} + v_{x2,x3} f(u,x3,x4,x5) - v_{x2,x4}\, n + v_{x2,x5} + u_{x2}\, n_{x3} + v_{x2}\, n_{x4}, -w1_{x3}\, u_{x4} - w1_{x3} f(u,x3,x4,x5) + w1_{x4}\, n + w4\, w1 - w4_{x4}\, v_{x1} - w4_{x3}\, u_{x1} - w1_{x5}\right\} \tag{69}$$

this implies that $w1 = w_1$, $w2 = w_2$ for some function $w$ and that $f(u, x3, x4, x5)$ is affine in u: $f(u, x3, x4, x5) \to h(x3, x4, x5) \cdot u + f(x3, x4, x5)$. Let us substitute this and redefine $n$, $w4$ :

```
> V1 := evalDG(q D_x1 - diff(u(var5), x1) D_x3 - diff(v(var5), x1) D_x4 + q diff(w(var5),
      x1) D_q) :
  V2 := evalDG(q D_x2 - diff(u(var5), x2) D_x3 - diff(v(var5), x2) D_x4 + q diff(w(var5),
      x2) D_q) :
  V3 := evalDG(D_x5 + (diff(u(var5), x4) + h(x3, x4, x5)·u(var5) + f(x3, x4, x5)) D_x3
      + (n(var5) + diff(v(var5), x4) + w(var5) - q) D_x4 + (q·(m(var5) - diff(w(var5),
      x4)) + q^2 h(x3, x4, x5)) D_q) :
> ToJet(V3, {u(var5), v(var5), w(var5), n(var5), m(var5), f(x3, x4, x5), h(x3, x4, x5)})
```

$$\left(h\, u + f + u_{x4}\right) D\_x3 + \left(n + v_{x4} + w - q\right) D\_x4 + D\_x5 + q\left(q\, h + m - w_{x4}\right) D\_q \tag{70}$$

```
> V12 := evalDG(LieDerivative(V1, V2) + diff(w(var5), x2) V1 - diff(w(var5), x1) V2) :
  V13 := evalDG(LieDerivative(V1, V3) + (m(var5) - diff(w(var5), x4) + q h(x3, x4,
      x5)) V1) :
```

$V23 := evalDG(LieDerivative(V2, V3) + (m(var5) - diff(w(var5), x4) + q\, h(x3, x4, x5))\, V2) :$

$> tmp1 := DGinfo(V12, \text{"CoefficientSet"}) : tmp2 := DGinfo(V13, \text{"CoefficientSet"}) : tmp3 := DGinfo(V23, \text{"CoefficientSet"}) : tmp := tmp1 \textbf{ union } tmp2 \textbf{ union } tmp3 :$

$> factor(map(coeffs, expand(ToJet(tmp, \{u(var5), v(var5), w(var5), n(var5), m(var5), f(x3, x4, x5), h(x3, x4, x5)\})), \{q\}))[1..8]$

$$\{-h\, v_{x1} + n_{x1}, -h\, v_{x2} + n_{x2}, 2\, h\, w_{x1} - h_{x3}\, u_{x1} - h_{x4}\, v_{x1} + m_{x1}, 2\, h\, w_{x2} - h_{x3}\, u_{x2} - h_{x4}\, v_{x2} + m_{x2}, -u_{x1}\, w_{x3, x2} + u_{x2}\, w_{x3, x1} - v_{x1}\, w_{x4, x2} + v_{x2}\, w_{x4, x1}, u_{x1}\, u_{x3, x2} - u_{x1}\, w_{x2} - u_{x2}\, u_{x3, x1} + w_{x1}\, u_{x2} - v_{x2}\, u_{x4, x1} + v_{x1}\, u_{x4, x2}, u_{x1}\, v_{x3, x2} - u_{x2}\, v_{x3, x1} + v_{x1}\, v_{x4, x2} - w_{x2}\, v_{x1} - v_{x2}\, v_{x4, x1} + w_{x1}\, v_{x2}, u\, h\, v_{x3, x1} + f\, v_{x3, x1} - m\, v_{x1} + n\, v_{x4, x1} + v_{x4, x1}\, w - u_{x1}\, n_{x3} - v_{x1}\, n_{x4} - u_{x1}\, v_{x3, x4} - u_{x1}\, w_{x3} + u_{x4}\, v_{x3, x1} - v_{x1}\, v_{x4, x4} + v_{x4, x1}\, v_{x4} + v_{x5, x1}\} \tag{71}$$

$> V1 := evalDG(q\, D\_x1 - diff(u(var5), x1)\, D\_x3 - diff(v(var5), x1)\, D\_x4 + q\, diff(w(var5), x1)\, D\_q) :$

$V2 := evalDG(q\, D\_x2 - diff(u(var5), x2)\, D\_x3 - diff(v(var5), x2)\, D\_x4 + q\, diff(w(var5), x2)\, D\_q) :$

$V3 := evalDG\big(D\_x5 + (diff(u(var5), x4) + h(x3, x4, x5) \cdot u(var5) + f(x3, x4, x5))\, D\_x3 + (h(x3, x4, x5) \cdot v(var5) + n(x3, x4, x5) + diff(v(var5), x4) + w(var5) - q)\, D\_x4 + \big(q \cdot (diff(h(x3, x4, x5), x3)\, u(var5) + diff(h(x3, x4, x5), x4)\, v(var5) - 2\, h(x3, x4, x5)\, w(var5) + m(x3, x4, x5) - diff(w(var5), x4)) + q^2\, h(x3, x4, x5)\big)\, D\_q\big) :$

$> ToJet(V3, \{u(var5), v(var5), w(var5), f(x3, x4, x5), m(x3, x4, x5), n(x3, x4, x5), h(x3, x4, x5)\})$

$$\left(h\, u + f + u_{x4}\right) D\_x3 + \left(h\, v + n - q + w + v_{x4}\right) D\_x4 + D\_x5 + q\, \left(q\, h - 2\, h\, w + u\, h_{x3} + v\, h_{x4} + m - w_{x4}\right) D\_q \tag{72}$$

$> V12 := evalDG(LieDerivative(V1, V2) + diff(w(var5), x2)\, V1 - diff(w(var5), x1)\, V2) :$

$V13 := evalDG(LieDerivative(V1, V3) + (diff(h(x3, x4, x5), x3)\, u(var5) + diff(h(x3, x4, x5), x4)\, v(var5) - 2\, h(x3, x4, x5)\, w(var5) + m(x3, x4, x5) - diff(w(var5), x4) + q\, h(x3, x4, x5))\, V1) :$

$V23 := evalDG(LieDerivative(V2, V3) + (diff(h(x3, x4, x5), x3)\, u(var5) + diff(h(x3, x4, x5), x4)\, v(var5) - 2\, h(x3, x4, x5)\, w(var5) + m(x3, x4, x5) - diff(w(var5), x4) + q\, h(x3, x4, x5))\, V2) :$

$> tmp1 := DGinfo(V12, \text{"CoefficientSet"}) : tmp2 := DGinfo(V13, \text{"CoefficientSet"}) : tmp3 := DGinfo(V23, \text{"CoefficientSet"}) : tmp := tmp1 \textbf{ union } tmp2 \textbf{ union } tmp3 :$

$> factor(map(coeffs, expand(ToJet(tmp, \{u(var5), v(var5), w(var5), f(x3, x4, x5), m(x3, x4, x5), n(x3, x4, x5), h(x3, x4, x5)\})), \{q\}))[1..8]$

$$\{-u_{x1}\, w_{x3, x2} + u_{x2}\, w_{x3, x1} - v_{x1}\, w_{x4, x2} + v_{x2}\, w_{x4, x1}, u_{x1}\, u_{x3, x2} - u_{x1}\, w_{x2} - u_{x2}\, u_{x3, x1} + w_{x1}\, u_{x2} - v_{x2}\, u_{x4, x1} + v_{x1}\, u_{x4, x2}, u_{x1}\, v_{x3, x2} - u_{x2}\, v_{x3, x1} + v_{x1}\, v_{x4, x2} - w_{x2}\, v_{x1} - v_{x2}\, v_{x4, x1} + w_{x1}\, v_{x2}, h\, u\, u_{x3, x1} + h\, v\, u_{x4, x1} + 2\, h\, w\, u_{x1} - h\, u_{x1}\, u_{x3} - h\, u_{x4}\, v_{x1} - 2\, u\, h_{x3}\, u_{x1} - u\, h_{x4}\, v_{x1} - v\, h_{x4}\, u_{x1} + f\, u_{x3, x1} - m\, u_{x1} + n\, u_{x4, x1} + u_{x4, x1}\, w - f_{x3}\, u_{x1} - f_{x4}\, v_{x1} - u_{x1}\, u_{x3, x4} + u_{x1}\, w_{x4} + u_{x4}\, u_{x3, x1} + u_{x4, x1}\, v_{x4} - v_{x1}\, u_{x4, x4} + u_{x5, x1}, h\, u\, u_{x3, x2} + h\, v\, u_{x4, x2} + 2\, h\, w\, u_{x2} - h\, u_{x2}\, u_{x3} - h\, u_{x4}\, v_{x2} - 2\, u\, h_{x3}\, u_{x2} - u\, h_{x4}\, v_{x2} - v\, h_{x4}\, u_{x2} + f\, u_{x3, x2} - m\, u_{x2} + n\, u_{x4, x2} + u_{x4, x2}\, w - f_{x3}\, u_{x2} - f_{x4}\, v_{x2} - u_{x2}\, u_{x3, x4} \tag{73}$$

$$+ u_{x2} w_{x4} + u_{x4} u_{x3, x2} + u_{x4, x2} v_{x4} - v_{x2} u_{x4, x4} + u_{x5, x2}, u h v_{x3, x1} + h v v_{x4, x1} + 2 h w v_{x1} - h u_{x1} v_{x3} - h v_{x1} v_{x4} - u h_{x3} v_{x1} - v h_{x3} u_{x1} - 2 v h_{x4} v_{x1} + f v_{x3, x1} - m v_{x1} + n v_{x4, x1} + v_{x4, x1} w - u_{x1} n_{x3} - v_{x1} n_{x4} - u_{x1} v_{x3, x4} - u_{x1} w_{x3} + u_{x4} v_{x3, x1} - v_{x1} v_{x4, x4} + v_{x4, x1} v_{x4} + v_{x5, x1}, v_{x3, x2} h u + h v v_{x4, x2} + 2 h w v_{x2} - h u_{x2} v_{x3} - h v_{x2} v_{x4} - u h_{x3} v_{x2} - v h_{x3} u_{x2} - 2 v h_{x4} v_{x2} + v_{x3, x2} f - v_{x2} m + n v_{x4, x2} + v_{x4, x2} w - u_{x2} n_{x3} - v_{x2} n_{x4} - u_{x2} v_{x3, x4} - u_{x2} w_{x3} + v_{x3, x2} u_{x4} - v_{x2} v_{x4, x4} + v_{x4, x2} v_{x4} + v_{x5, x2}, -u h w_{x3, x1} - h v w_{x4, x1} - 2 h w w_{x1} + 2 h u_{x1} w_{x3} + 2 h v_{x1} w_{x4} + u h_{x3} w_{x1} - u h_{x3, x3} u_{x1} - u h_{x3, x4} v_{x1} + v h_{x4} w_{x1} - v h_{x3, x4} u_{x1} - v h_{x4, x4} v_{x1} + 2 w h_{x3} u_{x1} + 2 w h_{x4} v_{x1} - u_{x1} u_{x3} h_{x3} - v_{x1} u_{x4} h_{x3} - u_{x1} v_{x3} h_{x4} - v_{x1} v_{x4} h_{x4} - f w_{x3, x1} + m w_{x1} - n w_{x4, x1} - w_{x4, x1} w - u_{x1} m_{x3} - m_{x4} v_{x1} + u_{x1} w_{x3, x4} - u_{x4} w_{x3, x1} + v_{x1} w_{x4, x4} - w_{x4, x1} v_{x4} - w_{x1} w_{x4} - w_{x5, x1}\}$$

```
> V1 := evalDG(q D_x1 − diff(u(var5), x1) D_x3 − diff(v(var5), x1) D_x4 + q diff(w(var5),
      x1) D_q) :
  V2 := evalDG(q D_x2 − diff(u(var5), x2) D_x3 − diff(v(var5), x2) D_x4 + q diff(w(var5),
      x2) D_q) :
  V3 := evalDG(D_x5 + (diff(u(var5), x4) + h(x3, x4, x5)·u(var5)) D_x3 + (h(x3, x4, x5)
      ·v(var5) + diff(v(var5), x4) + w(var5)−q) D_x4 + (q·(diff(h(x3, x4, x5), x3) u(var5)
      + diff(h(x3, x4, x5), x4) v(var5) − 2 h(x3, x4, x5) w(var5) − diff(w(var5), x4))
      + q^2 h(x3, x4, x5)) D_q) :
```

```
> ToJet(V3, {u(var5), v(var5), w(var5), f(x3, x4, x5), m(x3, x4, x5), n(x3, x4, x5), h(x3, x4,
      x5)})
```

$$\left(h u + u_{x4}\right) D\_x3 + \left(h v - q + w + v_{x4}\right) D\_x4 + D\_x5 + q \left(q h - 2 h w + h_{x3} u + h_{x4} v - w_{x4}\right) D\_q \tag{74}$$

```
> V12 := evalDG(LieDerivative(V1, V2) + diff(w(var5), x2) V1 − diff(w(var5), x1) V2) :
  V13 := evalDG(LieDerivative(V1, V3) + (diff(h(x3, x4, x5), x3) u(var5) + diff(h(x3, x4,
      x5), x4) v(var5) − 2 h(x3, x4, x5) w(var5) − diff(w(var5), x4) + q h(x3, x4, x5)) V1) :
  V23 := evalDG(LieDerivative(V2, V3) + (diff(h(x3, x4, x5), x3) u(var5) + diff(h(x3, x4,
      x5), x4) v(var5) − 2 h(x3, x4, x5) w(var5) − diff(w(var5), x4) + q h(x3, x4, x5)) V2) :
```

```
> tmp1 := DGinfo(V12, "CoefficientSet") : tmp2 := DGinfo(V13, "CoefficientSet") : tmp3 :=
      DGinfo(V23, "CoefficientSet") : tmp := tmp1 union tmp2 union tmp3 :
```

```
> map(coeffs, expand(ToJet(tmp, {u(var5), v(var5), w(var5), f(x3, x4, x5), m(x3, x4, x5), n(x3,
      x4, x5), h(x3, x4, x5)})), {q})
```

$$\{-u_{x1} w_{x3, x2} + u_{x2} w_{x3, x1} - v_{x1} w_{x4, x2} + v_{x2} w_{x4, x1}, u_{x1} u_{x3, x2} - u_{x1} w_{x2} - u_{x2} u_{x3, x1} + w_{x1} u_{x2} - v_{x2} u_{x4, x1} + v_{x1} u_{x4, x2}, u_{x1} v_{x3, x2} - u_{x2} v_{x3, x1} + v_{x1} v_{x4, x2} - w_{x2} v_{x1} - v_{x2} v_{x4, x1} + w_{x1} v_{x2}, h u u_{x3, x1} + h v u_{x4, x1} + 2 h w u_{x1} - h u_{x1} u_{x3} - h u_{x4} v_{x1} - 2 u h_{x3} u_{x1} - u h_{x4} v_{x1} - v h_{x4} u_{x1} + u_{x4, x1} w - u_{x1} u_{x3, x4} + u_{x1} w_{x4} + u_{x4} u_{x3, x1} + u_{x4, x1} v_{x4} - v_{x1} u_{x4, x4} + u_{x5, x1}, u h v_{x3, x1} + h v v_{x4, x1} + 2 h w v_{x1} - h u_{x1} v_{x3} - h v_{x1} v_{x4} - u h_{x3} v_{x1} - v h_{x3} u_{x1} - 2 v h_{x4} v_{x1} + v_{x4, x1} w - u_{x1} v_{x3, x4} - u_{x1} w_{x3} + u_{x4} v_{x3, x1} - v_{x1} v_{x4, x4} + v_{x4, x1} v_{x4} + v_{x5, x1}, h u u_{x3, x2} + h v u_{x4, x2} + 2 h w u_{x2} - h u_{x2} u_{x3} - h u_{x4} v_{x2} - 2 u h_{x3} u_{x2} - u h_{x4} v_{x2} - v h_{x4} u_{x2} + u_{x4, x2} w - u_{x2} u_{x3, x4} + u_{x2} w_{x4} \tag{75}$$

$+ u_{x4} u_{x3,x2} + u_{x4,x2} v_{x4} - v_{x2} u_{x4,x4} + u_{x5,x2}, v_{x3,x2} h u + h v v_{x4,x2} + 2 h w v_{x2} - h u_{x2} v_{x3}$
$- h v_{x2} v_{x4} - u h_{x3} v_{x2} - v h_{x3} u_{x2} - 2 v h_{x4} v_{x2} + v_{x4,x2} w - u_{x2} v_{x3,x4} - u_{x2} w_{x3} + v_{x3,x2} u_{x4}$
$- v_{x2} v_{x4,x4} + v_{x4,x2} v_{x4} + v_{x5,x2}, -u h w_{x3,x1} - h v w_{x4,x1} - 2 h w w_{x1} + 2 h u_{x1} w_{x3} + 2 h v_{x1} w_{x4}$
$+ u h_{x3} w_{x1} - u h_{x3,x3} u_{x1} - u h_{x3,x4} v_{x1} + v h_{x4} w_{x1} - v h_{x3,x4} u_{x1} - v h_{x4,x4} v_{x1} + 2 w h_{x3} u_{x1}$
$+ 2 w h_{x4} v_{x1} - u_{x1} u_{x3} h_{x3} - v_{x1} u_{x4} h_{x3} - u_{x1} v_{x3} h_{x4} - v_{x1} v_{x4} h_{x4} - w_{x4,x1} w + u_{x1} w_{x3,x4}$
$- u_{x4} w_{x3,x1} + v_{x1} w_{x4,x4} - w_{x4,x1} v_{x4} - w_{x1} w_{x4} - w_{x5,x1}, -w_{x3,x2} h u - h v w_{x4,x2} - 2 h w w_{x2}$
$+ 2 h u_{x2} w_{x3} + 2 h v_{x2} w_{x4} + u h_{x3} w_{x2} - u h_{x3,x3} u_{x2} - u h_{x3,x4} v_{x2} + v h_{x4} w_{x2} - v h_{x3,x4} u_{x2}$
$- v h_{x4,x4} v_{x2} + 2 w h_{x3} u_{x2} + 2 w h_{x4} v_{x2} - h_{x3} u_{x3} u_{x2} - h_{x3} u_{x4} v_{x2} - h_{x4} v_{x3} u_{x2} - h_{x4} v_{x4} v_{x2}$
$- w_{x4,x2} w + w_{x3,x4} u_{x2} - w_{x3,x2} u_{x4} + w_{x4,x4} v_{x2} - w_{x4,x2} v_{x4} - w_{x2} w_{x4} - w_{x5,x2}\}$

> *nops*(%)

9 **(76)**

> $V1h := evalDG(q\ D\_x1 - diff(u(var5), x1)\ D\_x3 - diff(v(var5), x1)\ D\_x4 + q\ diff(w(var5), x1)\ D\_q):$
$V2h := evalDG(q\ D\_x2 - diff(u(var5), x2)\ D\_x3 - diff(v(var5), x2)\ D\_x4 + q\ diff(w(var5), x2)\ D\_q):$
$V3h := evalDG\big(D\_x5 + (diff(u(var5), x4) + h(var5) \cdot u(var5))\ D\_x3 + (h(var5) \cdot v(var5) + diff(v(var5), x4) + w(var5) - q)\ D\_x4 + \big(q \cdot (diff(h(var5), x3)\ u(var5) + diff(h(var5), x4)\ v(var5) - 2\ h(var5)\ w(var5) - diff(w(var5), x4)) + q^2\ h(var5)\big)\ D\_q\big):$
$V12h := evalDG(LieDerivative(V1h, V2h) + diff(w(var5), x2)\ V1h - diff(w(var5), x1)\ V2h):$
$V13h := evalDG(LieDerivative(V1h, V3h) + (diff(h(var5), x3)\ u(var5) + diff(h(var5), x4)\ v(var5) - 2\ h(var5)\ w(var5) - diff(w(var5), x4) + q\ h(var5))\ V1h):$
$V23h := evalDG(LieDerivative(V2h, V3h) + (diff(h(var5), x3)\ u(var5) + diff(h(var5), x4)\ v(var5) - 2\ h(var5)\ w(var5) - diff(w(var5), x4) + q\ h(var5))\ V2h):$

> *tmp1h* := *DGinfo*(*V12h*, "CoefficientSet") : *tmp2h* := *DGinfo*(*V13h*, "CoefficientSet") : *tmp3h* := *DGinfo*(*V23h*, "CoefficientSet") : *tmph* := *tmp1h* **union** *tmp2h* **union** *tmp3h* :

> $Eq2h := map(coeffs, expand(ToJet(tmph, \{u(var5), v(var5), w(var5), h(var5)\}, notation = jetnumbers)), \{q\}) : el2h := eliminate\big(Eq2h, \{u_{1,4}, u_{1,5}, u_{2,5}, v_{1,4}, v_{1,5}, v_{2,5}, w_{1,4}, w_{1,5}, w_{2,5}, h_1, h_2\}\big) : sl2h := el2h[1]$ **union** $\{seq(h_{1,i} = 0, i = 1..5), seq(h_{2,i} = 0, i = 2..5)\}:$

> $Eq2h := Eq2h \setminus \{h_1\ u[\ ], h_1\ v[\ ], h_2\ u[\ ], h_2\ v[\ ], -2\ h_1\ w[\ ] + h_{1,3}\ u[\ ] + h_{1,4}\ v[\ ], -2\ h_2\ w[\ ] + h_{2,3}\ u[\ ] + h_{2,4}\ v[\ ]\} : nops(\%)$

11 **(77)**

> $DGsetup([var5], [u, v, w, h], Jh5, 5):$

> $V := evalDG(add((a \| i)(var5, u[\ ], v[\ ], w[\ ], h[\ ])\ D\_x \| i, i = 1..5) + b1(var5, u[\ ], v[\ ], w[\ ], h[\ ])\ D\_u[\ ] + b2(var5, u[\ ], v[\ ], w[\ ], h[\ ])\ D\_v[\ ] + b3(var5, u[\ ], v[\ ], w[\ ], h[\ ])\ D\_w[\ ] + b0(var5, u[\ ], v[\ ], w[\ ], h[\ ])\ D\_h[\ ]) : V2 := Prolong(V, 2):$

> $pdsysh := \{seq\big(map\big(coeffs, expand(LieDerivative(V2, Eq2h[i])), \{seq(u_i, i = 1..5), seq(v_i, i = 1..5), seq(w_i, i = 1..5), seq(h_i, i = 1..5), seq(seq(u_{i,j}, j = i..5), i = 1..5), seq(seq(v_{i,j}, j = i..5), i = 1..5), seq(seq(w_{i,j}, j = i..5), i = 1..5), seq(seq(h_{i,j}, j = i..5), i = 1..5)\}\big), i = 1$

..nops(Eq2h))} : nops(pdsysh)

$$11 \quad \textbf{(78)}$$

> # psl2h :=pdsolve(pdsysh) :

> V := evalDG(b1(var5, u[ ], v[ ], w[ ], h[ ]) D_u[ ] + b2(var5, u[ ], v[ ], w[ ], h[ ]) D_v[ ] + b3(var5, u[ ], v[ ], w[ ], h[ ]) D_w[ ] + b0(var5, u[ ], v[ ], w[ ], h[ ]) D_h[ ]) : V2 := Prolong(V, 2) :

> pdsysh := {seq(map(coeffs, expand(LieDerivative(V2, Eq2h[i])), {seq($u_i$, i = 1 ..5), seq($v_i$, i = 1 ..5), seq($w_i$, i = 1 ..5), seq($h_i$, i = 1 ..5), seq(seq($u_{i,j}$, j = i ..5), i = 1 ..5), seq(seq($v_{i,j}$, j = i ..5), i = 1 ..5), seq(seq($w_{i,j}$, j = i ..5), i = 1 ..5), seq(seq($h_{i,j}$, j = i ..5), i = 1 ..5)}), i = 1 ..nops(Eq2h))} : nops(pdsysh)

$$11 \quad \textbf{(79)}$$

> # psl2h :=pdsolve(pdsysh) :

>

> DGsetup([var5, q], [u, v, w, h], J6, 1) :

> V1h := evalDG(q D_x1 − diff(u(var5), x1) D_x3 − diff(v(var5), x1) D_x4 + q diff(w(var5), x1) D_q) :
V2h := evalDG(q D_x2 − diff(u(var5), x2) D_x3 − diff(v(var5), x2) D_x4 + q diff(w(var5), x2) D_q) :
V3h := evalDG(exp(h(var5))·D_x5 + diff(u(var5), x4) D_x3 + (diff(v(var5), x4) + w(var5) + diff(h(var5), x3)·u(var5) + diff(h(var5), x4)·v(var5) − q) D_x4 − diff(w(var5), x4) q D_q) :

> V12h := evalDG(LieDerivative(V1h, V2h) + diff(w(var5), x2) V1h − diff(w(var5), x1) V2h) :
V13h := evalDG(LieDerivative(V1h, V3h) − diff(w(var5), x4) V1h + (diff(h(var5), x3) diff(u(var5), x1) + diff(h(var5), x4) diff(v(var5), x1)) V3h) :

> V23h := evalDG(LieDerivative(V2h, V3h) − diff(w(var5), x4) V2h + (diff(h(var5), x3) diff(u(var5), x2) + diff(h(var5), x4) diff(v(var5), x2)) V3h) :

> tmp1h := DGinfo(V12h, "CoefficientSet") : tmp2h := DGinfo(V13h, "CoefficientSet") : tmp3h := DGinfo(V23h, "CoefficientSet") : tmph := tmp1h **union** tmp2h **union** tmp3h :

> Eq2h := map(coeffs, expand(ToJet(tmph, {u(var5), v(var5), w(var5), h(var5)}, notation =jetnumbers)), {q}) : el2h := eliminate(Eq2h, {$u_{1,4}, u_{1,5}, u_{2,5}, v_{1,4}, v_{1,5}, v_{2,5}, w_{1,4}, w_{1,5}, w_{2,5}, h_1, h_2$}) : sl2h := el2h[1] **union** {seq($h_{1,i}$ = 0, i = 1 ..5), seq($h_{2,i}$ = 0, i = 2 ..5)} :

> Eq2h

$$\{h_1 e^{h[\,]}, h_2 e^{h[\,]}, h_3 u[\,] u_{1,4} + h_4 v[\,] u_{1,4} + u_4 h_3 u_1 + u_4 h_4 v_1 + u_{1,4} v_4 + u_{1,4} w[\,] + u_1 w_4 + e^{h[\,]} u_{1,5} + u_4 u_{1,3} - u_1 u_{3,4} - v_1 u_{4,4}, h_3 u[\,] u_{2,4} + h_4 v[\,] u_{2,4} + h_3 u_4 u_2 + h_4 u_4 v_2 + e^{h[\,]} u_{2,5} + u_{2,4} v_4 + u_{2,4} w[\,] - u_2 u_{3,4} - v_2 u_{4,4} + u_4 u_{2,3} + u_2 w_4, -h_3 w_{2,4} u[\,] - h_3 w_4 u_2 - h_4 w_{2,4} v[\,] - h_4 v_2 w_4 - e^{h[\,]} w_{2,5} - w_2 w_4 - u_4 w_{2,3} - v_4 w_{2,4} - w_{2,4} w[\,] + v_2 w_{4,4} + u_2 w_{3,4}, -w_{1,4} h_3 u[\,] - w_{1,4} h_4 v[\,] - w_4 h_3 u_1 - w_4 h_4 v_1 - v_4 w_{1,4} - w_{1,4} w[\,] - w_1 w_4 + u_1 w_{3,4} - u_4 w_{1,3} - e^{h[\,]} w_{1,5} + v_1 w_{4,4}, -u_1 v_{3,4} - v_1 v_{4,4} + u_4 v_{1,3} + v_4 v_{1,4} + v_{1,4} w[\,] - u_1 v_3 h_4 - v_1 u_4 h_3 - u_1 u_3 h_3 + h_3 w[\,] u_1 + h_4 w[\,] v_1 - h_{3,3} u[\,] u_1 \quad \textbf{(80)}$$

$- v[\,]\, h_{3,4}\, u_1 - h_{3,4}\, u[\,]\, v_1 - v[\,]\, h_{4,4}\, v_1 - u_1\, w_3 + u[\,]\, h_3\, h_4\, v_1 + v[\,]\, h_3\, u_1\, h_4 + v_{1,4}\, h_3\, u[\,]$
$+ v_{1,4}\, h_4\, v[\,] + u[\,]\, h_3^2\, u_1 + v[\,]\, h_4^2\, v_1 + v_4\, h_3\, u_1 + e^{h[\,]}\, v_{1,5}, -h_{3,4}\, v[\,]\, u_2 - h_{3,4}\, v_2\, u[\,]$
$- h_{3,3}\, u_2\, u[\,] - h_{4,4}\, v[\,]\, v_2 + h_4\, w[\,]\, v_2 - u_2\, w_3 - u_2\, v_{3,4} - v_2\, v_{4,4} + u_4\, v_{2,3} + v_4\, v_{2,4}$
$+ v_{2,4}\, w[\,] + h_3\, h_4\, u[\,]\, v_2 - h_4\, v_3\, u_2 - h_3\, u_3\, u_2 - h_3\, u_4\, v_2 + h_3\, w[\,]\, u_2 + h_3^2\, u[\,]\, u_2 +$
$h_4^2\, v[\,]\, v_2 + h_3\, v_4\, u_2 + h_3\, v_{2,4}\, u[\,] + h_4\, v_{2,4}\, v[\,] + e^{h[\,]}\, v_{2,5} + h_3\, h_4\, v[\,]\, u_2, h_{1,3}\, u[\,]$
$+ h_{1,4}\, v[\,], h_{2,3}\, u[\,] + v[\,]\, h_{2,4}, -u_1\, w_{2,3} + u_2\, w_{1,3} - w_{2,4}\, v_1 + v_2\, w_{1,4}, u_1\, u_{2,3} - u_1\, w_2$
$- u_2\, u_{1,3} + u_2\, w_1 - v_2\, u_{1,4} + v_1\, u_{2,4}, u_1\, v_{2,3} - u_2\, v_{1,3} + v_1\, v_{2,4} - v_1\, w_2 - v_2\, v_{1,4} + v_2\, w_1\}$

> $Eq2h := Eq2h \setminus \{h_{1,3}\, u[\,] + h_{1,4}\, v[\,], h_{2,3}\, u[\,] + h_{2,4}\, v[\,]\} : nops(\%)$

$$11 \quad \textbf{(81)}$$

> $DGsetup([var5], [u, v, w, h], Jh5, 5) :$

> $V := evalDG(add((a \| i)(var5, u[\,], v[\,], w[\,], h[\,])\, D\_x \| i, i = 1..5) + b1(var5, u[\,], v[\,], w[\,], h[\,])\, D\_u[\,] + b2(var5, u[\,], v[\,], w[\,], h[\,])\, D\_v[\,] + b3(var5, u[\,], v[\,], w[\,], h[\,])\, D\_w[\,] + b0(var5, u[\,], v[\,], w[\,], h[\,])\, D\_h[\,]) : V2 := Prolong(V, 2) :$

> $pdsysh := \{seq(map(coeffs, expand(LieDerivative(V2, Eq2h[i])), \{seq(u_i, i = 1..5), seq(v_i, i = 1..5), seq(w_i, i = 1..5), seq(h_i, i = 1..5), seq(seq(u_{i,j}, j = i..5), i = 1..5), seq(seq(v_{i,j}, j = i..5), i = 1..5), seq(seq(w_{i,j}, j = i..5), i = 1..5), seq(seq(h_{i,j}, j = i..5), i = 1..5)\}), i = 1..nops(Eq2h))\} : nops(pdsysh)$

$$11 \quad \textbf{(82)}$$

> # psl2h :=pdsolve(pdsysh) :

> $V := evalDG(b1(var5, u[\,], v[\,], w[\,], h[\,])\, D\_u[\,] + b2(var5, u[\,], v[\,], w[\,], h[\,])\, D\_v[\,] + b3(var5, u[\,], v[\,], w[\,], h[\,])\, D\_w[\,] + b0(var5, u[\,], v[\,], w[\,], h[\,])\, D\_h[\,]) : V2 := Prolong(V, 2) :$

> $pdsysh := \{seq(map(coeffs, expand(LieDerivative(V2, Eq2h[i])), \{seq(u_i, i = 1..5), seq(v_i, i = 1..5), seq(w_i, i = 1..5), seq(h_i, i = 1..5), seq(seq(u_{i,j}, j = i..5), i = 1..5), seq(seq(v_{i,j}, j = i..5), i = 1..5), seq(seq(w_{i,j}, j = i..5), i = 1..5), seq(seq(h_{i,j}, j = i..5), i = 1..5)\}), i = 1..nops(Eq2h))\} : nops(pdsysh)$

$$11 \quad \textbf{(83)}$$

> # psl2h :=pdsolve(pdsysh) :

> $Eq2 := (Eq2h \setminus \{h_1\, e^{h[\,]}, h_2\, e^{h[\,]}\})$ **union** $\{h_1, h_2, seq(h_{1,i}, i = 1..5), seq(h_{2,i}, i = 2..5)\} :$
$el2 := eliminate(Eq2, \{u_{1,4}, u_{1,5}, u_{2,5}, v_{1,4}, v_{1,5}, v_{2,5}, w_{1,4}, w_{1,5}, w_{2,5}, h_1, h_2, seq(h_{1,i}, i = 1..5), seq(h_{2,i}, i = 2..5)\}) : sl2 := el2[1] : el2[2]$

$$\emptyset \quad \textbf{(84)}$$

> $Eq3 := \{seq(op(map(TotalDiff, Eq2, i)), i = 1..5)\} : el3 := eliminate(eval(Eq3, sl2), \{seq(u_{1,i,4}, i = 1..4), seq(u_{1,i,5}, i = 1..5), seq(u_{2,i,5}, i = 2..5), seq(v_{1,i,4}, i = 1..4), seq(v_{1,i,5}, i = 1..5), seq(v_{2,i,5}, i = 2..5), seq(w_{1,i,4}, i = 1..4), seq(w_{1,i,5}, i = 1..5), seq(w_{2,i,5}, i = 2..5), seq(seq(h_{1,i,j}, j = i..5), i = 1..5), seq(seq(h_{2,i,j}, j = i..5), i = 2..5)\}) :$
$sl3 := el3[1] : el3[2]$

$$\emptyset \quad \textbf{(85)}$$

> $Eq4 := \{seq(seq(op(map(TotalDiff, Eq2, [i,j])), j=i..5), i=1..5)\} : el4 :=$
$eliminate\left(eval(eval(Eq4, sl3), sl2), \left\{seq\left(seq\left(u_{1,i,j,4}, j=i..4\right), i=1..4\right), seq\left(seq\left(u_{1,i,j,5}, j=i..5\right), i=1..5\right), seq\left(seq\left(u_{2,i,j,5}, j=i..5\right), i=2..5\right), seq\left(seq\left(v_{1,i,j,4}, j=i..4\right), i=1..4\right), seq\left(seq\left(v_{1,i,j,5}, j=i..5\right), i=1..5\right), seq\left(seq\left(v_{2,i,j,5}, j=i..5\right), i=2..5\right), seq\left(seq\left(w_{1,i,j,4}, j=i..4\right), i=1..4\right), seq\left(seq\left(w_{1,i,j,5}, j=i..5\right), i=1..5\right), seq\left(seq\left(w_{2,i,j,5}, j=i..5\right), i=2..5\right), seq\left(seq\left(seq\left(h_{1,i,j,k}, k=j..5\right), j=i..5\right), i=1..5\right), seq\left(seq\left(seq\left(h_{2,i,j,k}, k=j..5\right), j=i..5\right), i=2..5\right)\right\}\right) : sl4 := el4[1] : el4[2]$

$$\varnothing \qquad (86)$$

>

S3.2

> $DGsetup([var6, q], M7) :$

> $\omega := evalDG\left(a(var6)\ dx1 + b(var6)\ dx2 + q\ (dx3 + m(var6)\ dx5 + n(var6)\ dx6) + q^2\ dx6\right) : \phi := evalDG\left(c(var6)\ dx1 + d(var6)\ dx2 + q\ (h(var6)\ dx4 + p(var6)\ dx5 + o(var6)\ dx6) + q^2\ dx5\right) :$

> $V1 := evalDG\left(q\ D\_x1 - a(var6)\ D\_x3 - \frac{c(var6)}{h(var6)}\ D\_x4 + S1\ D\_q\right) :$
$V2 := evalDG\left(q\ D\_x2 - b(var6)\ D\_x3 - \frac{d(var6)}{h(var6)}\ D\_x4 + S2\ D\_q\right) :$
$V3 := evalDG\left(D\_x5 - m(var6)\ D\_x3 - \frac{p(var6) + q}{h(var6)}\ D\_x4 + S3\ D\_q\right) :$
$V4 := evalDG\left(D\_x6 - (n(var6) + q)\ D\_x3 - \frac{o(var6)}{h(var6)}\ D\_x4 + S4\ D\_q\right) :$

> $seq\left(Hook(V \| i, \omega), i=1..4\right), seq\left(Hook(V \| i, \phi), i=1..4\right)$

$$0, 0, 0, 0, 0, 0, 0, 0 \qquad (87)$$

> $V12 := evalDG\left(LieDerivative(V1, V2) + \frac{S2}{q}\ V1 - \frac{S1}{q}\ V2\right) : V13 :=$
$evalDG\left(LieDerivative(V1, V3) + \frac{S3}{q}\ V1 - \frac{S1\ S3}{q}\ D\_q\right) : V23 :=$
$evalDG\left(LieDerivative(V2, V3) + \frac{S3}{q}\ V2 - \frac{S2\ S3}{q}\ D\_q\right) : V14 :=$
$evalDG\left(LieDerivative(V1, V4) + \frac{S4}{q}\ V1 - \frac{S1\ S4}{q}\ D\_q\right) : V24 :=$
$evalDG\left(LieDerivative(V2, V4) + \frac{S4}{q}\ V2 - \frac{S2\ S4}{q}\ D\_q\right) : V34 :=$
$evalDG(LieDerivative(V3, V4)) :$

> $LieDerivative(V12, x1), LieDerivative(V12, x2), LieDerivative(V12, x5), LieDerivative(V12, x6), LieDerivative(V12, q), LieDerivative(V13, x1), LieDerivative(V13, x2), LieDerivative(V13, x5), LieDerivative(V13, x6), LieDerivative(V13, q), LieDerivative(V23, x1), LieDerivative(V23, x2), LieDerivative(V23, x5), LieDerivative(V23, x6), LieDerivative(V23, q), LieDerivative(V14, x1), LieDerivative(V14, x2), LieDerivative(V14, x5), LieDerivative(V14, x6), LieDerivative(V14, q), LieDerivative(V24, x1), LieDerivative(V24, x2), LieDerivative(V24, x5), LieDerivative(V24, x6), LieDerivative(V24, q), LieDerivative(V34, x1), LieDerivative(V34, x2), LieDerivative(V34, x5), LieDerivative(V34, x6), LieDerivative(V34, q)$

$$0, 0, 0, 0, 0, 0, 0, 0, 0, 0, 0, 0, 0, 0, 0, 0, 0, 0, 0, 0, 0, 0, 0, 0, 0, 0, 0, 0, 0, 0 \quad (88)$$

```
> tmp1 := DGinfo(V12, "CoefficientSet") : tmp2 := DGinfo(V13, "CoefficientSet") : tmp3 :=
    DGinfo(V23, "CoefficientSet") : tmp4 := DGinfo(V14, "CoefficientSet") : tmp5 :=
    DGinfo(V24, "CoefficientSet") : tmp6 := DGinfo(V34, "CoefficientSet") :
  tmp := tmp1 union tmp2 union tmp3 union tmp4 union tmp5 union tmp6 : sltm :=
    eliminate(tmp, {S1, S2, S3, S4}) :
> collect(expand(ToJet(sltm[1][1..2], {a(var6), b(var6), c(var6), d(var6), m(var6), n(var6),
    p(var6), o(var6), h(var6)})), {q})
```

$$\left\{S1 = \left(-\frac{a_{x2}}{b} + \frac{b_{x1}}{b}\right) q^2 + \left(-\frac{a\, h_{x3}}{h} + \frac{a\, d_{x3}}{d} + \frac{a\, o_{x2}}{d} - \frac{a\, o\, h_{x2}}{d\, h} - \frac{2\, a\, b_{x3}}{b} - \frac{a\, n_{x2}}{b} + a_{x3} - \frac{c\, b_{x4}}{h\, b} + \frac{d\, a_{x4}}{h\, b}\right) q - \frac{b\, a\, o_{x3}}{d} + \frac{b\, a\, o\, h_{x3}}{d\, h} + a\, n_{x3} - \frac{a\, n\, h_{x3}}{h} + \frac{a\, n\, d_{x3}}{d} - \frac{a\, n\, b_{x3}}{b} + \frac{a\, h_{x6}}{h} - \frac{a\, o_{x4}}{h} - \frac{a\, d_{x6}}{d} + \frac{a\, o\, d_{x4}}{d\, h} + \frac{d\, a\, n_{x4}}{h\, b} + \frac{a\, b_{x6}}{b} - \frac{a\, o\, b_{x4}}{h\, b}, S2 = \left(-\frac{b\, h_{x3}}{h} + \frac{b\, d_{x3}}{d} + \frac{b\, o_{x2}}{d} - \frac{b\, o\, h_{x2}}{d\, h} - b_{x3} - n_{x2}\right) q - \frac{b^2\, o_{x3}}{d} + \frac{b^2\, o\, h_{x3}}{d\, h} + b\, n_{x3} - \frac{b\, n\, h_{x3}}{h} + \frac{b\, n\, d_{x3}}{d} - n\, b_{x3} + \frac{b\, h_{x6}}{h} - \frac{b\, o_{x4}}{h} - \frac{b\, d_{x6}}{d} + \frac{b\, o\, d_{x4}}{d\, h} + \frac{d\, n_{x4}}{h} + b_{x6} - \frac{o\, b_{x4}}{h}\right\} \quad (89)$$

```
> collect(expand(ToJet(sltm[1][3..4], {a(var6), b(var6), c(var6), d(var6), m(var6), n(var6),
    p(var6), o(var6), h(var6)})), {q})
```

$$\left\{S3 = \left(-\frac{m_{x2}}{b} - \frac{b_{x4}}{h\, b}\right) q^2 + \left(m_{x3} - \frac{m\, b_{x3}}{b} + \frac{d\, m_{x4}}{h\, b} + \frac{b_{x5}}{b} - \frac{p\, b_{x4}}{h\, b}\right) q, S4 = \left(\frac{h_{x3}}{h} - \frac{d_{x3}}{d} - \frac{o_{x2}}{d} + \frac{o\, h_{x2}}{h\, d}\right) q^2 + \left(\frac{b\, o_{x3}}{d} - \frac{b\, o\, h_{x3}}{h\, d} + \frac{n\, h_{x3}}{h} - \frac{n\, d_{x3}}{d} - \frac{h_{x6}}{h} + \frac{o_{x4}}{h} + \frac{d_{x6}}{d} - \frac{o\, d_{x4}}{h\, d}\right) q\right\} \quad (90)$$

```
> nops(sltm[2])
```

$$8 \quad (91)$$

```
> tmp := factor(ToJet(map(coeffs, sltm[2], {q}), {a(var6), b(var6), c(var6), d(var6),
    m(var6), n(var6), p(var6), o(var6), h(var6)}))
```

$$tmp := \{b\,(h\, m\, n_{x3} - h\, n\, m_{x3} + h\, m_{x6} - h\, n_{x5} - o\, m_{x4} + p\, n_{x4}), d\,(b\, h_{x1} + h\, a_{x2} - h\, b_{x1}), d\,(b\, c\, h_{x2} - b\, d\, h_{x1} - b\, h\, c_{x2} + b\, h\, d_{x1} + d\, h\, a_{x2} - d\, h\, b_{x1}), d\,(h\, m\, o_{x3} - h\, n\, p_{x3} - m\, o\, h_{x3} + n\, p\, h_{x3} - h\, o_{x5} + h\, p_{x6} + o\, h_{x5} - o\, p_{x4} - p\, h_{x6} + p\, o_{x4}), h\,(a_{x2} - b_{x1}), (b^2\, h\, o_{x3} - b^2\, o\, h_{x3} - b\, d\, h\, n_{x3} + b\, d\, n\, h_{x3} - b\, h\, n\, d_{x3} + d\, h\, n\, b_{x3} - b\, d\, h_{x6} + b\, d\, o_{x4} + b\, h\, d_{x6} - b\, o\, d_{x4} - d^2\, n_{x4} - d\, h\, b_{x6} + d\, o\, b_{x4})\,(a\, d - b\, c), h_{x2}\, b\, d, h\, m_{x2} + b_{x4}, a\, h\, m_{x2} - b\, h\, m_{x1} + a\, b_{x4} - b\, a_{x4}, 2\, d\, h_{x3} - h\, d_{x3} - h\, o_{x2} + o\, h_{x2}, -c\, h\, d_{x3} - c\, h\, o_{x2} + c\, o\, h_{x2} + d\, h\, c_{x3} + d\, h\, o_{x1} - d\, o\, h_{x1}, 2\, a\, h\, b_{x3} + a\, h\, n_{x2} - 2\, b\, h\, a_{x3} - b\, h\, n_{x1} + c\, b_{x4} - d\, a_{x4}, -2\, b\, h\, m_{x3} + h\, m\, b_{x3} + b\, n_{x4} - d\, m_{x4} - h\, b_{x5} \quad (92)$$

$+ p\, b_{x4}, a\, h\, m\, b_{x3} - b\, h\, m\, a_{x3} - a\, d\, m_{x4} - a\, h\, b_{x5} + a\, p\, b_{x4} + b\, c\, m_{x4} + b\, h\, a_{x5} - b\, p\, a_{x4},$
$a\, h\, n\, b_{x3} - b\, h\, n\, a_{x3} - a\, d\, n_{x4} - a\, h\, b_{x6} + a\, o\, b_{x4} + b\, c\, n_{x4} + b\, h\, a_{x6} - b\, o\, a_{x4}, b\, h\, o_{x3}$
$- b\, o\, h_{x3} - d\, h\, p_{x3} + 2\, d\, n\, h_{x3} + d\, p\, h_{x3} - h\, n\, d_{x3} - 2\, d\, h_{x6} + 2\, d\, o_{x4} + h\, d_{x6} - o\, d_{x4},$
$-b^2\, h\, d_{x3} - b^2\, h\, o_{x2} + b^2\, o\, h_{x2} + b\, d\, h\, b_{x3} + b\, d\, h\, n_{x2} - b\, d\, h\, p_{x2} + b\, d\, p\, h_{x2} + d^2\, h\, m_{x2}$
$- b\, d\, d_{x4} + d^2\, b_{x4}, -a\, d\, h\, o_{x3} + a\, d\, o\, h_{x3} + b\, c\, h\, o_{x3} - b\, c\, o\, h_{x3} - c\, h\, n\, d_{x3} + d\, h\, n\, c_{x3}$
$+ c\, h\, d_{x6} - c\, o\, d_{x4} - d\, h\, c_{x6} + d\, o\, c_{x4}, -a\, b\, h\, d_{x3} - a\, b\, h\, o_{x2} + a\, b\, o\, h_{x2} + 2\, a\, d\, h\, b_{x3}$
$+ a\, d\, h\, n_{x2} - b\, d\, h\, a_{x3} - b\, d\, h\, p_{x1} + b\, d\, p\, h_{x1} + c\, d\, h\, m_{x2} - b\, d\, c_{x4} + 2\, c\, d\, b_{x4} - d^2\, a_{x4},$
$2\, a\, b\, d^2\, h_{x3} - 2\, a\, b\, d\, h\, d_{x3} - a\, b\, d\, h\, o_{x2} + a\, b\, d\, o\, h_{x2} + 2\, a\, d^2\, h\, b_{x3} + a\, d^2\, h\, n_{x2} - 2\, b^2\, c\, d\, h_{x3}$
$+ b^2\, c\, h\, d_{x3} + b^2\, c\, h\, o_{x2} - b^2\, c\, o\, h_{x2} + b^2\, d\, h\, c_{x3} - b\, c\, d\, h\, b_{x3} - b\, c\, d\, h\, n_{x2} - b\, d^2\, h\, a_{x3}$
$- b\, c\, d\, d_{x4} + b\, d^2\, c_{x4} + c\, d^2\, b_{x4} - d^3\, a_{x4}, b^3\, h\, o_{x3} - b^3\, o\, h_{x3} - b^2\, d\, h\, n_{x3} + b^2\, d\, h\, p_{x3}$
$+ b^2\, d\, n\, h_{x3} - b^2\, d\, p\, h_{x3} - b^2\, h\, n\, d_{x3} - b\, d^2\, h\, m_{x3} + b\, d^2\, m\, h_{x3} - b\, d\, h\, m\, d_{x3} + b\, d\, h\, n\, b_{x3}$
$+ d^2\, h\, m\, b_{x3} - b^2\, d\, h_{x6} + b^2\, d\, o_{x4} + b^2\, h\, d_{x6} - b^2\, o\, d_{x4} - b\, d^2\, h_{x5} - b\, d^2\, n_{x4} + b\, d^2\, p_{x4}$
$- b\, d\, h\, b_{x6} + b\, d\, h\, d_{x5} + b\, d\, o\, b_{x4} - b\, d\, p\, d_{x4} - d^3\, m_{x4} - d^2\, h\, b_{x5} + d^2\, p\, b_{x4}, a\, b^2\, h\, o_{x3}$
$- a\, b^2\, o\, h_{x3} - a\, b\, d\, h\, n_{x3} + a\, b\, d\, h\, p_{x3} + a\, b\, d\, n\, h_{x3} - a\, b\, d\, p\, h_{x3} - a\, b\, h\, n\, d_{x3} + a\, d\, h\, n\, b_{x3}$
$- b\, c\, d\, h\, m_{x3} + b\, c\, d\, m\, h_{x3} - b\, d\, h\, m\, c_{x3} + c\, d\, h\, m\, b_{x3} - a\, b\, d\, h_{x6} + a\, b\, d\, o_{x4} + a\, b\, h\, d_{x6}$
$- a\, b\, o\, d_{x4} - a\, d^2\, n_{x4} - a\, d\, h\, b_{x6} + a\, d\, o\, b_{x4} - b\, c\, d\, h_{x5} + b\, c\, d\, p_{x4} + b\, d\, h\, c_{x5} - b\, d\, p\, c_{x4}$
$- c\, d^2\, m_{x4} - c\, d\, h\, b_{x5} + c\, d\, p\, b_{x4}\}$

> simplify(eval(tmp, {$a_{x2} = b_{x1}, c_{x2} = d_{x1}, h_{x1} = 0, h_{x2} = 0$}))

$\{0, b\, ((m\, n_{x3} - n\, m_{x3} + m_{x6} - n_{x5})\, h + p\, n_{x4} - o\, m_{x4}), d\, ((m\, o_{x3} - n\, p_{x3} - o_{x5} + p_{x6})\, h + ($ **(93)**
$-m\, h_{x3} + h_{x5} - p_{x4})\, o + p\, (n\, h_{x3} - h_{x6} + o_{x4})), -h\, ((d_{x3} + o_{x2})\, c - d\, (c_{x3} + o_{x1})),$
$-(a\, d - b\, c)\, ((-h\, o_{x3} + o\, h_{x3})\, b^2 + ((h\, n_{x3} - n\, h_{x3} + h_{x6} - o_{x4})\, d + (n\, d_{x3} - d_{x6})\, h$
$+ o\, d_{x4})\, b + (n_{x4}\, d + (-n\, b_{x3} + b_{x6})\, h - o\, b_{x4})\, d), (-d_{x3} - o_{x2})\, h + 2\, d\, h_{x3}, ((b\, o_{x3}$
$- n\, d_{x3} + d_{x6})\, c - d\, (a\, o_{x3} - n\, c_{x3} + c_{x6}))\, h + ((-b\, h_{x3} - d_{x4})\, c + d\, (a\, h_{x3} + c_{x4}))\, o,$
$((m\, b_{x3} - b_{x5})\, h + p\, b_{x4} - d\, m_{x4})\, a + b\, ((-m\, a_{x3} + a_{x5})\, h + m_{x4}\, c - p\, a_{x4}), ((n\, b_{x3}$
$- b_{x6})\, h + o\, b_{x4} - n_{x4}\, d)\, a + b\, ((-n\, a_{x3} + a_{x6})\, h + n_{x4}\, c - o\, a_{x4}), (h\, m_{x2} + b_{x4})\, a$

$-b\,(h\,m_{x1}+a_{x4}), -d^2\,a_{x4}+(((-p_{x1}-a_{x3})\,b+(n_{x2}+2\,b_{x3})\,a+m_{x2}\,c)\,h+2\,c\,b_{x4}$

$-c_{x4}\,b)\,d-a\,b\,h\,(d_{x3}+o_{x2}), ((n_{x2}+2\,b_{x3})\,a-b\,(n_{x1}+2\,a_{x3}))\,h+c\,b_{x4}-d\,a_{x4}, ($

$-p_{x3}\,h+(2\,n+p)\,h_{x3}-2\,h_{x6}+2\,o_{x4})\,d+(b\,o_{x3}-n\,d_{x3}+d_{x6})\,h-o\,(b\,h_{x3}+d_{x4}), ($

$-a\,n_{x4}-m_{x4}\,c)\,d^2+((((-n_{x3}+p_{x3})\,h+(n-p)\,h_{x3}-h_{x6}+o_{x4})\,a+(-c\,m_{x3}-m\,c_{x3}$

$+c_{x5})\,h+(m\,h_{x3}-h_{x5}+p_{x4})\,c-c_{x4}\,p)\,b+((n\,b_{x3}-b_{x6})\,h+o\,b_{x4})\,a+c\,((m\,b_{x3}$

$-b_{x5})\,h+p\,b_{x4}))\,d-a\,b\,((-h\,o_{x3}+o\,h_{x3})\,b+(n\,d_{x3}-d_{x6})\,h+o\,d_{x4}), -h\,(d_{x3}$

$+o_{x2})\,b^2-((p_{x2}-b_{x3}-n_{x2})\,h+d_{x4})\,d\,b+d^2\,(h\,m_{x2}+b_{x4}), -d^3\,a_{x4}+((2\,a\,h_{x3}$

$-h\,a_{x3}+c_{x4})\,b+a\,(n_{x2}+2\,b_{x3})\,h+c\,b_{x4})\,d^2-2\,b\left(\left(-\frac{c_{x3}\,h}{2}+h_{x3}\,c\right)b\right.$

$\left.+\left(\frac{(n_{x2}+b_{x3})\,c}{2}+a\left(d_{x3}+\frac{o_{x2}}{2}\right)\right)h+\frac{d_{x4}\,c}{2}\right)d+b^2\,c\,h\,(d_{x3}+o_{x2}), (h\,o_{x3}$

$-o\,h_{x3})\,b^3+(((-n_{x3}+p_{x3})\,h+(n-p)\,h_{x3}-h_{x6}+o_{x4})\,d+(-n\,d_{x3}+d_{x6})\,h$

$-o\,d_{x4})\,b^2-((h\,m_{x3}-m\,h_{x3}+h_{x5}+n_{x4}-p_{x4})\,d+(m\,d_{x3}-n\,b_{x3}+b_{x6}-d_{x5})\,h+d_{x4}\,p$

$-o\,b_{x4})\,d\,b-(d\,m_{x4}+(-m\,b_{x3}+b_{x5})\,h-p\,b_{x4})\,d^2, (-2\,b\,m_{x3}+m\,b_{x3}-b_{x5})\,h+b\,n_{x4}$

$-d\,m_{x4}+p\,b_{x4}, h\,m_{x2}+b_{x4}\}$

The first equations yield $a=u_1$, $b=u_2$, $c=v_1$, $d=v_2$, $h=h(x3,x4,x5,x6)$;

then the equations $h\,m_{x1}+a_{x4}=0, h\,m_{x2}+b_{x4}=0$ imply $m=-\frac{u_4}{h}+f(x3,x4,x5,x6)$, and $(d_{x3}+o_{x2})\,c-d\,(c_{x3}+o_{x1})=0$, $2\,d\,h_{x3}=(d_{x3}+o_{x2})\,h$ imply (intermediate $o=f2(v,x3,x4,x5,x6)-v_3$ and then) $o=\frac{2\,h_{x3}}{h}\,v-v_3+g(x3,x4,x5,x6)$.

Note that change of $u$ and $v$ by a function of $(x3,x4,x5,x6)$ eliminates $f$ and $g$. Collecting also the type of $S1..S4$ behavior in $q$ we restart

$> V1 := evalDG\left(q\ D\_x1-diff(u(var6),x1)\ D\_x3-\frac{diff(v(var6),x1)}{h(x3,x4,x5,x6)}\ D\_x4+(w1(var6)\ q+z1(var6))\ D\_q\right):$

$V2 := evalDG\left(q\ D\_x2-diff(u(var6),x2)\ D\_x3-\frac{diff(v(var6),x2)}{h(x3,x4,x5,x6)}\ D\_x4+(w2(var6)\ q+z2(var6))\ D\_q\right):$

```
V3 := evalDG(D_x5 + diff(u(var6), x4)/h(x3, x4, x5, x6) D_x3 - (m(var6) + q)/h(x3, x4, x5, x6) D_x4 + q (z3(var6) q
      + w3(var6)) D_q) :
V4 := evalDG(D_x6 - (n(var6) + q) D_x3 + (diff(v(var6), x3)/h(x3, x4, x5, x6)
      - 2 diff(h(x3, x4, x5, x6), x3)/h(x3, x4, x5, x6)^2 v(var6)) D_x4 + q (z4(var6) q + w4(var6)) D_q) :
```

```
> V12 := evalDG(LieDerivative(V1, V2) + (w2(var6) q + z2(var6))/q V1
      - (w1(var6) q + z1(var6))/q V2) : V13 := evalDG(LieDerivative(V1, V3) + (z3(var6) q
      + w3(var6)) V1) : V23 := evalDG(LieDerivative(V2, V3) + (z3(var6) q
      + w3(var6)) V2) : V14 := evalDG(LieDerivative(V1, V4) + (z4(var6) q
      + w4(var6)) V1) : V24 := evalDG(LieDerivative(V2, V4) + (z4(var6) q
      + w4(var6)) V2) : V34 := evalDG(LieDerivative(V3, V4)) :
```

```
> LieDerivative(V12, x1), LieDerivative(V12, x2), LieDerivative(V12, x5), LieDerivative(V12,
      x6), LieDerivative(V13, x1), LieDerivative(V13, x2), LieDerivative(V13, x5),
      LieDerivative(V13, x6), LieDerivative(V23, x1), LieDerivative(V23, x2),
      LieDerivative(V23, x5), LieDerivative(V23, x6), LieDerivative(V14, x1),
      LieDerivative(V14, x2), LieDerivative(V14, x5), LieDerivative(V14, x6),
      LieDerivative(V24, x1), LieDerivative(V24, x2), LieDerivative(V24, x5),
      LieDerivative(V24, x6), LieDerivative(V34, x1), LieDerivative(V34, x2),
      LieDerivative(V34, x5), LieDerivative(V34, x6)
```

$$0, 0, 0, 0, 0, 0, 0, 0, 0, 0, 0, 0, 0, 0, 0, 0, 0, 0, 0, 0, 0, 0, 0, 0 \qquad (94)$$

```
> collect(ToJet(numer(LieDerivative(V12, q)), {u(var6), v(var6), w1(var6), w2(var6),
      w3(var6), w4(var6), z1(var6), z2(var6), z3(var6), z4(var6), m(var6), n(var6), h(x3, x4,
      x5, x6)}), {q});
  collect(ToJet(numer(LieDerivative(V13, q)), {u(var6), v(var6), w1(var6), w2(var6),
      w3(var6), w4(var6), z1(var6), z2(var6), z3(var6), z4(var6), m(var6), n(var6), h(x3, x4,
      x5, x6)}), {q});
  collect(ToJet(numer(LieDerivative(V23, q)), {u(var6), v(var6), w1(var6), w2(var6),
      w3(var6), w4(var6), z1(var6), z2(var6), z3(var6), z4(var6), m(var6), n(var6), h(x3, x4,
      x5, x6)}), {q});
  collect(ToJet(numer(LieDerivative(V14, q)), {u(var6), v(var6), w1(var6), w2(var6),
      w3(var6), w4(var6), z1(var6), z2(var6), z3(var6), z4(var6), m(var6), n(var6), h(x3, x4,
      x5, x6)}), {q});
  collect(ToJet(numer(LieDerivative(V24, q)), {u(var6), v(var6), w1(var6), w2(var6),
      w3(var6), w4(var6), z1(var6), z2(var6), z3(var6), z4(var6), m(var6), n(var6), h(x3, x4,
      x5, x6)}), {q});
  collect(ToJet(numer(LieDerivative(V34, q)), {u(var6), v(var6), w1(var6), w2(var6),
      w3(var6), w4(var6), z1(var6), z2(var6), z3(var6), z4(var6), m(var6), n(var6), h(x3, x4,
      x5, x6)}), {q})
```

$$\left(-h\, w1_{x2} + h\, w2_{x1}\right) q^2 + \left(-h\, u_{x1}\, w2_{x3} + h\, u_{x2}\, w1_{x3} - h\, z1_{x2} + h\, z2_{x1} - v_{x1}\, w2_{x4} + v_{x2}\, w1_{x4}\right) q \\ - h\, w1\, z2 + h\, w2\, z1 - h\, u_{x1}\, z2_{x3} + h\, u_{x2}\, z1_{x3} - z2_{x4}\, v_{x1} + z1_{x4}\, v_{x2}$$

$$h\, z3_{x1}\, q^3 + \left(2\, h\, w1\, z3 - h\, u_{x1}\, z3_{x3} + h\, w3_{x1} - v_{x1}\, z3_{x4} + w1_{x4}\right) q^2 + \left(h\, w1\, w3 + 3\, h\, z1\, z3 - h\, u_{x1}\, w3_{x3} - h\, w1_{x5} + m\, w1_{x4} - u_{x4}\, w1_{x3} - v_{x1}\, w3_{x4} + z1_{x4}\right) q + 2\, h\, w3\, z1 - h\, z1_{x5} + m\, z1_{x4} - z1_{x3}\, u_{x4}$$

$$h\, z3_{x2}\, q^3 + \left(2\, h\, w2\, z3 - h\, u_{x2}\, z3_{x3} + h\, w3_{x2} - v_{x2}\, z3_{x4} + w2_{x4}\right) q^2 + \left(h\, w2\, w3 + 3\, h\, z2\, z3 - h\, u_{x2}\, w3_{x3} - h\, w2_{x5} + m\, w2_{x4} - u_{x4}\, w2_{x3} - v_{x2}\, w3_{x4} + z2_{x4}\right) q + 2\, h\, w3\, z2 - h\, z2_{x5} + m\, z2_{x4} - z2_{x3}\, u_{x4}$$

$$h^2\, z4_{x1}\, q^3 + \left(2\, h^2\, w1\, z4 - h^2\, u_{x1}\, z4_{x3} + h^2\, w1_{x3} + h^2\, w4_{x1} - h\, v_{x1}\, z4_{x4}\right) q^2 + \left(h^2\, n\, w1_{x3} + h^2\, w1\, w4 + 3\, h^2\, z1\, z4 - h^2\, u_{x1}\, w4_{x3} - h^2\, w1_{x6} + h^2\, z1_{x3} - h\, v_{x1}\, w4_{x4} - h\, v_{x3}\, w1_{x4} + 2\, v\, h_{x3}\, w1_{x4}\right) q + h^2\, n\, z1_{x3} + 2\, h^2\, w4\, z1 - h^2\, z1_{x6} - h\, v_{x3}\, z1_{x4} + 2\, v\, h_{x3}\, z1_{x4}$$

$$h^2\, z4_{x2}\, q^3 + \left(2\, h^2\, w2\, z4 - h^2\, u_{x2}\, z4_{x3} + h^2\, w2_{x3} + h^2\, w4_{x2} - h\, v_{x2}\, z4_{x4}\right) q^2 + \left(h^2\, n\, w2_{x3} + h^2\, w2\, w4 + 3\, h^2\, z2\, z4 - h^2\, u_{x2}\, w4_{x3} - h^2\, w2_{x6} + h^2\, z2_{x3} - h\, v_{x2}\, w4_{x4} - h\, v_{x3}\, w2_{x4} + 2\, v\, h_{x3}\, w2_{x4}\right) q + h^2\, n\, z2_{x3} + 2\, h^2\, w4\, z2 - h^2\, z2_{x6} - h\, v_{x3}\, z2_{x4} + 2\, v\, h_{x3}\, z2_{x4}$$

$$\left(h^2\, z3_{x3} - h\, z4_{x4}\right) q^3 + \left(h^2\, n\, z3_{x3} + h^2\, w3\, z4 - h^2\, w4\, z3 + h^2\, w3_{x3} - h^2\, z3_{x6} + h^2\, z4_{x5} - h\, m\, z4_{x4} + h\, u_{x4}\, z4_{x3} - h\, v_{x3}\, z3_{x4} + 2\, v\, h_{x3}\, z3_{x4} - h\, w4_{x4}\right) q^2 + \left(w3_{x3}\, h^2\, n - w3_{x6}\, h^2 + w4_{x5}\, h^2 - m\, h\, w4_{x4} + u_{x4}\, h\, w4_{x3} - w3_{x4}\, v_{x3}\, h + 2\, w3_{x4}\, h_{x3}\, v\right) q \tag{95}$$

Let us adjust $w$ by using the coefficients of $q^3$ and restart

> $V1 := evalDG\left(q\ D\_x1 - diff(u(var6), x1)\ D\_x3 - \frac{diff(v(var6), x1)}{h(x3, x4, x5, x6)}\ D\_x4 + (diff(w(var6), x1)\ q + z1(var6))\ D\_q\right):$
>
> $V2 := evalDG\left(q\ D\_x2 - diff(u(var6), x2)\ D\_x3 - \frac{diff(v(var6), x2)}{h(x3, x4, x5, x6)}\ D\_x4 + (diff(w(var6), x2)\ q + z2(var6))\ D\_q\right):$
>
> $V3 := evalDG\left(D\_x5 + \frac{diff(u(var6), x4)}{h(x3, x4, x5, x6)}\ D\_x3 - \frac{m(var6) + q}{h(x3, x4, x5, x6)}\ D\_x4 + q\ (z3(x3, x4, x5, x6)\ q + w3(var6))\ D\_q\right):$
>
> $V4 := evalDG\left(D\_x6 - (n(var6) + q)\ D\_x3 + \left(\frac{diff(v(var6), x3)}{h(x3, x4, x5, x6)} - \frac{2\ diff(h(x3, x4, x5, x6), x3)\ v(var6)}{h(x3, x4, x5, x6)^2}\right) D\_x4 + q\ (z4(x3, x4, x5, x6)\ q + w4(var6))\ D\_q\right):$

> $V12 := evalDG\left(LieDerivative(V1, V2) + \frac{diff(w(var6), x2)\ q + z2(var6)}{q}\ V1\right.$

```
 - (diff(w(var6), x1) q + z1(var6))/q V2) : V13 := evalDG(LieDerivative(V1, V3)
 + (z3(x3, x4, x5, x6) q + w3(var6)) V1) : V23 := evalDG(LieDerivative(V2, V3)
 + (z3(x3, x4, x5, x6) q + w3(var6)) V2) : V14 := evalDG(LieDerivative(V1, V4)
 + (z4(x3, x4, x5, x6) q + w4(var6)) V1) : V24 := evalDG(LieDerivative(V2, V4)
 + (z4(x3, x4, x5, x6) q + w4(var6)) V2) : V34 := evalDG(LieDerivative(V3, V4)) :
```

```
> LieDerivative(V12, x1), LieDerivative(V12, x2), LieDerivative(V12, x5), LieDerivative(V12,
    x6), LieDerivative(V13, x1), LieDerivative(V13, x2), LieDerivative(V13, x5),
    LieDerivative(V13, x6), LieDerivative(V23, x1), LieDerivative(V23, x2),
    LieDerivative(V23, x5), LieDerivative(V23, x6), LieDerivative(V14, x1),
    LieDerivative(V14, x2), LieDerivative(V14, x5), LieDerivative(V14, x6),
    LieDerivative(V24, x1), LieDerivative(V24, x2), LieDerivative(V24, x5),
    LieDerivative(V24, x6), LieDerivative(V34, x1), LieDerivative(V34, x2),
    LieDerivative(V34, x5), LieDerivative(V34, x6)
```

$$0, 0, 0, 0, 0, 0, 0, 0, 0, 0, 0, 0, 0, 0, 0, 0, 0, 0, 0, 0, 0, 0, 0, 0 \tag{96}$$

```
> collect(ToJet(numer(LieDerivative(V12, q))), {u(var6), v(var6), w(var6), w3(var6),
    w4(var6), z1(var6), z2(var6), z3(x3, x4, x5, x6), z4(x3, x4, x5, x6), m(var6), n(var6),
    h(x3, x4, x5, x6)}), {q});
  collect(ToJet(numer(LieDerivative(V13, q))), {u(var6), v(var6), w(var6), w3(var6),
    w4(var6), z1(var6), z2(var6), z3(x3, x4, x5, x6), z4(x3, x4, x5, x6), m(var6), n(var6),
    h(x3, x4, x5, x6)}), {q});
  collect(ToJet(numer(LieDerivative(V23, q))), {u(var6), v(var6), w(var6), w3(var6),
    w4(var6), z1(var6), z2(var6), z3(x3, x4, x5, x6), z4(x3, x4, x5, x6), m(var6), n(var6),
    h(x3, x4, x5, x6)}), {q});
  collect(ToJet(numer(LieDerivative(V14, q))), {u(var6), v(var6), w(var6), w3(var6),
    w4(var6), z1(var6), z2(var6), z3(x3, x4, x5, x6), z4(x3, x4, x5, x6), m(var6), n(var6),
    h(x3, x4, x5, x6)}), {q});
  collect(ToJet(numer(LieDerivative(V24, q))), {u(var6), v(var6), w(var6), w3(var6),
    w4(var6), z1(var6), z2(var6), z3(x3, x4, x5, x6), z4(x3, x4, x5, x6), m(var6), n(var6),
    h(x3, x4, x5, x6)}), {q});
  collect(ToJet(numer(LieDerivative(V34, q))), {u(var6), v(var6), w(var6), w3(var6),
    w4(var6), z1(var6), z2(var6), z3(x3, x4, x5, x6), z4(x3, x4, x5, x6), m(var6), n(var6),
    h(x3, x4, x5, x6)}), {q})
```

$$\left(-h\, u_{x1}\, w_{x3,x2} + h\, u_{x2}\, w_{x3,x1} - h\, z1_{x2} + h\, z2_{x1} - v_{x1}\, w_{x4,x2} + v_{x2}\, w_{x4,x1}\right) q + h\, z1\, w_{x2} - h\, z2\, w_{x1} - h\, u_{x1}\, z2_{x3} + h\, u_{x2}\, z1_{x3} - z2_{x4}\, v_{x1} + z1_{x4}\, v_{x2}$$

$$\left(2\, h\, z3\, w_{x1} - h\, u_{x1}\, z3_{x3} + h\, w3_{x1} - v_{x1}\, z3_{x4} + w_{x4,x1}\right) q^2 + \left(h\, w3\, w_{x1} + 3\, h\, z1\, z3 - h\, u_{x1}\, w3_{x3} - h\, w_{x5,x1} + m\, w_{x4,x1} - u_{x4}\, w_{x3,x1} - v_{x1}\, w3_{x4} + z1_{x4}\right) q + 2\, h\, w3\, z1 - h\, z1_{x5} + m\, z1_{x4} - z1_{x3}\, u_{x4}$$

$$\left(2\, h\, z3\, w_{x2} - h\, u_{x2}\, z3_{x3} + h\, w3_{x2} - v_{x2}\, z3_{x4} + w_{x4,x2}\right) q^2 + \left(h\, w3\, w_{x2} + 3\, h\, z2\, z3 - h\, u_{x2}\, w3_{x3} - h\, w_{x5,x2} + m\, w_{x4,x2} - u_{x4}\, w_{x3,x2} - v_{x2}\, w3_{x4} + z2_{x4}\right) q + 2\, h\, w3\, z2 - h\, z2_{x5} + m\, z2_{x4} - z2_{x3}\, u_{x4}$$

$$\left(2\, h^2\, z4\, w_{x1} - h^2\, u_{x1}\, z4_{x3} + h^2\, w_{x3,x1} + h^2\, w4_{x1} - h\, v_{x1}\, z4_{x4}\right) q^2 + \left(h^2\, n\, w_{x3,x1} + h^2\, w4\, w_{x1}\right.$$

$$+ 3h^2 z1\,z4 - h^2 u_{x1} w4_{x3} - h^2 w_{x6,x1} + h^2 z1_{x3} - h\,v_{x1} w4_{x4} - h\,v_{x3} w_{x4,x1} + 2\,v\,h_{x3} w_{x4,x1}\big)\,q$$

$$+ h^2 n\,z1_{x3} + 2h^2 w4\,z1 - h^2 z1_{x6} - h\,v_{x3} z1_{x4} + 2\,v\,h_{x3} z1_{x4}$$

$$\left(2h^2 z4\,w_{x2} - h^2 u_{x2} z4_{x3} + h^2 w_{x3,x2} + h^2 w4_{x2} - h\,v_{x2} z4_{x4}\right) q^2 + \big(h^2 n\,w_{x3,x2} + h^2 w4\,w_{x2}$$

$$+ 3h^2 z2\,z4 - h^2 u_{x2} w4_{x3} - h^2 w_{x6,x2} + h^2 z2_{x3} - h\,v_{x2} w4_{x4} - h\,v_{x3} w_{x4,x2} + 2\,v\,h_{x3} w_{x4,x2}\big)\,q$$

$$+ h^2 n\,z2_{x3} + 2h^2 w4\,z2 - h^2 z2_{x6} - h\,v_{x3} z2_{x4} + 2\,v\,h_{x3} z2_{x4}$$

$$\left(h^2 z3_{x3} - h\,z4_{x4}\right) q^3 + \big(h^2 n\,z3_{x3} + h^2 w3\,z4 - h^2 w4\,z3 + h^2 w3_{x3} - h^2 z3_{x6} + h^2 z4_{x5} - h\,m\,z4_{x4} \tag{97}$$

$$+ h\,u_{x4} z4_{x3} - h\,v_{x3} z3_{x4} + 2\,v\,h_{x3} z3_{x4} - h\,w4_{x4}\big)\,q^2 + \big(w3_{x3} h^2 n - w3_{x6} h^2 + w4_{x5} h^2$$

$$- m\,h\,w4_{x4} + u_{x4} h\,w4_{x3} - w3_{x4} v_{x3} h + 2\,w3_{x4} h_{x3} v\big)\,q$$

Again we can adjust $w$ by using the coefficients of $q^2$, eliminate one of the arising functions of four arguments and restart

$$> V1 := evalDG\Big(q\,D\_x1 - diff(u(var6), x1)\,D\_x3 - \frac{diff(v(var6), x1)}{h(x3, x4, x5, x6)}\,D\_x4 + (diff(w(var6), x1)\,q + z1(var6))\,D\_q\Big):$$

$$V2 := evalDG\Big(q\,D\_x2 - diff(u(var6), x2)\,D\_x3 - \frac{diff(v(var6), x2)}{h(x3, x4, x5, x6)}\,D\_x4 + (diff(w(var6), x2)\,q + z2(var6))\,D\_q\Big):$$

$$V3 := evalDG\Big(D\_x5 + \frac{diff(u(var6), x4)}{h(x3, x4, x5, x6)}\,D\_x3 - \frac{m(var6) + q}{h(x3, x4, x5, x6)}\,D\_x4 + q\,\Big(z3(x3, x4, x5, x6)\,q - \frac{diff(w(var6), x4)}{h(x3, x4, x5, x6)} - 2\,z3(x3, x4, x5, x6)\,w(var6) + diff(z3(x3, x4, x5, x6), x3)\,u(var6) + diff(z3(x3, x4, x5, x6), x4)\,\frac{v(var6)}{h(x3, x4, x5, x6)}\Big)\,D\_q\Big):$$

$$V4 := evalDG\Big(D\_x6 - (n(var6) + q)\,D\_x3 + \Big(\frac{diff(v(var6), x3)}{h(x3, x4, x5, x6)} - \frac{2\,diff(h(x3, x4, x5, x6), x3)}{h(x3, x4, x5, x6)^2}\,v(var6)\Big)\,D\_x4 + q\,\Big(z4(x3, x4, x5, x6)\,q - diff(w(var6), x3) - 2\,z4(x3, x4, x5, x6)\,w(var6) + diff(z4(x3, x4, x5, x6), x3)\,u(var6) + \frac{diff(z4(x3, x4, x5, x6), x4)}{h(x3, x4, x5, x6)}\,v(var6) + f(x3, x4, x5, x6)\Big)\,D\_q\Big):$$

$$> V12 := evalDG\Big(LieDerivative(V1, V2) + \frac{diff(w(var6), x2)\,q + z2(var6)}{q}\,V1 - \frac{diff(w(var6), x1)\,q + z1(var6)}{q}\,V2\Big) : V13 := evalDG\Big(LieDerivative(V1, V3) + \Big(z3(x3, x4, x5, x6)\,q - \frac{diff(w(var6), x4)}{h(x3, x4, x5, x6)} - 2\,z3(x3, x4, x5, x6)\,w(var6) + diff(z3(x3, x4, x5, x6), x3)\,u(var6) + diff(z3(x3, x4, x5, x6), x4)\,\frac{v(var6)}{h(x3, x4, x5, x6)}\Big)$$

$V1\Big)$ : $V23 := evalDG\Big(LieDerivative(V2, V3) + \Big(z3(x3, x4, x5, x6)\, q - \frac{diff(w(var6), x4)}{h(x3, x4, x5, x6)} - 2\, z3(x3, x4, x5, x6)\, w(var6) + diff(z3(x3, x4, x5, x6), x3)\, u(var6) + diff(z3(x3, x4, x5, x6), x4)\, \frac{v(var6)}{h(x3, x4, x5, x6)}\Big)\, V2\Big)$ : $V14 := evalDG\Big(LieDerivative(V1, V4) + \Big(z4(x3, x4, x5, x6)\, q - diff(w(var6), x3) - 2\, z4(x3, x4, x5, x6)\, w(var6) + diff(z4(x3, x4, x5, x6), x3)\, u(var6) + diff(z4(x3, x4, x5, x6), x4)\, \frac{v(var6)}{h(x3, x4, x5, x6)} + f(x3, x4, x5, x6)\Big)\, V1\Big)$ : $V24 := evalDG\Big(LieDerivative(V2, V4) + \Big(z4(x3, x4, x5, x6)\, q - diff(w(var6), x3) - 2\, z4(x3, x4, x5, x6)\, w(var6) + diff(z4(x3, x4, x5, x6), x3)\, u(var6) + diff(z4(x3, x4, x5, x6), x4)\, \frac{v(var6)}{h(x3, x4, x5, x6)} + f(x3, x4, x5, x6)\Big)\, V2\Big)$ : $V34 := evalDG(LieDerivative(V3, V4))$ :

> LieDerivative(V12, x1), LieDerivative(V12, x2), LieDerivative(V12, x5), LieDerivative(V12, x6), LieDerivative(V13, x1), LieDerivative(V13, x2), LieDerivative(V13, x5), LieDerivative(V13, x6), LieDerivative(V23, x1), LieDerivative(V23, x2), LieDerivative(V23, x5), LieDerivative(V23, x6), LieDerivative(V14, x1), LieDerivative(V14, x2), LieDerivative(V14, x5), LieDerivative(V14, x6), LieDerivative(V24, x1), LieDerivative(V24, x2), LieDerivative(V24, x5), LieDerivative(V24, x6), LieDerivative(V34, x1), LieDerivative(V34, x2), LieDerivative(V34, x5), LieDerivative(V34, x6)

0, 0, 0, 0, 0, 0, 0, 0, 0, 0, 0, 0, 0, 0, 0, 0, 0, 0, 0, 0, 0, 0, 0, 0 **(98)**

> # collect(ToJet(numer(LieDerivative(V12, q)), {u(var6), v(var6), w(var6), z1(var6), z2(var6), z3(x3, x4, x5, x6), z4(x3, x4, x5, x6), m(var6), n(var6), h(x3, x4, x5, x6)}), {q});
# collect(ToJet(numer(LieDerivative(V13, q)), {u(var6), v(var6), w(var6), z1(var6), z2(var6), z3(x3, x4, x5, x6), z4(x3, x4, x5, x6), m(var6), n(var6), h(x3, x4, x5, x6)}), {q});
# collect(ToJet(numer(LieDerivative(V23, q)), {u(var6), v(var6), w(var6), z1(var6), z2(var6), z3(x3, x4, x5, x6), z4(x3, x4, x5, x6), m(var6), n(var6), h(x3, x4, x5, x6)}), {q});
# collect(ToJet(numer(LieDerivative(V14, q)), {u(var6), v(var6), w(var6), z1(var6), z2(var6), z3(x3, x4, x5, x6), z4(x3, x4, x5, x6), m(var6), n(var6), h(x3, x4, x5, x6)}), {q});
# collect(ToJet(numer(LieDerivative(V24, q)), {u(var6), v(var6), w(var6), z1(var6), z2(var6), z3(x3, x4, x5, x6), z4(x3, x4, x5, x6), m(var6), n(var6), h(x3, x4, x5, x6)}), {q});
# collect(ToJet(numer(LieDerivative(V34, q)), {u(var6), v(var6), w(var6), z1(var6), z2(var6), z3(x3, x4, x5, x6), z4(x3, x4, x5, x6), m(var6), n(var6), h(x3, x4, x5, x6)}), {q})

> tmp1 := DGinfo(V12, "CoefficientSet") : tmp2 := DGinfo(V13, "CoefficientSet") : tmp3 := DGinfo(V23, "CoefficientSet") : tmp4 := DGinfo(V14, "CoefficientSet") : tmp5 := DGinfo(V24, "CoefficientSet") : tmp6 := DGinfo(V34, "CoefficientSet") :
tmp := tmp1 **union** tmp2 **union** tmp3 **union** tmp4 **union** tmp5 **union** tmp6 :

> tmp := factor(ToJet(map(coeffs, expand(numer(tmp)), {q}), {u(var6), v(var6), w(var6), z1(var6), z2(var6), z3(x3, x4, x5, x6), z4(x3, x4, x5, x6), m(var6), n(var6), h(x3, x4, x5, x6), f(x3, x4, x5, x6)})) :

> $tmp[1..2]$

$$\{h\,(z1\,u_{x2}-z2\,u_{x1}),\,h\,(z1\,v_{x2}-z2\,v_{x1})\}\tag{99}$$

Since general solutions $u,v$ are independent as functions of $x1,x2$, we conclude $z1=z2=0$. Adjust and restart

> $V1 := evalDG\left(q\,D\_x1-diff(u(var6),x1)\,D\_x3-\frac{diff(v(var6),x1)}{h(x3,x4,x5,x6)}\,D\_x4+diff(w(var6),x1)\,q\,D\_q\right):$
$V2 := evalDG\left(q\,D\_x2-diff(u(var6),x2)\,D\_x3-\frac{diff(v(var6),x2)}{h(x3,x4,x5,x6)}\,D\_x4+diff(w(var6),x2)\,q\,D\_q\right):$
$V3 := evalDG\left(D\_x5+\frac{diff(u(var6),x4)}{h(x3,x4,x5,x6)}\,D\_x3-\frac{m(var6)+q}{h(x3,x4,x5,x6)}\,D\_x4+q\left(z3(x3,x4,x5,x6)\,q-\frac{diff(w(var6),x4)}{h(x3,x4,x5,x6)}-2\,z3(x3,x4,x5,x6)\,w(var6)+diff(z3(x3,x4,x5,x6),x3)\,u(var6)+diff(z3(x3,x4,x5,x6),x4)\,\frac{v(var6)}{h(x3,x4,x5,x6)}\right)D\_q\right):$
$V4 := evalDG\left(D\_x6-(n(var6)+q)\,D\_x3+\left(\frac{diff(v(var6),x3)}{h(x3,x4,x5,x6)}-\frac{2\,diff(h(x3,x4,x5,x6),x3)\,v(var6)}{h(x3,x4,x5,x6)^2}\right)D\_x4+q\left(z4(x3,x4,x5,x6)\,q-diff(w(var6),x3)-2\,z4(x3,x4,x5,x6)\,w(var6)+diff(z4(x3,x4,x5,x6),x3)\,u(var6)+diff(z4(x3,x4,x5,x6),x4)\,\frac{v(var6)}{h(x3,x4,x5,x6)}+f(x3,x4,x5,x6)\right)D\_q\right):$

> $V12 := evalDG\left(LieDerivative(V1,V2)+\frac{diff(w(var6),x2)\,q}{q}\,V1-\frac{diff(w(var6),x1)\,q}{q}\,V2\right): V13 := evalDG\left(LieDerivative(V1,V3)+\left(z3(x3,x4,x5,x6)\,q-\frac{diff(w(var6),x4)}{h(x3,x4,x5,x6)}-2\,z3(x3,x4,x5,x6)\,w(var6)+diff(z3(x3,x4,x5,x6),x3)\,u(var6)+diff(z3(x3,x4,x5,x6),x4)\,\frac{v(var6)}{h(x3,x4,x5,x6)}\right)V1\right): V23 := evalDG\left(LieDerivative(V2,V3)+\left(z3(x3,x4,x5,x6)\,q-\frac{diff(w(var6),x4)}{h(x3,x4,x5,x6)}-2\,z3(x3,x4,x5,x6)\,w(var6)+diff(z3(x3,x4,x5,x6),x3)\,u(var6)+diff(z3(x3,x4,x5,x6),x4)\,\frac{v(var6)}{h(x3,x4,x5,x6)}\right)V2\right): V14 := evalDG\left(LieDerivative(V1,V4)+\left(z4(x3,x4,x5,x6)\,q-diff(w(var6),x3)-2\,z4(x3,x4,x5,x6)\,w(var6)+diff(z4(x3,x4,x5,x6),x3)\,u(var6)+diff(z4(x3,x4,x5,x6),x4)\,\frac{v(var6)}{h(x3,x4,x5,x6)}+f(x3,x4,x5,x6)\right)V1\right):$

$V24 := evalDG\Big(LieDerivative(V2, V4) + \Big(z4(x3, x4, x5, x6)\, q - diff(w(var6), x3) - 2\, z4(x3, x4, x5, x6)\, w(var6) + diff(z4(x3, x4, x5, x6), x3)\, u(var6) + diff(z4(x3, x4, x5, x6), x4)\, \frac{v(var6)}{h(x3, x4, x5, x6)} + f(x3, x4, x5, x6)\Big)\, V2\Big) : V34 := evalDG(LieDerivative(V3, V4)) :$

> $LieDerivative(V12, x1), LieDerivative(V12, x2), LieDerivative(V12, x5), LieDerivative(V12, x6), LieDerivative(V13, x1), LieDerivative(V13, x2), LieDerivative(V13, x5), LieDerivative(V13, x6), LieDerivative(V23, x1), LieDerivative(V23, x2), LieDerivative(V23, x5), LieDerivative(V23, x6), LieDerivative(V14, x1), LieDerivative(V14, x2), LieDerivative(V14, x5), LieDerivative(V14, x6), LieDerivative(V24, x1), LieDerivative(V24, x2), LieDerivative(V24, x5), LieDerivative(V24, x6), LieDerivative(V34, x1), LieDerivative(V34, x2), LieDerivative(V34, x5), LieDerivative(V34, x6)$

$$0, 0, 0, 0, 0, 0, 0, 0, 0, 0, 0, 0, 0, 0, 0, 0, 0, 0, 0, 0, 0, 0, 0, 0 \qquad \textbf{(100)}$$

> $tmp1 := DGinfo(V12, \text{"CoefficientSet"}) : tmp2 := DGinfo(V13, \text{"CoefficientSet"}) : tmp3 := DGinfo(V23, \text{"CoefficientSet"}) : tmp4 := DGinfo(V14, \text{"CoefficientSet"}) : tmp5 := DGinfo(V24, \text{"CoefficientSet"}) : tmp6 := DGinfo(V34, \text{"CoefficientSet"}) :$
$tmp := tmp1 \textbf{ union } tmp2 \textbf{ union } tmp3 \textbf{ union } tmp4 \textbf{ union } tmp5 \textbf{ union } tmp6 :$

> $tmp := factor(ToJet(map(coeffs, expand(numer(tmp)), \{q\}), \{u(var6), v(var6), w(var6), z3(x3, x4, x5, x6), z4(x3, x4, x5, x6), m(var6), n(var6), h(x3, x4, x5, x6), f(x3, x4, x5, x6)\})) :$

> $tmp[1..13]$

$$\{h^2\,(h\,z4 + h_{x3}),\, h^3\,(h\,z3_{x3} - z4_{x4}),\, -h\,(h\,z3\,v_{x1} + h\,m_{x1} + h\,w_{x1} + h_{x3}\,u_{x1} + v_{x4,x1}), -h\,(h\,z3\,v_{x2} + h\,m_{x2} + h\,w_{x2} + h_{x3}\,u_{x2} + v_{x4,x2}),\, -h\,(h^3\,u\,z3\,z4_{x3} - h^3\,u\,z4\,z3_{x3} + f\,h^3\,z3 - h^3\,n\,z3_{x3} - h^3\,u\,z3_{x3,x3} + 2\,h^3\,w\,z3_{x3} + h^3\,z3\,w_{x3} - h^3\,u_{x3}\,z3_{x3} + h^2\,v\,z3\,z4_{x4} - h^2\,v\,z4\,z3_{x4} + h^3\,z3_{x6} - h^3\,z4_{x5} + h^2\,m\,z4_{x4} + h^2\,u\,z4_{x3,x4} - h^2\,v\,z3_{x3,x4} - 2\,h^2\,w\,z4_{x4} - h^2\,z4\,w_{x4} - h\,v\,h_{x3}\,z3_{x4} + h^2\,f_{x4} + h\,v\,z4_{x4,x4} - h\,h_{x3}\,w_{x4} + h\,v_{x4}\,z4_{x4} - v\,h_{x4}\,z4_{x4}),\, -h^2\,(z4\,u_{x1} + n_{x1} + u_{x3,x1} + w_{x1}),\, -h^2\,(z4\,u_{x2} + n_{x2} + u_{x3,x2} + w_{x2}),\, -h^2\,(h^2\,u\,z3_{x3} - 2\,h^2\,w\,z3 + h\,v\,z3_{x4} - h\,n_{x4} - h\,u_{x3,x4} - h\,w_{x4} + h_{x3}\,u_{x4}),\, -h^4\,z3,\, -h^2\,v_{x1}\,(h\,z4 + h_{x3}),\, -h^2\,v_{x2}\,(h\,z4 + h_{x3}),\, -z3\,h^3\,u_{x1},\, -u_{x2}\,z3\,h^3\} \qquad \textbf{(101)}$$

> # $tmp[14..32]$

From this we conclude $z3$=0,
$z4 = -\frac{h_{x3}}{h}$, $z4_{x4} = 0$, $n = -u_3 - \frac{h_{x3}}{h}\,u - w + r$, $m = -\frac{v_4}{h} - \frac{h_{x3}}{h}\,u - w + s$, where $r$,$s$ are independent of $x1$,$x2$, and hence we restart:

> $V1 := evalDG\Big(q\,D\_x1 - diff(u(var6), x1)\,D\_x3 - \frac{diff(v(var6), x1)}{h(x3, x4, x5, x6)}\,D\_x4 + diff(w(var6), x1)\,q\,D\_q\Big) :$

$$V2 := evalDG\left(q\, D\_x2 - diff(u(var6), x2)\, D\_x3 - \frac{diff(v(var6), x2)}{h(x3, x4, x5, x6)}\, D\_x4 + diff(w(var6), x2)\, q\, D\_q\right) :$$

$$V3 := evalDG\left(D\_x5 + \frac{diff(u(var6), x4)}{h(x3, x4, x5, x6)}\, D\_x3 + \left(\frac{diff(v(var6), x4) + diff(h(x3, x4, x5, x6), x3)\, u(var6)}{h(x3, x4, x5, x6)^2} + \frac{w(var6) - q}{h(x3, x4, x5, x6)} + s(x3, x4, x5, x6)\right) D\_x4 - \frac{diff(w(var6), x4)}{h(x3, x4, x5, x6)}\, q\, D\_q\right) :$$

$$V4 := evalDG\Bigg(D\_x6 + \left(diff(u(var6), x3) + \frac{diff(h(x3, x4, x5, x6), x3)}{h(x3, x4, x5, x6)}\, u(var6) + w(var6) - q + r(x3, x4, x5, x6)\right) D\_x3 + \left(\frac{diff(v(var6), x3)}{h(x3, x4, x5, x6)} - \frac{2\, diff(h(x3, x4, x5, x6), x3)}{h(x3, x4, x5, x6)^2}\, v(var6)\right) D\_x4 + q\Bigg(-\frac{diff(h(x3, x4, x5, x6), x3)}{h(x3, x4, x5, x6)}\, q - diff(w(var6), x3) + 2\, \frac{diff(h(x3, x4, x5, x6), x3)}{h(x3, x4, x5, x6)}\, w(var6) - diff\left(\frac{diff(h(x3, x4, x5, x6), x3)}{h(x3, x4, x5, x6)}, x3\right) u(var6) - diff\left(\frac{diff(h(x3, x4, x5, x6), x3)}{h(x3, x4, x5, x6)}, x4\right) \frac{v(var6)}{h(x3, x4, x5, x6)} + f(x3, x4, x5, x6)\Bigg) D\_q\Bigg) :$$

> $$V12 := evalDG\left(LieDerivative(V1, V2) + \frac{diff(w(var6), x2)\, q}{q}\, V1 - \frac{diff(w(var6), x1)\, q}{q}\, V2\right) : V13 := evalDG\left(LieDerivative(V1, V3) - \frac{diff(w(var6), x4)}{h(x3, x4, x5, x6)}\, V1\right) : V23 := evalDG\left(LieDerivative(V2, V3) - \frac{diff(w(var6), x4)}{h(x3, x4, x5, x6)}\, V2\right) : V14 := evalDG\Bigg(LieDerivative(V1, V4) + \Bigg(-\frac{diff(h(x3, x4, x5, x6), x3)}{h(x3, x4, x5, x6)}\, q - diff(w(var6), x3) + 2\, \frac{diff(h(x3, x4, x5, x6), x3)}{h(x3, x4, x5, x6)}\, w(var6) - diff\left(\frac{diff(h(x3, x4, x5, x6), x3)}{h(x3, x4, x5, x6)}, x3\right) u(var6) - diff\left(\frac{diff(h(x3, x4, x5, x6), x3)}{h(x3, x4, x5, x6)}, x4\right) \frac{v(var6)}{h(x3, x4, x5, x6)} + f(x3, x4, x5, x6)\Bigg) V1\Bigg) :$$
$$V24 := evalDG\Bigg(LieDerivative(V2, V4) + \Bigg(-\frac{diff(h(x3, x4, x5, x6), x3)}{h(x3, x4, x5, x6)}\, q - diff(w(var6), x3) + 2\, \frac{diff(h(x3, x4, x5, x6), x3)}{h(x3, x4, x5, x6)}\, w(var6) - diff\left(\frac{diff(h(x3, x4, x5, x6), x3)}{h(x3, x4, x5, x6)}, x3\right) u(var6) - diff\left(\frac{diff(h(x3, x4, x5, x6), x3)}{h(x3, x4, x5, x6)}, x4\right) \frac{v(var6)}{h(x3, x4, x5, x6)} + f(x3, x4, x5, x6)\Bigg) V2\Bigg) : V34 := evalDG(LieDerivative(V3,$$

V4)):

> LieDerivative(V12, x1), LieDerivative(V12, x2), LieDerivative(V12, x5), LieDerivative(V12, x6), LieDerivative(V13, x1), LieDerivative(V13, x2), LieDerivative(V13, x5), LieDerivative(V13, x6), LieDerivative(V23, x1), LieDerivative(V23, x2), LieDerivative(V23, x5), LieDerivative(V23, x6), LieDerivative(V14, x1), LieDerivative(V14, x2), LieDerivative(V14, x5), LieDerivative(V14, x6), LieDerivative(V24, x1), LieDerivative(V24, x2), LieDerivative(V24, x5), LieDerivative(V24, x6), LieDerivative(V34, x1), LieDerivative(V34, x2), LieDerivative(V34, x5), LieDerivative(V34, x6)

$$0, 0, 0, 0, 0, 0, 0, 0, 0, 0, 0, 0, 0, 0, 0, 0, 0, 0, 0, 0, 0, 0, 0, 0 \quad \textbf{(102)}$$

> tmp1 := DGinfo(V12, "CoefficientSet") : tmp2 := DGinfo(V13, "CoefficientSet") : tmp3 := DGinfo(V23, "CoefficientSet") : tmp4 := DGinfo(V14, "CoefficientSet") : tmp5 := DGinfo(V24, "CoefficientSet") : tmp6 := DGinfo(V34, "CoefficientSet") :
tmp := tmp1 **union** tmp2 **union** tmp3 **union** tmp4 **union** tmp5 **union** tmp6 :

> tmp := factor(ToJet(map(coeffs, expand(numer(tmp)), {q}), {u(var6), v(var6), w(var6), r(x3, x4, x5, x6), s(x3, x4, x5, x6), h(x3, x4, x5, x6), f(x3, x4, x5, x6)})) :

> solve$\left(h\, h_{x3, x4} - h_{x3}\, h_{x4}, \{h_{x3, x4}\}\right)$ ;
\# pdsolve(h(x3, x4) diff(h(x3, x4), x3, x4) = diff(h(x3, x4), x3) diff(h(x3, x4), x4))

$$\left\{h_{x3, x4} = \frac{h_{x3}\, h_{x4}}{h}\right\} \quad \textbf{(103)}$$

> simplify$\left(\mathit{eval}\left(\mathit{tmp}, \left\{h_{x3, x4} = \frac{h_{x3}\, h_{x4}}{h}\right\}\right)\right)[1 ..13]$

$$\Big\{0, h\Big(\Big(\big((w_{x3, x3} - f_{x3})\, u_{x1} + (f - w_{x3})\, w_{x1} + (-u_{x3} - r - w)\, w_{x3, x1} - w_{x6, x1}\big)\, h^4 + \Big(\big(-u\, w_{x3, x1} + 2\, w\, w_{x1} - 2\, u_{x1}\, w_{x3}\big)\, h_{x3} + \big(h_{x3, x3, x3}\, u + h_{x3, x3}\, (u_{x3} - 2\, w)\big)\, u_{x1} + \big(w_{x3, x4} - f_{x4}\big)\, v_{x1} - w_{x1}\, u\, h_{x3, x3} - v_{x3}\, w_{x4, x1}\Big)\, h^3 + \Big(\big((-u_{x3} + 2\, w)\, u_{x1} + w_{x1}\, u\big)\, h_{x3}^2 + \big(-3\, u\, h_{x3, x3}\, u_{x1} + 2\, v\, w_{x4, x1} - 2\, v_{x1}\, w_{x4}\big)\, h_{x3} + v\, h_{x3, x3, x4}\, u_{x1} + v_{x1}\, \big(u\, h_{x3, x3, x4} + h_{x3, x3}\, u_{x4}\big)\Big)\, h^2 + \Big(2\, h_{x3}^3\, u_{x1}\, u - v_{x1}\, h_{x3}^2\, u_{x4} - v\, u_{x1}\, h_{x3, x3}\, h_{x4} - v_{x1}\, \big(u\, h_{x4}\, h_{x3, x3} - v\, h_{x3, x4, x4}\big)\Big)\, h - v_{x1}\, h_{x3}\, v\, h_{x4, x4}\Big), h\Big(\Big(\big((w_{x3, x3} - f_{x3})\, u_{x2} + (f - w_{x3})\, w_{x2} + (-u_{x3} - r - w)\, w_{x3, x2} - w_{x6, x2}\big)\, h^4 + \Big(\big(-u\, w_{x3, x2} + 2\, w\, w_{x2} - 2\, u_{x2}\, w_{x3}\big)\, h_{x3} + \big(h_{x3, x3, x3}\, u + h_{x3, x3}\, (u_{x3} - 2\, w)\big)\, u_{x2} + \big(w_{x3, x4} - f_{x4}\big)\, v_{x2} - w_{x2}\, u\, h_{x3, x3} - v_{x3}\, w_{x4, x2}\Big)\, h^3 + \Big(\big((-u_{x3} + 2\, w)\, u_{x2} + w_{x2}\, u\big)\, h_{x3}^2 + \big(-3\, u\, h_{x3, x3}\, u_{x2} + 2\, v\, w_{x4, x2} - 2\, v_{x2}\, w_{x4}\big)\, h_{x3} + v\, h_{x3, x3, x4}\, u_{x2} + v_{x2}\, \big(u\, h_{x3, x3, x4} + h_{x3, x3}\, u_{x4}\big)\Big)\, h^2 + \Big(2\, h_{x3}^3\, u_{x2}\, u - v_{x2}\, h_{x3}^2\, u_{x4} - v\, u_{x2}\, h_{x3, x3}\, h_{x4} - v_{x2}\, \big(u\, h_{x4}\, h_{x3, x3} - v\, h_{x3, x4, x4}\big)\Big)\, h - h_{x3}\, v_{x2}\, h_{x4, x4}\, v\Big), \big(h^3\, s_{x3} + f\, h^2 + (-r\, h_{x3} - h_{x6})\, h - 2\, u\, h_{x3}^2\big)\, h^2, -h\Big(\Big(\big(f + u_{x3, x3} + r_{x3}\big)\, u_{x1} + (-u_{x3} - r - w)\, u_{x3, x1} - u_{x6, x1}\Big)\, h^2 + \Big(\big((u_{x3} + 2\, w)\, u_{x1} - u_{x3, x1}\, u\big)\, h_{x3} + \big(w_{x4} + u_{x3, x4} + r_{x4}\big)\, v_{x1} - v_{x3}\, u_{x4, x1}\Big)\, h + h_{x3}\, \big(2\, v\, u_{x4, x1} + u_{x4}\, v_{x1}\big)\Big), -h\Big(\Big(\big(f + u_{x3, x3} + r_{x3}\big)\, u_{x2} + (-u_{x3} - r - w)\, u_{x3, x2} - u_{x6, x2}\Big)\, h^2 + \Big(\big((u_{x3} + 2\, w)\, u_{x2} - u_{x3, x2}\, u\big)\, h_{x3} + \big(w_{x4} + u_{x3, x4} + r_{x4}\big)\, v_{x2} - v_{x3}\, u_{x4, x2}\Big)\, h + h_{x3}\, \big(2\, v\, u_{x4, x2} + u_{x4}\, v_{x2}\big)\Big), \quad \textbf{(104)}$$

$$-h\left(\left(\left(f-w_{x3}\right)v_{x1}+\left(-u_{x3}-r-w\right)v_{x3,x1}+v_{x3,x3}u_{x1}-v_{x6,x1}\right)h^2+\left(\left(\left(u_{x3}+r+3w\right)h_{x3}-h_{x3,x3}u+v_{x3,x4}+h_{x6}\right)v_{x1}+\left(-u\,v_{x3,x1}-3u_{x1}v_{x3}\right)h_{x3}-2h_{x3,x3}v\,u_{x1}-v_{x3}v_{x4,x1}\right)h-2\left(\left(-u\,h_{x3}+v_{x4}\right)v_{x1}-v\left(2h_{x3}u_{x1}+v_{x4,x1}\right)\right)h_{x3}\right), -h\left(\left(\left(f-w_{x3}\right)v_{x2}+\left(-u_{x3}-r-w\right)v_{x3,x2}+v_{x3,x3}u_{x2}-v_{x6,x2}\right)h^2+\left(\left(\left(u_{x3}+r+3w\right)h_{x3}-h_{x3,x3}u+v_{x3,x4}+h_{x6}\right)v_{x2}+\left(-u\,v_{x3,x2}-3u_{x2}v_{x3}\right)h_{x3}-2h_{x3,x3}v\,u_{x2}-v_{x3}v_{x4,x2}\right)h-2\left(\left(-u\,h_{x3}+v_{x4}\right)v_{x2}-v\left(2h_{x3}u_{x2}+v_{x4,x2}\right)\right)h_{x3}\right), -h\left(\left(\left(w_{x3,x4}-f_{x4}\right)s+w_{x3,x5}-f_{x5}\right)h^5+\left(\left(-2s\,w_{x4}-2w_{x5}\right)h_{x3}+\left(s\,h_{x3,x3,x4}+h_{x3,x3,x5}\right)u+\left(s\,h_{x3,x3}-f_{x3}+w_{x3,x3}\right)u_{x4}+h_{x3,x3}u_{x5}+\left(-2h_{x3,x5}-f_{x4}\right)w+\left(-u_{x3}-r\right)w_{x3,x4}-w_{x4,x6}\right)h^4+\left(\left(-s\,u_{x4}-u_{x5}\right)h_{x3}^2+\left(\left(-2h_{x3,x5}-f_{x4}\right)u-2u_{x4}w_{x3}+\left(2h_{x5}-w_{x4}\right)w+w_{x4}\left(u_{x3}+r\right)\right)h_{x3}+\left(h_{x3,x3,x3}u_{x4}+\left(-s\,h_{x4}-h_{x5}\right)h_{x3,x3}+h_{x3,x3,x4}w\right)u+h_{x3,x3}\left(u_{x3}-w\right)u_{x4}+\left(s\,h_{x3,x4,x4}+h_{x3,x4,x5}\right)v+\left(w_{x3,x4}-f_{x4}\right)v_{x4}+h_{x6}w_{x4}-w_{x4,x4}v_{x3}\right)h^3+\left(\left(\left(2h_{x5}-w_{x4}\right)u-u_{x4}\left(u_{x3}-w\right)\right)h_{x3}^2+\left(h_{x3,x3,x4}u^2-2u\,h_{x3,x3}u_{x4}+\left(-s\,h_{x4,x4}-h_{x4,x5}+2w_{x4,x4}\right)v-2v_{x4}w_{x4}\right)h_{x3}+\left(-w\,h_{x4}h_{x3,x3}+h_{x3,x3,x4}v_{x4}\right)u+\left(v\,h_{x3,x3,x4}+h_{x3,x3}v_{x4}\right)u_{x4}+\left(w\,h_{x3,x4,x4}-h_{x4}h_{x3,x5}\right)v+w_{x4}v_{x3}h_{x4}\right)h^2+\left(h_{x3}^3u\,u_{x4}-h_{x3}^2u_{x4}v_{x4}+\left(-h_{x4}h_{x3,x3}u^2+h_{x3,x4,x4}v\,u+v\left(-h_{x4,x4}w+h_{x4}\left(h_{x5}-2w_{x4}\right)\right)\right)h_{x3}-u\,h_{x4}h_{x3,x3}v_{x4}-v\left(h_{x4}h_{x3,x3}u_{x4}-h_{x3,x4,x4}v_{x4}\right)\right)h-h_{x3}h_{x4,x4}v\left(u\,h_{x3}+v_{x4}\right)\right), -h^2\left(h\,r_{x4}+2h_{x3}u_{x4}\right), -\left(\left(f_{x4}+h_{x3,x5}\right)h^3+\left(-u\,h_{x3,x3,x4}-h_{x3}h_{x5}\right)h^2+\left(u\,h_{x4}h_{x3,x3}-v\,h_{x3,x4,x4}\right)h+v\,h_{x3}h_{x4,x4}\right)h^2, 2h^2h_{x3}u_{x1}, 2h^2u_{x2}h_{x3}\Big\}$$

```
> simplify(eval(tmp, {h = 1, h_x3 = 0, h_x4 = 0, h_x5 = 0, h_x6 = 0, h_x3,x3 = 0, h_x3,x4 = 0, h_x4,x4 = 0, h_x3,x5
      = 0, h_x3,x6 = 0, h_x4,x5 = 0, h_x4,x6 = 0, h_x3,x3,x3 = 0, h_x3,x3,x4 = 0, h_x3,x4,x4 = 0, h_x4,x4,x4 = 0}))[1..4]
```

$$\left\{0, -f_{x4}, -r_{x4}, f+s_{x3}\right\} \tag{105}$$

Thus we get $h=h(x4)$ and a change of variables yields $h=1$. In addition we obtain that $f,r$ are functions of $(x3,x5,x6)$ and s is affine in $x4$. We update the Lax distribution and restart:

```
> V1 := evalDG(q D_x1 − diff(u(var6), x1) D_x3 − diff(v(var6), x1) D_x4 + diff(w(var6),
      x1) q D_q) :
  V2 := evalDG(q D_x2 − diff(u(var6), x2) D_x3 − diff(v(var6), x2) D_x4 + diff(w(var6),
      x2) q D_q) :
  V3 := evalDG(D_x5 + diff(u(var6), x4) D_x3 + (diff(v(var6), x4) + w(var6) − q + s(x4,
      x5, x6) − t(x3, x5, x6)) D_x4 − diff(w(var6), x4) q D_q) :
  V4 := evalDG(D_x6 + (diff(u(var6), x3) + w(var6) − q + r(x3, x5, x6)) D_x3
       + diff(v(var6), x3) D_x4 + q (−diff(w(var6), x3) + diff(t(x3, x5, x6), x3)) D_q) :
```

We can eliminate $t$ by modifing $w$, then we eliminate $r$ by modifing $u$ and eliminate $s$ by modifing $v$. Finally we get the required Lax distribution and hence the required ω and ϕ:

```
> V1 := evalDG(q D_x1 − diff(u(var6), x1) D_x3 − diff(v(var6), x1) D_x4 + diff(w(var6),
      x1) q D_q) :
  V2 := evalDG(q D_x2 − diff(u(var6), x2) D_x3 − diff(v(var6), x2) D_x4 + diff(w(var6),
      x2) q D_q) :
```

```
V3 := evalDG(D_x5 + diff(u(var6), x4) D_x3 + (diff(v(var6), x4) + w(var6) - q) D_x4
    - diff(w(var6), x4) q D_q) :
V4 := evalDG(D_x6 + (diff(u(var6), x3) + w(var6) - q) D_x3 + diff(v(var6), x3) D_x4
    - diff(w(var6), x3) q D_q) :
>
>
>
>
>
>
>
```
