# Supplementary material for: Involutive scroll structures on solutions of 4D dispersionless integrable hierarchies
Source: arXiv:2503.10897 ancillary file (2025-03-13)
Supplement: Supplementary file 2 [file EFBK25-Scroll-Suppl-2.pdf]

Computation of Lax distribution, verification of involutivity and characteristic property for dispersionless integrable hierarchies of EFBK-2025-Scroll paper

```
> 
> with(DifferentialGeometry) : with(Tensor) : with(JetCalculus) : with(GroupActions) :
    with(Tools) : with(PDETools) : with(LinearAlgebra) : Preferences("ShowFramePrompt",
    'false') :
> interface(warnlevel = 0) : interface(rtablesize = 50) :
```

# DFK equation hierarchy

```
> var := x, y, t1, t2, t3, t4 : varq := x, y, t1, t2, t3, t4, q : DGsetup([varq], M6p) :
> V1 := evalDG(D_t1 + (diff(v(var), x) - q) D_x + diff(u(var), x) D_y + diff(w(var),
    x) D_q) :
  V2 := evalDG(D_t2 + diff(v(var), y) D_x + (diff(u(var), y) - q) D_y + diff(w(var),
    y) D_q) :
> eq12 := ToJet(DGinfo(LieDerivative(V1, V2), "CoefficientSet"), {u(var), v(var),
    w(var)}, notation = jetnumbers)
```

$$eq12 := \{u_1\, w_{2,2} - u_2\, w_{1,2} + v_1\, w_{1,2} - v_2\, w_{1,1} - w_{1,4} + w_{2,3}, u_1\, u_{2,2} - u_2\, u_{1,2} - u_{1,1}\, v_2 + u_{1,2}\, v_1 - u_{1,4} + u_{2,3} - w_1, u_1\, v_{2,2} - u_2\, v_{1,2} + v_1\, v_{1,2} - v_2\, v_{1,1} - v_{1,4} + v_{2,3} + w_2\} \quad \textbf{(1.1)}$$

```
> V3 := evalDG(D_t3 + (diff(v(var), t1) - w(var)) D_x + diff(u(var), t1) D_y - q D_t1
    + diff(w(var), t1) D_q) :
  V4 := evalDG(D_t4 + diff(v(var), t2) D_x + (diff(u(var), t2) - w(var)) D_y - q D_t2
    + diff(w(var), t2) D_q) :
> V3a := evalDG(V3 + q V1) : V4a := evalDG(V4 + q V2) :
> eq13 := ToJet(DGinfo(LieDerivative(V1, V3a), "CoefficientSet"), {u(var), v(var),
    w(var)}, notation = jetnumbers);
  eq23 := map(coeffs, ToJet(DGinfo(LieDerivative(V2, V3a), "CoefficientSet"), {u(var),
    v(var), w(var)}, notation = jetnumbers), {q})
```

$$eq13 := \{u_1\, u_{2,3} + u_1\, w_1 - u_3\, u_{1,2} - u_{1,1}\, v_3 + u_{1,1}\, w[\,] + u_{1,3}\, v_1 - u_{1,5} + u_{3,3}, u_1\, v_{2,3} - u_1\, w_2 - u_3\, v_{1,2} + v_1\, v_{1,3} - v_3\, v_{1,1} + v_{1,1}\, w[\,] - v_{1,5} + v_{3,3}, u_1\, w_{2,3} - u_3\, w_{1,2} + v_1\, w_{1,3} - v_3\, w_{1,1} + w[\,]\, w_{1,1} + w_1^2 - w_{1,5} + w_{3,3}\}$$

$$eq23 := \{-u_1\, w_{2,2} + u_2\, w_{1,2} - v_1\, w_{1,2} + v_2\, w_{1,1} + w_{1,4} - w_{2,3}, -u_1\, u_{2,2} + u_2\, u_{1,2} + u_{1,1}\, v_2 - u_{1,2}\, v_1 + u_{1,4} - u_{2,3} + w_1, -u_1\, v_{2,2} + u_2\, v_{1,2} - v_1\, v_{1,2} + v_2\, v_{1,1} + v_{1,4} - v_{2,3} - w_2, u_2\, w_{2,3} - u_3\, w_{2,2} + v_2\, w_{1,3} - v_3\, w_{1,2} + w[\,]\, w_{1,2} + w_1\, w_2 - w_{2,5} + w_{3,4}, u_1\, w_2 + u_2\, u_{2,3} - u_3\, u_{2,2} - u_{1,2}\, v_3 + u_{1,2}\, w[\,] + u_{1,3}\, v_2 - u_{2,5} + u_{3,4} + w_3, u_2\, v_{2,3} - u_2\, w_2 - u_3\, v_{2,2} + v_1\, w_2 + v_2\, v_{1,3} - v_2\, w_1 - v_3\, v_{1,2} + v_{1,2}\, w[\,] - v_{2,5} + v_{3,4} - w_4\} \quad \textbf{(1.2)}$$

```
> nops(eq12), nops(eq13), nops(eq23)
```

$$3, 3, 6 \quad \textbf{(1.3)}$$

```
> eq14 := map(coeffs, ToJet(DGinfo(LieDerivative(V1, V4a), "CoefficientSet"), {u(var),
    v(var), w(var)}, notation = jetnumbers), {q});
  eq24 := ToJet(DGinfo(LieDerivative(V2, V4a), "CoefficientSet"), {u(var), v(var),
```

$w(var)\}, notation = jetnumbers)$

$$eq14 := \{u_1\, w_{2,2} - u_2\, w_{1,2} + v_1\, w_{1,2} - v_2\, w_{1,1} - w_{1,4} + w_{2,3}, u_1\, u_{2,2} - u_2\, u_{1,2} - u_{1,1}\, v_2 + u_{1,2}\, v_1 - u_{1,4} + u_{2,3} - w_1, u_1\, v_{2,2} - u_2\, v_{1,2} + v_1\, v_{1,2} - v_2\, v_{1,1} - v_{1,4} + v_{2,3} + w_2, u_1\, w_{2,4} - u_4\, w_{1,2} + v_1\, w_{1,4} - v_4\, w_{1,1} + w[\,]\, w_{1,2} + w_1\, w_2 - w_{1,6} + w_{3,4}, u_1\, v_{2,4} - u_4\, v_{1,2} + v_1\, v_{1,4} + v_2\, w_1 - v_4\, v_{1,1} + v_{1,2}\, w[\,] - v_{1,6} + v_{3,4} + w_4, u_1\, u_{2,4} - u_1\, w_2 + u_2\, w_1 - u_4\, u_{1,2} - u_{1,1}\, v_4 + u_{1,2}\, w[\,] + u_{1,4}\, v_1 - v_1\, w_1 - u_{1,6} + u_{3,4} - w_3\}$$

$$eq24 := \{u_2\, u_{2,4} - u_4\, u_{2,2} - u_{1,2}\, v_4 + u_{1,4}\, v_2 + u_{2,2}\, w[\,] - v_2\, w_1 - u_{2,6} + u_{4,4}, u_2\, v_{2,4} - u_4\, v_{2,2} + v_2\, v_{1,4} + v_2\, w_2 - v_4\, v_{1,2} + v_{2,2}\, w[\,] - v_{2,6} + v_{4,4}, u_2\, w_{2,4} - u_4\, w_{2,2} + v_2\, w_{1,4} - v_4\, w_{1,2} + w[\,]\, w_{2,2} + w_2^2 - w_{2,6} + w_{4,4}\} \quad (1.4)$$

> $eq34 := map(coeffs, expand(ToJet(DGinfo(LieDerivative(V3a, V4a), \text{"CoefficientSet"}), \{u(var), v(var), w(var)\}, notation = jetnumbers)), \{q\})$

$$eq34 := \{u_1\, w_{2,2} - u_2\, w_{1,2} + v_1\, w_{1,2} - v_2\, w_{1,1} - w_{1,4} + w_{2,3}, u_1\, u_{2,2} - u_2\, u_{1,2} - u_{1,1}\, v_2 + u_{1,2}\, v_1 - u_{1,4} + u_{2,3} - w_1, u_1\, v_{2,2} - u_2\, v_{1,2} + v_1\, v_{1,2} - v_2\, v_{1,1} - v_{1,4} + v_{2,3} + w_2, u_3\, w_{2,4} - u_4\, w_{2,3} + v_3\, w_{1,4} - v_4\, w_{1,3} - w[\,]\, w_{1,4} + w[\,]\, w_{2,3} - w_1\, w_4 + w_2\, w_3 - w_{3,6} + w_{4,5}, u_1\, w_{2,4} - u_2\, w_{2,3} + u_3\, w_{2,2} - u_4\, w_{1,2} + v_1\, w_{1,4} - v_2\, w_{1,3} + v_3\, w_{1,2} - v_4\, w_{1,1} - w_{1,6} + w_{2,5}, -u_1\, w_4 + u_2\, w_3 + u_3\, u_{2,4} - u_3\, w_2 - u_4\, u_{2,3} - u_{1,3}\, v_4 + u_{1,4}\, v_3 - u_{1,4}\, w[\,] + u_{2,3}\, w[\,] - v_3\, w_1 + w[\,]\, w_1 - u_{3,6} + u_{4,5} - w_5, u_3\, v_{2,4} - u_4\, v_{2,3} + u_4\, w_2 - v_1\, w_4 + v_2\, w_3 + v_3\, v_{1,4} - v_4\, v_{1,3} + v_4\, w_1 - v_{1,4}\, w[\,] + v_{2,3}\, w[\,] - w[\,]\, w_2 - v_{3,6} + v_{4,5} + w_6, u_1\, u_{2,4} - 2\, u_1\, w_2 - u_2\, u_{2,3} + u_2\, w_1 + u_3\, u_{2,2} - u_4\, u_{1,2} - u_{1,1}\, v_4 + u_{1,2}\, v_3 - u_{1,3}\, v_2 + u_{1,4}\, v_1 - v_1\, w_1 - u_{1,6} + u_{2,5} - 2\, w_3, u_1\, v_{2,4} - u_2\, v_{2,3} + u_2\, w_2 + u_3\, v_{2,2} - u_4\, v_{1,2} + v_1\, v_{1,4} - v_1\, w_2 - v_2\, v_{1,3} + 2\, v_2\, w_1 + v_3\, v_{1,2} - v_4\, v_{1,1} - v_{1,6} + v_{2,5} + 2\, w_4\} \quad (1.5)$$

> $nops(eq12), nops(eq13), nops(eq23), nops(eq14), nops(eq24), nops(eq34)$

$$3, 3, 6, 6, 3, 9 \quad (1.6)$$

> $slv123 := solve\big(eq12$ **union** $eq13$ **union** $eq23[4..6], \{u_{1,1}, u_{1,2}, u_{2,2}, v_{1,1}, v_{1,2}, v_{2,2}, w_{1,1}, w_{1,2}, w_{2,2}\}\big) : simplify(eval(eq12$ **union** $eq13$ **union** $eq23, slv123))$

$$\{0\} \quad (1.7)$$

> $slv1234 := solve\big(eq12$ **union** $eq13$ **union** $eq23[4..6]$ **union** $eq14[4..6]$ **union** $eq24$ **union** $eq34[4..4]$ **union** $eq34[6..7], \{u_{1,1}, u_{1,2}, u_{2,2}, u_{1,3}, u_{2,3}, u_{3,4}, v_{1,1}, v_{1,2}, v_{2,2}, v_{1,3}, v_{2,3}, v_{3,4}, w_{1,1}, w_{1,2}, w_{2,2}, w_{1,3}, w_{2,3}, w_{3,4}\}\big) : simplify(eval(eq12$ **union** $eq13$ **union** $eq23$ **union** $eq14$ **union** $eq24$ **union** $eq34, slv1234))$

$$\{0\} \quad (1.8)$$

> $eq12$ **union** $eq13$ **union** $eq23[4..6]$

$$\{u_1\, w_{2,2} - u_2\, w_{1,2} + v_1\, w_{1,2} - v_2\, w_{1,1} - w_{1,4} + w_{2,3}, u_1\, u_{2,2} - u_2\, u_{1,2} - u_{1,1}\, v_2 + u_{1,2}\, v_1 - u_{1,4} + u_{2,3} - w_1, u_1\, v_{2,2} - u_2\, v_{1,2} + v_1\, v_{1,2} - v_2\, v_{1,1} - v_{1,4} + v_{2,3} + w_2, u_1\, u_{2,3} + u_1\, w_1 - u_3\, u_{1,2} - u_{1,1}\, v_3 + u_{1,1}\, w[\,] + u_{1,3}\, v_1 - u_{1,5} + u_{3,3}, u_1\, v_{2,3} - u_1\, w_2 - u_3\, v_{1,2} \quad (1.9)$$

$+ v_1 v_{1,3} - v_3 v_{1,1} + v_{1,1} w[\,] - v_{1,5} + v_{3,3}, u_1 w_{2,3} - u_3 w_{1,2} + v_1 w_{1,3} - v_3 w_{1,1}$
$+ w[\,] w_{1,1} + w_1^2 - w_{1,5} + w_{3,3}, u_2 w_{2,3} - u_3 w_{2,2} + v_2 w_{1,3} - v_3 w_{1,2} + w[\,] w_{1,2}$
$+ w_1 w_2 - w_{2,5} + w_{3,4}, u_1 w_2 + u_2 u_{2,3} - u_3 u_{2,2} - u_{1,2} v_3 + u_{1,2} w[\,] + u_{1,3} v_2 - u_{2,5}$
$+ u_{3,4} + w_3, u_2 v_{2,3} - u_2 w_2 - u_3 v_{2,2} + v_1 w_2 + v_2 v_{1,3} - v_2 w_1 - v_3 v_{1,2} + v_{1,2} w[\,]$
$- v_{2,5} + v_{3,4} - w_4\}$

> *eq14*[4..6] **union** *eq24* **union** *eq34*[4..4] **union** *eq34*[6..7]

$\{u_2 u_{2,4} - u_4 u_{2,2} - u_{1,2} v_4 + u_{1,4} v_2 + u_{2,2} w[\,] - v_2 w_1 - u_{2,6} + u_{4,4}, u_2 v_{2,4} - u_4 v_{2,2}$ **(1.10)**
$+ v_2 v_{1,4} + v_2 w_2 - v_4 v_{1,2} + v_{2,2} w[\,] - v_{2,6} + v_{4,4}, u_2 w_{2,4} - u_4 w_{2,2} + v_2 w_{1,4}$
$- v_4 w_{1,2} + w[\,] w_{2,2} + w_2^2 - w_{2,6} + w_{4,4}, u_1 w_{2,4} - u_4 w_{1,2} + v_1 w_{1,4} - v_4 w_{1,1}$
$+ w[\,] w_{1,2} + w_1 w_2 - w_{1,6} + w_{3,4}, u_1 v_{2,4} - u_4 v_{1,2} + v_1 v_{1,4} + v_2 w_1 - v_4 v_{1,1}$
$+ v_{1,2} w[\,] - v_{1,6} + v_{3,4} + w_4, u_3 w_{2,4} - u_4 w_{2,3} + v_3 w_{1,4} - v_4 w_{1,3} - w[\,] w_{1,4}$
$+ w[\,] w_{2,3} - w_1 w_4 + w_2 w_3 - w_{3,6} + w_{4,5}, u_1 u_{2,4} - u_1 w_2 + u_2 w_1 - u_4 u_{1,2} - u_{1,1} v_4$
$+ u_{1,2} w[\,] + u_{1,4} v_1 - v_1 w_1 - u_{1,6} + u_{3,4} - w_3, -u_1 w_4 + u_2 w_3 + u_3 u_{2,4} - u_3 w_2$
$- u_4 u_{2,3} - u_{1,3} v_4 + u_{1,4} v_3 - u_{1,4} w[\,] + u_{2,3} w[\,] - v_3 w_1 + w[\,] w_1 - u_{3,6} + u_{4,5}$
$- w_5, u_3 v_{2,4} - u_4 v_{2,3} + u_4 w_2 - v_1 w_4 + v_2 w_3 + v_3 v_{1,4} - v_4 v_{1,3} + v_4 w_1 - v_{1,4} w[\,]$
$+ v_{2,3} w[\,] - w[\,] w_2 - v_{3,6} + v_{4,5} + w_6\}$

> $nops(\{u_{1,1}, u_{1,2}, u_{2,2}, u_{1,3}, u_{2,3}, u_{3,4}, v_{1,1}, v_{1,2}, v_{2,2}, v_{1,3}, v_{2,3}, v_{3,4}, w_{1,1}, w_{1,2}, w_{2,2}, w_{1,3}, w_{2,3}, w_{3,4}\})$

18 **(1.11)**

> # *Ss* :={ } :**for** *i* **to** *nops*(*slv1234*) **do if** *lhs*(*slv1234*[*i*]) = *rhs*(*slv1234*[*i*]) **then** *Ss* := *Ss* **union** {*lhs*(*slv1234*[*i*])} :**fi**:**od**: *nops*(*Ss*)

## computing Char

> $smu := f \to add\left(add\left(diff\left(f, u_{i,j}\right) p_i p_j, j = i..6\right), i = 1..6\right) : smv := f \to add\left(add\left(diff\left(f, v_{i,j}\right) p_i p_j, j = i..6\right), i = 1..6\right) : smw := f \to add\left(add\left(diff\left(f, w_{i,j}\right) p_i p_j, j = i..6\right), i = 1..6\right) :$

> *sys* := *eq12* : *Ma* := *Matrix*([*seq*([*smu*(*sys*[*i*]), *smv*(*sys*[*i*]), *smw*(*sys*[*i*])], *i* **in** [1, 2, 3])]) : *Ma*

$$\left[\begin{array}{cc} 0 & \cdots \\ -v_2 p_1^2 + \left(-u_2 + v_1\right) p_1 p_2 - p_1 p_4 + u_1 p_2^2 + p_2 p_3 & \cdots \\ 0 & -v_2 \cdots \end{array}\right]$$ **(1.1.1)**

> *sys* := *eq13* : *Ma* := *Matrix*([*seq*([*smu*(*sys*[*i*]), *smv*(*sys*[*i*]), *smw*(*sys*[*i*])], *i* **in** [1, 2, 3])]) : *Ma*

$$\begin{bmatrix} \left(-v_3 + w[\,]\right) p_1^2 - u_3 p_1 p_2 + v_1 p_1 p_3 - p_1 p_5 + u_1 p_2 p_3 + p_3^2 & \cdots \\ 0 & \cdots \\ 0 & \cdots \end{bmatrix} \quad \textbf{(1.1.2)}$$

> *sys* := *eq23*[4 ..6] : *Ma* := *Matrix*([*seq*([*smu*(*sys*[*i*]), *smv*(*sys*[*i*]), *smw*(*sys*[*i*])], *i* **in**[1, 2, 3])]) : *Ma*

$$\begin{bmatrix} 0 & \cdots \\ \left(-v_3 + w[\,]\right) p_1 p_2 + v_2 p_1 p_3 - u_3 p_2^2 + u_2 p_2 p_3 - p_2 p_5 + p_3 p_4 & \cdots \\ 0 & \cdots \end{bmatrix} \quad \textbf{(1.1.3)}$$

> *sys* := *eq12* **union** *eq13* **union** *eq23*[4 ..6] :
> *Ma* := *Matrix*([*seq*([*smu*(*sys*[*i*]), *smv*(*sys*[*i*]), *smw*(*sys*[*i*])], *i* **in**[2, 4, 8, 3, 5, 9, 1, 6, 7])]) :

> *Ma*[1 ..9, 1 ..1], *Ma*[1 ..9, 2 ..2]; *Ma*[1 ..9, 3 ..3]

$$\begin{bmatrix} -v_2 p_1^2 + \left(-u_2 + v_1\right) p_1 p_2 - p_1 p_4 + u_1 p_2^2 + p_2 p_3 \\ \left(-v_3 + w[\,]\right) p_1^2 - u_3 p_1 p_2 + v_1 p_1 p_3 - p_1 p_5 + u_1 p_2 p_3 + p_3^2 \\ \left(-v_3 + w[\,]\right) p_1 p_2 + v_2 p_1 p_3 - u_3 p_2^2 + u_2 p_2 p_3 - p_2 p_5 + p_3 p_4 \\ 0 \\ 0 \\ 0 \\ 0 \\ 0 \\ 0 \end{bmatrix},$$

$$\begin{bmatrix} 0 \\ 0 \\ 0 \\ -v_2 p_1^2 + (-u_2 + v_1) p_1 p_2 - p_1 p_4 + u_1 p_2^2 + p_2 p_3 \\ (-v_3 + w[\,]) p_1^2 - u_3 p_1 p_2 + v_1 p_1 p_3 - p_1 p_5 + u_1 p_2 p_3 + p_3^2 \\ (-v_3 + w[\,]) p_1 p_2 + v_2 p_1 p_3 - u_3 p_2^2 + u_2 p_2 p_3 - p_2 p_5 + p_3 p_4 \\ 0 \\ 0 \\ 0 \end{bmatrix}$$

$$\begin{bmatrix} 0 \\ 0 \\ 0 \\ 0 \\ 0 \\ 0 \\ -v_2 p_1^2 + (-u_2 + v_1) p_1 p_2 - p_1 p_4 + u_1 p_2^2 + p_2 p_3 \\ (-v_3 + w[\,]) p_1^2 - u_3 p_1 p_2 + v_1 p_1 p_3 - p_1 p_5 + u_1 p_2 p_3 + p_3^2 \\ (-v_3 + w[\,]) p_1 p_2 + v_2 p_1 p_3 - u_3 p_2^2 + u_2 p_2 p_3 - p_2 p_5 + p_3 p_4 \end{bmatrix} \quad \textbf{(1.1.4)}$$

> $slabc1 := solve\Big(\Big\{coeffs\Big(expand\Big(add\Big(add\big((a\,||\,i\,||\,j)p_j, j=1..5\big)\cdot Ma[i,1], i=1..3\Big)\Big), \{seq(p_i, i=1..5)\}\Big)\Big\}, \{seq(seq(a\,||\,i\,||\,j, j=1..5), i=1..3)\}\Big)$ : $Ss1 := \{\,\}$ :**for** $i$ **to** $nops(slabc1)$ **do if** $lhs(slabc1[i]) = rhs(slabc1[i])$ **then** $Ss1 := Ss1$ **union** $\{lhs(slabc1[i])\}$ :**fi**:**od**: $Ss1, nops(Ss1)$

$$\{a31, a33\}, 2 \quad \textbf{(1.1.5)}$$

> $slabc2 := solve\Big(\Big\{coeffs\Big(expand\Big(add\Big(add\big(add\big((a\,||\,i\,||\,j1\,||\,j2)p_{j1}p_{j2}, j2=j1..5\big), j1=1..5\big)\cdot Ma[i,1], i=1..3\Big)\Big), \{seq(p_i, i=1..5)\}\Big)\Big\}, \{seq(seq(seq(a\,||\,i\,||\,j1\,||\,j2, j2=j1..5), j1=1..5), i=1..3)\}\Big)$ : $Ss2 := \{\,\}$ :**for** $i$ **to** $nops(slabc2)$ **do if** $lhs(slabc2[i]) = rhs(slabc2[i])$ **then** $Ss2 := Ss2$ **union** $\{lhs(slabc2[i])\}$ :**fi**:**od**: $nops(Ss2)$

$$10 \quad \textbf{(1.1.6)}$$

> $slabc3 := solve\Big(\Big\{coeffs\Big(expand\Big(add\Big(add\Big(add\Big(add\big((a\,||\,i\,||\,j1\,||\,j2\,||\,j3)p_{j1}p_{j2}p_{j3}, j3=j2$

$..5), j2 = j1..5), j1 = 1..5) \cdot Ma[i, 1], i = 1..3)), \{seq(p_i, i = 1..5)\})\},$
$\{seq(seq(seq(seq(a \| i \| j1 \| j2 \| j3, j3 = j2..5), j2 = j1..5), j1 = 1..5), i = 1..3)\})$ :
$Ss3 := \{\}$ **:for** $i$ **to** $nops(slabc3)$ **do if** $lhs(slabc3[i]) = rhs(slabc3[i])$ **then** $Ss3 :=$
$Ss3$ **union** $\{lhs(slabc3[i])\}$ **:fi:od:** $nops(Ss3)$

$$30 \qquad \textbf{(1.1.7)}$$

\> $slabc4 := solve(\{coeffs(expand(add(add(add(add(add((a \| i \| j1 \| j2 \| j3$
$\| j4) p_{j1} p_{j2} p_{j3} p_{j4}, j4 = j3..5), j3 = j2..5), j2 = j1..5), j1 = 1..5) \cdot Ma[i, 1], i = 1..3)),$
$\{seq(p_i, i = 1..5)\})\}, \{seq(seq(seq(seq(seq(a \| i \| j1 \| j2 \| j3 \| j4, j4 = j3..5), j3 = j2$
$..5), j2 = j1..5), j1 = 1..5), i = 1..3)\})$ : $Ss4 := \{\}$ **:for** $i$ **to** $nops(slabc4)$ **do**
**if** $lhs(slabc4[i]) = rhs(slabc4[i])$ **then** $Ss4 := Ss4$ **union** $\{lhs(slabc4[i])\}$ **:fi:od:**
$nops(Ss4)$

$$70 \qquad \textbf{(1.1.8)}$$

\> $syz1 := eval(eval(eval([seq(add((a \| i \| j) p_j, j = 1..5), i = 1..3)], slabc1), \{a31 = 1,$
$a33 = 0\}), \{seq(seq(a \| i \| j = 0, j = 1..5), i = 1..3)\})$;
$syz2 := eval(eval(eval([seq(add((a \| i \| j) p_j, j = 1..5), i = 1..3)], slabc1), \{a31 = 0,$
$a33 = 1\}), \{seq(seq(a \| i \| j = 0, j = 1..5), i = 1..3)\})$

$$syz1 := [p_3, -p_2, p_1]$$

$$syz2 := [(v_3 - w[\,])\, p_1 + u_3 p_2 - v_1 p_3 + p_5, -v_2 p_1 + (-u_2 + v_1)\, p_2 - p_4, p_2 u_1 + p_3] \qquad \textbf{(1.1.9)}$$

\> $simplify([add(syz1[i]\, Ma[i, 1], i = 1..3), add(syz2[i]\, Ma[i, 1], i = 1..3)])$

$$[0, 0] \qquad \textbf{(1.1.10)}$$

\> $solve(eval(Ma[1, 1], \{p_1 = 1\}), \{p_4\})$

$$\{p_4 = u_1 p_2^2 + p_2 p_3 - p_2 u_2 + p_2 v_1 - v_2\} \qquad \textbf{(1.1.11)}$$

\> $solve(eval(Ma[2, 1], \{p_1 = 1, p_4 = u_1 p_2^2 + p_2 p_3 - p_2 u_2 + p_2 v_1 - v_2\}), \{p_5\})$

$$\{p_5 = u_1 p_2 p_3 - u_3 p_2 + p_3^2 + v_1 p_3 - v_3 + w[\,]\} \qquad \textbf{(1.1.12)}$$

\> $simplify(eval(Ma[3, 1], \{p_1 = 1, p_4 = u_1 p_2^2 + p_2 p_3 - p_2 u_2 + p_2 v_1 - v_2, p_5 = u_1 p_2 p_3$
$- u_3 p_2 + p_3^2 + v_1 p_3 - v_3 + w[\,]\}))$

$$0 \qquad \textbf{(1.1.13)}$$

\> $[1, \chi, \lambda, u_1 \chi^2 + \chi \lambda - \chi u_2 + \chi v_1 - v_2, u_1 \chi \lambda - u_3 \chi + \lambda^2 + v_1 \lambda - v_3 + w[\,]]$

$$[1, \chi, \lambda, u_1 \chi^2 + \chi \lambda - \chi u_2 + \chi v_1 - v_2, u_1 \chi \lambda - u_3 \chi + \lambda^2 + v_1 \lambda - v_3 + w[\,]] \qquad \textbf{(1.1.14)}$$

\> $simplify(eval([1, \chi, \lambda, u_1 \chi^2 + \chi \lambda - \chi u_2 + \chi v_1 - v_2, u_1 \chi \lambda - u_3 \chi + \lambda^2 + v_1 \lambda - v_3$
$+ w[\,]], \{\chi = \chi, \lambda = \lambda - u_1 \chi - v_1\}))$

$$[1, \chi, -u_1 \chi + \lambda - v_1, (\lambda - u_2)\, \chi - v_2, \lambda^2 + (-u_1 \chi - v_1)\, \lambda - u_3 \chi + w[\,] - v_3] \qquad \textbf{(1.1.15)}$$

\> $[1, 0, \lambda - v_1, -v_2, \lambda^2 - v_1 \lambda + w[\,] - v_3] + \chi \cdot [0, 1, -u_1, \lambda - u_2, -u_1 \lambda - u_3]$

\>

\> $\# solve(\{Ma[1, 1], Ma[2, 1], Ma[3, 1]\})$

```
>
> sys := eq12 union eq13 union eq23[4 ..6] union eq14[4 ..6] union eq24 union eq34[4
    ..4] union eq34[6 ..7] : nops(sys)
```

$$18 \qquad \textbf{(1.1.16)}$$

```
> Ma := Matrix([seq([smu(sys[i]), smv(sys[i]), smw(sys[i])], i in [2, 4, 7, 12, 15, 17, 3,
    5, 8, 16, 13, 18, 1, 6, 9, 11, 10, 14])]) :
> Ma[1 ..6, 1 ..1], Ma[1 ..6, 2 ..2], Ma[1 ..6, 3 ..3]; Ma[7 ..12, 1 ..1], Ma[7 ..12, 2 ..2], Ma[7
    ..12, 3 ..3]; Ma[13 ..18, 1 ..1], Ma[13 ..18, 2 ..2], Ma[13 ..18, 3 ..3]
```

$$\begin{bmatrix} 1 & -v_2 p_1^2 + (-u_2 + v_1) p_1 p_2 - p_1 p_4 + u_1 p_2^2 + p_2 \cdots \\ 2 & (-v_3 + w[\ ]) p_1^2 - u_3 p_1 p_2 + v_1 p_1 p_3 - p_1 p_5 + u_1 p_2 \cdots \\ 3 & -v_4 p_1 p_2 + v_2 p_1 p_4 + (-u_4 + w[\ ]) p_2^2 + u_2 p_2 p_4 - p_2 \cdots \\ 4 & (-v_3 + w[\ ]) p_1 p_2 + v_2 p_1 p_3 - u_3 p_2^2 + u_2 p_2 p_3 - p_2 p_5 \cdots \\ 5 & -v_4 p_1^2 + (-u_4 + w[\ ]) p_1 p_2 + v_1 p_1 p_4 - p_1 p_6 + u_1 p_2 \cdots \\ 6 & -v_4 p_1 p_3 + (v_3 - w[\ ]) p_1 p_4 + (-u_4 + w[\ ]) p_2 p_3 + u_3 p_2 p_4 \cdots \end{bmatrix},$$

$$\begin{bmatrix} 0 \\ 0 \\ 0 \\ 0 \\ 0 \\ 0 \end{bmatrix}, \begin{bmatrix} 0 \\ 0 \\ 0 \\ 0 \\ 0 \\ 0 \end{bmatrix}$$

$$\begin{bmatrix} 0 \\ 0 \\ 0 \\ 0 \\ 0 \\ 0 \end{bmatrix},$$

$$
\left[\begin{array}{r}
-v_2\,p_1^2+\left(-u_2+v_1\right)p_1\,p_2-p_1\,p_4+u_1\,p_2^2+p_2\,p_3\cdots\\
\left(-v_3+w[\,]\right)p_1^2-u_3\,p_1\,p_2+v_1\,p_1\,p_3-p_1\,p_5+u_1\,p_2\,p_3\cdots\\
-v_4\,p_1\,p_2+v_2\,p_1\,p_4+\left(-u_4+w[\,]\right)p_2^2+u_2\,p_2\,p_4-p_2\,[illegible]\cdots\\
\left(-v_3+w[\,]\right)p_1\,p_2+v_2\,p_1\,p_3-u_3\,p_2^2+u_2\,p_2\,p_3-p_2\,p_5-\cdots\\
-v_4\,p_1^2+\left(-u_4+w[\,]\right)p_1\,p_2+v_1\,p_1\,p_4-p_1\,p_6+u_1\,p_2\,p_4\cdots\\
-v_4\,p_1\,p_3+\left(v_3-w[\,]\right)p_1\,p_4+\left(-u_4+w[\,]\right)p_2\,p_3+u_3\,p_2\,p_4-\cdots
\end{array}\right],
\left[\begin{array}{c}0\\0\\0\\0\\0\\0\end{array}\right]
$$

$$
\left[\begin{array}{c}0\\0\\0\\0\\0\\0\end{array}\right],
\left[\begin{array}{c}0\\0\\0\\0\\0\\0\end{array}\right],
\qquad \textbf{(1.1.17)}
$$

$$
\left[\begin{array}{r}
-v_2\,p_1^2+\left(-u_2+v_1\right)p_1\,p_2-p_1\,p_4+u_1\,p_2^2+p_2\,p_3\cdots\\
\left(-v_3+w[\,]\right)p_1^2-u_3\,p_1\,p_2+v_1\,p_1\,p_3-p_1\,p_5+u_1\,p_2\,p_3\cdots\\
-v_4\,p_1\,p_2+v_2\,p_1\,p_4+\left(-u_4+w[\,]\right)p_2^2+u_2\,p_2\,p_4-p_2\,[illegible]\cdots\\
\left(-v_3+w[\,]\right)p_1\,p_2+v_2\,p_1\,p_3-u_3\,p_2^2+u_2\,p_2\,p_3-p_2\,p_5-\cdots\\
-v_4\,p_1^2+\left(-u_4+w[\,]\right)p_1\,p_2+v_1\,p_1\,p_4-p_1\,p_6+u_1\,p_2\,p_4\cdots\\
-v_4\,p_1\,p_3+\left(v_3-w[\,]\right)p_1\,p_4+\left(-u_4+w[\,]\right)p_2\,p_3+u_3\,p_2\,p_4-\cdots
\end{array}\right]
$$

```
> slabc1 := solve({coeffs(expand(add(add((a||i||j)p_j, j = 1..5)·Ma[i, 1], i = 1..6)),
    {seq(p_i, i = 1..5)})}, {seq(seq(a||i||j, j = 1..5), i = 1..6)}) : Ss1 := { } :for i
    to nops(slabc1) do if lhs(slabc1[i]) = rhs(slabc1[i]) then Ss1 := Ss1
    union {lhs(slabc1[i])} :fi:od: Ss1, nops(Ss1)
```

$$\{a41, a43, a52, a61, a62\}, 5 \tag{1.1.18}$$

```
> slabc2 := solve({coeffs(expand(add(add(add((a||i||j1||j2)p_j1 p_j2, j2 = j1..5), j1 = 1
    ..5)·Ma[i, 1], i = 1..6)), {seq(p_i, i = 1..5)})}, {seq(seq(seq(a||i||j1||j2, j2 = j1
    ..5), j1 = 1..5), i = 1..6)}) : Ss2 := { } :for i to nops(slabc2) do if lhs(slabc2[i])
    = rhs(slabc2[i]) then Ss2 := Ss2 union {lhs(slabc2[i])} :fi:od: nops(Ss2)
```

$$24 \tag{1.1.19}$$

```
> slabc3 := solve({coeffs(expand(add(add(add(add((a||i||j1||j2||j3)p_j1 p_j2 p_j3, j3 = j2
    ..5), j2 = j1..5), j1 = 1..5)·Ma[i, 1], i = 1..6)), {seq(p_i, i = 1..5)})},
    {seq(seq(seq(seq(a||i||j1||j2||j3, j3 = j2..5), j2 = j1..5), j1 = 1..5), i = 1..6)}) :
    Ss3 := { } :for i to nops(slabc3) do if lhs(slabc3[i]) = rhs(slabc3[i]) then Ss3 :=
    Ss3 union {lhs(slabc3[i])} :fi:od: nops(Ss3)
```

$$70 \tag{1.1.20}$$

```
> slabc4 := solve({coeffs(expand(add(add(add(add(add((a||i||j1||j2||j3
    ||j4)p_j1 p_j2 p_j3 p_j4, j4 = j3..5), j3 = j2..5), j2 = j1..5), j1 = 1..5)·Ma[i, 1], i = 1..6)),
    {seq(p_i, i = 1..5)})}, {seq(seq(seq(seq(seq(a||i||j1||j2||j3||j4, j4 = j3..5), j3 = j2
    ..5), j2 = j1..5), j1 = 1..5), i = 1..6)}) : Ss4 := { } :for i to nops(slabc4) do
    if lhs(slabc4[i]) = rhs(slabc4[i]) then Ss4 := Ss4 union {lhs(slabc4[i])} :fi:od:
    nops(Ss4)
```

$$160 \tag{1.1.21}$$

```
> syz1 := eval(eval(eval([seq(add((a||i||j)p_j, j = 1..5), i = 1..6)], slabc1), {a41 = 1,
    a43 = 0, a52 = 0, a61 = 0, a62 = 0}), {seq(seq(a||i||j = 0, j = 1..5), i = 1..3)});
  syz2 := eval(eval(eval([seq(add((a||i||j)p_j, j = 1..5), i = 1..6)], slabc1), {a41 = 0,
    a43 = 1, a52 = 0, a61 = 0, a62 = 0}), {seq(seq(a||i||j = 0, j = 1..5), i = 1..3)});
  syz3 := eval(eval(eval([seq(add((a||i||j)p_j, j = 1..5), i = 1..6)], slabc1), {a41 = 0,
    a43 = 0, a52 = 1, a61 = 0, a62 = 0}), {seq(seq(a||i||j = 0, j = 1..5), i = 1..3)});
  syz4 := eval(eval(eval([seq(add((a||i||j)p_j, j = 1..5), i = 1..6)], slabc1), {a41 = 0,
    a43 = 0, a52 = 0, a61 = 1, a62 = 0}), {seq(seq(a||i||j = 0, j = 1..5), i = 1..3)});
  syz5 := eval(eval(eval([seq(add((a||i||j)p_j, j = 1..5), i = 1..6)], slabc1), {a41 = 0,
    a43 = 0, a52 = 0, a61 = 0, a62 = 1}), {seq(seq(a||i||j = 0, j = 1..5), i = 1..3)})
```

$$syz1 := [p_3, -p_2, 0, p_1, 0, 0]$$

$$syz2 := [(v_3 - w[\,])\,p_1 + u_3\,p_2 - v_1\,p_3 + p_5, -v_2\,p_1 + (-u_2 + v_1)\,p_2 - p_4, 0, p_2\,u_1 + p_3, 0, 0]$$

$$syz3 := [-p_4, 0, -p_1, 0, p_2, 0]$$

$$syz4 := [0, p_4, 0, 0, -p_3, p_1]$$

$$syz5 := [0, 0, -p_3, p_4, 0, p_2] \tag{1.1.22}$$

> $simplify([add(syz1[i]\,Ma[i,1], i=1..6), add(syz2[i]\,Ma[i,1], i=1..6), add(syz3[i]\,Ma[i,1], i=1..6), add(syz4[i]\,Ma[i,1], i=1..6), add(syz5[i]\,Ma[i,1], i=1..6)])$

$$[0, 0, 0, 0, 0] \quad \textbf{(1.1.23)}$$

> $[seq(p_4\,syz1[i] + p_3\,syz3[i] + p_2\,syz4[i] - p_1\,syz5[i], i=1..6)]$

$$[0, 0, 0, 0, 0, 0] \quad \textbf{(1.1.24)}$$

> $solve(eval(Ma[1,1], \{p_1=1\}), \{p_4\})$

$$\{p_4 = u_1\,p_2^2 + p_2\,p_3 - p_2\,u_2 + p_2\,v_1 - v_2\} \quad \textbf{(1.1.25)}$$

> $solve(eval(Ma[2,1], \{p_1=1, p_4=u_1\,p_2^2 + p_2\,p_3 - p_2\,u_2 + p_2\,v_1 - v_2\}), \{p_5\})$

$$\{p_5 = u_1\,p_2\,p_3 - u_3\,p_2 + p_3^2 + v_1\,p_3 - v_3 + w[\,]\} \quad \textbf{(1.1.26)}$$

> $solve(eval(Ma[5,1], \{p_1=1, p_4=u_1\,p_2^2 + p_2\,p_3 - p_2\,u_2 + p_2\,v_1 - v_2, p_5=u_1\,p_2\,p_3 - u_3\,p_2 + p_3^2 + v_1\,p_3 - v_3 + w[\,]\}), \{p_6\})$

$$\{p_6 = p_2^3\,u_1^2 + 2\,p_2^2\,p_3\,u_1 - p_2^2\,u_1\,u_2 + 2\,p_2^2\,u_1\,v_1 + p_2\,p_3^2 - u_2\,p_2\,p_3 + 2\,p_2\,p_3\,v_1 - p_2\,u_1\,v_2 - p_2\,u_2\,v_1 + p_2\,v_1^2 - p_2\,u_4 + p_2\,w[\,] - p_3\,v_2 - v_1\,v_2 - v_4\} \quad \textbf{(1.1.27)}$$

> $simplify(eval([Ma[3,1], Ma[4,1], Ma[6,1]], \{p_1=1, p_4=u_1\,p_2^2 + p_2\,p_3 - p_2\,u_2 + p_2\,v_1 - v_2, p_5=u_1\,p_2\,p_3 - u_3\,p_2 + p_3^2 + v_1\,p_3 - v_3 + w[\,], p_6=p_2^3\,u_1^2 + 2\,p_2^2\,p_3\,u_1 - p_2^2\,u_1\,u_2 + 2\,p_2^2\,u_1\,v_1 + p_2\,p_3^2 - u_2\,p_2\,p_3 + 2\,p_2\,p_3\,v_1 - p_2\,u_1\,v_2 - p_2\,u_2\,v_1 + p_2\,v_1^2 - p_2\,u_4 + p_2\,w[\,] - p_3\,v_2 - v_1\,v_2 - v_4\}))$

$$[0, 0, 0] \quad \textbf{(1.1.28)}$$

> $tmp := expand(eval([1, p_2, p_3, u_1\,p_2^2 + p_2\,p_3 - p_2\,u_2 + p_2\,v_1 - v_2, u_1\,p_2\,p_3 - u_3\,p_2 + p_3^2 + v_1\,p_3 - v_3 + w[\,], p_2^3\,u_1^2 + 2\,p_2^2\,p_3\,u_1 - p_2^2\,u_1\,u_2 + 2\,p_2^2\,u_1\,v_1 + p_2\,p_3^2 - u_2\,p_2\,p_3 + 2\,p_2\,p_3\,v_1 - p_2\,u_1\,v_2 - p_2\,u_2\,v_1 + p_2\,v_1^2 - p_2\,u_4 + p_2\,w[\,] - p_3\,v_2 - v_1\,v_2 - v_4], \{p_2=\chi, p_3=\lambda - u_1\,\chi\}))$

$$tmp := [1, \chi, -u_1\,\chi + \lambda, \chi\,\lambda - u_2\,\chi + \chi\,v_1 - v_2, -\chi\,\lambda\,u_1 - \chi\,u_1\,v_1 - u_3\,\chi + \lambda^2 + \lambda\,v_1 - v_3 + w[\,], \chi\,\lambda^2 - \chi\,\lambda\,u_2 + 2\,\chi\,\lambda\,v_1 - \chi\,u_2\,v_1 + \chi\,v_1^2 - \chi\,u_4 + \chi\,w[\,] - \lambda\,v_2 - v_1\,v_2 - v_4] \quad \textbf{(1.1.29)}$$

> $tmp00 := eval(tmp, \{\chi=0, \lambda=0\}) : tmp01 := eval(diff(eval(tmp, \{\chi=0\}), \lambda), \{\lambda=0\}) : tmp02 := diff(eval(tmp, \{\chi=0\}), \lambda\$2) :$
> $tmp10 := eval(diff(tmp, \chi), \{\lambda=0\}) : tmp11 := eval(diff(tmp, \chi, \lambda), \{\lambda=0\}) :$
> $tmp12 := diff(tmp, \chi, \lambda\$2) :$

> $(tmp00 + \lambda\,tmp01 + \lambda^2\,tmp02) + \chi\,(tmp10 + \lambda\,tmp11 + \lambda^2\,tmp12)$

$$[1, 0, 0, -v_2, -v_3 + w[\,], -v_1\,v_2 - v_4] + \lambda\,[0, 0, 1, 0, v_1, -v_2] + \lambda^2\,[0, 0, 0, 0, 2, 0] + \chi\,(\lambda^2\,[0, 0, 0, 0, 0, 2] + \lambda\,[0, 0, 0, 1, -u_1, -u_2 + 2\,v_1] + [0, 1, -u_1, -u_2 + v_1, -u_1\,v_1 - u_3, -u_2\,v_1 + v_1^2 - u_4 + w[\,]]) \quad \textbf{(1.1.30)}$$

> $Matrix([tmp00, tmp01, tmp02, tmp10, tmp11, tmp12])$

$$\begin{bmatrix} 1 & 0 & 0 & -v_2 & -v_3 + w[\,] & -v_1 v_2 - v_4 & \cdots \\ 0 & 0 & 1 & 0 & v_1 & -v_2 & \cdots \\ 0 & 0 & 0 & 0 & 2 & 0 & \cdots \\ 0 & 1 & -u_1 & -u_2 + v_1 & -u_1 v_1 - u_3 & -u_2 v_1 + v_1^2 - u_4 + w & \cdots \\ 0 & 0 & 0 & 1 & -u_1 & -u_2 + 2 v_1 & \cdots \\ 0 & 0 & 0 & 0 & 0 & 2 & \cdots \end{bmatrix} \quad \textbf{(1.1.31)}$$

> $simplify(LinearAlgebra\text{:-}Determinant(Matrix([tmp00, tmp01, tmp02, tmp10, tmp11, tmp12])))$

$$-4 \quad \textbf{(1.1.32)}$$

# compatibility

> $DGsetup([x, y, t1, t2, t3], [u, v, w], M5J, 5):$

> $eq12$ **union** $eq13$ **union** $eq23[4..6]$; $nops(\%)$

$$\{u_1 w_{2,2} - u_2 w_{1,2} + v_1 w_{1,2} - v_2 w_{1,1} - w_{1,4} + w_{2,3}, u_1 u_{2,2} - u_2 u_{1,2} - u_{1,1} v_2 + u_{1,2} v_1 - u_{1,4} + u_{2,3} - w_1, u_1 v_{2,2} - u_2 v_{1,2} + v_1 v_{1,2} - v_2 v_{1,1} - v_{1,4} + v_{2,3} + w_2, u_1 u_{2,3} + u_1 w_1 - u_3 u_{1,2} - u_{1,1} v_3 + u_{1,1} w[\,] + u_{1,3} v_1 - u_{1,5} + u_{3,3}, u_1 v_{2,3} - u_1 w_2 - u_3 v_{1,2} + v_1 v_{1,3} - v_3 v_{1,1} + v_{1,1} w[\,] - v_{1,5} + v_{3,3}, u_1 w_{2,3} - u_3 w_{1,2} + v_1 w_{1,3} - v_3 w_{1,1} + w[\,] w_{1,1} + w_1^2 - w_{1,5} + w_{3,3}, u_2 w_{2,3} - u_3 w_{2,2} + v_2 w_{1,3} - v_3 w_{1,2} + w[\,] w_{1,2} + w_1 w_2 - w_{2,5} + w_{3,4}, u_1 w_2 + u_2 u_{2,3} - u_3 u_{2,2} - u_{1,2} v_3 + u_{1,2} w[\,] + u_{1,3} v_2 - u_{2,5} + u_{3,4} + w_3, u_2 v_{2,3} - u_2 w_2 - u_3 v_{2,2} + v_1 w_2 + v_2 v_{1,3} - v_2 w_1 - v_3 v_{1,2} + v_{1,2} w[\,] - v_{2,5} + v_{3,4} - w_4\}$$

$$9 \quad \textbf{(1.2.1)}$$

> $eq5u := \{u_1 u_{2,2} - u_2 u_{1,2} - u_{1,1} v_2 + u_{1,2} v_1 - u_{1,4} + u_{2,3} - w_1, u_1 u_{2,3} + u_1 w_1 - u_3 u_{1,2} - u_{1,1} v_3 + u_{1,1} w[\,] + u_{1,3} v_1 - u_{1,5} + u_{3,3}, u_1 w_2 + u_2 u_{2,3} - u_3 u_{2,2} - u_{1,2} v_3 + u_{1,2} w[\,] + u_{1,3} v_2 - u_{2,5} + u_{3,4} + w_3\}:$
>
> $eq5v := \{u_1 v_{2,2} - u_2 v_{1,2} + v_1 v_{1,2} - v_2 v_{1,1} - v_{1,4} + v_{2,3} + w_2, u_1 v_{2,3} - u_1 w_2 - u_3 v_{1,2} + v_1 v_{1,3} - v_3 v_{1,1} + v_{1,1} w[\,] - v_{1,5} + v_{3,3}, u_2 v_{2,3} - u_2 w_2 - u_3 v_{2,2} + v_1 w_2 + v_2 v_{1,3} - v_2 w_1 - v_3 v_{1,2} + v_{1,2} w[\,] - v_{2,5} + v_{3,4} - w_4\}:$
>
> $eq5w := \{u_1 w_{2,2} - u_2 w_{1,2} + v_1 w_{1,2} - v_2 w_{1,1} - w_{1,4} + w_{2,3}, u_1 w_{2,3} - u_3 w_{1,2} + v_1 w_{1,3} - v_3 w_{1,1} + w[\,] w_{1,1} + w_1^2 - w_{1,5} + w_{3,3}, u_2 w_{2,3} - u_3 w_{2,2} + v_2 w_{1,3} - v_3 w_{1,2} + w[\,] w_{1,2} + w_1 w_2 - w_{2,5} + w_{3,4}\}:$

> $sl2u := solve(eq5u, \{u_{1,4}, u_{1,5}, u_{2,5}\}) : sl2v := solve(eq5v, \{v_{1,4}, v_{1,5}, v_{2,5}\}) : sl2w :=$

$solve(eq5w, \{w_{1,4}, w_{1,5}, w_{2,5}\})$ : $sl2 := sl2u$ **union** $sl2v$ **union** $sl2w$ :

> $jet2 := \{seq(seq(u_{i,j}, j = i..5), i = 1..5), seq(seq(v_{i,j}, j = i..5), i = 1..5), seq(seq(w_{i,j}, j = i..5), i = 1..5)\}$ :
> $jet3 := \{seq(seq(seq(u_{i,j,k}, k = j..5), j = i..5), i = 1..5), seq(seq(seq(v_{i,j,k}, k = j..5), j = i..5), i = 1..5), seq(seq(seq(w_{i,j,k}, k = j..5), j = i..5), i = 1..5)\}$ :

> # for k to nops(eq5w) **do**: $S2 := \{\}$ :**for** i **to** nops(jet2) **do if** $diff(eq5w[k], jet2[i]) \neq 0$ **then** $S2 := S2$ **union** $\{jet2[i]\}$ :**fi**:**od**: print(S2);**od**:

> $eliminate(eval(\{seq(seq(TotalDiff(eq5u[i], j), j = 1..5), i = 1..nops(eq5u))\}, sl2), \{u_{1,1,4}, u_{1,2,4}, u_{1,3,4}, u_{1,4,4}, u_{1,4,5}, u_{1,1,5}, u_{1,2,5}, u_{1,3,5}, u_{1,5,5}, u_{2,2,5}, u_{2,3,5}, u_{2,4,5}, u_{2,5,5}\})[2]$,
> $eliminate(eval(\{seq(seq(TotalDiff(eq5v[i], j), j = 1..5), i = 1..nops(eq5v))\}, sl2), \{v_{1,1,4}, v_{1,2,4}, v_{1,3,4}, v_{1,4,4}, v_{1,4,5}, v_{1,1,5}, v_{1,2,5}, v_{1,3,5}, v_{1,5,5}, v_{2,2,5}, v_{2,3,5}, v_{2,4,5}, v_{2,5,5}\})[2]$,
> $eliminate(eval(\{seq(seq(TotalDiff(eq5w[i], j), j = 1..5), i = 1..nops(eq5w))\}, sl2), \{w_{1,1,4}, w_{1,2,4}, w_{1,3,4}, w_{1,4,4}, w_{1,4,5}, w_{1,1,5}, w_{1,2,5}, w_{1,3,5}, w_{1,5,5}, w_{2,2,5}, w_{2,3,5}, w_{2,4,5}, w_{2,5,5}\})[2]$

$$\varnothing, \varnothing, \varnothing \qquad \textbf{(1.2.2)}$$

> $DGsetup([x, y, t1, t2, t3, t4], [u, v, w], M5J, 5)$ :

> $eq12$ **union** $eq13$ **union** $eq23[4..6]$ **union** $eq14[4..6]$ **union** $eq24$ **union** $eq34[4..4]$ **union** $eq34[6..7]$; $nops(\%)$

$$\{u_1 w_{2,2} - u_2 w_{1,2} + v_1 w_{1,2} - v_2 w_{1,1} - w_{1,4} + w_{2,3}, u_1 u_{2,2} - u_2 u_{1,2} - u_{1,1} v_2 + u_{1,2} v_1 - u_{1,4} + u_{2,3} - w_1, u_1 v_{2,2} - u_2 v_{1,2} + v_1 v_{1,2} - v_2 v_{1,1} - v_{1,4} + v_{2,3} + w_2, u_1 u_{2,3} + u_1 w_1 - u_3 u_{1,2} - u_{1,1} v_3 + u_{1,1} w[\,] + u_{1,3} v_1 - u_{1,5} + u_{3,3}, u_1 v_{2,3} - u_1 w_2 - u_3 v_{1,2} + v_1 v_{1,3} - v_3 v_{1,1} + v_{1,1} w[\,] - v_{1,5} + v_{3,3}, u_1 w_{2,3} - u_3 w_{1,2} + v_1 w_{1,3} - v_3 w_{1,1} + w[\,] w_{1,1} + w_1^2 - w_{1,5} + w_{3,3}, u_2 u_{2,4} - u_4 u_{2,2} - u_{1,2} v_4 + u_{1,4} v_2 + u_{2,2} w[\,] - v_2 w_1 - u_{2,6} + u_{4,4}, u_2 v_{2,4} - u_4 v_{2,2} + v_2 v_{1,4} + v_2 w_2 - v_4 v_{1,2} + v_{2,2} w[\,] - v_{2,6} + v_{4,4}, w_{2,4} u_2 - u_4 w_{2,2} + v_2 w_{1,4} - v_4 w_{1,2} + w[\,] w_{2,2} + w_2^2 - w_{2,6} + w_{4,4}, u_1 w_{2,4} - u_4 w_{1,2} + v_1 w_{1,4} - v_4 w_{1,1} + w[\,] w_{1,2} + w_1 w_2 - w_{1,6} + w_{3,4}, u_2 w_{2,3} - u_3 w_{2,2} + v_2 w_{1,3} - v_3 w_{1,2} + w[\,] w_{1,2} + w_1 w_2 - w_{2,5} + w_{3,4}, u_1 w_2 + u_2 u_{2,3} - u_3 u_{2,2} - u_{1,2} v_3 + u_{1,2} w[\,] + u_{1,3} v_2 - u_{2,5} + u_{3,4} + w_3, u_1 v_{2,4} - u_4 v_{1,2} + v_1 v_{1,4} + v_2 w_1 - v_4 v_{1,1} + v_{1,2} w[\,] - v_{1,6} + v_{3,4} + w_4, u_3 w_{2,4} - u_4 w_{2,3} + v_3 w_{1,4} - v_4 w_{1,3} - w[\,] w_{1,4} + w[\,] w_{2,3} - w_1 w_4 + w_2 w_3 - w_{3,6} + w_{4,5}, u_1 u_{2,4} - u_1 w_2 + u_2 w_1 - u_4 u_{1,2} - u_{1,1} v_4 + u_{1,2} w[\,] + u_{1,4} v_1 - v_1 w_1 - u_{1,6} + u_{3,4} - w_3, u_2 v_{2,3} - u_2 w_2 - u_3 v_{2,2} + v_1 w_2 + v_2 v_{1,3} - v_2 w_1 - v_3 v_{1,2} + v_{1,2} w[\,] - v_{2,5} + v_{3,4} - w_4, -u_1 w_4 + u_2 w_3 + u_3 u_{2,4} - u_3 w_2 - u_4 u_{2,3} - u_{1,3} v_4 + u_{1,4} v_3 - u_{1,4} w[\,] + u_{2,3} w[\,] - v_3 w_1 + w[\,] w_1 - u_{3,6} + u_{4,5} - w_5,$$

$$u_3 v_{2,4} - u_4 v_{2,3} + u_4 w_2 - v_1 w_4 + v_2 w_3 + v_3 v_{1,4} - v_4 v_{1,3} + v_4 w_1 - v_{1,4} w[\,] + v_{2,3} w[\,] - w[\,] w_2 - v_{3,6} + v_{4,5} + w_6\}$$

18 **(1.2.3)**

> $eq6u := \{u_1 u_{2,2} - u_2 u_{1,2} - u_{1,1} v_2 + u_{1,2} v_1 - u_{1,4} + u_{2,3} - w_1,\ u_1 u_{2,3} + u_1 w_1 - u_3 u_{1,2} - u_{1,1} v_3 + u_{1,1} w[\,] + u_{1,3} v_1 - u_{1,5} + u_{3,3},\ u_1 w_2 + u_2 u_{2,3} - u_3 u_{2,2} - u_{1,2} v_3 + u_{1,2} w[\,] + u_{1,3} v_2 - u_{2,5} + u_{3,4} + w_3,\ u_2 u_{2,4} - u_4 u_{2,2} - u_{1,2} v_4 + u_{1,4} v_2 + u_{2,2} w[\,] - v_2 w_1 - u_{2,6} + u_{4,4},\ u_1 u_{2,4} - u_1 w_2 + u_2 w_1 - u_4 u_{1,2} - u_{1,1} v_4 + u_{1,2} w[\,] + u_{1,4} v_1 - v_1 w_1 - u_{1,6} + u_{3,4} - w_3,\ -u_1 w_4 + u_2 w_3 + u_3 u_{2,4} - u_3 w_2 - u_4 u_{2,3} - u_{1,3} v_4 + u_{1,4} v_3 - u_{1,4} w[\,] + u_{2,3} w[\,] - v_3 w_1 + w[\,] w_1 - u_{3,6} + u_{4,5} - w_5\}:$

$eq6v := \{u_1 v_{2,2} - u_2 v_{1,2} + v_1 v_{1,2} - v_2 v_{1,1} - v_{1,4} + v_{2,3} + w_2,\ u_1 v_{2,3} - u_1 w_2 - u_3 v_{1,2} + v_1 v_{1,3} - v_3 v_{1,1} + v_{1,1} w[\,] - v_{1,5} + v_{3,3},\ u_2 v_{2,3} - u_2 w_2 - u_3 v_{2,2} + v_1 w_2 + v_2 v_{1,3} - v_2 w_1 - v_3 v_{1,2} + v_{1,2} w[\,] - v_{2,5} + v_{3,4} - w_4,\ u_2 v_{2,4} - u_4 v_{2,2} + v_2 v_{1,4} + v_2 w_2 - v_4 v_{1,2} + v_{2,2} w[\,] - v_{2,6} + v_{4,4},\ u_1 v_{2,4} - u_4 v_{1,2} + v_1 v_{1,4} + v_2 w_1 - v_4 v_{1,1} + v_{1,2} w[\,] - v_{1,6} + v_{3,4} + w_4,\ u_3 v_{2,4} - u_4 v_{2,3} + u_4 w_2 - v_1 w_4 + v_2 w_3 + v_3 v_{1,4} - v_4 v_{1,3} + v_4 w_1 - v_{1,4} w[\,] + v_{2,3} w[\,] - w[\,] w_2 - v_{3,6} + v_{4,5} + w_6\}:$

$eq6w := \{u_1 w_{2,2} - u_2 w_{1,2} + v_1 w_{1,2} - v_2 w_{1,1} - w_{1,4} + w_{2,3},\ u_1 w_{2,3} - u_3 w_{1,2} + v_1 w_{1,3} - v_3 w_{1,1} + w[\,] w_{1,1} + w_1^2 - w_{1,5} + w_{3,3},\ u_2 w_{2,3} - u_3 w_{2,2} + v_2 w_{1,3} - v_3 w_{1,2} + w[\,] w_{1,2} + w_1 w_2 - w_{2,5} + w_{3,4},\ w_{2,4} u_2 - u_4 w_{2,2} + v_2 w_{1,4} - v_4 w_{1,2} + w[\,] w_{2,2} + w_2^2 - w_{2,6} + w_{4,4},\ u_1 w_{2,4} - u_4 w_{1,2} + v_1 w_{1,4} - v_4 w_{1,1} + w[\,] w_{1,2} + w_1 w_2 - w_{1,6} + w_{3,4},\ u_3 w_{2,4} - u_4 w_{2,3} + v_3 w_{1,4} - v_4 w_{1,3} - w[\,] w_{1,4} + w[\,] w_{2,3} - w_1 w_4 + w_2 w_3 - w_{3,6} + w_{4,5}\}:$

> $sl2u := solve(eq6u, \{u_{1,4}, u_{1,5}, u_{2,5}, u_{1,6}, u_{2,6}, u_{3,6}\}) : sl2v := solve(eq6v, \{v_{1,4}, v_{1,5}, v_{2,5}, v_{1,6}, v_{2,6}, v_{3,6}\}) : sl2w := solve(eq6w, \{w_{1,4}, w_{1,5}, w_{2,5}, w_{1,6}, w_{2,6}, w_{3,6}\}) :$
$sl2 := sl2u$ **union** $sl2v$ **union** $sl2w :$

> $jet2 := \{seq(seq(u_{i,j}, j = i..6), i = 1..6), seq(seq(v_{i,j}, j = i..6), i = 1..6), seq(seq(w_{i,j}, j = i..6), i = 1..6)\}:$

$jet3 := \{seq(seq(seq(u_{i,j,k}, k = j..6), j = i..6), i = 1..6), seq(seq(seq(v_{i,j,k}, k = j..6), j = i..6), i = 1..6), seq(seq(seq(w_{i,j,k}, k = j..6), j = i..6), i = 1..6)\}:$

> \# *for k to nops(eq6w)* **do**: $S2 := \{\}$ :**for** *i* **to** *nops(jet2)* **do if** $diff(eq6w[k], jet2[i]) \neq 0$ **then** $S2 := S2$ **union** $\{jet2[i]\}$ :**fi**:**od**: *print(S2)*;**od**:

> $eliminate(eval(\{seq(seq(TotalDiff(eq5u[i], j), j = 1..6), i = 1..nops(eq5u))\}, sl2), \{u_{1,1,4}, u_{1,2,4}, u_{1,3,4}, u_{1,4,4}, u_{1,4,5}, u_{1,4,6}, u_{1,1,5}, u_{1,2,5}, u_{1,3,5}, u_{1,5,5}, u_{1,5,6}, u_{2,2,5}, u_{2,3,5}, u_{2,4,5}, u_{2,5,5}, u_{2,5,6}, u_{1,1,6}, u_{1,2,6}, u_{1,3,6}, u_{1,6,6}, u_{2,2,6}, u_{2,3,6}, u_{2,4,6}, u_{2,6,6}, u_{3,3,6}, u_{3,4,6}, u_{3,5,6}, u_{3,6,6}\})[2],$

$eliminate(eval(\{seq(seq(TotalDiff(eq5v[i], j), j = 1..6), i = 1..nops(eq5v))\}, sl2), \{v_{1,1,4}, v_{1,2,4}, v_{1,3,4}, v_{1,4,4}, v_{1,4,5}, v_{1,4,6}, v_{1,1,5}, v_{1,2,5}, v_{1,3,5}, v_{1,5,5}, v_{1,5,6}, v_{2,2,5}, v_{2,3,5}, v_{2,4,5}, v_{2,5,5}, v_{2,5,6}, v_{1,1,6}, v_{1,2,6}, v_{1,3,6}, v_{1,6,6}, v_{2,2,6}, v_{2,3,6}, v_{2,4,6}, v_{2,6,6}, v_{3,3,6}, v_{3,4,6},$

$v_{3,5,6}, v_{3,6,6}\}\big)[2],$

$eliminate\Big(eval\big(\{seq(seq(TotalDiff(eq5w[i], j), j=1..6), i=1..nops(eq5w))\}, sl2\big),$
$\{w_{1,1,4}, w_{1,2,4}, w_{1,3,4}, w_{1,4,4}, w_{1,4,5}, w_{1,4,6}, w_{1,1,5}, w_{1,2,5}, w_{1,3,5}, w_{1,5,5}, w_{1,5,6}, w_{2,2,5}, w_{2,3,5}, w_{2,4,5}, w_{2,5,5}, u_{2,5,6}, w_{1,1,6}, w_{1,2,6}, w_{1,3,6}, w_{1,6,6}, w_{2,2,6}, w_{2,3,6}, w_{2,4,6}, w_{2,6,6}, w_{3,3,6}, w_{3,4,6}, w_{3,5,6}, w_{3,6,6}\}\Big)[2]$

$$\varnothing, \varnothing, \varnothing \quad \textbf{(1.2.4)}$$

\>

\> $ChangeFrame(M6p):$

\>

\> $var := x, y, t1, t2, t3, t4, t5, t6 : varq := x, y, t1, t2, t3, t4, t5, t6, q : DGsetup([varq], M8p):$

\> $V1 := evalDG(D\_t1 + diff(v(var), x)\, D\_x + diff(u(var), x)\, D\_y - q\, D\_x + diff(w(var), x)\, D\_q):$
$V2 := evalDG(D\_t2 + diff(v(var), y)\, D\_x + diff(u(var), y)\, D\_y - q\, D\_y + diff(w(var), y)\, D\_q):$

\> $ToJet(V1, \{u(var), v(var), w(var)\}, notation = jetnumbers), ToJet(V2, \{u(var), v(var), w(var)\}, notation = jetnumbers)$

$$-(-v_1 + q)\, D\_x + u_1\, D\_y + D\_t1 + w_1\, D\_q,\ v_2\, D\_x - (-u_2 + q)\, D\_y + D\_t2 + w_2\, D\_q \quad \textbf{(1.12)}$$

\> $eq12 := ToJet(DGinfo(LieDerivative(V1, V2), \text{"CoefficientSet"}), \{u(var), v(var), w(var)\}, notation = jetnumbers)$

$$eq12 := \{u_1 w_{2,2} - u_2 w_{1,2} + w_{1,2} v_1 - v_2 w_{1,1} - w_{1,4} + w_{2,3}, u_1 u_{2,2} - u_{1,2} u_2 - u_{1,1} v_2 + u_{1,2} v_1 - u_{1,4} + u_{2,3} - w_1, v_{2,2} u_1 - u_2 v_{1,2} + v_{1,2} v_1 - v_2 v_{1,1} - v_{1,4} + v_{2,3} + w_2\} \quad \textbf{(1.13)}$$

\> $V3 := evalDG(D\_t3 + diff(v(var), t1)\, D\_x + diff(u(var), t1)\, D\_y - w(var)\, D\_x - q\, D\_t1 + diff(w(var), t1)\, D\_q):$
$V4 := evalDG(D\_t4 + diff(v(var), t2)\, D\_x + diff(u(var), t2)\, D\_y - w(var)\, D\_y - q\, D\_t2 + diff(w(var), t2)\, D\_q):$

\> $ToJet(V3, \{u(var), v(var), w(var)\}, notation = jetnumbers), ToJet(V4, \{u(var), v(var), w(var)\}, notation = jetnumbers)$

$$(v_3 - w[\,])\, D\_x + u_3\, D\_y - q\, D\_t1 + D\_t3 + w_3\, D\_q,\ v_4\, D\_x + (u_4 - w[\,])\, D\_y - q\, D\_t2 + D\_t4 + w_4\, D\_q \quad \textbf{(1.14)}$$

\> $V3a := evalDG(V3 + q\, V1) : V4a := evalDG(V4 + q\, V2):$

\> $eq13 := ToJet(DGinfo(LieDerivative(V1, V3a), \text{"CoefficientSet"}), \{u(var), v(var), w(var)\}, notation = jetnumbers);$
$eq23 := map(coeffs, ToJet(DGinfo(LieDerivative(V2, V3a), \text{"CoefficientSet"}), \{u(var), v(var), w(var)\}, notation = jetnumbers), \{q\})$

$$eq13 := \{u_1 u_{2,3} + u_1 w_1 - u_3 u_{1,2} - u_{1,1} v_3 + u_{1,1} w[\,] + u_{1,3} v_1 - u_{1,5} + u_{3,3}, v_{2,3} u_1 - u_1 w_2 - v_{1,2} u_3 + v_{1,3} v_1 - v_{1,1} v_3 + v_{1,1} w[\,] - v_{1,5} + v_{3,3}, u_1 w_{2,3} - u_3 w_{1,2} + v_1 w_{1,3} - v_3 w_{1,1} + w[\,] w_{1,1} + w_1^2 - w_{1,5} + w_{3,3}\}$$

$$eq23 := \{-u_1 w_{2,2} + u_2 w_{1,2} - w_{1,2} v_1 + v_2 w_{1,1} + w_{1,4} - w_{2,3}, -u_1 u_{2,2} + u_{1,2} u_2 + u_{1,1} v_2 - u_{1,2} v_1 + u_{1,4} - u_{2,3} + w_1, -v_{2,2} u_1 + u_2 v_{1,2} - v_{1,2} v_1 + v_2 v_{1,1} + v_{1,4} \quad \textbf{(1.15)}$$

$- v_{2,3} - w_2, u_2 w_{2,3} - u_3 w_{2,2} + v_2 w_{1,3} - v_3 w_{1,2} + w[\ ] w_{1,2} + w_1 w_2 - w_{2,5} + w_{3,4},$
$u_1 w_2 + u_{2,3} u_2 - u_3 u_{2,2} - u_{1,2} v_3 + u_{1,2} w[\ ] + u_{1,3} v_2 - u_{2,5} + u_{3,4} + w_3, u_2 v_{2,3}$
$- u_2 w_2 - v_{2,2} u_3 + w_2 v_1 + v_2 v_{1,3} - v_2 w_1 - v_{1,2} v_3 + v_{1,2} w[\ ] - v_{2,5} + v_{3,4} - w_4\}$

> *nops(eq12), nops(eq13), nops(eq23)*

$$3, 3, 6 \quad \textbf{(1.16)}$$

> *eq14 := map(coeffs, ToJet(DGinfo(LieDerivative(V1, V4a), "CoefficientSet"), {u(var), v(var), w(var)}, notation = jetnumbers), {q});*
> *eq24 := ToJet(DGinfo(LieDerivative(V2, V4a), "CoefficientSet"), {u(var), v(var), w(var)}, notation = jetnumbers)*

$eq14 := \{u_1 w_{2,2} - u_2 w_{1,2} + w_{1,2} v_1 - v_2 w_{1,1} - w_{1,4} + w_{2,3}, u_1 u_{2,2} - u_{1,2} u_2 - u_{1,1} v_2$
$+ u_{1,2} v_1 - u_{1,4} + u_{2,3} - w_1, v_{2,2} u_1 - u_2 v_{1,2} + v_{1,2} v_1 - v_2 v_{1,1} - v_{1,4} + v_{2,3} + w_2,$
$u_1 w_{2,4} - u_4 w_{1,2} + v_1 w_{1,4} - v_4 w_{1,1} + w[\ ] w_{1,2} + w_1 w_2 - w_{1,6} + w_{3,4}, u_1 v_{2,4}$
$- v_{1,2} u_4 + v_1 v_{1,4} + v_2 w_1 - v_4 v_{1,1} + v_{1,2} w[\ ] - v_{1,6} + v_{3,4} + w_4, u_{2,4} u_1 - u_1 w_2$
$+ u_2 w_1 - u_4 u_{1,2} - v_4 u_{1,1} + u_{1,2} w[\ ] + v_1 u_{1,4} - w_1 v_1 - u_{1,6} + u_{3,4} - w_3\}$

$eq24 := \{u_2 u_{2,4} - u_4 u_{2,2} - u_{1,2} v_4 + u_{1,4} v_2 + u_{2,2} w[\ ] - v_2 w_1 - u_{2,6} + u_{4,4}, v_{2,4} u_2$ **(1.17)**
$- u_4 v_{2,2} + v_{1,4} v_2 + w_2 v_2 - v_4 v_{1,2} + v_{2,2} w[\ ] - v_{2,6} + v_{4,4}, w_{2,4} u_2 - u_4 w_{2,2}$
$+ v_2 w_{1,4} - v_4 w_{1,2} + w[\ ] w_{2,2} + w_2^2 - w_{2,6} + w_{4,4}\}$

> *eq34 := map(coeffs, expand(ToJet(DGinfo(LieDerivative(V3a, V4a), "CoefficientSet"), {u(var), v(var), w(var)}, notation = jetnumbers)), {q})*

$eq34 := \{u_1 w_{2,2} - u_2 w_{1,2} + w_{1,2} v_1 - v_2 w_{1,1} - w_{1,4} + w_{2,3}, u_1 u_{2,2} - u_{1,2} u_2 - u_{1,1} v_2$ **(1.18)**
$+ u_{1,2} v_1 - u_{1,4} + u_{2,3} - w_1, v_{2,2} u_1 - u_2 v_{1,2} + v_{1,2} v_1 - v_2 v_{1,1} - v_{1,4} + v_{2,3} + w_2,$
$u_3 w_{2,4} - u_4 w_{2,3} + v_3 w_{1,4} - v_4 w_{1,3} - w[\ ] w_{1,4} + w[\ ] w_{2,3} - w_1 w_4 + w_2 w_3 - w_{3,6}$
$+ w_{4,5}, u_1 w_{2,4} - u_2 w_{2,3} + u_3 w_{2,2} - u_4 w_{1,2} + v_1 w_{1,4} - v_2 w_{1,3} + v_3 w_{1,2} - v_4 w_{1,1}$
$- w_{1,6} + w_{2,5}, -u_1 w_4 + u_2 w_3 + u_3 u_{2,4} - u_3 w_2 - u_4 u_{2,3} - u_{1,3} v_4 + u_{1,4} v_3$
$- u_{1,4} w[\ ] + u_{2,3} w[\ ] - w_1 v_3 + w_1 w[\ ] - u_{3,6} + u_{4,5} - w_5, u_3 v_{2,4} - u_4 v_{2,3} + u_4 w_2$
$- v_1 w_4 + v_2 w_3 + v_3 v_{1,4} - v_4 v_{1,3} + v_4 w_1 - v_{1,4} w[\ ] + v_{2,3} w[\ ] - w_2 w[\ ] - v_{3,6}$
$+ v_{4,5} + w_6, u_{2,4} u_1 - 2 u_1 w_2 - u_{2,3} u_2 + u_2 w_1 + u_3 u_{2,2} - u_4 u_{1,2} - v_4 u_{1,1} + u_{1,2} v_3$
$- u_{1,3} v_2 + v_1 u_{1,4} - w_1 v_1 - u_{1,6} + u_{2,5} - 2 w_3, u_1 v_{2,4} - u_2 v_{2,3} + u_2 w_2 + v_{2,2} u_3$
$- v_{1,2} u_4 + v_1 v_{1,4} - w_2 v_1 - v_2 v_{1,3} + 2 v_2 w_1 + v_{1,2} v_3 - v_4 v_{1,1} - v_{1,6} + v_{2,5} + 2 w_4\}$

> *slv123 := solve(eq12* **union** *eq13* **union** *eq23[4 ..6],* $\{u_{1,1}, u_{1,2}, u_{2,2}, v_{1,1}, v_{1,2}, v_{2,2}, w_{1,1}, w_{1,2}, w_{2,2}\}$*) : simplify(eval(eq23[1 ..6], slv123))*

$$\{0\} \quad \textbf{(1.19)}$$

> *ToJet(V1, {u(var), v(var), w(var)}); ToJet(V2, {u(var), v(var), w(var)}); ToJet(V3, {u(var), v(var), w(var)}); ToJet(V4, {u(var), v(var), w(var)})*

$$-(-v_x + q)\, D\_x + u_x\, D\_y + D\_t1 + w_x\, D\_q$$

$$v_y D\_x - \left(-u_y + q\right) D\_y + D\_t2 + w_y D\_q$$
$$-\left(-v_{t1} + w\right) D\_x + u_{t1} D\_y - q D\_t1 + D\_t3 + w_{t1} D\_q$$
$$v_{t2} D\_x - \left(-u_{t2} + w\right) D\_y - q D\_t2 + D\_t4 + w_{t2} D\_q \quad \textbf{(1.20)}$$

> $ToJet(V3a, \{u(var), v(var), w(var)\}); ToJet(V4a, \{u(var), v(var), w(var)\})$

$$-\left(q^2 - q v_x + w - v_{t1}\right) D\_x + \left(q u_x + u_{t1}\right) D\_y + D\_t3 + \left(q w_x + w_{t1}\right) D\_q$$
$$\left(q v_y + v_{t2}\right) D\_x - \left(q^2 - q u_y + w - u_{t2}\right) D\_y + D\_t4 + \left(q w_y + w_{t2}\right) D\_q \quad \textbf{(1.21)}$$

> $V5 := evalDG(D\_t5 + (diff(v(var), t3) - q\, w(var))\, D\_x + diff(u(var), t3)\, D\_y - q\, D\_t3 + diff(w(var), t3)\, D\_q) :$
> $V6 := evalDG(D\_t6 + diff(v(var), t4)\, D\_x + (diff(u(var), t4) - q\, w(var))\, D\_y - q\, D\_t4 + diff(w(var), t4)\, D\_q) :$

> $V5a := evalDG(V5 + q\, V3a) : V6a := evalDG(V6 + q\, V4a) :$

> $ToJet(V5a, \{u(var), v(var), w(var), z1(var), z2(var)\}); ToJet(V6a, \{u(var), v(var), w(var), z1(var), z2(var)\})$

$$-\left(q^3 - v_x q^2 + 2 q w - v_{t1} q - v_{t3}\right) D\_x + \left(u_x q^2 + u_{t1} q + u_{t3}\right) D\_y + D\_t5 + \left(w_x q^2 + w_{t1} q + w_{t3}\right) D\_q$$
$$\left(v_y q^2 + v_{t2} q + v_{t4}\right) D\_x - \left(q^3 - u_y q^2 + 2 q w - u_{t2} q - u_{t4}\right) D\_y + D\_t6 + \left(w_y q^2 + w_{t2} q + w_{t4}\right) D\_q \quad \textbf{(1.22)}$$

> $V5 := evalDG(D\_t5 + diff(v(var), t3)\, D\_x + diff(u(var), t3)\, D\_y - w(var)\, D\_t1 - q\, D\_t3 + diff(w(var), t3)\, D\_q) :$
> $V6 := evalDG(D\_t6 + diff(v(var), t4)\, D\_x + diff(u(var), t4)\, D\_y - w(var)\, D\_t2 - q\, D\_t4 + diff(w(var), t4)\, D\_q) :$

> $V5a := evalDG(V5 + q\, V3a + w(var)\, V1) : V6a := evalDG(V6 + q\, V4a + w(var)\, V2) :$

> $ToJet(V5, \{u(var), v(var), w(var), z1(var), z2(var)\}); ToJet(V6, \{u(var), v(var), w(var), z1(var), z2(var)\})$

$$v_{t3} D\_x + u_{t3} D\_y - w D\_t1 - q D\_t3 + D\_t5 + w_{t3} D\_q$$
$$v_{t4} D\_x + u_{t4} D\_y - w D\_t2 - q D\_t4 + D\_t6 + w_{t4} D\_q \quad \textbf{(1.23)}$$

> $ToJet(V5a, \{u(var), v(var), w(var), z1(var), z2(var)\}); ToJet(V6a, \{u(var), v(var), w(var), z1(var), z2(var)\})$

$$-\left(q^3 - v_x q^2 + 2 q w - v_{t1} q - w v_x - v_{t3}\right) D\_x + \left(u_x q^2 + u_{t1} q + w u_x + u_{t3}\right) D\_y + D\_t5 + \left(w_x q^2 + w_{t1} q + w w_x + w_{t3}\right) D\_q$$
$$\left(v_y q^2 + v_{t2} q + w v_y + v_{t4}\right) D\_x - \left(q^3 - u_y q^2 + 2 q w - u_{t2} q - w u_y - u_{t4}\right) D\_y + D\_t6 + \left(w_y q^2 + w_{t2} q + w w_y + w_{t4}\right) D\_q \quad \textbf{(1.24)}$$

> $V5 := evalDG(D\_t5 + diff(v(var), t3)\, D\_x + diff(u(var), t3)\, D\_y + (z1(var) + q\, z2(var))\, D\_x - (w(var) + z2(var))\, D\_t1 - q\, D\_t3 + diff(w(var), t3)\, D\_q) :$
> $V6 := evalDG(D\_t6 + diff(v(var), t4)\, D\_x + diff(u(var), t4)\, D\_y + (z1(var) + q\, z2(var))\, D\_y - (w(var) + z2(var))\, D\_t2 - q\, D\_t4 + diff(w(var), t4)\, D\_q) :$

> $V5a := evalDG\left(V5 + q\, V3 + \left(q^2 + w(var) + z2(var)\right) V1\right) : V6a := evalDG\left(V6 + q\, V4 + \left(q^2 + w(var) + z2(var)\right) V2\right) :$

> simplify(ToJet(V5a, {u(var), v(var), w(var), z0(var), z1(var), z2(var), z3(var)}));
ToJet(V6a, {u(var), v(var), w(var), z0(var), z1(var), z2(var), z3(var)})

$$-\left(-\left(q^2+w+z2\right) v_x+q^3-\left(-2\,w+v_{t1}\right) q-z1-v_{t3}\right) D\_x+\left(\left(q^2+w+z2\right) u_x+u_{t1}\,q+u_{t3}\right) D\_y+D\_t5+\left(\left(q^2+w+z2\right) w_x+w_{t1}\,q+w_{t3}\right) D\_q$$

$$\left(\left(q^2+w+z2\right) v_y+v_{t2}\,q+v_{t4}\right) D\_x-\left(-\left(q^2+w+z2\right)\left(u_y-q\right)-q\left(u_{t2}-w\right)-z1-q\,z2-u_{t4}\right) D\_y+D\_t6+\left(\left(q^2+w+z2\right) w_y+w_{t4}+w_{t2}\,q\right) D\_q \quad \textbf{(1.25)}$$

> eq15 := map(coeffs, expand(ToJet(DGinfo(LieDerivative(V1, V5a), "CoefficientSet"), {u(var), v(var), w(var), z1(var), z2(var)}, notation = jetnumbers)), {q});
eq25 := map(coeffs, expand(ToJet(DGinfo(LieDerivative(V2, V5a), "CoefficientSet"), {u(var), v(var), w(var), z1(var), z2(var)}, notation = jetnumbers)), {q})

$$eq15 := \{u_1 u_{2,3}+u_1 w_1-u_1 z2_1-u_3 u_{1,2}-u_{1,1} v_3+u_{1,1} w[\,]-u_{1,1} z2[\,]+u_{1,3} v_1-u_{1,5}+u_{3,3},\ u_1 w_{2,3}-u_3 w_{1,2}+v_1 w_{1,3}-v_3 w_{1,1}+w[\,] w_{1,1}+w_1^2-w_1 z2_1-w_{1,1} z2[\,]-w_{1,5}+w_{3,3},\ u_1 v_{2,3}-2 u_1 w_2-v_{1,2} u_3+v_1 v_{1,3}-w_1 v_1-z2_1 v_1-v_{1,1} v_3+v_{1,1} w[\,]-v_{1,1} z2[\,]-v_{1,5}+v_{3,3}-w_3-z1_1,\ u_1 w_1 w_2+u_1 w_1 z2_2+v_1 w_1^2+v_1 w_1 z2_1+u_1 w_{2,5}-w_{1,2} u_5+v_1 w_{1,5}-w_{1,1} v_5+w_{1,3} w[\,]+2 w_1 w_3+w_1 z2_3-w_{1,1} z1[\,]+w_{1,3} z2[\,]-w_{1,7}+w_{3,5},\ u_1^2 w_2+u_1^2 z2_2+u_1 v_1 w_1+v_1 u_1 z2_1+u_1 u_{2,5}+u_1 w_3+u_1 z2_3+w_1 u_3-u_{1,2} u_5-u_{1,1} v_5-u_{1,1} z1[\,]+u_{1,3} w[\,]+u_{1,3} z2[\,]+v_1 u_{1,5}-u_{1,7}+u_{3,5},\ u_1 v_1 w_2+u_1 z2_2 v_1+v_1^2 w_1+z2_1 v_1^2+u_1 v_{2,5}+u_1 z1_2-v_{1,2} u_5+v_1 v_{1,5}+w_3 v_1+v_1 z1_1+z2_3 v_1+w_1 v_3-v_{1,1} v_5-v_{1,1} z1[\,]+v_{1,3} w[\,]+v_{1,3} z2[\,]-w[\,] w_1+w_1 z2[\,]-v_{1,7}+v_{3,5}+w_5+z1_3\}$$

$$eq25 := \{-w_{2,2} u_1+u_2 w_{1,2}-w_{1,2} v_1+v_2 w_{1,1}+w_{1,4}-w_{2,3},\ -u_1 u_{2,2}+u_2 u_{1,2}+u_{1,1} v_2-u_{1,2} v_1+u_{1,4}-u_{2,3}+w_1,\ -u_1 v_{2,2}+u_2 v_{1,2}-v_1 v_{1,2}+v_2 v_{1,1}+v_{1,4}-v_{2,3}-w_2,\ u_2 w_{2,3}-u_3 w_{2,2}+v_2 w_{1,3}-v_3 w_{1,2}+w[\,] w_{1,2}+w_1 w_2-w_1 z2_2-w_{1,2} z2[\,]-w_{2,5}+w_{3,4},\ u_1 w_2-u_1 z2_2+u_2 u_{2,3}-u_3 u_{2,2}-u_{1,2} v_3+u_{1,2} w[\,]-u_{1,2} z2[\,]+u_{1,3} v_2-u_{2,5}+u_{3,4}+w_3,\ u_2 v_{2,3}-2 u_2 w_2-v_{2,2} u_3+w_2 v_1-z2_2 v_1+v_2 v_{1,3}-2 v_2 w_1-v_{1,2} v_3+v_{1,2} w[\,]-v_{1,2} z2[\,]-v_{2,5}+v_{3,4}-2 w_4-z1_2,\ -u_1 w[\,] w_{2,2}-w_{2,2} u_1 z2[\,]+u_2 w_{1,2} w[\,]+u_2 w_1 w_2+u_2 w_1 z2_2+u_2 w_{1,2} z2[\,]-v_1 w_{1,2} w[\,]-w_{1,2} z2[\,] v_1+w_{1,1} v_2 w[\,]+v_2 w_1^2+v_2 w_1 z2_1+v_2 w_{1,1} z2[\,]+u_2 w_{2,5}-u_5 w_{2,2}+v_2 w_{1,5}-v_5 w_{1,2}+w_{1,4} w[\,]+w_1 w_4+w_1 z2_4+w_2 w_3-w_{1,2} z1[\,]+w_{1,4} z2[\,]-w_{2,7}+w_{4,5},\ u_1 u_2 w_2+u_1 u_2 z2_2-u_1 u_{2,2} w[\,]-u_1 u_{2,2} z2[\,]+u_1 v_2 w_1+v_2 u_1 z2_1+u_2 u_{1,2} w[\,]+u_2 u_{1,2} z2[\,]+u_{1,1} v_2 w[\,]+u_{1,1} v_2 z2[\,]-u_{1,2} v_1 w[\,]-u_{1,2} v_1 z2[\,]+u_1 w_4+u_1 z2_4+u_2 u_{2,5}+w_2 u_3-u_5 u_{2,2} \quad \textbf{(1.26)}$$

$$- v_{5} u_{1,2} - u_{1,2} z1[\,] + u_{1,4} w[\,] + u_{1,4} z2[\,] + v_{2} u_{1,5} + w[\,] w_{1} + w_{1} z2[\,] - u_{2,7}$$
$$+ u_{4,5} + w_{5}, -u_{1} v_{2,2} w[\,] - u_{1} v_{2,2} z2[\,] + u_{2} v_{1} w_{2} + u_{2} v_{1} z2_{2} + u_{2} v_{1,2} w[\,]$$
$$+ u_{2} v_{1,2} z2[\,] + v_{1} v_{2} w_{1} + v_{1} v_{2} z2_{1} - v_{1} v_{1,2} w[\,] - v_{1} v_{1,2} z2[\,] + v_{2} v_{1,1} w[\,]$$
$$+ v_{2} v_{1,1} z2[\,] + u_{2} v_{2,5} + u_{2} z1_{2} - u_{5} v_{2,2} + v_{1} w_{4} + z2_{4} v_{1} + v_{2} v_{1,5} + v_{2} z1_{1} + v_{3} w_{2}$$
$$- v_{5} v_{1,2} - v_{1,2} z1[\,] + v_{1,4} w[\,] + v_{1,4} z2[\,] - 2 w_{2} w[\,] - v_{2,7} + v_{4,5} + z1_{4}\}$$

```
> eq16 := map(coeffs, expand(ToJet(DGinfo(LieDerivative(V1, V6a), "CoefficientSet"),
      {u(var), v(var), w(var), z1(var), z2(var)}, notation = jetnumbers)), {q});
  eq26 := map(coeffs, expand(ToJet(DGinfo(LieDerivative(V2, V6a), "CoefficientSet"),
      {u(var), v(var), w(var), z1(var), z2(var)}, notation = jetnumbers)), {q})
```

$$eq16 := \{w_{2,2} u_{1} - u_{2} w_{1,2} + w_{1,2} v_{1} - v_{2} w_{1,1} - w_{1,4} + w_{2,3}, u_{1} u_{2,2} - u_{2} u_{1,2} - u_{1,1} v_{2}$$
$$+ u_{1,2} v_{1} - u_{1,4} + u_{2,3} - w_{1}, u_{1} v_{2,2} - u_{2} v_{1,2} + v_{1} v_{1,2} - v_{2} v_{1,1} - v_{1,4} + v_{2,3} + w_{2},$$
$$u_{1} w_{2,4} - u_{4} w_{1,2} + w_{1,4} v_{1} - v_{4} w_{1,1} + w[\,] w_{1,2} + w_{1} w_{2} - w_{2} z2_{1} - w_{1,2} z2[\,] - w_{1,6}$$
$$+ w_{3,4}, v_{2,4} u_{1} - u_{4} v_{1,2} + v_{1,4} v_{1} + v_{2} w_{1} - v_{2} z2_{1} - v_{4} v_{1,1} + v_{1,2} w[\,] - v_{1,2} z2[\,]$$
$$- v_{1,6} + v_{3,4} + w_{4}, u_{2,4} u_{1} - 2 u_{1} w_{2} + u_{2} w_{1} - z2_{1} u_{2} - u_{4} u_{1,2} - v_{4} u_{1,1} + u_{1,2} w[\,]$$
$$- u_{1,2} z2[\,] + u_{1,4} v_{1} - 2 w_{1} v_{1} - u_{1,6} + u_{3,4} - 2 w_{3} - z1_{1}, u_{1} w[\,] w_{2,2} + u_{1} w_{2}^{2}$$
$$+ u_{1} w_{2} z2_{2} + w_{2,2} u_{1} z2[\,] - u_{2} w_{1,2} w[\,] - u_{2} w_{1,2} z2[\,] + v_{1} w_{1,2} w[\,] + v_{1} w_{1} w_{2}$$
$$+ v_{1} w_{2} z2_{1} + w_{1,2} z2[\,] v_{1} - w_{1,1} v_{2} w[\,] - v_{2} w_{1,1} z2[\,] + w_{2,6} u_{1} - u_{6} w_{1,2} + w_{1,6} v_{1}$$
$$- v_{6} w_{1,1} + w[\,] w_{2,3} + w_{1} w_{4} + w_{2} w_{3} + w_{2} z2_{3} - w_{1,2} z1[\,] + w_{2,3} z2[\,] - w_{1,8}$$
$$+ w_{3,6}, u_{1} v_{2} w_{2} + u_{1} v_{2} z2_{2} + u_{1} v_{2,2} w[\,] + u_{1} v_{2,2} z2[\,] - u_{2} v_{1,2} w[\,] - u_{2} v_{1,2} z2[\,]$$
$$+ v_{1} v_{2} w_{1} + v_{1} v_{2} z2_{1} + v_{1} v_{1,2} w[\,] + v_{1} v_{1,2} z2[\,] - v_{2} v_{1,1} w[\,] - v_{2} v_{1,1} z2[\,] + v_{2,6} u_{1}$$
$$- u_{6} v_{1,2} + v_{1,6} v_{1} + v_{2} w_{3} + v_{2} z2_{3} + v_{4} w_{1} - v_{6} v_{1,1} - v_{1,2} z1[\,] + v_{2,3} w[\,] + v_{2,3} z2[\,]$$
$$+ w_{2} w[\,] + w_{2} z2[\,] - v_{1,8} + v_{3,6} + w_{6}, u_{1} u_{2} w_{2} + u_{1} u_{2} z2_{2} + u_{1} u_{2,2} w[\,]$$
$$+ u_{1} u_{2,2} z2[\,] - u_{2} u_{1,2} w[\,] - u_{2} u_{1,2} z2[\,] + u_{2} v_{1} w_{1} + u_{2} v_{1} z2_{1} - u_{1,1} v_{2} w[\,]$$
$$- u_{1,1} v_{2} z2[\,] + u_{1,2} v_{1} w[\,] + u_{1,2} v_{1} z2[\,] + u_{2,6} u_{1} + u_{1} z1_{2} + u_{2} w_{3} + z2_{3} u_{2} + u_{4} w_{1}$$
$$- u_{6} u_{1,2} - v_{6} u_{1,1} - u_{1,2} z1[\,] + u_{1,6} v_{1} + w[\,] u_{2,3} + u_{2,3} z2[\,] + v_{1} z1_{1} - 2 w[\,] w_{1}$$
$$- u_{1,8} + u_{3,6} + z1_{3}\}$$

$$eq26 := \{u_{2} v_{2,4} - u_{4} v_{2,2} + v_{2} v_{1,4} + v_{2} w_{2} - v_{2} z2_{2} - v_{4} v_{1,2} + v_{2,2} w[\,] - v_{2,2} z2[\,] - v_{2,6} \quad \mathbf{(1.27)}$$
$$+ v_{4,4}, w_{2,4} u_{2} - u_{4} w_{2,2} + v_{2} w_{1,4} - v_{4} w_{1,2} + w[\,] w_{2,2} + w_{2}^{2} - w_{2} z2_{2} - w_{2,2} z2[\,]$$
$$- w_{2,6} + w_{4,4}, u_{2} u_{2,4} - u_{2} w_{2} - u_{2} z2_{2} - u_{4} u_{2,2} - u_{1,2} v_{4} + u_{1,4} v_{2} + u_{2,2} w[\,]$$
$$- u_{2,2} z2[\,] - 2 v_{2} w_{1} - u_{2,6} + u_{4,4} - w_{4} - z1_{2}, u_{2} w_{2}^{2} + u_{2} w_{2} z2_{2} + w_{1} w_{2} v_{2}$$
$$+ v_{2} w_{2} z2_{1} + u_{2} w_{2,6} - w_{2,2} u_{6} + v_{2} w_{1,6} - v_{6} w_{1,2} + w[\,] w_{2,4} + 2 w_{2} w_{4} + w_{2} z2_{4}$$
$$- w_{2,2} z1[\,] + w_{2,4} z2[\,] - w_{2,8} + w_{4,6}, u_{2} v_{2} w_{2} + u_{2} v_{2} z2_{2} + v_{2}^{2} w_{1} + v_{2}^{2} z2_{1} + u_{2} v_{2,6}$$

$- v_{2,2} u_6 + v_2 v_{1,6} + v_2 w_4 + v_2 z2_4 + v_4 w_2 - v_6 v_{1,2} - v_{2,2} z1[\,] + v_{2,4} w[\,] + v_{2,4} z2[\,]$
$- v_{2,8} + v_{4,6}, u_2^2 w_2 + u_2^2 z2_2 + v_2 u_2 w_1 + u_2 v_2 z2_1 + u_2 u_{2,6} + w_4 u_2 + u_2 z1_2 + z2_4 u_2$
$+ u_4 w_2 - u_{2,2} u_6 - u_{1,2} v_6 + v_2 u_{1,6} - u_{2,2} z1[\,] + u_{2,4} w[\,] + u_{2,4} z2[\,] + v_2 z1_1$
$- w_2 w[\,] + w_2 z2[\,] - u_{2,8} + u_{4,6} + w_6 + z1_4\}$

> eq35 := map(coeffs, expand(ToJet(DGinfo(LieDerivative(V3a, V5a), "CoefficientSet"), {u(var), v(var), w(var), z1(var), z2(var)}, notation = jetnumbers)), {q});
> eq45 := map(coeffs, expand(ToJet(DGinfo(LieDerivative(V4a, V5a), "CoefficientSet"), {u(var), v(var), w(var), z1(var), z2(var)}, notation = jetnumbers)), {q})

$eq35 := \{-u_1 z2_1 - u_{1,1} z2[\,], -w_1 z2_1 - w_{1,1} z2[\,], -u_1 w_2 - w_1 v_1 - z2_1 v_1 - v_{1,1} z2[\,]$
$- w_3 - z1_1, u_1 w_1 w_2 + u_1 w_1 z2_2 + v_1 w_1^2 + v_1 w_1 z2_1 + u_1 w_{2,5} - w_{1,2} u_5 + v_1 w_{1,5}$
$- w_{1,1} v_5 + w_{1,3} w[\,] + 2 w_1 w_3 - w_{1,1} z1[\,] - w_{1,7} + w_{3,5}, u_1^2 w_2 + u_1^2 z2_2 + u_1 v_1 w_1$
$+ v_1 u_1 z2_1 + u_1 u_{2,5} + u_1 w_3 + w_1 u_3 - u_{1,2} u_5 - u_{1,1} v_5 - u_{1,1} z1[\,] + u_{1,3} w[\,]$
$+ v_1 u_{1,5} - u_{1,7} + u_{3,5}, u_1 v_1 w_2 + u_1 z2_2 v_1 + v_1^2 w_1 + z2_1 v_1^2 + u_1 v_{2,5} + u_1 z1_2 - w_2 u_3$
$- v_{1,2} u_5 + v_1 v_{1,5} + v_1 w_3 + v_1 z1_1 - v_{1,1} v_5 - v_{1,1} z1[\,] + v_{1,3} w[\,] + 2 w_1 z2[\,] - v_{1,7}$
$+ v_{3,5}, u_1 u_3 w_2 + u_1 u_3 z2_2 - u_1 u_{2,3} w[\,] - u_1 u_{2,3} z2[\,] + u_1 v_3 w_1 + u_1 v_3 z2_1$
$- 2 u_1 w[\,] w_1 - u_1 w[\,] z2_1 - u_1 w_1 z2[\,] + u_3 u_{1,2} w[\,] + u_3 u_{1,2} z2[\,] + u_{1,1} v_3 w[\,]$
$+ u_{1,1} v_3 z2[\,] - u_{1,1} w[\,]^2 - u_{1,1} w[\,] z2[\,] - u_{1,3} v_1 w[\,] - u_{1,3} v_1 z2[\,] + u_1 z2_5$
$+ u_3 u_{2,5} + u_3 w_3 - u_5 u_{2,3} - u_{1,3} v_5 - u_{1,3} z1[\,] + u_{1,5} v_3 + u_{1,5} z2[\,] - u_{3,7} + u_{5,5},$
$-u_1 w[\,] w_{2,3} - u_1 w_{2,3} z2[\,] + u_3 w_{1,2} w[\,] + u_3 w_1 w_2 + u_3 w_1 z2_2 + u_3 w_{1,2} z2[\,]$
$- v_1 w_{1,3} w[\,] - v_1 w_{1,3} z2[\,] + v_3 w[\,] w_{1,1} + w_1^2 v_3 + v_3 w_1 z2_1 + v_3 w_{1,1} z2[\,]$
$- w[\,]^2 w_{1,1} - 2 w_1^2 w[\,] - w[\,] w_1 z2_1 - w[\,] w_{1,1} z2[\,] - w_1^2 z2[\,] + u_3 w_{2,5} - u_5 w_{2,3}$
$+ v_3 w_{1,5} - v_5 w_{1,3} + w_1 z2_5 + w_3^2 - w_{1,3} z1[\,] + w_{1,5} z2[\,] - w_{3,7} + w_{5,5},$
$-u_1 v_{2,3} w[\,] - u_1 v_{2,3} z2[\,] + u_1 w[\,] w_2 + u_1 w_2 z2[\,] + u_3 v_1 w_2 + u_3 v_1 z2_2$
$+ u_3 v_{1,2} w[\,] + u_3 v_{1,2} z2[\,] + v_1 v_3 w_1 + v_1 v_3 z2_1 - v_1 v_{1,3} w[\,] - v_1 v_{1,3} z2[\,]$
$- v_1 w[\,] w_1 - v_1 w[\,] z2_1 + v_3 v_{1,1} w[\,] + v_3 v_{1,1} z2[\,] - v_{1,1} w[\,]^2 - v_{1,1} w[\,] z2[\,]$
$+ u_3 v_{2,5} + u_3 z1_2 - u_5 v_{2,3} + u_5 w_2 + z2_5 v_1 + v_3 v_{1,5} + v_3 w_3 + v_3 z1_1 - v_5 v_{1,3} + v_5 w_1$
$- v_{1,3} z1[\,] + v_{1,5} z2[\,] - 2 w[\,] w_3 - w[\,] z1_1 + w_1 z1[\,] - v_{3,7} + v_{5,5} + w_7 + z1_5\}$

$eq45 := \{-v_3 v_{1,4} - v_5 v_{1,2} - v_{1,2} z1[\,] + 2 v_{1,4} w[\,] - u_3 v_{2,4} - u_5 v_{2,2} - v_2 w_3 + v_2 v_{1,5}$ **(1.28)**
$+ v_4 v_{1,3} - 2 v_4 w_1 + u_2 v_{2,5} + u_4 v_{2,3} - v_{2,3} w[\,] + 2 v_1 w_4 + v_3 w_2 + v_1 v_2 w_1 + v_2 z1_1$
$+ u_2 z1_2 - v_1 v_{1,2} z2[\,] - u_1 v_{2,2} z2[\,] + v_1 v_2 z2_1 + v_2 v_{1,1} z2[\,] + u_2 v_1 z2_2$
$+ u_2 v_{1,2} z2[\,] - v_{2,7} - 2 u_4 w_2 + v_{3,6} - 2 w_6 + v_2 v_{1,1} w[\,] + u_2 v_{1,2} w[\,] - v_1 v_{1,2} w[\,]$

$$- u_{1} v_{2,2} w[\,] + u_{2} v_{1} w_{2}, -w_{2,2} u_{1} + u_{2} w_{1,2} - w_{1,2} v_{1} + v_{2} w_{1,1} + w_{1,4} - w_{2,3},$$
$$-u_{1} u_{2,2} + u_{2} u_{1,2} + u_{1,1} v_{2} - u_{1,2} v_{1} + u_{1,4} - u_{2,3} + w_{1}, -u_{1} v_{2,2} + u_{2} v_{1,2} - v_{1} v_{1,2}$$
$$+ v_{2} v_{1,1} + v_{1,4} - v_{2,3} - w_{2}, -u_{1} w_{2,4} + u_{2} w_{2,3} - u_{3} w_{2,2} + u_{4} w_{1,2} - w_{1,4} v_{1} + v_{2} w_{1,3}$$
$$- v_{3} w_{1,2} + v_{4} w_{1,1} - w_{1} z2_{2} - w_{1,2} z2[\,] + w_{1,6} - w_{2,5}, -u_{2,4} u_{1} + 2 u_{1} w_{2} - u_{1} z2_{2}$$
$$+ u_{2} u_{2,3} - u_{2} w_{1} - u_{3} u_{2,2} + u_{4} u_{1,2} + v_{4} u_{1,1} - u_{1,2} v_{3} - u_{1,2} z2[\,] + u_{1,3} v_{2} - u_{1,4} v_{1}$$
$$+ w_{1} v_{1} + u_{1,6} - u_{2,5} + 2 w_{3}, -v_{2,4} u_{1} + u_{2} v_{2,3} - 2 u_{2} w_{2} - v_{2,2} u_{3} + u_{4} v_{1,2} - v_{1,4} v_{1}$$
$$+ w_{2} v_{1} - z2_{2} v_{1} + v_{2} v_{1,3} - 3 v_{2} w_{1} - v_{1,2} v_{3} + v_{4} v_{1,1} - v_{1,2} z2[\,] + v_{1,6} - v_{2,5} - 3 w_{4}$$
$$- z1_{2}, -u_{1} w[\,] w_{2,2} - w_{2,2} u_{1} z2[\,] + u_{2} w_{1,2} w[\,] + u_{2} w_{1} w_{2} + u_{2} w_{1} z2_{2}$$
$$+ u_{2} w_{1,2} z2[\,] - v_{1} w_{1,2} w[\,] - w_{1,2} z2[\,] v_{1} + w_{1,1} v_{2} w[\,] + v_{2} w_{1}^{2} + v_{2} w_{1} z2_{1}$$
$$+ v_{2} w_{1,1} z2[\,] + u_{2} w_{2,5} - u_{3} w_{2,4} + u_{4} w_{2,3} - u_{5} w_{2,2} + v_{2} w_{1,5} - w_{1,4} v_{3} + v_{4} w_{1,3}$$
$$- v_{5} w_{1,2} + 2 w_{1,4} w[\,] - w[\,] w_{2,3} + 2 w_{1} w_{4} - w_{1,2} z1[\,] - w_{2,7} + w_{3,6},$$
$$-u_{1} w[\,] w_{2,4} - u_{1} w_{2,4} z2[\,] + u_{4} w[\,] w_{1,2} + u_{4} w_{1} w_{2} + u_{4} w_{1} z2_{2} + u_{4} w_{1,2} z2[\,]$$
$$- v_{1} w[\,] w_{1,4} - v_{1} w_{1,4} z2[\,] + v_{4} w[\,] w_{1,1} + v_{4} w_{1}^{2} + v_{4} w_{1} z2_{1} + v_{4} w_{1,1} z2[\,]$$
$$- w[\,]^{2} w_{1,2} - 2 w[\,] w_{1} w_{2} - w[\,] w_{1} z2_{2} - w[\,] w_{1,2} z2[\,] - w_{1} w_{2} z2[\,] + u_{4} w_{2,5}$$
$$- u_{5} w_{2,4} + v_{4} w_{1,5} - v_{5} w_{1,4} + w_{1,6} w[\,] - w[\,] w_{2,5} + w_{1} w_{6} + w_{1} z2_{6} - w_{2} w_{5}$$
$$+ w_{3} w_{4} - w_{1,4} z1[\,] + w_{1,6} z2[\,] - w_{4,7} + w_{5,6}, u_{1} u_{2} w_{2} + u_{1} u_{2} z2_{2} - u_{1} u_{2,2} w[\,]$$
$$- u_{1} u_{2,2} z2[\,] + u_{1} v_{2} w_{1} + v_{2} u_{1} z2_{1} + u_{2} u_{1,2} w[\,] + u_{2} u_{1,2} z2[\,] + u_{1,1} v_{2} w[\,]$$
$$+ u_{1,1} v_{2} z2[\,] - u_{1,2} v_{1} w[\,] - u_{1,2} v_{1} z2[\,] + 2 u_{1} w_{4} + u_{2} u_{2,5} - u_{2} w_{3} - u_{2,4} u_{3}$$
$$+ 2 w_{2} u_{3} + u_{4} u_{2,3} - u_{5} u_{2,2} - v_{5} u_{1,2} - u_{1,2} z1[\,] + v_{4} u_{1,3} - u_{1,4} v_{3} + 2 u_{1,4} w[\,]$$
$$+ v_{2} u_{1,5} - w[\,] u_{2,3} + w_{1} v_{3} + 2 w_{1} z2[\,] - u_{2,7} + u_{3,6} + 2 w_{5}, -u_{1} v_{2,4} w[\,]$$
$$- u_{1} v_{2,4} z2[\,] + u_{4} v_{1} w_{2} + u_{4} v_{1} z2_{2} + u_{4} v_{1,2} w[\,] + u_{4} v_{1,2} z2[\,] + v_{1} v_{4} w_{1} + v_{1} v_{4} z2_{1}$$
$$- v_{1} v_{1,4} w[\,] - v_{1} v_{1,4} z2[\,] - v_{1} w[\,] w_{2} - v_{1} w[\,] z2_{2} - v_{2} w[\,] w_{1} - v_{2} w_{1} z2[\,]$$
$$+ v_{4} v_{1,1} w[\,] + v_{4} v_{1,1} z2[\,] - v_{1,2} w[\,]^{2} - v_{1,2} w[\,] z2[\,] + u_{4} v_{2,5} + u_{4} z1_{2} - u_{5} v_{2,4}$$
$$+ v_{1} w_{6} + z2_{6} v_{1} - v_{2} w_{5} + v_{3} w_{4} + v_{4} v_{1,5} + v_{4} z1_{1} - v_{5} v_{1,4} - v_{1,4} z1[\,] + v_{1,6} w[\,]$$
$$+ v_{1,6} z2[\,] - v_{2,5} w[\,] - 2 w[\,] w_{4} - w[\,] z1_{2} - v_{4,7} + v_{5,6} + z1_{6}, u_{1} u_{4} w_{2} + u_{1} u_{4} z2_{2}$$
$$- u_{1} u_{2,4} w[\,] - u_{1} u_{2,4} z2[\,] + u_{1} v_{4} w_{1} + u_{1} v_{4} z2_{1} - u_{1} w[\,] z2_{2} + u_{1} w_{2} z2[\,]$$
$$- u_{2} w[\,] w_{1} - u_{2} w_{1} z2[\,] + u_{4} u_{1,2} w[\,] + u_{4} u_{1,2} z2[\,] + u_{1,1} v_{4} w[\,] + u_{1,1} v_{4} z2[\,]$$
$$- u_{1,2} w[\,]^{2} - u_{1,2} w[\,] z2[\,] - u_{1,4} v_{1} w[\,] - u_{1,4} v_{1} z2[\,] + v_{1} w[\,] w_{1} + v_{1} w_{1} z2[\,]$$
$$+ u_{1} w_{6} + u_{1} z2_{6} - u_{2} w_{5} + u_{3} w_{4} + u_{4} u_{2,5} - u_{5} u_{2,4} + u_{5} w_{2} - u_{1,4} v_{5} - u_{1,4} z1[\,]$$

$+ u_{1,5} v_4 + u_{1,6} w[\,] + u_{1,6} z2[\,] - u_{2,5} w[\,] + v_5 w_1 + w_1 z1[\,] - u_{4,7} + u_{5,6} + w_7\}$

> eq36 := map(coeffs, expand(ToJet(DGinfo(LieDerivative(V3a, V6a), "CoefficientSet"), {u(var), v(var), w(var), z1(var), z2(var)}, notation = jetnumbers)), {q});
> eq46 := map(coeffs, expand(ToJet(DGinfo(LieDerivative(V4a, V6a), "CoefficientSet"), {u(var), v(var), w(var), z1(var), z2(var)}, notation = jetnumbers)), {q})

$$eq36 := \{u_1 w_{2,2} - u_2 w_{1,2} + v_1 w_{1,2} - v_2 w_{1,1} - w_{1,4} + w_{2,3}, u_1 u_{2,2} - u_2 u_{1,2} - u_{1,1} v_2 + u_{1,2} v_1 - u_{1,4} + u_{2,3} - w_1, u_1 v_{2,2} - u_2 v_{1,2} + v_1 v_{1,2} - v_2 v_{1,1} - v_{1,4} + v_{2,3} + w_2, u_1 w_{2,4} - u_2 w_{2,3} + u_3 w_{2,2} - u_4 w_{1,2} + w_{1,4} v_1 - v_2 w_{1,3} + v_3 w_{1,2} - v_4 w_{1,1} - w_{1,6} + w_{2,5}, v_{2,4} u_1 - u_2 v_{2,3} + u_2 w_2 + v_{2,2} u_3 - u_4 v_{1,2} + v_{1,4} v_1 - w_2 v_1 - v_2 v_{1,3} + 2 v_2 w_1 + v_{1,2} v_3 - v_4 v_{1,1} - v_{1,6} + v_{2,5} + 2 w_4, u_{2,4} u_1 - 3 u_1 w_2 - u_2 u_{2,3} + u_2 w_1 + u_3 u_{2,2} - u_4 u_{1,2} - v_4 u_{1,1} + u_{1,2} v_3 - u_{1,3} v_2 + u_{1,4} v_1 - 2 w_1 v_1 - u_{1,6} + u_{2,5} - 3 w_3 - z1_1, -u_2 w[\,] w_{2,3} + u_3 w[\,] w_{2,2} + u_3 w_2^2 - v_2 w[\,] w_{1,3} + w[\,] w_{1,2} v_3 + v_3 w_1 w_2 - w[\,]^2 w_{1,2} - 2 w[\,] w_1 w_2 + w_{2,6} u_3 - u_6 w_{2,3} + w_{1,6} v_3 - v_6 w_{1,3} - w_{1,6} w[\,] + w[\,] w_{2,5} - w_1 w_6 + w_2 w_5 + w_3 w_4 - w_{2,3} z1[\,] - w_{3,8} + w_{5,6}, u_1 w[\,] w_{2,2} + u_1 w_2^2 - u_2 w_{1,2} w[\,] + v_1 w_{1,2} w[\,] + v_1 w_1 w_2 - w_{1,1} v_2 w[\,] + w_{2,6} u_1 + u_3 w_{2,4} - u_4 w_{2,3} - u_6 w_{1,2} + w_{1,6} v_1 + w_{1,4} v_3 - v_4 w_{1,3} - v_6 w_{1,1} - w_{1,4} w[\,] + 2 w[\,] w_{2,3} + 2 w_2 w_3 - w_{1,2} z1[\,] - w_{1,8} + w_{4,5}, u_1 v_2 w_2 + u_1 v_{2,2} w[\,] - u_2 v_{1,2} w[\,] + v_1 v_2 w_1 + v_1 v_{1,2} w[\,] - v_2 v_{1,1} w[\,] + v_{2,6} u_1 + u_3 v_{2,4} - u_4 v_{2,3} + u_4 w_2 - u_6 v_{1,2} + v_{1,6} v_1 - v_1 w_4 + 2 v_2 w_3 + v_3 v_{1,4} - v_4 v_{1,3} + 2 v_4 w_1 - v_6 v_{1,1} - v_{1,2} z1[\,] - v_{1,4} w[\,] + 2 v_{2,3} w[\,] - v_{1,8} + v_{4,5} + 2 w_6, -u_2 v_{2,3} w[\,] + u_2 w[\,] w_2 + u_3 v_2 w_2 + u_3 v_{2,2} w[\,] - v_1 w[\,] w_2 + v_2 v_3 w_1 - v_2 v_{1,3} w[\,] + v_3 v_{1,2} w[\,] - v_{1,2} w[\,]^2 + u_3 v_{2,6} - u_6 v_{2,3} + u_6 w_2 - v_1 w_6 + v_2 w_5 + v_3 v_{1,6} + v_4 w_3 - v_6 v_{1,3} + v_6 w_1 - v_{1,6} w[\,] - v_{2,3} z1[\,] + v_{2,5} w[\,] + w_2 z1[\,] - v_{3,8} + v_{5,6} + w_8, -u_1 w[\,] w_2 + u_2 u_3 w_2 - u_2 u_{2,3} w[\,] + u_2 v_3 w_1 - u_2 w[\,] w_1 + u_3 u_{2,2} w[\,] + u_{1,2} v_3 w[\,] - u_{1,2} w[\,]^2 - u_{1,3} v_2 w[\,] - u_1 w_6 + u_2 w_5 + u_3 u_{2,6} + u_3 z1_2 + u_4 w_3 - u_6 u_{2,3} - u_{1,3} v_6 + u_{1,6} v_3 - u_{1,6} w[\,] - u_{2,3} z1[\,] + u_{2,5} w[\,] + v_3 z1_1 - 2 w[\,] w_3 - w[\,] z1_1 - u_{3,8} + u_{5,6} + z1_5, u_1 u_2 w_2 + u_1 u_{2,2} w[\,] - u_2 u_{1,2} w[\,] + u_2 v_1 w_1 - u_{1,1} v_2 w[\,] + u_{1,2} v_1 w[\,] + u_{2,6} u_1 - u_1 w_4 + u_1 z1_2 + 2 u_2 w_3 + u_{2,4} u_3 - 2 w_2 u_3 - u_4 u_{2,3} + u_4 w_1 - u_6 u_{1,2} - v_6 u_{1,1} - u_{1,2} z1[\,] - v_4 u_{1,3} + u_{1,4} v_3 - u_{1,4} w[\,] + u_{1,6} v_1 + 2 w[\,] u_{2,3} + v_1 z1_1 - 2 w_1 v_3 - u_{1,8} + u_{4,5} - 2 w_5\}$$

$$eq46 := \{-u_2 w_2 - v_2 w_1 - w_4 - z1_2, u_2 w_2^2 + w_1 w_2 v_2 + u_2 w_{2,6} - u_6 w_{2,2} + v_2 w_{1,6} \qquad \textbf{(1.29)}$$

$$- v_6 w_{1,2} + w[\,] w_{2,4} + 2 w_2 w_4 - w_{2,2} \mathit{z1}[\,] - w_{2,8} + w_{4,6}, u_2 v_2 w_2 + v_2^2 w_1 + v_{2,6} u_2$$
$$- u_6 v_{2,2} + v_{1,6} v_2 + v_2 w_4 + v_4 w_2 - v_{1,2} v_6 - v_{2,2} \mathit{z1}[\,] + v_{2,4} w[\,] - v_{2,8} + v_{4,6}, u_2^2 w_2$$
$$+ u_2 v_2 w_1 + u_2 u_{2,6} + w_4 u_2 + u_2 \mathit{z1}_2 - u_6 u_{2,2} - v_6 u_{1,2} + v_2 u_{1,6} - u_{2,2} \mathit{z1}[\,]$$
$$+ u_{2,4} w[\,] + v_2 \mathit{z1}_1 - v_4 w_1 - u_{2,8} + u_{4,6}, -u_2 v_{2,4} w[\,] + u_4 v_2 w_2 + u_4 v_{2,2} w[\,]$$
$$+ v_2 v_4 w_1 - v_2 v_{1,4} w[\,] - 2 v_2 w[\,] w_2 + v_4 v_{1,2} w[\,] - v_{2,2} w[\,]^2 + v_{2,6} u_4 - u_6 v_{2,4}$$
$$+ v_{1,6} v_4 + v_4 w_4 - v_6 v_{1,4} - v_{2,4} \mathit{z1}[\,] - v_{4,8} + v_{6,6}, -w[\,] w_{2,4} u_2 + w[\,] u_4 w_{2,2} + u_4$$
$$w_2^2 - v_2 w[\,] w_{1,4} + v_4 w[\,] w_{1,2} + v_4 w_1 w_2 - w[\,]^2 w_{2,2} - 2 w[\,] w_2^2 + w_{2,6} u_4$$
$$- u_6 w_{2,4} + w_{1,6} v_4 - v_6 w_{1,4} + w_4^2 - w_{2,4} \mathit{z1}[\,] - w_{4,8} + w_{6,6}, u_2 u_4 w_2 - u_2 u_{2,4} w[\,]$$
$$+ u_2 v_4 w_1 - u_2 w[\,] w_2 + u_4 u_{2,2} w[\,] + u_{1,2} v_4 w[\,] - u_{1,4} v_2 w[\,] - u_{2,2} w[\,]^2$$
$$+ v_2 w[\,] w_1 + u_{2,6} u_4 + u_4 w_4 + u_4 \mathit{z1}_2 - u_6 u_{2,4} + u_6 w_2 - v_6 u_{1,4} + u_{1,6} v_4$$
$$- u_{2,4} \mathit{z1}[\,] + v_4 \mathit{z1}_1 + v_6 w_1 - 2 w[\,] w_4 - w[\,] \mathit{z1}_2 + w_2 \mathit{z1}[\,] - u_{4,8} + u_{6,6} + w_8$$
$$+ \mathit{z1}_6 \}$$

```
> eq56 := map(coeffs, expand(ToJet(DGinfo(LieDerivative(V5a, V6a), "CoefficientSet"),
      {u(var), v(var), w(var), z1(var), z2(var)}, notation = jetnumbers)), {q})
```

$$eq56 := \{ -v_2 u_{1,5} - u_2 u_{2,5} - u_{1,8} + u_{2,7} - 3 w_5 + v_5 u_{1,2} + u_5 u_{2,2} - 2 u_{1,1} v_2 w[\,] \qquad \textbf{(1.30)}$$
$$- 2 u_2 u_{1,2} w[\,] + u_2 v_1 w_1 + 2 u_{1,2} v_1 w[\,] + 2 u_1 u_{2,2} w[\,] - v_4 u_{1,3} - v_6 u_{1,1} - u_4 u_{2,3}$$
$$+ 2 w[\,] u_{2,3} - u_6 u_{1,2} - 2 u_1 w_4 + u_{1,4} v_3 - 2 u_{1,4} w[\,] + u_{1,6} v_1 + u_{2,4} u_3 - 3 w_2 u_3$$
$$+ u_{2,6} u_1 + 2 u_2 w_3 + u_4 w_1 - w[\,] w_1 - 2 w_1 v_3 + u_1 \mathit{z1}_2 + v_1 \mathit{z1}_1 - u_1 v_2 w_1, v_3 v_{1,4}$$
$$+ v_5 v_{1,2} - 2 v_{1,4} w[\,] + u_3 v_{2,4} + u_5 v_{2,2} + 2 v_2 w_3 - v_2 v_{1,5} - v_4 v_{1,3} + 3 v_4 w_1$$
$$- u_2 v_{2,5} - u_4 v_{2,3} + 2 v_{2,3} w[\,] - 2 v_1 w_4 - v_3 w_2 - v_{1,8} + w_2 w[\,] - v_2 \mathit{z1}_1 - u_2 \mathit{z1}_2$$
$$+ v_{2,7} + 2 u_4 w_2 + 3 w_6 - 2 v_2 v_{1,1} w[\,] - 2 u_2 v_{1,2} w[\,] + 2 v_1 v_{1,2} w[\,] + u_1 v_2 w_2$$
$$+ 2 u_1 v_{2,2} w[\,] - v_6 v_{1,1} - u_6 v_{1,2} + v_{1,6} v_1 + v_{2,6} u_1 - u_2 v_1 w_2, u_{1,4} \mathit{z1}[\,] + v_3 \mathit{z1}_1$$
$$- 2 w[\,] \mathit{z1}_1 - 2 w_1 \mathit{z1}[\,] + u_3 \mathit{z1}_2 - u_{2,3} \mathit{z1}[\,] + u_{4,7} - 2 u_1 w_6 - u_3 w_4 + u_{1,4} v_5$$
$$+ u_{1,6} v_3 - 2 u_{1,6} w[\,] + u_3 u_{2,6} + u_5 u_{2,4} + 2 u_2 w_5 + u_4 w_3 - 2 w_7 - u_{1,3} v_6 - u_{1,5} v_4$$
$$- u_4 u_{2,5} - u_6 u_{2,3} + 2 u_{2,5} w[\,] - u_{3,8} - u_1 v_4 w_1 - u_{1,1} v_4 w[\,] - u_{1,3} v_2 w[\,]$$
$$- u_1 u_4 w_2 - 2 u_1 w[\,] w_2 - u_2 u_{2,3} w[\,] - u_4 u_{1,2} w[\,] + u_2 v_3 w_1 + u_{1,2} v_3 w[\,]$$
$$+ u_{1,4} v_1 w[\,] - 2 v_1 w[\,] w_1 + u_1 u_{2,4} w[\,] + u_2 u_3 w_2 + u_3 u_{2,2} w[\,] - 2 u_5 w_2$$
$$- 2 v_5 w_1 - 2 w[\,] w_3, v_{1,4} \mathit{z1}[\,] + v_{4,7} - v_4 v_{1,5} - v_6 v_{1,3} + 2 v_6 w_1 - u_4 v_{2,5} - u_6 v_{2,3}$$
$$+ 2 u_6 w_2 + 2 w_8 - v_{3,8} - 2 v_1 w_6 - v_3 w_4 + 2 w[\,] w_4 + v_3 v_{1,6} + v_5 v_{1,4} - 2 v_{1,6} w[\,]$$
$$+ u_3 v_{2,6} + u_5 v_{2,4} + 2 v_2 w_5 + v_4 w_3 + 2 v_{2,5} w[\,] - v_1 v_4 w_1 - v_2 v_{1,3} w[\,]$$

$+ 2\, v_2\, w[\ ]\, w_1 - v_4\, v_{1,1}\, w[\ ] - u_2\, v_{2,3}\, w[\ ] + 2\, u_2\, w[\ ]\, w_2 - u_4\, v_1\, w_2 - u_4\, v_{1,2}\, w[\ ]$

$+ v_1\, v_{1,4}\, w[\ ] + v_2\, v_3\, w_1 + v_3\, v_{1,2}\, w[\ ] + u_1\, v_{2,4}\, w[\ ] + u_3\, v_2\, w_2 + u_3\, v_{2,2}\, w[\ ] - v_4\, z1_1$

$- u_4\, z1_2 - v_{2,3}\, z1[\ ] + 2\, w[\ ]\, z1_2 + 2\, w_2\, z1[\ ],\ -v_6\, u_{1,5} - u_6\, u_{2,5} - w_6\, u_3 + z1_7$

$- u_{2,5}\, z1[\ ] + u_{1,6}\, z1[\ ] + v_5\, z1_1 + z1[\ ]\, z1_1 + u_5\, z1_2 - u_{1,1}\, v_2\, w[\ ]^2 - u_1\, v_6\, w_1$

$- u_{1,1}\, v_6\, w[\ ] - u_{1,5}\, v_2\, w[\ ] + v_5\, u_{1,6} + u_5\, u_{2,6} + w_5\, u_4 - 2\, w_5\, w[\ ] - u_2\, u_{1,2}\, w[\ ]^2$

$- u_1\, u_6\, w_2 - u_1\, w_2\, z1[\ ] - u_2\, u_{2,5}\, w[\ ] - u_6\, u_{1,2}\, w[\ ] - u_3\, w[\ ]\, w_2 + u_{1,2}\, v_1\, w[\ ]^2$

$+ u_2\, v_5\, w_1 + u_2\, w_1\, z1[\ ] + u_{1,2}\, v_5\, w[\ ] + u_{1,6}\, v_1\, w[\ ] + v_1\, w[\ ]\, z1_1 + u_1\, u_{2,2}\, w[\ ]^2$

$+ u_1\, u_{2,6}\, w[\ ] + u_1\, w[\ ]\, z1_2 + u_2\, u_5\, w_2 + u_5\, u_{2,2}\, w[\ ] + w_7\, u_2 - u_{1,8}\, w[\ ] + u_{2,7}\, w[\ ]$

$- 2\, w[\ ]^2\, w_1 + u_2\, v_1\, w[\ ]\, w_1 + u_4\, w[\ ]\, w_1 - u_{5,8} + u_{6,7} - w_8\, u_1 - u_1\, v_2\, w[\ ]\, w_1,$

$-w_8\, v_1 - v_{1,8}\, w[\ ] + 2\, w[\ ]^2\, w_2 + v_{2,7}\, w[\ ] - z1_8 - v_6\, z1_1 - u_6\, z1_2 - v_{2,5}\, z1[\ ]$

$- z1[\ ]\, z1_2 + v_{1,6}\, z1[\ ] + v_5\, v_{1,6} + u_5\, v_{2,6} + w_5\, v_4 - w_6\, v_3 + 2\, w_6\, w[\ ] - v_6\, v_{1,5}$

$- u_6\, v_{2,5} - u_2\, v_1\, w[\ ]\, w_2 + u_1\, v_2\, w[\ ]\, w_2 - v_2\, v_{1,1}\, w[\ ]^2 - v_1\, v_6\, w_1 - v_2\, v_{1,5}\, w[\ ]$

$- v_2\, w[\ ]\, z1_1 - v_6\, v_{1,1}\, w[\ ] - u_2\, v_{1,2}\, w[\ ]^2 - u_2\, v_{2,5}\, w[\ ] - u_2\, w[\ ]\, z1_2 - u_6\, v_1\, w_2$

$- u_6\, v_{1,2}\, w[\ ] - v_1\, w_2\, z1[\ ] - v_{5,8} + v_{6,7} - v_3\, w[\ ]\, w_2 + v_1\, v_{1,2}\, w[\ ]^2 + v_1\, v_{1,6}\, w[\ ]$

$+ v_2\, v_5\, w_1 + v_2\, w_1\, z1[\ ] + v_5\, v_{1,2}\, w[\ ] + u_1\, v_{2,2}\, w[\ ]^2 + u_1\, v_{2,6}\, w[\ ] + u_5\, v_2\, w_2$

$+ u_5\, v_{2,2}\, w[\ ] + v_4\, w[\ ]\, w_1 + w_7\, v_2,\ u_1\, w_{2,2} - u_2\, w_{1,2} + v_1\, w_{1,2} - v_2\, w_{1,1} - w_{1,4}$

$+ w_{2,3},\ u_1\, u_{2,2} - u_2\, u_{1,2} - u_{1,1}\, v_2 + u_{1,2}\, v_1 - u_{1,4} + u_{2,3} - w_1,\ u_1\, v_{2,2} - u_2\, v_{1,2}$

$+ v_1\, v_{1,2} - v_2\, v_{1,1} - v_{1,4} + v_{2,3} + w_2,\ u_1\, w_{2,4} - u_2\, w_{2,3} + u_3\, w_{2,2} - u_4\, w_{1,2} + w_{1,4}\, v_1$

$- v_2\, w_{1,3} + v_3\, w_{1,2} - v_4\, w_{1,1} - w_{1,6} + w_{2,5},\ u_{2,4}\, u_1 - 3\, u_1\, w_2 - u_2\, u_{2,3} + u_2\, w_1$

$+ u_3\, u_{2,2} - u_4\, u_{1,2} - v_4\, u_{1,1} + u_{1,2}\, v_3 - u_{1,3}\, v_2 + u_{1,4}\, v_1 - 2\, w_1\, v_1 - u_{1,6} + u_{2,5} - 3\, w_3$

$- z1_1,\ v_{2,4}\, u_1 - u_2\, v_{2,3} + 2\, u_2\, w_2 + v_{2,2}\, u_3 - u_4\, v_{1,2} + v_{1,4}\, v_1 - w_2\, v_1 - v_2\, v_{1,3} + 3\, v_2\, w_1$

$+ v_{1,2}\, v_3 - v_4\, v_{1,1} - v_{1,6} + v_{2,5} + 3\, w_4 + z1_2,\ 2\, u_1\, w[\ ]\, w_{2,2} + u_1\, w_2^2 - 2\, u_2\, w_{1,2}\, w[\ ]$

$- u_2\, w_1\, w_2 + 2\, v_1\, w_{1,2}\, w[\ ] + v_1\, w_1\, w_2 - 2\, w_{1,1}\, v_2\, w[\ ] - v_2\, w_1^2 + w_{2,6}\, u_1 - u_2\, w_{2,5}$

$+ u_3\, w_{2,4} - u_4\, w_{2,3} + u_5\, w_{2,2} - u_6\, w_{1,2} + w_{1,6}\, v_1 - v_2\, w_{1,5} + w_{1,4}\, v_3 - v_4\, w_{1,3}$

$+ v_5\, w_{1,2} - v_6\, w_{1,1} - 2\, w_{1,4}\, w[\ ] + 2\, w[\ ]\, w_{2,3} - w_1\, w_4 + w_2\, w_3 - w_{1,8} + w_{2,7},$

$u_1\, w[\ ]\, w_{2,4} - u_2\, w[\ ]\, w_{2,3} + u_3\, w[\ ]\, w_{2,2} + u_3\, w_2^2 - u_4\, w[\ ]\, w_{1,2} - u_4\, w_1\, w_2$

$+ v_1\, w[\ ]\, w_{1,4} - v_2\, w[\ ]\, w_{1,3} + w[\ ]\, w_{1,2}\, v_3 + v_3\, w_1\, w_2 - v_4\, w[\ ]\, w_{1,1} - v_4\, w_1^2 + w_{2,6}\, u_3$

$- u_4\, w_{2,5} + u_5\, w_{2,4} - u_6\, w_{2,3} + w_{1,6}\, v_3 - v_4\, w_{1,5} + v_5\, w_{1,4} - v_6\, w_{1,3} - 2\, w_{1,6}\, w[\ ]$

$+ 2\, w[\ ]\, w_{2,5} - 2\, w_1\, w_6 + 2\, w_2\, w_5 + w_{1,4}\, z1[\ ] - w_{2,3}\, z1[\ ] - w_{3,8} + w_{4,7},$

$$u_1 w[\,]^2 w_{2,2} + u_1 w[\,] w_2^2 - u_2 w_{1,2} w[\,]^2 - u_2 w[\,] w_1 w_2 + v_1 w_{1,2} w[\,]^2 + v_1 w[\,] w_1 w_2 - w_{1,1} v_2 w[\,]^2 - w_1^2 v_2 w[\,] + u_1 w[\,] w_{2,6} - u_2 w[\,] w_{2,5} + u_5 w[\,] w_{2,2} + u_5 w_2^2 - u_6 w[\,] w_{1,2} - u_6 w_1 w_2 + v_1 w[\,] w_{1,6} - v_2 w[\,] w_{1,5} + v_5 w[\,] w_{1,2} + v_5 w_1 w_2 - v_6 w[\,] w_{1,1} - v_6 w_1^2 + w[\,] w_1 w_4 - w[\,] w_2 w_3 + u_5 w_{2,6} - u_6 w_{2,5} + v_5 w_{1,6} - v_6 w_{1,5} - w[\,] w_{1,8} + w[\,] w_{2,7} - w_1 w_8 + w_2 w_7 - w_6 w_3 + w_5 w_4 + w_{1,6} z1[\,] - w_{2,5} z1[\,] - w_{5,8} + w_{6,7}\}$$

\>

\> $smu := f \to add\left(add\left(diff\left(f, u_{i,j}\right) p_i p_j, j = i..8\right), i = 1..8\right) : smv := f \to add\left(add\left(diff\left(f, v_{i,j}\right) p_i p_j, j = i..8\right), i = 1..8\right) : smw := f \to add\left(add\left(diff\left(f, w_{i,j}\right) p_i p_j, j = i..8\right), i = 1..8\right) :$

\> *map*(*smu*, *eq12* **union** *eq13* **union** *eq14* **union** *eq15* **union** *eq16* **union** *eq23* **union** *eq24* **union** *eq25* **union** *eq26* **union** *eq34* **union** *eq35* **union** *eq36* **union** *eq45* **union** *eq46* **union** *eq56*) : *nops*(%);
*map*(*smv*, *eq12* **union** *eq13* **union** *eq14* **union** *eq15* **union** *eq16* **union** *eq23* **union** *eq24* **union** *eq25* **union** *eq26* **union** *eq34* **union** *eq35* **union** *eq36* **union** *eq45* **union** *eq46* **union** *eq56*) : *nops*(%);
*map*(*smw*, *eq12* **union** *eq13* **union** *eq14* **union** *eq15* **union** *eq16* **union** *eq23* **union** *eq24* **union** *eq25* **union** *eq26* **union** *eq34* **union** *eq35* **union** *eq36* **union** *eq45* **union** *eq46* **union** *eq56*) : *nops*(%)

23
23
23 **(1.31)**

\>

\> $V1 := evalDG(D\_t1 + (diff(v(var), x) - q)\, D\_x + diff(u(var), x)\, D\_y + diff(w(var), x)\, D\_q) :$
$V2 := evalDG(D\_t2 + diff(v(var), y)\, D\_x + (diff(u(var), y) - q)\, D\_y + diff(w(var), y)\, D\_q) :$

\> $eq12 := ToJet(DGinfo(LieDerivative(V1, V2), \text{"CoefficientSet"}), \{u(var), v(var), w(var)\}, notation = jetnumbers)$

$$eq12 := \{u_1 w_{2,2} - u_2 w_{1,2} + v_1 w_{1,2} - v_2 w_{1,1} - w_{1,4} + w_{2,3}, u_1 u_{2,2} - u_2 u_{1,2} - u_{1,1} v_2 + u_{1,2} v_1 - u_{1,4} + u_{2,3} - w_1, u_1 v_{2,2} - u_2 v_{1,2} + v_1 v_{1,2} - v_2 v_{1,1} - v_{1,4} + v_{2,3} + w_2\} \quad \textbf{(1.32)}$$

\> $V3 := evalDG(D\_t3 + (diff(v(var), t1) - w(var))\, D\_x + diff(u(var), t1)\, D\_y - q\, D\_t1 + diff(w(var), t1)\, D\_q) :$
$V4 := evalDG(D\_t4 + diff(v(var), t2)\, D\_x + (diff(u(var), t2) - w(var))\, D\_y - q\, D\_t2 + diff(w(var), t2)\, D\_q) :$

\> $V3a := evalDG(V3 + q\, V1) : V4a := evalDG(V4 + q\, V2) :$

\>

\>

# Bogdanov Dunajski hierarchy

\> $var := x, y, t1, t2, t3, t4 : varq := x, y, t1, t2, t3, t4, q : DGsetup([varq], M6p) :$

```
> V1 := evalDG(D_t1 + (diff(u(var), x, y) - q) D_x - diff(u(var), x, x) D_y
      + diff(v(var), x) D_q) :
  V2 := evalDG(D_t2 + diff(u(var), y, y) D_x - (diff(u(var), x, y) + q) D_y
      + diff(v(var), y) D_q) :
> ToJet(V1, {u(var), v(var), w(var)}, notation = jetnumbers), ToJet(V2, {u(var), v(var),
      w(var)}, notation = jetnumbers)
```

$$-\left(q - u_{1, 2}\right) D\_x - u_{1, 1}\, D\_y + D\_t1 + v_1\, D\_q,\ u_{2, 2}\, D\_x - \left(q + u_{1, 2}\right) D\_y + D\_t2 + v_2\, D\_q \quad \mathbf{(2.1)}$$

```
> eq12 := ToJet(DGinfo(LieDerivative(V1, V2), "CoefficientSet"), {u(var), v(var),
      w(var)}, notation = jetnumbers)
```

$$eq12 := \{-u_{1, 1}\, v_{2, 2} + 2\, u_{1, 2}\, v_{1, 2} - u_{2, 2}\, v_{1, 1} - v_{1, 4} + v_{2, 3},\ u_{1, 1}\, u_{1, 2, 2} - 2\, u_{1, 2}\, u_{1, 1, 2} + u_{2, 2}\, u_{1, 1, 1} + u_{1, 1, 4} - u_{1, 2, 3} - v_1,\ -u_{1, 1}\, u_{2, 2, 2} + 2\, u_{1, 2}\, u_{1, 2, 2} - u_{2, 2}\, u_{1, 1, 2} - u_{1, 2, 4} + u_{2, 2, 3} + v_2\} \quad \mathbf{(2.2)}$$

```
> V3 := evalDG(D_t3 + (diff(u(var), y, t1) - v(var)) D_x - diff(u(var), x, t1) D_y
      - q D_t1 + diff(v(var), t1) D_q) :
  V4 := evalDG(D_t4 + diff(u(var), y, t2) D_x - (diff(u(var), x, t2) + v(var)) D_y
      - q D_t2 + diff(v(var), t2) D_q) :
> ToJet(V3, {u(var), v(var), w(var)}, notation = jetnumbers), ToJet(V4, {u(var), v(var),
      w(var)}, notation = jetnumbers)
```

$$\left(u_{2, 3} - v[\,]\right) D\_x - u_{1, 3}\, D\_y - q\, D\_t1 + D\_t3 + v_3\, D\_q,\ u_{2, 4}\, D\_x - \left(u_{1, 4} + v[\,]\right) D\_y - q\, D\_t2 + D\_t4 + v_4\, D\_q \quad \mathbf{(2.3)}$$

```
> V3a := evalDG(V3 + q V1) : V4a := evalDG(V4 + q V2) :
> eq13 := ToJet(DGinfo(LieDerivative(V1, V3a), "CoefficientSet"), {u(var), v(var)},
      notation = jetnumbers);
  eq23 := map(coeffs, ToJet(DGinfo(LieDerivative(V2, V3a), "CoefficientSet"), {u(var),
      v(var)}, notation = jetnumbers), {q})
```

$$eq13 := \{u_{1, 1}\, u_{1, 2, 3} - u_{1, 1}\, v_1 - u_{1, 2}\, u_{1, 1, 3} - u_{1, 3}\, u_{1, 1, 2} + u_{2, 3}\, u_{1, 1, 1} - u_{1, 1, 1}\, v[\,] + u_{1, 1, 5} - u_{1, 3, 3},\ -u_{1, 1}\, u_{2, 2, 3} + u_{1, 1}\, v_2 + u_{1, 2}\, u_{1, 2, 3} + u_{1, 3}\, u_{1, 2, 2} - u_{2, 3}\, u_{1, 1, 2} + u_{1, 1, 2}\, v[\,] - u_{1, 2, 5} + u_{2, 3, 3},\ -u_{1, 1}\, v_{2, 3} + u_{1, 2}\, v_{1, 3} + u_{1, 3}\, v_{1, 2} - u_{2, 3}\, v_{1, 1} + v[\,]\, v_{1, 1} + v_1^2 - v_{1, 5} + v_{3, 3}\}$$

$$eq23 := \{u_{1, 1}\, v_{2, 2} - 2\, u_{1, 2}\, v_{1, 2} + u_{2, 2}\, v_{1, 1} + v_{1, 4} - v_{2, 3},\ -u_{1, 1}\, u_{1, 2, 2} + 2\, u_{1, 2}\, u_{1, 1, 2} - u_{2, 2}\, u_{1, 1, 1} - u_{1, 1, 4} + u_{1, 2, 3} + v_1,\ u_{1, 1}\, u_{2, 2, 2} - 2\, u_{1, 2}\, u_{1, 2, 2} + u_{2, 2}\, u_{1, 1, 2} + u_{1, 2, 4} - u_{2, 2, 3} - v_2,\ -u_{1, 2}\, v_{2, 3} + u_{1, 3}\, v_{2, 2} + u_{2, 2}\, v_{1, 3} - u_{2, 3}\, v_{1, 2} + v[\,]\, v_{1, 2} + v_1\, v_2 - v_{2, 5} + v_{3, 4},\ -u_{1, 1}\, v_2 + u_{1, 2}\, u_{1, 2, 3} - u_{1, 3}\, u_{1, 2, 2} - u_{2, 2}\, u_{1, 1, 3} + u_{2, 3}\, u_{1, 1, 2} - u_{1, 1, 2}\, v[\,] + u_{1, 2, 5} - u_{1, 3, 4} + v_3,\ -u_{1, 2}\, u_{2, 2, 3} + 2\, u_{1, 2}\, v_2 + u_{1, 3}\, u_{2, 2, 2} + u_{2, 2}\, u_{1, 2, 3} - u_{2, 2}\, v_1 - u_{2, 3}\, u_{1, 2, 2} + u_{1, 2, 2}\, v[\,] - u_{2, 2, 5} + u_{2, 3, 4} - v_4\} \quad \mathbf{(2.4)}$$

```
> EQ2a := {u[1,1] u[2,2] - u[1,2]^2 + u[1,4] - u[2,3] - v[[]], u[1,1] v[2,2] - 2 u[1,2] v[1,2] + u[2,2] v[1,1] + v[1,4]
      - v[2,3], u[1,2] u[1,3] - u[1,1] u[2,3] + u[1,1] v[] - u[1,5] + u[3,3], -u[1,1] v[2,3] + u[1,2] v[1,3] + u[1,3] v[1,2]
```

$-u_{2,3}v_{1,1}+v[\,]v_{1,1}+v_1^2-v_{1,5}+v_{3,3}, -u_{1,2}v_{2,3}+u_{1,3}v_{2,2}+u_{2,2}v_{1,3}-u_{2,3}v_{1,2}$
$+v[\,]v_{1,2}+v_1v_2-v_{2,5}+v_{3,4}, u_{1,2}u_{2,3}-u_{1,3}u_{2,2}-u_{1,2}v[\,]+u_{2,5}-u_{3,4}+w_{[\,]}\}$

$$EQ2a := \{u_{1,1}u_{2,2}-u_{1,2}^2+u_{1,4}-u_{2,3}-v[\,], -u_{1,1}u_{2,3}+u_{1,1}v[\,]+u_{1,2}u_{1,3}-u_{1,5}+u_{3,3}, u_{1,1}v_{2,2}-2u_{1,2}v_{1,2}+u_{2,2}v_{1,1}+v_{1,4}-v_{2,3}, u_{1,2}u_{2,3}-u_{1,2}v[\,]-u_{2,2}u_{1,3}+u_{2,5}-u_{3,4}+w[\,], -u_{1,1}v_{2,3}+u_{1,2}v_{1,3}+u_{1,3}v_{1,2}-u_{2,3}v_{1,1}+v[\,]v_{1,1}+v_1^2-v_{1,5}+v_{3,3}, -u_{1,2}v_{2,3}+u_{1,3}v_{2,2}+u_{2,2}v_{1,3}-u_{2,3}v_{1,2}+v[\,]v_{1,2}+v_1v_2-v_{2,5}+v_{3,4}\} \quad \textbf{(2.5)}$$

> # where $\{w_1 = v_3 - u_{1,1}v_2 + u_{1,2}v_1, w_2 = v_4 - u_{1,2}v_2 + u_{2,2}v_1\}$

> nops(eq12), nops(eq13), nops(eq23)

$$3, 3, 6 \quad \textbf{(2.6)}$$

> eq14 := map(coeffs, ToJet(DGinfo(LieDerivative(V1, V4a), "CoefficientSet"), {u(var), v(var)}, notation = jetnumbers), {q});
eq24 := ToJet(DGinfo(LieDerivative(V2, V4a), "CoefficientSet"), {u(var), v(var)}, notation = jetnumbers)

$$eq14 := \{-u_{1,1}v_{2,2}+2u_{1,2}v_{1,2}-u_{2,2}v_{1,1}-v_{1,4}+v_{2,3}, u_{1,1}u_{1,2,2}-2u_{1,2}u_{1,1,2}+u_{2,2}u_{1,1,1}+u_{1,1,4}-u_{1,2,3}-v_1, -u_{1,1}u_{2,2,2}+2u_{1,2}u_{1,2,2}-u_{2,2}u_{1,1,2}-u_{1,2,4}+u_{2,2,3}+v_2, -u_{1,1}v_{2,4}+u_{1,2}v_{1,4}+u_{1,4}v_{1,2}-u_{2,4}v_{1,1}+v[\,]v_{1,2}+v_1v_2-v_{1,6}+v_{3,4}, -u_{1,1}u_{2,2,4}+u_{1,2}u_{1,2,4}+u_{1,4}u_{1,2,2}+u_{2,2}v_1-u_{2,4}u_{1,1,2}+u_{1,2,2}v[\,]-u_{1,2,6}+u_{2,3,4}+v_4, u_{1,1}u_{1,2,4}+u_{1,1}v_2-u_{1,2}u_{1,1,4}-2u_{1,2}v_1-u_{1,4}u_{1,1,2}+u_{2,4}u_{1,1,1}-u_{1,1,2}v[\,]+u_{1,1,6}-u_{1,3,4}-v_3\}$$

$$eq24 := \{u_{1,2}u_{1,2,4}-u_{1,4}u_{1,2,2}-u_{2,2}u_{1,1,4}-u_{2,2}v_1+u_{2,4}u_{1,1,2}-u_{1,2,2}v[\,]+u_{1,2,6}-u_{1,4,4}, -u_{1,2}u_{2,2,4}+u_{1,4}u_{2,2,2}+u_{2,2}u_{1,2,4}+u_{2,2}v_2-u_{2,4}u_{1,2,2}+u_{2,2,2}v[\,]-u_{2,2,6}+u_{2,4,4}, -u_{1,2}v_{2,4}+u_{1,4}v_{2,2}+u_{2,2}v_{1,4}-u_{2,4}v_{1,2}+v[\,]v_{2,2}+v_2^2-v_{2,6}+v_{4,4}\} \quad \textbf{(2.7)}$$

> eq34 := map(coeffs, expand(ToJet(DGinfo(LieDerivative(V3a, V4a), "CoefficientSet"), {u(var), v(var)}, notation = jetnumbers)), {q})

$$eq34 := \{-u_{1,1}v_{2,2}+2u_{1,2}v_{1,2}-u_{2,2}v_{1,1}-v_{1,4}+v_{2,3}, u_{1,1}u_{1,2,2}-2u_{1,2}u_{1,1,2}+u_{2,2}u_{1,1,1}+u_{1,1,4}-u_{1,2,3}-v_1, -u_{1,1}u_{2,2,2}+2u_{1,2}u_{1,2,2}-u_{2,2}u_{1,1,2}-u_{1,2,4}+u_{2,2,3}+v_2, -u_{1,3}v_{2,4}+u_{1,4}v_{2,3}+u_{2,3}v_{1,4}-u_{2,4}v_{1,3}-v[\,]v_{1,4}+v[\,]v_{2,3}-v_1v_4+v_2v_3-v_{3,6}+v_{4,5}, -u_{1,1}v_{2,4}+u_{1,2}v_{1,4}+u_{1,2}v_{2,3}-u_{1,3}v_{2,2}+u_{1,4}v_{1,2}-u_{2,2}v_{1,3}+u_{2,3}v_{1,2}-u_{2,4}v_{1,1}-v_{1,6}+v_{2,5}, u_{1,1}u_{1,2,4}+2u_{1,1}v_2-u_{1,2}u_{1,1,4}-u_{1,2}u_{1,2,3}-2u_{1,2}v_1+u_{1,3}u_{1,2,2}-u_{1,4}u_{1,1,2}+u_{2,2}u_{1,1,3}-u_{2,3}u_{1,1,2}+u_{2,4}u_{1,1,1}+u_{1,1,6}-u_{1,2,5}-2v_3, -u_{1,1}u_{2,2,4}+u_{1,2}u_{1,2,4}+u_{1,2}u_{2,2,3}-2u_{1,2}v_2-u_{1,3}u_{2,2,2}+u_{1,4}u_{1,2,2}-u_{2,2}u_{1,2,3}+2u_{2,2}v_1+u_{2,3}u_{1,2,2}-u_{2,4}u_{1,1,2}-u_{1,2,6}+u_{2,2,5}+2v_4, u_{1,1}v_4-u_{1,2}v_3+u_{1,3}u_{1,2,4}+u_{1,3}v_2-u_{1,4}u_{1,2,3}-u_{2,3}u_{1,1,4}-u_{2,3}v_1+u_{2,4}u_{1,1,3}$$

$+ u_{1,1,4} v[\ ] - u_{1,2,3} v[\ ] + v[\ ] v_1 + u_{1,3,6} - u_{1,4,5} - v_5, -u_{1,2} v_4 - u_{1,3} u_{2,2,4} + u_{1,4} u_{2,2,3} - u_{1,4} v_2 + u_{2,2} v_3 + u_{2,3} u_{1,2,4} - u_{2,4} u_{1,2,3} + u_{2,4} v_1 - u_{1,2,4} v[\ ] + u_{2,2,3} v[\ ] - v[\ ] v_2 - u_{2,3,6} + u_{2,4,5} + v_6\}$

> $EQ2b := \{u_{1,1} u_{2,4} - u_{1,2} u_{1,4} - u_{1,2} v[\ ] + u_{1,6} - u_{3,4} - w_{[\ ]}, u_{1,2} u_{2,4} - u_{1,4} u_{2,2} - u_{2,2} v[\ ] + u_{2,6} - u_{4,4}, -u_{1,1} v_{2,4} + u_{1,2} v_{1,4} + u_{1,4} v_{1,2} - u_{2,4} v_{1,1} + v[\ ] v_{1,2} + v_1 v_2 - v_{1,6} + v_{3,4}, -u_{1,2} v_{2,4} + u_{1,4} v_{2,2} + u_{2,2} v_{1,4} - u_{2,4} v_{1,2} + v[\ ] v_{2,2} + v_2^2 - v_{2,6} + v_{4,4}, -u_{1,3} v_{2,4} + u_{1,4} v_{2,3} + u_{2,3} v_{1,4} - u_{2,4} v_{1,3} - v[\ ] v_{1,4} + v[\ ] v_{2,3} - v_1 v_4 + v_2 v_3 - v_{3,6} + v_{4,5}, u_{1,3} u_{2,4} - u_{1,4} u_{2,3} + u_{1,4} v[\ ] - u_{2,3} v[\ ] + \frac{1}{2} v[\ ]^2 + u_{3,6} - u_{4,5} - z_{[\ ]}\}$

$$EQ2b := \left\{ u_{1,3} u_{2,4} - u_{1,4} u_{2,3} + u_{1,4} v[\ ] - u_{2,3} v[\ ] + \frac{1}{2} v[\ ]^2 + u_{3,6} - u_{4,5} - z[\ ], u_{1,2} u_{2,4} - u_{1,4} u_{2,2} - u_{2,2} v[\ ] + u_{2,6} - u_{4,4}, u_{1,1} u_{2,4} - u_{1,2} u_{1,4} - u_{1,2} v[\ ] + u_{1,6} - u_{3,4} - w[\ ], -u_{1,2} v_{2,4} + u_{1,4} v_{2,2} + u_{2,2} v_{1,4} - u_{2,4} v_{1,2} + v[\ ] v_{2,2} + v_2^2 - v_{2,6} + v_{4,4}, -u_{1,1} v_{2,4} + u_{1,2} v_{1,4} + u_{1,4} v_{1,2} - u_{2,4} v_{1,1} + v[\ ] v_{1,2} + v_1 v_2 - v_{1,6} + v_{3,4}, -u_{1,3} v_{2,4} + u_{1,4} v_{2,3} + u_{2,3} v_{1,4} - u_{2,4} v_{1,3} - v[\ ] v_{1,4} + v[\ ] v_{2,3} - v_1 v_4 + v_2 v_3 - v_{3,6} + v_{4,5} \right\} \tag{2.9}$$

> # where $\{z_1 = v_5 - u_{1,1} v_4 + u_{1,2} v_3 - u_{1,3} v_2 + u_{1,4} v_1, z_2 = v_6 - u_{1,2} v_4 + u_{2,2} v_3 - u_{2,3} v_2 + u_{2,4} v_1\}$

>

> # *slv123* :=*solve*(*eq12* **union** *eq13* **union** *eq23*[4 ..6], $\{u_{1,1}, u_{1,2}, u_{2,2}, v_{1,1}, v_{1,2}, v_{2,2}\}$) : *simplify*(*eval*(*eq23*[1 ..6], *slv123*))

> # *slv1234* :=*solve*(*eq12* **union** *eq13* **union** *eq23* **union** *eq14* **union** *eq24* **union** *eq34*, $\{u_{1,1}, u_{1,2}, u_{2,2}, u_{1,3}, u_{2,3}, u_{3,4}, v_{1,1}, v_{1,2}, v_{2,2}, v_{1,3}, v_{2,3}, v_{3,4}, w_{1,1}, w_{1,2}, w_{2,2}, w_{1,3}, w_{2,3}, w_{3,4}\}$) :

> # *Sss* :={ } :**for** *i* **to** *nops*(*slv1234*) **do if** *lsh*(*slv1234*[*i*]) = *rhs*(*slv1234*[*i*]) **then** *Sss* := *Sss* **union** {*lhs*(*slv1234*[*i*])} :**fi**:**od**: *Sss*

>

>

# Second heavenly equation hierarchy

> *var* := *x*, *y*, *t1*, *t2*, *t3*, *t4*, *t5*, *t6* : *DGsetup*([*var*], *M8p*) :

dimensions 4 to 6

> *V1* := *evalDG*(*D_t1* + *diff*(*u*(*var*), *x*, *y*) *D_x* − *diff*(*u*(*var*), *x*, *x*) *D_y* − *q D_x*) :
*V2* := *evalDG*(*D_t2* + *diff*(*u*(*var*), *y*, *y*) *D_x* − *diff*(*u*(*var*), *x*, *y*) *D_y* − *q D_y*) :

> *eq12* := *ToJet*(*DGinfo*(*LieDerivative*(*V1*, *V2*), "CoefficientSet"), {*u*(*var*)}, *notation* =*jetnumbers*)

(3.1)

$$eq12 := \{u_{1,1}\,u_{1,2,2} - 2\,u_{1,2}\,u_{1,1,2} + u_{2,2}\,u_{1,1,1} + u_{1,1,4} - u_{1,2,3}, -u_{1,1}\,u_{2,2,2} + 2\,u_{1,2}\,u_{1,2,2} - u_{2,2}\,u_{1,1,2} - u_{1,2,4} + u_{2,2,3}\} \quad \textbf{(3.1)}$$

```
> V3 := evalDG(D_t3 + diff(u(var), y, t1) D_x - diff(u(var), x, t1) D_y - q D_t1) :
  V4 := evalDG(D_t4 + diff(u(var), y, t2) D_x - diff(u(var), x, t2) D_y - q D_t2) :
> V3a := evalDG(V3 + q V1) : V4a := evalDG(V4 + q V2) :
> eq13 := ToJet(DGinfo(LieDerivative(V1, V3a), "CoefficientSet"), {u(var)}, notation
      =jetnumbers);
  eq23 := map(coeffs, ToJet(DGinfo(LieDerivative(V2, V3a), "CoefficientSet"), {u(var)},
      notation =jetnumbers), {q})
```

$$eq13 := \{u_{1,1}\,u_{1,2,3} - u_{1,2}\,u_{1,1,3} - u_{1,3}\,u_{1,1,2} + u_{2,3}\,u_{1,1,1} + u_{1,1,5} - u_{1,3,3}, -u_{1,1}\,u_{2,2,3} + u_{1,2}\,u_{1,2,3} + u_{1,3}\,u_{1,2,2} - u_{2,3}\,u_{1,1,2} - u_{1,2,5} + u_{2,3,3}\}$$

$$eq23 := \{-u_{1,1}\,u_{1,2,2} + 2\,u_{1,2}\,u_{1,1,2} - u_{2,2}\,u_{1,1,1} - u_{1,1,4} + u_{1,2,3}, u_{1,1}\,u_{2,2,2} - 2\,u_{1,2}\,u_{1,2,2} + u_{2,2}\,u_{1,1,2} + u_{1,2,4} - u_{2,2,3}, u_{1,2}\,u_{1,2,3} - u_{1,3}\,u_{1,2,2} - u_{2,2}\,u_{1,1,3} + u_{2,3}\,u_{1,1,2} + u_{1,2,5} - u_{1,3,4}, -u_{1,2}\,u_{2,2,3} + u_{1,3}\,u_{2,2,2} + u_{2,2}\,u_{1,2,3} - u_{2,3}\,u_{1,2,2} - u_{2,2,5} + u_{2,3,4}\} \quad \textbf{(3.2)}$$

```
> EQ2a := {u_{1,1} u_{2,2} - u_{1,2}^2 + u_{1,4} - u_{2,3}, u_{1,1} u_{2,3} - u_{1,2} u_{1,3} + u_{1,5} - u_{3,3}, u_{1,2} u_{2,3}
      - u_{1,3} u_{2,2} + u_{2,5} - u_{3,4}}
```

$$EQ2a := \{u_{1,1}\,u_{2,2} - u_{1,2}^2 + u_{1,4} - u_{2,3}, u_{1,1}\,u_{2,3} - u_{1,2}\,u_{1,3} + u_{1,5} - u_{3,3}, u_{1,2}\,u_{2,3} - u_{1,3}\,u_{2,2} + u_{2,5} - u_{3,4}\} \quad \textbf{(3.3)}$$

```
> eq14 := map(coeffs, ToJet(DGinfo(LieDerivative(V1, V4a), "CoefficientSet"), {u(var)},
      notation =jetnumbers), {q});
  eq24 := ToJet(DGinfo(LieDerivative(V2, V4a), "CoefficientSet"), {u(var)}, notation
      =jetnumbers)
```

$$eq14 := \{u_{1,1}\,u_{1,2,2} - 2\,u_{1,2}\,u_{1,1,2} + u_{2,2}\,u_{1,1,1} + u_{1,1,4} - u_{1,2,3}, -u_{1,1}\,u_{2,2,2} + 2\,u_{1,2}\,u_{1,2,2} - u_{2,2}\,u_{1,1,2} - u_{1,2,4} + u_{2,2,3}, u_{1,1}\,u_{1,2,4} - u_{1,2}\,u_{1,1,4} - u_{1,4}\,u_{1,1,2} + u_{2,4}\,u_{1,1,1} + u_{1,1,6} - u_{1,3,4}, -u_{1,1}\,u_{2,2,4} + u_{1,2}\,u_{1,2,4} + u_{1,4}\,u_{1,2,2} - u_{2,4}\,u_{1,1,2} - u_{1,2,6} + u_{2,3,4}\}$$

$$eq24 := \{u_{1,2}\,u_{1,2,4} - u_{1,4}\,u_{1,2,2} - u_{2,2}\,u_{1,1,4} + u_{2,4}\,u_{1,1,2} + u_{1,2,6} - u_{1,4,4}, -u_{1,2}\,u_{2,2,4} + u_{1,4}\,u_{2,2,2} + u_{2,2}\,u_{1,2,4} - u_{2,4}\,u_{1,2,2} - u_{2,2,6} + u_{2,4,4}\} \quad \textbf{(3.4)}$$

```
> eq34 := map(coeffs, expand(ToJet(DGinfo(LieDerivative(V3a, V4a), "CoefficientSet"),
      {u(var)}, notation =jetnumbers)), {q})
```

$$eq34 := \{u_{1,1}\,u_{1,2,2} - 2\,u_{1,2}\,u_{1,1,2} + u_{2,2}\,u_{1,1,1} + u_{1,1,4} - u_{1,2,3}, -u_{1,1}\,u_{2,2,2} + 2\,u_{1,2}\,u_{1,2,2} - u_{2,2}\,u_{1,1,2} - u_{1,2,4} + u_{2,2,3}, u_{1,3}\,u_{1,2,4} - u_{1,4}\,u_{1,2,3} - u_{2,3}\,u_{1,1,4} + u_{2,4}\,u_{1,1,3} + u_{1,3,6} - u_{1,4,5}, -u_{1,3}\,u_{2,2,4} + u_{1,4}\,u_{2,2,3} + u_{2,3}\,u_{1,2,4} - u_{2,4}\,u_{1,2,3} - u_{2,3,6} + u_{2,4,5}, u_{1,1}\,u_{1,2,4} - u_{1,2}\,u_{1,1,4} - u_{1,2}\,u_{1,2,3} + u_{1,3}\,u_{1,2,2} - u_{1,4}\,u_{1,1,2} + u_{2,2}\,u_{1,1,3} - u_{2,3}\,u_{1,1,2} + u_{2,4}\,u_{1,1,1} + u_{1,1,6} - u_{1,2,5}, -u_{1,1}\,u_{2,2,4} + u_{1,2}\,u_{1,2,4} + u_{1,2}\,u_{2,2,3} - u_{1,3}\,u_{2,2,2} + u_{1,4}\,u_{1,2,2} - u_{2,2}\,u_{1,2,3} + u_{2,3}\,u_{1,2,2} - u_{2,4}\,u_{1,1,2} - u_{1,2,6} + u_{2,2,5}\} \quad \textbf{(3.5)}$$

```
> EQ2b := {u_{1,1} u_{2,4} - u_{1,2} u_{1,4} + u_{1,6} - u_{3,4}, u_{1,2} u_{2,4} - u_{1,4} u_{2,2} + u_{2,6} - u_{4,4}, u_{1,3} u_{2,4}
```

$-u_{1,4}\,u_{2,3}+u_{3,6}-u_{4,5}\}$

$$EQ2b := \{u_{1,1}\,u_{2,4}-u_{1,2}\,u_{1,4}+u_{1,6}-u_{3,4},\, u_{1,2}\,u_{2,4}-u_{1,4}\,u_{2,2}+u_{2,6}-u_{4,4},\, u_{1,3}\,u_{2,4} - u_{1,4}\,u_{2,3}+u_{3,6}-u_{4,5}\} \quad \textbf{(3.6)}$$

> $slv2ab := solve(EQ2a$ **union** $EQ2b, \{u_{1,3}, u_{1,4}, u_{1,5}, u_{1,6}, u_{2,5}, u_{2,6}\})$

$$slv2ab := \left\{u_{1,3} = -\frac{u_{1,1}\,u_{2,2}\,u_{2,3}-u_{1,2}^2\,u_{2,3}-u_{2,3}^2+u_{3,6}-u_{4,5}}{u_{2,4}},\, u_{1,4} = -u_{1,1}\,u_{2,2}+u_{1,2}^2 + u_{2,3},\, u_{1,5} = -\frac{1}{u_{2,4}}\left(u_{1,1}\,u_{1,2}\,u_{2,2}\,u_{2,3}-u_{1,2}^3\,u_{2,3}+u_{1,1}\,u_{2,3}\,u_{2,4}-u_{1,2}\,u_{2,3}^2+u_{1,2}\,u_{3,6} - u_{1,2}\,u_{4,5}-u_{3,3}\,u_{2,4}\right),\, u_{1,6} = -u_{1,1}\,u_{1,2}\,u_{2,2}+u_{1,2}^3-u_{1,1}\,u_{2,4}+u_{1,2}\,u_{2,3}+u_{3,4},\, u_{2,5} = -\frac{1}{u_{2,4}}\left(u_{1,1}\,u_{2,2}^2\,u_{2,3}-u_{1,2}^2\,u_{2,2}\,u_{2,3}+u_{1,2}\,u_{2,3}\,u_{2,4}-u_{2,2}\,u_{2,3}^2+u_{2,2}\,u_{3,6} - u_{2,2}\,u_{4,5}-u_{3,4}\,u_{2,4}\right),\, u_{2,6} = -u_{1,1}\,u_{2,2}^2+u_{1,2}^2\,u_{2,2}-u_{1,2}\,u_{2,4}+u_{2,2}\,u_{2,3}+u_{4,4}\right\} \quad \textbf{(3.7)}$$

```
> # Ss:={ } :for i to nops(slv1234) do if lhs(slv1234[i]) = rhs(slv1234[i]) then Ss := Ss
    union {lhs(slv1234[i])} :fi:od: nops(Ss)
```

## computing Char

> $smu := f \to add\left(add\left(diff\left(f, u_{i,j}\right) p_i\, p_j, j = i..8\right), i = 1..8\right)$ :

> $map(smu, EQ2a)$

$$\{u_{2,2}\,p_1^2-2\,u_{1,2}\,p_1\,p_2+u_{1,1}\,p_2^2+p_1\,p_4-p_2\,p_3,\, u_{2,3}\,p_1^2-u_{1,3}\,p_1\,p_2-u_{1,2}\,p_1\,p_3 + u_{1,1}\,p_2\,p_3+p_1\,p_5-p_3^2,\, -u_{2,2}\,u_{1,1,3}\,p_1\,p_3-u_{1,3}\,u_{1,1,3}\,p_2^2+u_{2,3}\,p_1\,p_2+u_{1,2}\,p_2\,p_3 + p_2\,p_5-p_3\,p_4\} \quad \textbf{(3.1.1)}$$

> $map(smu, EQ2b)$

$$\{u_{2,4}\,p_1\,p_2-u_{2,2}\,p_1\,p_4-u_{1,4}\,p_2^2+u_{1,2}\,p_2\,p_4+p_2\,p_6-p_4^2,\, u_{2,4}\,p_1^2-u_{1,4}\,p_1\,p_2 - u_{1,2}\,p_1\,p_4+u_{1,1}\,p_2\,p_4+p_1\,p_6-p_3\,p_4,\, u_{2,4}\,p_1\,p_3-u_{2,3}\,p_1\,p_4-u_{1,4}\,p_2\,p_3 + u_{1,3}\,p_2\,p_4+p_3\,p_6-p_4\,p_5\} \quad \textbf{(3.1.2)}$$

## compatibility

> $DGsetup([x, y, t1, t2, t3], [u, v, w], M5J, 5)$ :

> $eq12$ **union** $eq13$ **union** $eq23[4..6]$; $nops(\%)$

$\{u_1 w_{2,2} - u_2 w_{1,2} + v_1 w_{1,2} - v_2 w_{1,1} - w_{1,4} + w_{2,3}, u_1 u_{2,2} - u_2 u_{1,2} - u_{1,1} v_2 + u_{1,2} v_1 - u_{1,4} + u_{2,3} - w_1, u_1 v_{2,2} - u_2 v_{1,2} + v_1 v_{1,2} - v_2 v_{1,1} - v_{1,4} + v_{2,3} + w_2, u_1 u_{2,3} + u_1 w_1 - u_3 u_{1,2} - u_{1,1} v_3 + u_{1,1} w[\,] + u_{1,3} v_1 - u_{1,5} + u_{3,3}, u_1 v_{2,3} - u_1 w_2 - u_3 v_{1,2} + v_1 v_{1,3} - v_3 v_{1,1} + v_{1,1} w[\,] - v_{1,5} + v_{3,3}, u_1 w_{2,3} - u_3 w_{1,2} + v_1 w_{1,3} - v_3 w_{1,1} + w[\,] w_{1,1} + w_1^2 - w_{1,5} + w_{3,3}, u_2 w_{2,3} - u_3 w_{2,2} + v_2 w_{1,3} - v_3 w_{1,2} + w[\,] w_{1,2} + w_1 w_2 - w_{2,5} + w_{3,4}, u_1 w_2 + u_2 u_{2,3} - u_3 u_{2,2} - u_{1,2} v_3 + u_{1,2} w[\,] + u_{1,3} v_2 - u_{2,5} + u_{3,4} + w_3, u_2 v_{2,3} - u_2 w_2 - u_3 v_{2,2} + v_1 w_2 + v_2 v_{1,3} - v_2 w_1 - v_3 v_{1,2} + v_{1,2} w[\,] - v_{2,5} + v_{3,4} - w_4\}$

9 **(3.2.1)**

```
> eq5u := {u[1] u[2,2] - u[2] u[1,2] - u[1,1] v[2] + u[1,2] v[1] - u[1,4] + u[2,3] - w[1], u[1] u[2,3] + u[1] w[1]
      - u[3] u[1,2] - u[1,1] v[3] + u[1,1] w[ ] + u[1,3] v[1] - u[1,5] + u[3,3], u[1] w[2] + u[2] u[2,3] - u[3] u[2,2]
      - u[1,2] v[3] + u[1,2] w[ ] + u[1,3] v[2] - u[2,5] + u[3,4] + w[3]} :
  eq5v := {u[1] v[2,2] - u[2] v[1,2] + v[1] v[1,2] - v[2] v[1,1] - v[1,4] + v[2,3] + w[2], u[1] v[2,3] - u[1] w[2] - u[3] v[1,2]
      + v[1] v[1,3] - v[3] v[1,1] + v[1,1] w[ ] - v[1,5] + v[3,3], u[2] v[2,3] - u[2] w[2] - u[3] v[2,2] + v[1] w[2]
      + v[2] v[1,3] - v[2] w[1] - v[3] v[1,2] + v[1,2] w[ ] - v[2,5] + v[3,4] - w[4]} :
  eq5w := {u[1] w[2,2] - u[2] w[1,2] + v[1] w[1,2] - v[2] w[1,1] - w[1,4] + w[2,3], u[1] w[2,3] - u[3] w[1,2] + v[1] w[1,3]
      - v[3] w[1,1] + w[ ] w[1,1] + w[1]^2 - w[1,5] + w[3,3], u[2] w[2,3] - u[3] w[2,2] + v[2] w[1,3] - v[3] w[1,2]
      + w[ ] w[1,2] + w[1] w[2] - w[2,5] + w[3,4]} :
> sl2u := solve(eq5u, {u[1,4], u[1,5], u[2,5]}) : sl2v := solve(eq5v, {v[1,4], v[1,5], v[2,5]}) : sl2w :=
      solve(eq5w, {w[1,4], w[1,5], w[2,5]}) : sl2 := sl2u union sl2v union sl2w :
> jet2 := {seq(seq(u[i,j], j = i..5), i = 1..5), seq(seq(v[i,j], j = i..5), i = 1..5), seq(seq(w[i,j], j
      = i..5), i = 1..5)} :
  jet3 := {seq(seq(seq(u[i,j,k], k = j..5), j = i..5), i = 1..5), seq(seq(seq(v[i,j,k], k = j..5), j = i
      ..5), i = 1..5), seq(seq(seq(w[i,j,k], k = j..5), j = i..5), i = 1..5)} :
> # for k to nops(eq5w) do: S2 := { } :for i to nops(jet2) do if diff(eq5w[k], jet2[i]) ≠ 0
      then S2 := S2 union {jet2[i]} :fi:od: print(S2);od:
> eliminate(eval({seq(seq(TotalDiff(eq5u[i], j), j = 1..5), i = 1..nops(eq5u))}, sl2),
      {u[1,1,4], u[1,2,4], u[1,3,4], u[1,4,4], u[1,4,5], u[1,1,5], u[1,2,5], u[1,3,5], u[1,5,5], u[2,2,5], u[2,3,5], u[2,4,5],
      u[2,5,5]})[2],
  eliminate(eval({seq(seq(TotalDiff(eq5v[i], j), j = 1..5), i = 1..nops(eq5v))}, sl2),
      {v[1,1,4], v[1,2,4], v[1,3,4], v[1,4,4], v[1,4,5], v[1,1,5], v[1,2,5], v[1,3,5], v[1,5,5], v[2,2,5], v[2,3,5], v[2,4,5], v[2,5,5]})
      [2],
  eliminate(eval({seq(seq(TotalDiff(eq5w[i], j), j = 1..5), i = 1..nops(eq5w))}, sl2),
      {w[1,1,4], w[1,2,4], w[1,3,4], w[1,4,4], w[1,4,5], w[1,1,5], w[1,2,5], w[1,3,5], w[1,5,5], w[2,2,5], w[2,3,5], w[2,4,5],
      w[2,5,5]})[2]
```

$\emptyset, \emptyset, \emptyset$ **(3.2.2)**

```
> DGsetup([x, y, t1, t2, t3, t4], [u, v, w], M5J, 5) :
```

> *eq12* **union** *eq13* **union** *eq23*[4..6] **union** *eq14*[4..6] **union** *eq24* **union** *eq34*[4..4] **union** *eq34*[6..7]; *nops*(%)

$$\{u_1 w_{2,2} - u_2 w_{1,2} + v_1 w_{1,2} - v_2 w_{1,1} - w_{1,4} + w_{2,3}, u_1 u_{2,2} - u_2 u_{1,2} - u_{1,1} v_2 + u_{1,2} v_1 - u_{1,4} + u_{2,3} - w_1, u_1 v_{2,2} - u_2 v_{1,2} + v_1 v_{1,2} - v_2 v_{1,1} - v_{1,4} + v_{2,3} + w_2, u_1 u_{2,3} + u_1 w_1 - u_3 u_{1,2} - u_{1,1} v_3 + u_{1,1} w[\,] + u_{1,3} v_1 - u_{1,5} + u_{3,3}, u_1 v_{2,3} - u_1 w_2 - u_3 v_{1,2} + v_1 v_{1,3} - v_3 v_{1,1} + v_{1,1} w[\,] - v_{1,5} + v_{3,3}, u_1 w_{2,3} - u_3 w_{1,2} + v_1 w_{1,3} - v_3 w_{1,1} + w[\,] w_{1,1} + w_1^2 - w_{1,5} + w_{3,3}, u_2 u_{2,4} - u_4 u_{2,2} - u_{1,2} v_4 + u_{1,4} v_2 + u_{2,2} w[\,] - v_2 w_1 - u_{2,6} + u_{4,4}, u_2 v_{2,4} - u_4 v_{2,2} + v_2 v_{1,4} + v_2 w_2 - v_4 v_{1,2} + v_{2,2} w[\,] - v_{2,6} + v_{4,4}, w_{2,4} u_2 - u_4 w_{2,2} + v_2 w_{1,4} - v_4 w_{1,2} + w[\,] w_{2,2} + w_2^2 - w_{2,6} + w_{4,4}, u_1 w_{2,4} - u_4 w_{1,2} + v_1 w_{1,4} - v_4 w_{1,1} + w[\,] w_{1,2} + w_1 w_2 - w_{1,6} + w_{3,4}, u_2 w_{2,3} - u_3 w_{2,2} + v_2 w_{1,3} - v_3 w_{1,2} + w[\,] w_{1,2} + w_1 w_2 - w_{2,5} + w_{3,4}, u_1 w_2 + u_2 u_{2,3} - u_3 u_{2,2} - u_{1,2} v_3 + u_{1,2} w[\,] + u_{1,3} v_2 - u_{2,5} + u_{3,4} + w_3, u_1 v_{2,4} - u_4 v_{1,2} + v_1 v_{1,4} + v_2 w_1 - v_4 v_{1,1} + v_{1,2} w[\,] - v_{1,6} + v_{3,4} + w_4, u_3 w_{2,4} - u_4 w_{2,3} + v_3 w_{1,4} - v_4 w_{1,3} - w[\,] w_{1,4} + w[\,] w_{2,3} - w_1 w_4 + w_2 w_3 - w_{3,6} + w_{4,5}, u_1 u_{2,4} - u_1 w_2 + u_2 w_1 - u_4 u_{1,2} - u_{1,1} v_4 + u_{1,2} w[\,] + u_{1,4} v_1 - v_1 w_1 - u_{1,6} + u_{3,4} - w_3, u_2 v_{2,3} - u_2 w_2 - u_3 v_{2,2} + v_1 w_2 + v_2 v_{1,3} - v_2 w_1 - v_3 v_{1,2} + v_{1,2} w[\,] - v_{2,5} + v_{3,4} - w_4, -u_1 w_4 + u_2 w_3 + u_3 u_{2,4} - u_3 w_2 - u_4 u_{2,3} - u_{1,3} v_4 + u_{1,4} v_3 - u_{1,4} w[\,] + u_{2,3} w[\,] - v_3 w_1 + w[\,] w_1 - u_{3,6} + u_{4,5} - w_5, u_3 v_{2,4} - u_4 v_{2,3} + u_4 w_2 - v_1 w_4 + v_2 w_3 + v_3 v_{1,4} - v_4 v_{1,3} + v_4 w_1 - v_{1,4} w[\,] + v_{2,3} w[\,] - w[\,] w_2 - v_{3,6} + v_{4,5} + w_6\}$$

$$18 \qquad \textbf{(3.2.3)}$$

> $eq6u := \{u_1 u_{2,2} - u_2 u_{1,2} - u_{1,1} v_2 + u_{1,2} v_1 - u_{1,4} + u_{2,3} - w_1, u_1 u_{2,3} + u_1 w_1 - u_3 u_{1,2} - u_{1,1} v_3 + u_{1,1} w[\,] + u_{1,3} v_1 - u_{1,5} + u_{3,3}, u_1 w_2 + u_2 u_{2,3} - u_3 u_{2,2} - u_{1,2} v_3 + u_{1,2} w[\,] + u_{1,3} v_2 - u_{2,5} + u_{3,4} + w_3, u_2 u_{2,4} - u_4 u_{2,2} - u_{1,2} v_4 + u_{1,4} v_2 + u_{2,2} w[\,] - v_2 w_1 - u_{2,6} + u_{4,4}, u_1 u_{2,4} - u_1 w_2 + u_2 w_1 - u_4 u_{1,2} - u_{1,1} v_4 + u_{1,2} w[\,] + u_{1,4} v_1 - v_1 w_1 - u_{1,6} + u_{3,4} - w_3, -u_1 w_4 + u_2 w_3 + u_3 u_{2,4} - u_3 w_2 - u_4 u_{2,3} - u_{1,3} v_4 + u_{1,4} v_3 - u_{1,4} w[\,] + u_{2,3} w[\,] - v_3 w_1 + w[\,] w_1 - u_{3,6} + u_{4,5} - w_5\}:$

$eq6v := \{u_1 v_{2,2} - u_2 v_{1,2} + v_1 v_{1,2} - v_2 v_{1,1} - v_{1,4} + v_{2,3} + w_2, u_1 v_{2,3} - u_1 w_2 - u_3 v_{1,2} + v_1 v_{1,3} - v_3 v_{1,1} + v_{1,1} w[\,] - v_{1,5} + v_{3,3}, u_2 v_{2,3} - u_2 w_2 - u_3 v_{2,2} + v_1 w_2 + v_2 v_{1,3} - v_2 w_1 - v_3 v_{1,2} + v_{1,2} w[\,] - v_{2,5} + v_{3,4} - w_4, u_2 v_{2,4} - u_4 v_{2,2} + v_2 v_{1,4} + v_2 w_2 - v_4 v_{1,2} + v_{2,2} w[\,] - v_{2,6} + v_{4,4}, u_1 v_{2,4} - u_4 v_{1,2} + v_1 v_{1,4} + v_2 w_1 - v_4 v_{1,1} + v_{1,2} w[\,] - v_{1,6} + v_{3,4} + w_4, u_3 v_{2,4} - u_4 v_{2,3} + u_4 w_2 - v_1 w_4 + v_2 w_3 + v_3 v_{1,4} - v_4 v_{1,3} + v_4 w_1 - v_{1,4} w[\,] + v_{2,3} w[\,] - w[\,] w_2 - v_{3,6} + v_{4,5} + w_6\}:$

$eq6w := \{u_1 w_{2,2} - u_2 w_{1,2} + v_1 w_{1,2} - v_2 w_{1,1} - w_{1,4} + w_{2,3}, u_1 w_{2,3} - u_3 w_{1,2} + v_1 w_{1,3}$

$- v_3 w_{1,1} + w[\ ] w_{1,1} + w_1^2 - w_{1,5} + w_{3,3}, u_2 w_{2,3} - u_3 w_{2,2} + v_2 w_{1,3} - v_3 w_{1,2} + w[\ ] w_{1,2} + w_1 w_2 - w_{2,5} + w_{3,4}, w_{2,4} u_2 - u_4 w_{2,2} + v_2 w_{1,4} - v_4 w_{1,2} + w[\ ] w_{2,2} + w_2^2 - w_{2,6} + w_{4,4}, u_1 w_{2,4} - u_4 w_{1,2} + v_1 w_{1,4} - v_4 w_{1,1} + w[\ ] w_{1,2} + w_1 w_2 - w_{1,6} + w_{3,4}, u_3 w_{2,4} - u_4 w_{2,3} + v_3 w_{1,4} - v_4 w_{1,3} - w[\ ] w_{1,4} + w[\ ] w_{2,3} - w_1 w_4 + w_2 w_3 - w_{3,6} + w_{4,5}\} :$

> $sl2u := solve(eq6u, \{u_{1,4}, u_{1,5}, u_{2,5}, u_{1,6}, u_{2,6}, u_{3,6}\}) : sl2v := solve(eq6v, \{v_{1,4}, v_{1,5}, v_{2,5}, v_{1,6}, v_{2,6}, v_{3,6}\}) : sl2w := solve(eq6w, \{w_{1,4}, w_{1,5}, w_{2,5}, w_{1,6}, w_{2,6}, w_{3,6}\}) :$
> $sl2 := sl2u$ **union** $sl2v$ **union** $sl2w$ :

> $jet2 := \{seq(seq(u_{i,j}, j = i..6), i = 1..6), seq(seq(v_{i,j}, j = i..6), i = 1..6), seq(seq(w_{i,j}, j = i..6), i = 1..6)\} :$
> $jet3 := \{seq(seq(seq(u_{i,j,k}, k = j..6), j = i..6), i = 1..6), seq(seq(seq(v_{i,j,k}, k = j..6), j = i..6), i = 1..6), seq(seq(seq(w_{i,j,k}, k = j..6), j = i..6), i = 1..6)\} :$

> *# for k to nops(eq6w)* **do**: *S2* := { } :**for** *i* **to** *nops(jet2)* **do if** $diff(eq6w[k], jet2[i]) \neq 0$ **then** *S2* := *S2* **union** {*jet2*[*i*]} :**fi**:**od**: *print(S2)*;**od**:

> $eliminate(eval(\{seq(seq(TotalDiff(eq5u[i], j), j = 1..6), i = 1..nops(eq5u))\}, sl2), \{u_{1,1,4}, u_{1,2,4}, u_{1,3,4}, u_{1,4,4}, u_{1,4,5}, u_{1,4,6}, u_{1,1,5}, u_{1,2,5}, u_{1,3,5}, u_{1,5,5}, u_{1,5,6}, u_{2,2,5}, u_{2,3,5}, u_{2,4,5}, u_{2,5,5}, u_{2,5,6}, u_{1,1,6}, u_{1,2,6}, u_{1,3,6}, u_{1,6,6}, u_{2,2,6}, u_{2,3,6}, u_{2,4,6}, u_{2,6,6}, u_{3,3,6}, u_{3,4,6}, u_{3,5,6}, u_{3,6,6}\})[2],$
> $eliminate(eval(\{seq(seq(TotalDiff(eq5v[i], j), j = 1..6), i = 1..nops(eq5v))\}, sl2), \{v_{1,1,4}, v_{1,2,4}, v_{1,3,4}, v_{1,4,4}, v_{1,4,5}, v_{1,4,6}, v_{1,1,5}, v_{1,2,5}, v_{1,3,5}, v_{1,5,5}, v_{1,5,6}, v_{2,2,5}, v_{2,3,5}, v_{2,4,5}, v_{2,5,5}, v_{2,5,6}, v_{1,1,6}, v_{1,2,6}, v_{1,3,6}, v_{1,6,6}, v_{2,2,6}, v_{2,3,6}, v_{2,4,6}, v_{2,6,6}, v_{3,3,6}, v_{3,4,6}, v_{3,5,6}, v_{3,6,6}\})[2],$
> $eliminate(eval(\{seq(seq(TotalDiff(eq5w[i], j), j = 1..6), i = 1..nops(eq5w))\}, sl2), \{w_{1,1,4}, w_{1,2,4}, w_{1,3,4}, w_{1,4,4}, w_{1,4,5}, w_{1,4,6}, w_{1,1,5}, w_{1,2,5}, w_{1,3,5}, w_{1,5,5}, w_{1,5,6}, w_{2,2,5}, w_{2,3,5}, w_{2,4,5}, w_{2,5,5}, u_{2,5,6}, w_{1,1,6}, w_{1,2,6}, w_{1,3,6}, w_{1,6,6}, w_{2,2,6}, w_{2,3,6}, w_{2,4,6}, w_{2,6,6}, w_{3,3,6}, w_{3,4,6}, w_{3,5,6}, w_{3,6,6}\})[2]$

$$\emptyset, \emptyset, \emptyset \quad (3.2.4)$$

>

> *ChangeFrame(M6p)* :

higher dimensions up to 8

> $ToJet(V1, \{u(var)\}); ToJet(V2, \{u(var)\}); ToJet(V3, \{u(var)\}); ToJet(V4, \{u(var)\})$

$$-(q - u_{x,y})\, D\_x - u_{x,x}\, D\_y + D\_t1$$
$$u_{y,y}\, D\_x - (q + u_{x,y})\, D\_y + D\_t2$$
$$u_{y,t1}\, D\_x - u_{x,t1}\, D\_y - q\, D\_t1 + D\_t3$$
$$u_{y,t2}\, D\_x - u_{x,t2}\, D\_y - q\, D\_t2 + D\_t4 \quad (3.8)$$

> $ToJet(V3a, \{u(var)\}); ToJet(V4a, \{u(var)\})$

$$-(q^2 - q\, u_{x,y} - u_{y,t1})\, D\_x - (q\, u_{x,x} + u_{x,t1})\, D\_y + D\_t3$$
$$(q\, u_{y,y} + u_{y,t2})\, D\_x - (q^2 + q\, u_{x,y} + u_{x,t2})\, D\_y + D\_t4 \quad (3.9)$$

```
> V5 := evalDG(D_t5 + diff(u(var), y, t3) D_x − diff(u(var), x, t3) D_y − q D_t3) :
  V6 := evalDG(D_t6 + diff(u(var), y, t4) D_x − diff(u(var), x, t4) D_y − q D_t4) :
> ToJet(V5, {u(var)}); ToJet(V6, {u(var)})
```

$$u_{y,t3}\,D\_x - u_{x,t3}\,D\_y - q\,D\_t3 + D\_t5$$
$$u_{y,t4}\,D\_x - u_{x,t4}\,D\_y - q\,D\_t4 + D\_t6 \qquad \textbf{(3.10)}$$

```
> V5a := evalDG(V5 + q V3a) : V6a := evalDG(V6 + q V4a) :
> ToJet(V5a, {u(var)}); ToJet(V6a, {u(var)})
```

$$-\left(q^3 - u_{x,y}\,q^2 - u_{y,t1}\,q - u_{y,t3}\right) D\_x - \left(u_{x,x}\,q^2 + u_{x,t1}\,q + u_{x,t3}\right) D\_y + D\_t5$$
$$\left(u_{y,y}\,q^2 + u_{y,t2}\,q + u_{y,t4}\right) D\_x - \left(q^3 + u_{x,y}\,q^2 + u_{x,t2}\,q + u_{x,t4}\right) D\_y + D\_t6 \qquad \textbf{(3.11)}$$

```
> eq15 := map(coeffs, expand(ToJet(DGinfo(LieDerivative(V1, V5a), "CoefficientSet"),
      {u(var)}, notation = jetnumbers)), {q});
  eq25 := map(coeffs, expand(ToJet(DGinfo(LieDerivative(V2, V5a), "CoefficientSet"),
      {u(var)}, notation = jetnumbers)), {q})
```

$$eq15 := \{u_{1,1}\,u_{1,2,3} - u_{1,2}\,u_{1,1,3} - u_{1,3}\,u_{1,1,2} + u_{2,3}\,u_{1,1,1} + u_{1,1,5} - u_{1,3,3}, -u_{1,1}\,u_{2,2,3} + u_{1,2}\,u_{1,2,3} + u_{1,3}\,u_{1,2,2} - u_{2,3}\,u_{1,1,2} - u_{1,2,5} + u_{2,3,3}, u_{1,1}\,u_{1,2,5} - u_{1,2}\,u_{1,1,5} - u_{1,5}\,u_{1,1,2} + u_{2,5}\,u_{1,1,1} + u_{1,1,7} - u_{1,3,5}, -u_{1,1}\,u_{2,2,5} + u_{1,2}\,u_{1,2,5} + u_{1,5}\,u_{1,2,2} - u_{2,5}\,u_{1,1,2} - u_{1,2,7} + u_{2,3,5}\}$$

$$eq25 := \{-u_{1,1}\,u_{1,2,2} + 2\,u_{1,2}\,u_{1,1,2} - u_{2,2}\,u_{1,1,1} - u_{1,1,4} + u_{1,2,3}, u_{1,1}\,u_{2,2,2} - 2\,u_{1,2}\,u_{1,2,2} + u_{2,2}\,u_{1,1,2} + u_{1,2,4} - u_{2,2,3}, u_{1,2}\,u_{1,2,3} - u_{1,3}\,u_{1,2,2} - u_{2,2}\,u_{1,1,3} + u_{2,3}\,u_{1,1,2} + u_{1,2,5} - u_{1,3,4}, -u_{1,2}\,u_{2,2,3} + u_{1,3}\,u_{2,2,2} + u_{2,2}\,u_{1,2,3} - u_{2,3}\,u_{1,2,2} - u_{2,2,5} + u_{2,3,4}, u_{1,2}\,u_{1,2,5} - u_{1,5}\,u_{1,2,2} - u_{2,2}\,u_{1,1,5} + u_{2,5}\,u_{1,1,2} + u_{1,2,7} - u_{1,4,5}, -u_{1,2}\,u_{2,2,5} + u_{1,5}\,u_{2,2,2} + u_{2,2}\,u_{1,2,5} - u_{2,5}\,u_{1,2,2} - u_{2,2,7} + u_{2,4,5}\} \qquad \textbf{(3.12)}$$

```
> eq16 := map(coeffs, expand(ToJet(DGinfo(LieDerivative(V1, V6a), "CoefficientSet"),
      {u(var)}, notation = jetnumbers)), {q});
  eq26 := map(coeffs, expand(ToJet(DGinfo(LieDerivative(V2, V6a), "CoefficientSet"),
      {u(var)}, notation = jetnumbers)), {q})
```

$$eq16 := \{u_{1,1}\,u_{1,2,2} - 2\,u_{1,2}\,u_{1,1,2} + u_{2,2}\,u_{1,1,1} + u_{1,1,4} - u_{1,2,3}, -u_{1,1}\,u_{2,2,2} + 2\,u_{1,2}\,u_{1,2,2} - u_{2,2}\,u_{1,1,2} - u_{1,2,4} + u_{2,2,3}, u_{1,1}\,u_{1,2,4} - u_{1,2}\,u_{1,1,4} - u_{1,4}\,u_{1,1,2} + u_{2,4}\,u_{1,1,1} + u_{1,1,6} - u_{1,3,4}, -u_{1,1}\,u_{2,2,4} + u_{1,2}\,u_{1,2,4} + u_{1,4}\,u_{1,2,2} - u_{2,4}\,u_{1,1,2} - u_{1,2,6} + u_{2,3,4}, u_{1,1}\,u_{1,2,6} - u_{1,2}\,u_{1,1,6} - u_{1,6}\,u_{1,1,2} + u_{2,6}\,u_{1,1,1} + u_{1,1,8} - u_{1,3,6}, -u_{1,1}\,u_{2,2,6} + u_{1,2}\,u_{1,2,6} + u_{1,6}\,u_{1,2,2} - u_{2,6}\,u_{1,1,2} - u_{1,2,8} + u_{2,3,6}\}$$

$$eq26 := \{u_{1,2}\,u_{1,2,4} - u_{1,4}\,u_{1,2,2} - u_{2,2}\,u_{1,1,4} + u_{2,4}\,u_{1,1,2} + u_{1,2,6} - u_{1,4,4}, -u_{1,2}\,u_{2,2,4} + u_{1,4}\,u_{2,2,2} + u_{2,2}\,u_{1,2,4} - u_{2,4}\,u_{1,2,2} - u_{2,2,6} + u_{2,4,4}, u_{1,2}\,u_{1,2,6} - u_{1,6}\,u_{1,2,2} - u_{2,2}\,u_{1,1,6} + u_{2,6}\,u_{1,1,2} + u_{1,2,8} - u_{1,4,6}, -u_{1,2}\,u_{2,2,6} + u_{1,6}\,u_{2,2,2} + u_{2,2}\,u_{1,2,6} - u_{2,6}\,u_{1,2,2} - u_{2,2,8} + u_{2,4,6}\} \qquad \textbf{(3.13)}$$

```
> eq35 := map(coeffs, expand(ToJet(DGinfo(LieDerivative(V3a, V5a), "CoefficientSet"),
```

$\{u(var)\}, notation = jetnumbers)), \{q\});$

$eq45 := map(coeffs, expand(ToJet(DGinfo(LieDerivative(V4a, V5a), "CoefficientSet"), \{u(var)\}, notation = jetnumbers)), \{q\})$

$$eq35 := \{u_{1,1} u_{1,2,5} - u_{1,2} u_{1,1,5} - u_{1,5} u_{1,1,2} + u_{2,5} u_{1,1,1} + u_{1,1,7} - u_{1,3,5}, -u_{1,1} u_{2,2,5} + u_{1,2} u_{1,2,5} + u_{1,5} u_{1,2,2} - u_{2,5} u_{1,1,2} - u_{1,2,7} + u_{2,3,5}, u_{1,3} u_{1,2,5} - u_{1,5} u_{1,2,3} - u_{2,3} u_{1,1,5} + u_{2,5} u_{1,1,3} + u_{1,3,7} - u_{1,5,5}, -u_{1,3} u_{2,2,5} + u_{1,5} u_{2,2,3} + u_{2,3} u_{1,2,5} - u_{2,5} u_{1,2,3} - u_{2,3,7} + u_{2,5,5}\}$$

$$eq45 := \{-u_{1,1} u_{1,2,2} + 2 u_{1,2} u_{1,1,2} - u_{2,2} u_{1,1,1} - u_{1,1,4} + u_{1,2,3}, u_{1,1} u_{2,2,2} - 2 u_{1,2} u_{1,2,2} + u_{2,2} u_{1,1,2} + u_{1,2,4} - u_{2,2,3}, u_{1,4} u_{1,2,5} - u_{1,5} u_{1,2,4} - u_{2,4} u_{1,1,5} + u_{2,5} u_{1,1,4} + u_{1,4,7} - u_{1,5,6}, -u_{1,4} u_{2,2,5} + u_{1,5} u_{2,2,4} + u_{2,4} u_{1,2,5} - u_{2,5} u_{1,2,4} - u_{2,4,7} + u_{2,5,6}, -u_{1,1} u_{1,2,4} + u_{1,2} u_{1,1,4} + u_{1,2} u_{1,2,3} - u_{1,3} u_{1,2,2} + u_{1,4} u_{1,1,2} - u_{2,2} u_{1,1,3} + u_{2,3} u_{1,1,2} - u_{2,4} u_{1,1,1} - u_{1,1,6} + u_{1,2,5}, u_{1,1} u_{2,2,4} - u_{1,2} u_{1,2,4} - u_{1,2} u_{2,2,3} + u_{1,3} u_{2,2,2} - u_{1,4} u_{1,2,2} + u_{2,2} u_{1,2,3} - u_{2,3} u_{1,2,2} + u_{2,4} u_{1,1,2} + u_{1,2,6} - u_{2,2,5}, u_{1,2} u_{1,2,5} - u_{1,3} u_{1,2,4} + u_{1,4} u_{1,2,3} - u_{1,5} u_{1,2,2} - u_{2,2} u_{1,1,5} + u_{2,3} u_{1,1,4} - u_{2,4} u_{1,1,3} + u_{2,5} u_{1,1,2} + u_{1,2,7} - u_{1,3,6}, -u_{1,2} u_{2,2,5} + u_{1,3} u_{2,2,4} - u_{1,4} u_{2,2,3} + u_{1,5} u_{2,2,2} + u_{2,2} u_{1,2,5} - u_{2,3} u_{1,2,4} + u_{2,4} u_{1,2,3} - u_{2,5} u_{1,2,2} - u_{2,2,7} + u_{2,3,6}\} \quad (3.14)$$

> $eq36 := map(coeffs, expand(ToJet(DGinfo(LieDerivative(V3a, V6a), "CoefficientSet"), \{u(var)\}, notation = jetnumbers)), \{q\});$
> $eq46 := map(coeffs, expand(ToJet(DGinfo(LieDerivative(V4a, V6a), "CoefficientSet"), \{u(var)\}, notation = jetnumbers)), \{q\})$

$$eq36 := \{u_{1,1} u_{1,2,2} - 2 u_{1,2} u_{1,1,2} + u_{2,2} u_{1,1,1} + u_{1,1,4} - u_{1,2,3}, -u_{1,1} u_{2,2,2} + 2 u_{1,2} u_{1,2,2} - u_{2,2} u_{1,1,2} - u_{1,2,4} + u_{2,2,3}, u_{1,3} u_{1,2,6} - u_{1,6} u_{1,2,3} - u_{2,3} u_{1,1,6} + u_{2,6} u_{1,1,3} + u_{1,3,8} - u_{1,5,6}, -u_{1,3} u_{2,2,6} + u_{1,6} u_{2,2,3} + u_{2,3} u_{1,2,6} - u_{2,6} u_{1,2,3} - u_{2,3,8} + u_{2,5,6}, u_{1,1} u_{1,2,4} - u_{1,2} u_{1,1,4} - u_{1,2} u_{1,2,3} + u_{1,3} u_{1,2,2} - u_{1,4} u_{1,1,2} + u_{2,2} u_{1,1,3} - u_{2,3} u_{1,1,2} + u_{2,4} u_{1,1,1} + u_{1,1,6} - u_{1,2,5}, -u_{1,1} u_{2,2,4} + u_{1,2} u_{1,2,4} + u_{1,2} u_{2,2,3} - u_{1,3} u_{2,2,2} + u_{1,4} u_{1,2,2} - u_{2,2} u_{1,2,3} + u_{2,3} u_{1,2,2} - u_{2,4} u_{1,1,2} - u_{1,2,6} + u_{2,2,5}, u_{1,1} u_{1,2,6} - u_{1,2} u_{1,1,6} + u_{1,3} u_{1,2,4} - u_{1,4} u_{1,2,3} - u_{1,6} u_{1,1,2} - u_{2,3} u_{1,1,4} + u_{2,4} u_{1,1,3} + u_{2,6} u_{1,1,1} + u_{1,1,8} - u_{1,4,5}, -u_{1,1} u_{2,2,6} + u_{1,2} u_{1,2,6} - u_{1,3} u_{2,2,4} + u_{1,4} u_{2,2,3} + u_{1,6} u_{1,2,2} + u_{2,3} u_{1,2,4} - u_{2,4} u_{1,2,3} - u_{2,6} u_{1,1,2} - u_{1,2,8} + u_{2,4,5}\}$$

$$eq46 := \{u_{1,2} u_{1,2,6} - u_{1,6} u_{1,2,2} - u_{2,2} u_{1,1,6} + u_{2,6} u_{1,1,2} + u_{1,2,8} - u_{1,4,6}, -u_{1,2} u_{2,2,6} + u_{1,6} u_{2,2,2} + u_{2,2} u_{1,2,6} - u_{2,6} u_{1,2,2} - u_{2,2,8} + u_{2,4,6}, u_{1,4} u_{1,2,6} - u_{1,6} u_{1,2,4} - u_{2,4} u_{1,1,6} + u_{2,6} u_{1,1,4} + u_{1,4,8} - u_{1,6,6}, -u_{1,4} u_{2,2,6} + u_{1,6} u_{2,2,4} + u_{2,4} u_{1,2,6} - u_{2,6} u_{1,2,4} - u_{2,4,8} + u_{2,6,6}\} \quad (3.15)$$

> $eq56 := map(coeffs, expand(ToJet(DGinfo(LieDerivative(V5a, V6a), "CoefficientSet"), \{u(var)\}, notation = jetnumbers)), \{q\})$

(3.16)

$$eq56 := \{u_{1,1}u_{1,2,2} - 2u_{1,2}u_{1,1,2} + u_{2,2}u_{1,1,1} + u_{1,1,4} - u_{1,2,3}, -u_{1,1}u_{2,2,2} + 2u_{1,2}u_{1,2,2} - u_{2,2}u_{1,1,2} - u_{1,2,4} + u_{2,2,3}, u_{1,5}u_{1,2,6} - u_{1,6}u_{1,2,5} - u_{2,5}u_{1,1,6} + u_{2,6}u_{1,1,5} + u_{1,5,8} - u_{1,6,7}, -u_{1,5}u_{2,2,6} + u_{1,6}u_{2,2,5} + u_{2,5}u_{1,2,6} - u_{2,6}u_{1,2,5} - u_{2,5,8} + u_{2,6,7}, u_{1,1}u_{1,2,4} - u_{1,2}u_{1,1,4} - u_{1,2}u_{1,2,3} + u_{1,3}u_{1,2,2} - u_{1,4}u_{1,1,2} + u_{2,2}u_{1,1,3} - u_{2,3}u_{1,1,2} + u_{2,4}u_{1,1,1} + u_{1,1,6} - u_{1,2,5}, -u_{1,1}u_{2,2,4} + u_{1,2}u_{1,2,4} + u_{1,2}u_{2,2,3} - u_{1,3}u_{2,2,2} + u_{1,4}u_{1,2,2} - u_{2,2}u_{1,2,3} + u_{2,3}u_{1,2,2} - u_{2,4}u_{1,1,2} - u_{1,2,6} + u_{2,2,5}, u_{1,3}u_{1,2,6} - u_{1,4}u_{1,2,5} + u_{1,5}u_{1,2,4} - u_{1,6}u_{1,2,3} - u_{2,3}u_{1,1,6} + u_{2,4}u_{1,1,5} - u_{2,5}u_{1,1,4} + u_{2,6}u_{1,1,3} + u_{1,3,8} - u_{1,4,7}, -u_{1,3}u_{2,2,6} + u_{1,4}u_{2,2,5} - u_{1,5}u_{2,2,4} + u_{1,6}u_{2,2,3} + u_{2,3}u_{1,2,6} - u_{2,4}u_{1,2,5} + u_{2,5}u_{1,2,4} - u_{2,6}u_{1,2,3} - u_{2,3,8} + u_{2,4,7}, u_{1,1}u_{1,2,6} - u_{1,2}u_{1,1,6} - u_{1,2}u_{1,2,5} + u_{1,3}u_{1,2,4} - u_{1,4}u_{1,2,3} + u_{1,5}u_{1,2,2} - u_{1,6}u_{1,1,2} + u_{2,2}u_{1,1,5} - u_{2,3}u_{1,1,4} + u_{2,4}u_{1,1,3} - u_{2,5}u_{1,1,2} + u_{2,6}u_{1,1,1} + u_{1,1,8} - u_{1,2,7}, -u_{1,1}u_{2,2,6} + u_{1,2}u_{1,2,6} + u_{1,2}u_{2,2,5} - u_{1,3}u_{2,2,4} + u_{1,4}u_{2,2,3} - u_{1,5}u_{2,2,2} + u_{1,6}u_{1,2,2} - u_{2,2}u_{1,2,5} + u_{2,3}u_{1,2,4} - u_{2,4}u_{1,2,3} + u_{2,5}u_{1,2,2} - u_{2,6}u_{1,1,2} - u_{1,2,8} + u_{2,2,7}\} \quad (3.16)$$

> $EQ2c := \{u_{1,1}u_{2,5} - u_{1,2}u_{1,5} + u_{1,7} - u_{3,5}, u_{1,2}u_{2,5} - u_{1,5}u_{2,2} + u_{2,7} - u_{4,5}, u_{1,1}u_{2,6} - u_{1,2}u_{1,6} + u_{1,8} - u_{3,6}, u_{1,2}u_{2,6} - u_{1,6}u_{2,2} + u_{2,8} - u_{4,6}, u_{1,3}u_{2,5} - u_{1,5}u_{2,3} + u_{3,7} - u_{5,5}, u_{1,4}u_{2,5} - u_{1,5}u_{2,4} + u_{4,7} - u_{5,6}, u_{1,3}u_{2,6} - u_{1,6}u_{2,3} + u_{3,8} - u_{5,6}, u_{1,4}u_{2,6} - u_{1,6}u_{2,4} + u_{4,8} - u_{6,6}, u_{1,5}u_{2,6} - u_{1,6}u_{2,5} + u_{5,8} - u_{6,7}\}$

$$EQ2c := \{u_{1,1}u_{2,5} - u_{1,2}u_{1,5} + u_{1,7} - u_{3,5}, u_{1,1}u_{2,6} - u_{1,2}u_{1,6} + u_{1,8} - u_{3,6}, u_{1,2}u_{2,5} - u_{1,5}u_{2,2} + u_{2,7} - u_{4,5}, u_{1,2}u_{2,6} - u_{1,6}u_{2,2} + u_{2,8} - u_{4,6}, u_{1,3}u_{2,5} - u_{1,5}u_{2,3} + u_{3,7} - u_{5,5}, u_{1,3}u_{2,6} - u_{1,6}u_{2,3} + u_{3,8} - u_{5,6}, u_{1,4}u_{2,5} - u_{1,5}u_{2,4} + u_{4,7} - u_{5,6}, u_{1,4}u_{2,6} - u_{1,6}u_{2,4} + u_{4,8} - u_{6,6}, u_{1,5}u_{2,6} - u_{1,6}u_{2,5} + u_{5,8} - u_{6,7}\} \quad (3.17)$$

> $slv2abc := solve(EQ2a \textbf{ union } EQ2b \textbf{ union } EQ2c, \{u_{1,3}, u_{1,4}, u_{1,5}, u_{1,6}, u_{1,7}, u_{1,8}, u_{2,5}, u_{2,6}, u_{2,7}, u_{2,8}, u_{3,7}, u_{3,8}, u_{4,7}, u_{4,8}, u_{6,7}\}) :$

> $nops(slv2abc)$

$$15 \quad (3.18)$$

## computing Char

> $smu := f \to add(add(diff(f, u_{i,j})\, p_i p_j, j = i..8), i = 1..8) :$

> $map(smu, EQ2a)$

$$\{u_{2,2}p_1^2 - 2u_{1,2}p_1p_2 + u_{1,1}p_2^2 + p_1p_4 - p_2p_3, u_{2,3}p_1^2 - u_{1,3}p_1p_2 - u_{1,2}p_1p_3 + u_{1,1}p_2p_3 + p_1p_5 - p_3^2, u_{2,3}p_1p_2 - u_{2,2}p_1p_3 - u_{1,3}p_2^2 + u_{1,2}p_2p_3 + p_2p_5 - p_3p_4\} \quad (3.3.1)$$

> $map(smu, EQ2b)$

(3.3.2)

$$\{u_{2,4}p_1p_2 - u_{2,2}p_1p_4 - u_{1,4}p_2^2 + u_{1,2}p_2p_4 + p_2p_6 - p_4^2, u_{2,4}p_1^2 - u_{1,4}p_1p_2 - u_{1,2}p_1p_4 + u_{1,1}p_2p_4 + p_1p_6 - p_3p_4, u_{2,4}p_1p_3 - u_{2,3}p_1p_4 - u_{1,4}p_2p_3 + u_{1,3}p_2p_4 + p_3p_6 - p_4p_5\} \quad (3.3.2)$$

> $map(smu, EQ2c)$

$$\{u_{2,5}p_1^2 - u_{1,5}p_1p_2 - u_{1,2}p_1p_5 + u_{1,1}p_2p_5 + p_1p_7 - p_3p_5, u_{2,5}p_1p_3 - u_{2,3}p_1p_5 - u_{1,5}p_2p_3 + u_{1,3}p_2p_5 + p_3p_7 - p_5^2, u_{2,6}p_1^2 - u_{1,6}p_1p_2 - u_{1,2}p_1p_6 + u_{1,1}p_2p_6 + p_1p_8 - p_3p_6, u_{2,5}p_1p_2 - u_{2,2}p_1p_5 - u_{1,5}p_2^2 + u_{1,2}p_2p_5 + p_2p_7 - p_4p_5, u_{2,6}p_1p_2 - u_{2,2}p_1p_6 - u_{1,6}p_2^2 + u_{1,2}p_2p_6 + p_2p_8 - p_4p_6, u_{2,6}p_1p_4 - u_{2,4}p_1p_6 - u_{1,6}p_2p_4 + u_{1,4}p_2p_6 + p_4p_8 - p_6^2, u_{2,6}p_1p_3 - u_{2,3}p_1p_6 - u_{1,6}p_2p_3 + u_{1,3}p_2p_6 + p_3p_8 - p_5p_6, u_{2,5}p_1p_4 - u_{2,4}p_1p_5 - u_{1,5}p_2p_4 + u_{1,4}p_2p_5 + p_4p_7 - p_5p_6, u_{2,6}p_1p_5 - u_{2,5}p_1p_6 - u_{1,6}p_2p_5 + u_{1,5}p_2p_6 + p_5p_8 - p_6p_7\} \quad (3.3.3)$$

> $solve(eval(map(smu, EQ2a), \{p_1 = 1\}), \{p_4, p_5\})$

$$\{p_4 = -u_{1,1}p_2^2 + p_2p_3 + 2p_2u_{1,2} - u_{2,2}, p_5 = -u_{1,1}p_2p_3 + p_2u_{1,3} + p_3^2 + p_3u_{1,2} - u_{2,3}\} \quad (3.3.4)$$

> $solve(eval(map(smu, EQ2b), \{p_1 = 1, p_4 = -u_{1,1}p_2^2 + p_2p_3 + 2p_2u_{1,2} - u_{2,2}, p_5 = -u_{1,1}p_2p_3 + p_2u_{1,3} + p_3^2 + p_3u_{1,2} - u_{2,3}\}), \{p_6\})$

$$\{p_6 = p_2^3u_{1,1}^2 - 2p_2^2p_3u_{1,1} - 3p_2^2u_{1,1}u_{1,2} + p_2p_3^2 + 3p_2p_3u_{1,2} + p_2u_{1,1}u_{2,2} + 2p_2u_{1,2}^2 + u_{1,4}p_2 - p_3u_{2,2} - u_{1,2}u_{2,2} - u_{2,4}\} \quad (3.3.5)$$

> $solve(eval(map(smu, EQ2c), \{p_1 = 1, p_4 = -u_{1,1}p_2^2 + p_2p_3 + 2p_2u_{1,2} - u_{2,2}, p_5 = -u_{1,1}p_2p_3 + p_2u_{1,3} + p_3^2 + p_3u_{1,2} - u_{2,3}, p_6 = p_2^3u_{1,1}^2 - 2p_2^2p_3u_{1,1} - 3p_2^2u_{1,1}u_{1,2} + p_2p_3^2 + 3p_2p_3u_{1,2} + p_2u_{1,1}u_{2,2} + 2p_2u_{1,2}^2 + u_{1,4}p_2 - p_3u_{2,2} - u_{1,2}u_{2,2} - u_{2,4}\}), \{p_7, p_8\})$

$$\{p_7 = p_2^2p_3u_{1,1}^2 - p_2^2u_{1,1}u_{1,3} - 2p_2p_3^2u_{1,1} - 2p_2p_3u_{1,1}u_{1,2} + p_2p_3u_{1,3} + p_2u_{1,1}u_{2,3} + p_2u_{1,2}u_{1,3} + p_3^3 + 2p_3^2u_{1,2} + p_3u_{1,2}^2 + u_{1,5}p_2 - p_3u_{2,3} - u_{1,2}u_{2,3} - u_{2,5}, p_8 = -p_2^4u_{1,1}^3 + 3p_2^3p_3u_{1,1}^2 + 4p_2^3u_{1,1}^2u_{1,2} - 3p_2^2p_3^2u_{1,1} - 8p_2^2p_3u_{1,1}u_{1,2} - p_2^2u_{1,1}^2u_{2,2} - 5p_2^2u_{1,1}u_{1,2}^2 - p_2^2u_{1,1}u_{1,4} + p_2p_3^3 + 4p_2p_3^2u_{1,2} + 2p_2p_3u_{1,1}u_{2,2} + 5p_2p_3u_{1,2}^2 + 2p_2u_{1,1}u_{1,2}u_{2,2} + 2p_2u_{1,2}^3 + u_{1,4}p_2p_3 + p_2u_{1,1}u_{2,4} + p_2u_{1,2}u_{1,4} - p_3^2u_{2,2} - 2p_3u_{1,2}u_{2,2} - u_{1,2}^2u_{2,2} + u_{1,6}p_2 - u_{2,4}p_3 - u_{1,2}u_{2,4} - u_{2,6}\} \quad (3.3.6)$$

> $scroll8 := simplify(eval([1, p_2, p_3, -u_{1,1}p_2^2 + p_2p_3 + 2p_2u_{1,2} - u_{2,2}, -u_{1,1}p_2p_3 + p_2u_{1,3} + p_3^2 + p_3u_{1,2} - u_{2,3}, p_2^3u_{1,1}^2 - 2p_2^2p_3u_{1,1} - 3p_2^2u_{1,1}u_{1,2} + p_2p_3^2$

$$+ 3 p_2 p_3 u_{1,2} + p_2 u_{1,1} u_{2,2} + 2 p_2 u_{1,2}^2 + u_{1,4} p_2 - p_3 u_{2,2} - u_{1,2} u_{2,2} - u_{2,4}, p_2^2 p_3 u_{1,1}^2 - p_2^2 u_{1,1} u_{1,3} - 2 p_2 p_3^2 u_{1,1} - 2 p_2 p_3 u_{1,1} u_{1,2} + p_2 p_3 u_{1,3} + p_2 u_{1,1} u_{2,3} + p_2 u_{1,2} u_{1,3} + p_3^3 + 2 p_3^2 u_{1,2} + p_3 u_{1,2}^2 + u_{1,5} p_2 - p_3 u_{2,3} - u_{1,2} u_{2,3} - u_{2,5}, -p_2^4 u_{1,1}^3 + 3 p_2^3 p_3 u_{1,1}^2 + 4 p_2^3 u_{1,1}^2 u_{1,2} - 3 p_2^2 p_3^2 u_{1,1} - 8 p_2^2 p_3 u_{1,1} u_{1,2} - p_2^2 u_{1,1}^2 u_{2,2} - 5 p_2^2 u_{1,1} u_{1,2}^2 - p_2^2 u_{1,1} u_{1,4} + p_2 p_3^3 + 4 p_2 p_3^2 u_{1,2} + 2 p_2 p_3 u_{1,1} u_{2,2} + 5 p_2 p_3 u_{1,2}^2 + 2 p_2 u_{1,1} u_{1,2} u_{2,2} + 2 p_2 u_{1,2}^3 + u_{1,4} p_2 p_3 + p_2 u_{1,1} u_{2,4} + p_2 u_{1,2} u_{1,4} - p_3^2 u_{2,2} - 2 p_3 u_{1,2} u_{2,2} - u_{1,2}^2 u_{2,2} + u_{1,6} p_2 - u_{2,4} p_3 - u_{1,2} u_{2,4} - u_{2,6}], \{p_2 = \chi, p_3 = \lambda + \chi u_{1,1}\}))$$

$$scroll8 := [1, \chi, \chi u_{1,1} + \lambda, (\lambda + 2 u_{1,2}) \chi - u_{2,2}, \lambda^2 + (\chi u_{1,1} + u_{1,2}) \lambda + (u_{1,1} u_{1,2} + u_{1,3}) \chi - u_{2,3}, (\lambda^2 + 3 \lambda u_{1,2} + 2 u_{1,2}^2 + u_{1,4}) \chi - \lambda u_{2,2} - u_{1,2} u_{2,2} - u_{2,4}, \lambda^3 + (\chi u_{1,1} + 2 u_{1,2}) \lambda^2 + (2 \chi u_{1,1} u_{1,2} + \chi u_{1,3} + u_{1,2}^2 - u_{2,3}) \lambda + \chi u_{1,1} u_{1,2}^2 + (\chi u_{1,3} - u_{2,3}) u_{1,2} + u_{1,5} \chi - u_{2,5}, 2 \chi u_{1,2}^3 + (5 \chi \lambda - u_{2,2}) u_{1,2}^2 + (4 \chi \lambda^2 + \chi u_{1,4} - 2 \lambda u_{2,2} - u_{2,4}) u_{1,2} + \chi \lambda^3 - \lambda^2 u_{2,2} + (\chi u_{1,4} - u_{2,4}) \lambda + u_{1,6} \chi - u_{2,6}] \quad \textbf{(3.3.7)}$$

> $diff(scroll8, \chi\$2)$

$$[0, 0, 0, 0, 0, 0, 0, 0] \quad \textbf{(3.3.8)}$$

> $scroll80 := eval(scroll8, \chi = 0) : scroll81 := diff(scroll8, \chi) :$

> $scroll80 + \chi \cdot scroll81$

$$\chi [0, 1, u_{1,1}, \lambda + 2 u_{1,2}, u_{1,1} \lambda + u_{1,1} u_{1,2} + u_{1,3}, \lambda^2 + 3 \lambda u_{1,2} + 2 u_{1,2}^2 + u_{1,4}, u_{1,1} \lambda^2 + (2 u_{1,1} u_{1,2} + u_{1,3}) \lambda + u_{1,1} u_{1,2}^2 + u_{1,2} u_{1,3} + u_{1,5}, 2 u_{1,2}^3 + 5 \lambda u_{1,2}^2 + (4 \lambda^2 + u_{1,4}) u_{1,2} + \lambda^3 + u_{1,4} \lambda + u_{1,6}] + [1, 0, \lambda, -u_{2,2}, \lambda^2 + \lambda u_{1,2} - u_{2,3}, -\lambda u_{2,2} - u_{1,2} u_{2,2} - u_{2,4}, \lambda^3 + 2 \lambda^2 u_{1,2} + (u_{1,2}^2 - u_{2,3}) \lambda - u_{1,2} u_{2,3} - u_{2,5}, -u_{1,2}^2 u_{2,2} + (-2 \lambda u_{2,2} - u_{2,4}) u_{1,2} - \lambda^2 u_{2,2} - \lambda u_{2,4} - u_{2,6}] \quad \textbf{(3.3.9)}$$

> $eval(diff(scroll80, \lambda), \lambda = 0)$

$$[0, 0, 1, 0, u_{1,2}, -u_{2,2}, u_{1,2}^2 - u_{2,3}, -2 u_{1,2} u_{2,2} - u_{2,4}] \quad \textbf{(3.3.10)}$$

> $Ma8 := Matrix([eval(scroll80, \lambda = 0), eval(diff(scroll80, \lambda), \lambda = 0), eval(diff(scroll80, \lambda\$2), \lambda = 0), diff(scroll80, \lambda\$3), eval(scroll81, \lambda = 0), eval(diff(scroll81, \lambda), \lambda = 0), eval(diff(scroll81, \lambda\$2), \lambda = 0), diff(scroll81, \lambda\$3)])$

$$Ma8 := \quad \textbf{(3.3.11)}$$

$$\begin{bmatrix} 1 & 0 & 0 & -u_{2,2} & -u_{2,3} & -u_{1,2}u_{2,2}-u_{2,4} & \cdots \\ 0 & 0 & 1 & 0 & u_{1,2} & -u_{2,2} & \cdots \\ 0 & 0 & 0 & 0 & 2 & 0 & \cdots \\ 0 & 0 & 0 & 0 & 0 & 0 & \cdots \\ 0 & 1 & u_{1,1} & 2u_{1,2} & u_{1,1}u_{1,2}+u_{1,3} & 2u_{1,2}^2+u_{1,4} & u\cdots \\ 0 & 0 & 0 & 1 & u_{1,1} & 3u_{1,2} & \cdots \\ 0 & 0 & 0 & 0 & 0 & 2 & \cdots \\ 0 & 0 & 0 & 0 & 0 & 0 & \cdots \end{bmatrix}$$

> *Determinant*(*Ma8*)

144 **(3.3.12)**

## compatibility

> *DGsetup*([*x*, *y*, *t1*, *t2*, *t3*, *t4*, *t5*, *t6*], [*u*], *M8J*, 5) :

> *EQ2* := *EQ2a* **union** *EQ2b* **union** *EQ2c* : *nops*(*EQ2*)

15 **(3.4.1)**

> $jet2 := \{seq(seq(u_{i,j}, j=i..8), i=1..8)\} : jet3 := \{seq(seq(seq(u_{i,j,k}, k=j..8), j=i..8), i=1..8)\}$ :

> # *for k to nops*(*eq5w*) **do**: *S2* := { } :**for** *i* **to** *nops*(*jet2*) **do if** *diff*(*eq5w*[*k*], *jet2*[*i*]) ≠ 0 **then** *S2* := *S2* **union** {*jet2*[*i*]} :**fi**:**od**: *print*(*S2*);**od**:

> *eliminate*(*eval*({*seq*(*seq*(*TotalDiff*(*EQ2*[*i*], *j*), *j* = 1 ..8), *i* = 1 ..*nops*(*Eq2*))}, *slv2abc*), *jet3*)[2]

∅ **(3.4.2)**

> *ChangeFrame*(*M8p*) :

>

>
