# Supplementary material for: Involutive scroll structures on solutions of 4D dispersionless integrable hierarchies
Source: arXiv:2503.10897 ancillary file (2025-03-13)
Supplement: Supplementary file 3 [file EFBK25-Scroll-Suppl-3.pdf]

Computation of symmetry algebras of rational normal scrolls S[n,m]<P^{n+m+1} of degree (n+m) for EFBK-2025-Scroll paper

```
>
> with(DifferentialGeometry) : with(Tensor) : with(JetCalculus) : with(GroupActions) :
    with(Tools) : with(PDETools) : with(LieAlgebras) : with(LinearAlgebra) :
    with(PolynomialIdeals) : with(Groebner) : Preferences("ShowFramePrompt",'false') :
>
> n := 1 : m := 1 :
> var := seq(x||i, i=0..n), seq(y||j, j=0..m) : Dvar := seq(D_x||i, i=0..n), seq(D_y||j, j=0
    ..m) : dvar := seq(dx||i, i=0..n), seq(dy||j, j=0..m) : DGsetup([var], M) :
> X := evalDG(add(add((a||i||j) var[i] Dvar[j], j=1..n+m+2), i=1..n+m+2)) :
> EQ := {seq(seq((x||i)·(x||j) − (x||(i+1))·(x||(j−1)), j=i+2..n), i=0..n−2), seq(seq
    ((x||i)·(y||j) − (x||(i+1))·(y||(j−1)), j=1..m), i=0..n−1), seq(seq((y||i)·(y||j)
    − (y||(i+1))·(y||(j−1)), j=i+2..m), i=0..m−2)}:
> rns := {seq(x||i = a λ^i, i=0..n), seq(y||j = b λ^j, j=0..m)} : simplify(eval(EQ, rns))
```

$$\{0\} \tag{1}$$

```
> J := ⟨op(EQ)⟩ : HilbertDimension(J)
```

$$3 \tag{2}$$

```
> sol := solve({seq(coeffs(expand(eval(LieDerivative(X, EQ[k]), rns)), {a, b, λ}), k=1
    ..nops(EQ))}) : free := { } :for i to nops(sol) do if lhs(sol[i]) = rhs(sol[i]) then free :=
    {op(free), lhs(sol[i])} :fi:od: d := nops(free)
```

$$d := 7 \tag{3}$$

```
> Xtmp := eval(X, sol) :for i to d do X||i := DGsimplify(eval(Xtmp, {seq(free[j]=0, j=1..i
    − 1), free[i]=1, seq(free[j]=0, j=i+1..d)})) :od:
> seq(X||i, i=1..7)
```

x0 D_x0 + x1 D_x1, x0 D_y0 + x1 D_y1, x0 D_x0 + y0 D_y0, x0 D_x1 + y0 D_y1, y0 D_x0 + y1 D_x1, x1 D_x0 + y1 D_y0, −x0 D_x0 + y1 D_y1 **(4)**

```
> L := LieAlgebraData([seq(X||i, i=1..d)], alg) : DGsetup(L) : LD := LeviDecomposition( )
```

$$LD := [[e1 + e3 + e7], [e1 - e3, e2, e4, e5, e6, e7]] \tag{5}$$

```
> Center( )
```

$$[e1 + e3 + e7] \tag{6}$$

```
> LieAlgebraData([e1 − e3 + e7, e6, e4, e7 − e1 + e3, e5, e2, e1 + e3 + e7])
```

$$[[e1, e2] = 2\,e2, [e1, e3] = -2\,e3, [e2, e3] = e1, [e4, e5] = 2\,e5, [e4, e6] = -2\,e6, [e5, e6] = e4] \tag{7}$$

```
> evalDG(X1 − X3 + X7), X6, X4; evalDG(X7 − X1 + X3), X5, X2
```

−x0 D_x0 + x1 D_x1 − y0 D_y0 + y1 D_y1, x1 D_x0 + y1 D_y0, x0 D_x1 + y0 D_y1

−x0 D_x0 − x1 D_x1 + y0 D_y0 + y1 D_y1, y0 D_x0 + y1 D_x1, x0 D_y0 + x1 D_y1 **(8)**

```
>
> n := 1 : m := 2 :
> var := seq(x||i, i=0..n), seq(y||j, j=0..m) : Dvar := seq(D_x||i, i=0..n), seq(D_y||j, j=0
    ..m) : dvar := seq(dx||i, i=0..n), seq(dy||j, j=0..m) : DGsetup([var], M) :
> X := evalDG(add(add((a||i||j) var[i] Dvar[j], j=1..n+m+2), i=1..n+m+2)) :
> EQ := {seq(seq((x||i)·(x||j) − (x||(i+1))·(x||(j−1)), j=i+2..n), i=0..n−2), seq(seq
```

$((x\|i)\cdot(y\|j)-(x\|(i+1))\cdot(y\|(j-1)), j=1..m), i=0..n-1), seq(seq((y\|i)\cdot(y\|j)-(y\|(i+1))\cdot(y\|(j-1)), j=i+2..m), i=0..m-2)\}:$

> $rns := \{seq(x\|i = a\,\lambda^i, i=0..n), seq(y\|j = b\,\lambda^j, j=0..m)\} : simplify(eval(EQ, rns))$

$$\{0\} \quad \textbf{(9)}$$

> $J := \langle op(EQ)\rangle : HilbertDimension(J)$

$$3 \quad \textbf{(10)}$$

> $sol := solve(\{seq(coeffs(expand(eval(LieDerivative(X, EQ[k]), rns)), \{a, b, \lambda\}), k=1..nops(EQ))\}) : free := \{\ \}$ :**for** $i$ **to** $nops(sol)$ **do if** $lhs(sol[i]) = rhs(sol[i])$ **then** $free := \{op(free), lhs(sol[i])\}$ :**fi**:**od**: $d := nops(free)$

$$d := 7 \quad \textbf{(11)}$$

> $Xtmp := eval(X, sol)$ :**for** $i$ **to** $d$ **do** $X\|i := DGsimplify(eval(Xtmp, \{seq(free[j]=0, j=1..i-1), free[i]=1, seq(free[j]=0, j=i+1..d)\}))$ :**od**:

> $L := LieAlgebraData([seq(X\|i, i=1..d)], alg) : DGsetup(L) : LD := LeviDecomposition(\ )$

$$LD := [[e1, e3, e4+e7, e5], [e1+2\,e7, e2, e6]] \quad \textbf{(12)}$$

> $Center(\ )$

$$[e1+e4+e7] \quad \textbf{(13)}$$

> $LieAlgebraData([e1, e3, e5]); LieAlgebraData([e1+2\,e7, e6, e2]); LieAlgebraData([e1+2\,e7, e1, e3, e5])$

$$[[e1, e2] = -e2, [e1, e3] = -e3]$$

$$[[e1, e2] = 2\,e2, [e1, e3] = -2\,e3, [e2, e3] = e1]$$

$$[[e1, e3] = -e3, [e1, e4] = e4, [e2, e3] = -e3, [e2, e4] = -e4] \quad \textbf{(14)}$$

> $LieAlgebraData([e1, e3, e5])$

$$[[e1, e2] = -e2, [e1, e3] = -e3] \quad \textbf{(15)}$$

> $Centralizer([e1+k\,e3])$

$$\left[e7, -k\,e5+e6, e1+e4, \frac{e1}{k}+e3, e2\right] \quad \textbf{(16)}$$

> $LieAlgebraData([e1+k\,e7, e2])$

$$[[e1, e2] = -e2\,k] \quad \textbf{(17)}$$

> $X1, X3, X5; evalDG(X1+2\,X7), X2, X6$

$$x0\,D\_x0+x1\,D\_x1, y0\,D\_x0+y1\,D\_x1, y1\,D\_x0+y2\,D\_x1$$

$$-x0\,D\_x0+x1\,D\_x1-2\,y0\,D\_y0+2\,y2\,D\_y2, x0\,D\_x1+y0\,D\_y1+2\,y1\,D\_y2, x1\,D\_x0+2\,y1\,D\_y0+y2\,D\_y1 \quad \textbf{(18)}$$

> $evalDG(X1+k\,X4+l\,X7)$

$$(k\,x0-l\,x0+x0)\,D\_x0+x1\,D\_x1+(2\,k\,y0-l\,y0)\,D\_y0+k\,y1\,D\_y1+l\,y2\,D\_y2 \quad \textbf{(19)}$$

>

> $n := 1 : m := 3 :$

> $var := seq(x\|i, i=0..n), seq(y\|j, j=0..m) : Dvar := seq(D\_x\|i, i=0..n), seq(D\_y\|j, j=0..m) : dvar := seq(dx\|i, i=0..n), seq(dy\|j, j=0..m) : DGsetup([var], M) :$

> $X := evalDG(add(add((a\|i\|j)\,var[i]\,Dvar[j], j=1..n+m+2), i=1..n+m+2)) :$

> $EQ := \{seq(seq((x\|i)\cdot(x\|j)-(x\|(i+1))\cdot(x\|(j-1)), j=i+2..n), i=0..n-2), seq(seq((x\|i)\cdot(y\|j)-(x\|(i+1))\cdot(y\|(j-1)), j=1..m), i=0..n-1), seq(seq((y\|i)\cdot(y\|j)$

$-(y\|(i+1))\cdot(y\|(j-1)), j=i+2..m), i=0..m-2)\}$:

> $rns := \{seq(x\|i = a\lambda^i, i=0..n), seq(y\|j = b\lambda^j, j=0..m)\} : simplify(eval(EQ, rns))$

$$\{0\} \quad (20)$$

> $J := \langle op(EQ)\rangle : HilbertDimension(J)$

$$3 \quad (21)$$

> $sol := solve(\{seq(coeffs(expand(eval(LieDerivative(X, EQ[k]), rns)), \{a, b, \lambda\}), k=1..nops(EQ))\})$ : $free := \{\}$ :**for** $i$ **to** $nops(sol)$ **do if** $lhs(sol[i]) = rhs(sol[i])$ **then** $free := \{op(free), lhs(sol[i])\}$ :**fi**:**od**: $d := nops(free)$

$$d := 8 \quad (22)$$

> $Xtmp := eval(X, sol)$ :**for** $i$ **to** $d$ **do** $X\|i := DGsimplify(eval(Xtmp, \{seq(free[j]=0, j=1..i-1), free[i]=1, seq(free[j]=0, j=i+1..d)\}))$ :**od**:

> $L := LieAlgebraData([seq(X\|i, i=1..d)], alg) : DGsetup(L) : LD := LeviDecomposition(\,)$

$$LD := [[e1, e2, e3, e4+e8, e6], [e1+e4+3\,e8, e5, e7]] \quad (23)$$

> $Center(\,)$

$$[e1+e4+e8] \quad (24)$$

> $LieAlgebraData([e1, e2, e3, e6]); LieAlgebraData([e1+e4+3\,e8, e7, 3\,e5]); LieAlgebraData([e1+e4+3\,e8, e1, e2, e3, e6])$

$$[[e1, e2] = -e2, [e1, e3] = -e3, [e1, e4] = -e4]$$
$$[[e1, e2] = 2\,e2, [e1, e3] = -2\,e3, [e2, e3] = e1]$$
$$[[e1, e3] = -2\,e3, [e1, e5] = 2\,e5, [e2, e3] = -e3, [e2, e4] = -e4, [e2, e5] = -e5] \quad (25)$$

> $X1, X2, X3, evalDG(X4 + X8), X6; evalDG(X1 + X4 + 3\,X8), evalDG(3\,X5), X7$

$$x0\,D\_x0 + x1\,D\_x1, y0\,D\_x0 + y1\,D\_x1, y1\,D\_x0 + y2\,D\_x1, y0\,D\_y0 + y1\,D\_y1 + y2\,D\_y2 + y3\,D\_y3, y2\,D\_x0 + y3\,D\_x1$$
$$-x0\,D\_x0 + x1\,D\_x1 - 3\,y0\,D\_y0 - y1\,D\_y1 + y2\,D\_y2 + 3\,y3\,D\_y3, x0\,D\_x1 + y0\,D\_y1 + 2\,y1\,D\_y2 + 3\,y2\,D\_y3, x1\,D\_x0 + 3\,y1\,D\_y0 + 2\,y2\,D\_y1 + y3\,D\_y2 \quad (26)$$

>

> $n := 1 : m := 4 :$

> $var := seq(x\|i, i=0..n), seq(y\|j, j=0..m) : Dvar := seq(D\_x\|i, i=0..n), seq(D\_y\|j, j=0..m) : dvar := seq(dx\|i, i=0..n), seq(dy\|j, j=0..m) : DGsetup([var], M) :$

> $X := evalDG(add(add((a\|i\|j)\, var[i]\, Dvar[j], j=1..n+m+2), i=1..n+m+2)) :$

> $EQ := \{seq(seq((x\|i)\cdot(x\|j) - (x\|(i+1))\cdot(x\|(j-1)), j=i+2..n), i=0..n-2), seq(seq((x\|i)\cdot(y\|j) - (x\|(i+1))\cdot(y\|(j-1)), j=1..m), i=0..n-1), seq(seq((y\|i)\cdot(y\|j) - (y\|(i+1))\cdot(y\|(j-1)), j=i+2..m), i=0..m-2)\}$:

> $rns := \{seq(x\|i = a\lambda^i, i=0..n), seq(y\|j = b\lambda^j, j=0..m)\} : simplify(eval(EQ, rns))$

$$\{0\} \quad (27)$$

> $J := \langle op(EQ)\rangle : HilbertDimension(J)$

$$3 \quad (28)$$

> $sol := solve(\{seq(coeffs(expand(eval(LieDerivative(X, EQ[k]), rns)), \{a, b, \lambda\}), k=1..nops(EQ))\})$ : $free := \{\}$ :**for** $i$ **to** $nops(sol)$ **do if** $lhs(sol[i]) = rhs(sol[i])$ **then** $free := \{op(free), lhs(sol[i])\}$ :**fi**:**od**: $d := nops(free)$

$$d := 9 \quad (29)$$

```
> Xtmp := eval(X, sol) :for i to d do X||i := DGsimplify(eval(Xtmp, {seq(free[j] = 0, j = 1 ..i
      - 1), free[i] = 1, seq(free[j] = 0, j = i + 1 ..d)})) :od:
> L := LieAlgebraData([seq(X||i, i = 1 ..d)], alg) : DGsetup(L) : LD := LeviDecomposition( )
```

$$LD := [[e1, e2, e3, e4, e5 + e9, e7], [e1 + 2\, e5 + 4\, e9, e6, e8]] \tag{30}$$

```
> Center( )
```

$$[e1 + e5 + e9] \tag{31}$$

```
> LieAlgebraData([e1, e2, e3, e4, e7, e1 + e5 + e9]); LieAlgebraData([e2, e3, e4, e7]);
    LieAlgebraData([e1 + 2 e5 + 4 e9, e8, 4 e6, e1 + e5 + e9]); LieAlgebraData([-e1 - 2 e4
    + 2 e9, e1 + 2 e4, e2, e3, e4, e7])
```

$$[[e1, e2] = -e2, [e1, e3] = -e3, [e1, e4] = -e4, [e1, e5] = -e5]$$

$$[\,]$$

$$[[e1, e2] = 2\, e2, [e1, e3] = -2\, e3, [e2, e3] = e1]$$

$$[[e1, e3] = -3\, e3, [e1, e4] = -e4, [e1, e5] = e5, [e1, e6] = 3\, e6, [e2, e3] = -e3, [e2, e4] = -e4, [e2, e5] = -e5, [e2, e6] = -e6] \tag{32}$$

```
> evalDG(X1 + X5 + X9); evalDG(X1 + 2 X5 + 4 X9), X8, X6, evalDG(X1 + 2 X5 - 2 X9);
    X2, X3, X4, X7
```

$$x0\, D\_x0 + x1\, D\_x1 + y0\, D\_y0 + y1\, D\_y1 + y2\, D\_y2 + y3\, D\_y3 + y4\, D\_y4$$

$$-x0\, D\_x0 + x1\, D\_x1 - 4\, y0\, D\_y0 - 2\, y1\, D\_y1 + 2\, y3\, D\_y3 + 4\, y4\, D\_y4, x1\, D\_x0 + 4\, y1\, D\_y0 + 3\, y2\, D\_y1 + 2\, y3\, D\_y2 + y4\, D\_y3, \frac{x0\, D\_x1}{4} + \frac{y0\, D\_y1}{4} + \frac{y1\, D\_y2}{2} + \frac{3\, y2\, D\_y3}{4} + y3\, D\_y4, 5\, x0\, D\_x0 + x1\, D\_x1 + 14\, y0\, D\_y0 + 10\, y1\, D\_y1 + 6\, y2\, D\_y2 + 2\, y3\, D\_y3 - 2\, y4\, D\_y4$$

$$y0\, D\_x0 + y1\, D\_x1, y1\, D\_x0 + y2\, D\_x1, y2\, D\_x0 + y3\, D\_x1, y3\, D\_x0 + y4\, D\_x1 \tag{33}$$

```
>
> n := 2 : m := 2 :
> var := seq(x||i, i = 0 ..n), seq(y||j, j = 0 ..m) : Dvar := seq(D_x||i, i = 0 ..n), seq(D_y||j, j = 0
      ..m) : dvar := seq(dx||i, i = 0 ..n), seq(dy||j, j = 0 ..m) : DGsetup([var], M) :
> X := evalDG(add(add((a||i||j) var[i] Dvar[j], j = 1 ..n + m + 2), i = 1 ..n + m + 2)) :
> EQ := {seq(seq((x||i)·(x||j) - (x||(i + 1))·(x||(j - 1)), j = i + 2 ..n), i = 0 ..n - 2), seq(seq
      ((x||i)·(y||j) - (x||(i + 1))·(y||(j - 1)), j = 1 ..m), i = 0 ..n - 1), seq(seq((y||i)·(y||j)
      - (y||(i + 1))·(y||(j - 1)), j = i + 2 ..m), i = 0 ..m - 2)}:
> rns := {seq(x||i = a λ^i, i = 0 ..n), seq(y||j = b λ^j, j = 0 ..m)} : simplify(eval(EQ, rns))
```

$$\{0\} \tag{34}$$

```
> J := ⟨op(EQ)⟩ : HilbertDimension(J)
```

$$3 \tag{35}$$

```
> sol := solve({seq(coeffs(expand(eval(LieDerivative(X, EQ[k]), rns)), {a, b, λ}), k = 1
      ..nops(EQ))}) : free := { } :for i to nops(sol) do if lhs(sol[i]) = rhs(sol[i]) then free :=
      {op(free), lhs(sol[i])} :fi:od: d := nops(free)
```

$$d := 7 \tag{36}$$

```
> Xtmp := eval(X, sol) :for i to d do X||i := DGsimplify(eval(Xtmp, {seq(free[j] = 0, j = 1 ..i
      - 1), free[i] = 1, seq(free[j] = 0, j = i + 1 ..d)})) :od:
```

```
> L := LieAlgebraData([seq(X||i, i=1..d)], alg) : DGsetup(L) : LD := LeviDecomposition( )
                LD := [[e1 + e3 + e7], [e1 + e7, e2, e3 + 2 e7, e4, e5, e6]]          (37)
> Center( )
                [e1 + e3 + e7]                                                          (38)
> LieAlgebraData([2 e1 + 2 e7, 2 e6, e4, e3 + 2 e7 - (e1 + e7), e5, e2])
  [[e1, e2] = 2 e2, [e1, e3] = -2 e3, [e2, e3] = e1, [e4, e5] = 2 e5, [e4, e6] = -2 e6, [e5, e6] = e4]   (39)
>
> n := 2 : m := 3 :
> var := seq(x||i, i=0..n), seq(y||j, j=0..m) : Dvar := seq(D_x||i, i=0..n), seq(D_y||j, j=0
     ..m) : dvar := seq(dx||i, i=0..n), seq(dy||j, j=0..m) : DGsetup([var], M) :
> X := evalDG(add(add((a||i||j) var[i] Dvar[j], j=1..n + m + 2), i=1..n + m + 2)) :
> EQ := {seq(seq((x||i)·(x||j) - (x||(i + 1))·(x||(j - 1)), j=i + 2..n), i=0..n - 2), seq(seq
     ((x||i)·(y||j) - (x||(i + 1))·(y||(j - 1)), j=1..m), i=0..n - 1), seq(seq((y||i)·(y||j)
     - (y||(i + 1))·(y||(j - 1)), j=i + 2..m), i=0..m - 2)}:
> rns := {seq(x||i = a λ^i, i=0..n), seq(y||j = b λ^j, j=0..m)} : simplify(eval(EQ, rns))
                {0}                                                                     (40)
> J := ⟨op(EQ)⟩ : HilbertDimension(J)
                3                                                                       (41)
> sol := solve({seq(coeffs(expand(eval(LieDerivative(X, EQ[k]), rns)), {a, b, λ}), k=1
     ..nops(EQ))}) : free := { } :for i to nops(sol) do if lhs(sol[i]) = rhs(sol[i]) then free :=
     {op(free), lhs(sol[i])} :fi:od: d := nops(free)
                d := 7                                                                  (42)
> Xtmp := eval(X, sol) :for i to d do X||i := DGsimplify(eval(Xtmp, {seq(free[j]=0, j=1..i
     - 1), free[i]=1, seq(free[j]=0, j=i + 1..d)})) :od:
> L := LieAlgebraData([seq(X||i, i=1..d)], alg) : DGsetup(L) : LD := LeviDecomposition( )
                LD := [[e1, e2, e3 + e7, e5], [e1 + e3/2 + 3 e7/2, e4, e6]]           (43)
> Center( )
                [e1 + e3 + e7]                                                          (44)
> LieAlgebraData([e1, e2, e5]); LieAlgebraData([2 e1 + e3 + 3 e7, e6, 3 e4]);
     LieAlgebraData([2 e1 + e3 + 3 e7, e1, e2, e5])
                [[e1, e2] = -e2, [e1, e3] = -e3]
                [[e1, e2] = 2 e2, [e1, e3] = -2 e3, [e2, e3] = e1]
                [[e1, e3] = -e3, [e1, e4] = e4, [e2, e3] = -e3, [e2, e4] = -e4]        (45)
>
> n := 2 : m := 4 :
> var := seq(x||i, i=0..n), seq(y||j, j=0..m) : Dvar := seq(D_x||i, i=0..n), seq(D_y||j, j=0
     ..m) : dvar := seq(dx||i, i=0..n), seq(dy||j, j=0..m) : DGsetup([var], M) :
> X := evalDG(add(add((a||i||j) var[i] Dvar[j], j=1..n + m + 2), i=1..n + m + 2)) :
> EQ := {seq(seq((x||i)·(x||j) - (x||(i + 1))·(x||(j - 1)), j=i + 2..n), i=0..n - 2), seq(seq
     ((x||i)·(y||j) - (x||(i + 1))·(y||(j - 1)), j=1..m), i=0..n - 1), seq(seq((y||i)·(y||j)
     - (y||(i + 1))·(y||(j - 1)), j=i + 2..m), i=0..m - 2)}:
```

> $rns := \{seq(x \| i = a\,\lambda^i, i = 0..n), seq(y \| j = b\,\lambda^j, j = 0..m)\} : simplify(eval(EQ, rns))$

$$\{0\} \quad (46)$$

> $J := \langle op(EQ) \rangle : HilbertDimension(J)$

$$3 \quad (47)$$

> $sol := solve(\{seq(coeffs(expand(eval(LieDerivative(X, EQ[k]), rns)), \{a, b, \lambda\}), k = 1..nops(EQ))\}) : free := \{\,\} :$ **for** $i$ **to** $nops(sol)$ **do if** $lhs(sol[i]) = rhs(sol[i])$ **then** $free := \{op(free), lhs(sol[i])\}$ **fi**:**od**: $d := nops(free)$

$$d := 8 \quad (48)$$

> $Xtmp := eval(X, sol) :$ **for** $i$ **to** $d$ **do** $X \| i := DGsimplify(eval(Xtmp, \{seq(free[j] = 0, j = 1..i - 1), free[i] = 1, seq(free[j] = 0, j = i + 1..d)\}))$ **:od**:

> $L := LieAlgebraData([seq(X \| i, i = 1..d)], alg) : DGsetup(L) : LD := LeviDecomposition(\,)$

$$LD := [[e1, e2, e3, e4 + e8, e6], [e1 + e4 + 2\,e8, e5, e7]] \quad (49)$$

> $Center(\,)$

$$[e1 + e4 + e8] \quad (50)$$

> $LieAlgebraData([e1, e2, e3, e6]); LieAlgebraData([2\,e1 + 2\,e4 + 4\,e8, e7, 4\,e5]); LieAlgebraData([2\,e1 + 2\,e4 + 4\,e8, e1, e2, e3, e6])$

$$[[e1, e2] = -e2, [e1, e3] = -e3, [e1, e4] = -e4]$$

$$[[e1, e2] = 2\,e2, [e1, e3] = -2\,e3, [e2, e3] = e1]$$

$$[[e1, e3] = -2\,e3, [e1, e5] = 2\,e5, [e2, e3] = -e3, [e2, e4] = -e4, [e2, e5] = -e5] \quad (51)$$

>

> $n := 3 : m := 3 :$

> $var := seq(x \| i, i = 0..n), seq(y \| j, j = 0..m) : Dvar := seq(D\_x \| i, i = 0..n), seq(D\_y \| j, j = 0..m) : dvar := seq(dx \| i, i = 0..n), seq(dy \| j, j = 0..m) : DGsetup([var], M) :$

> $X := evalDG(add(add((a \| i \| j)\, var[i]\, Dvar[j], j = 1..n + m + 2), i = 1..n + m + 2)) :$

> $EQ := \{seq(seq((x \| i) \cdot (x \| j) - (x \| (i + 1)) \cdot (x \| (j - 1)), j = i + 2..n), i = 0..n - 2), seq(seq((x \| i) \cdot (y \| j) - (x \| (i + 1)) \cdot (y \| (j - 1)), j = 1..m), i = 0..n - 1), seq(seq((y \| i) \cdot (y \| j) - (y \| (i + 1)) \cdot (y \| (j - 1)), j = i + 2..m), i = 0..m - 2)\}:$

> $rns := \{seq(x \| i = a\,\lambda^i, i = 0..n), seq(y \| j = b\,\lambda^j, j = 0..m)\} : simplify(eval(EQ, rns))$

$$\{0\} \quad (52)$$

> $J := \langle op(EQ) \rangle : HilbertDimension(J)$

$$3 \quad (53)$$

> $sol := solve(\{seq(coeffs(expand(eval(LieDerivative(X, EQ[k]), rns)), \{a, b, \lambda\}), k = 1..nops(EQ))\}) : free := \{\,\} :$ **for** $i$ **to** $nops(sol)$ **do if** $lhs(sol[i]) = rhs(sol[i])$ **then** $free := \{op(free), lhs(sol[i])\}$ **fi**:**od**: $d := nops(free)$

$$d := 7 \quad (54)$$

> $Xtmp := eval(X, sol) :$ **for** $i$ **to** $d$ **do** $X \| i := DGsimplify(eval(Xtmp, \{seq(free[j] = 0, j = 1..i - 1), free[i] = 1, seq(free[j] = 0, j = i + 1..d)\}))$ **:od**:

> $L := LieAlgebraData([seq(X \| i, i = 1..d)], alg) : DGsetup(L) : LD := LeviDecomposition(\,)$

$$LD := \left[[e1 + e3 + e7], \left[e1 + \frac{e7}{2}, e2, e3 + \frac{3\,e7}{2}, e4, e5, e6\right]\right] \quad (55)$$

> $Center(\,)$

(56)

$$[e1 + e3 + e7] \quad (56)$$

> LieAlgebraData([e1 − e3 − e7, e2, e5, 3 e1 + e3 + 3 e7, e6, 3 e4])

$$[[e1, e2] = 2\,e2, [e1, e3] = -2\,e3, [e2, e3] = e1, [e4, e5] = 2\,e5, [e4, e6] = -2\,e6, [e5, e6] = e4] \quad (57)$$

>

> n := 3 : m := 4 :

> var := seq(x || i, i = 0 ..n), seq(y || j, j = 0 ..m) : Dvar := seq(D_x || i, i = 0 ..n), seq(D_y || j, j = 0 ..m) : dvar := seq(dx || i, i = 0 ..n), seq(dy || j, j = 0 ..m) : DGsetup([var], M) :

> X := evalDG(add(add((a || i || j) var[i] Dvar[j], j = 1 ..n + m + 2), i = 1 ..n + m + 2)) :

> EQ := {seq(seq((x || i)·(x || j) − (x || (i + 1))·(x || (j − 1)), j = i + 2 ..n), i = 0 ..n − 2), seq(seq((x || i)·(y || j) − (x || (i + 1))·(y || (j − 1)), j = 1 ..m), i = 0 ..n − 1), seq(seq((y || i)·(y || j) − (y || (i + 1))·(y || (j − 1)), j = i + 2 ..m), i = 0 ..m − 2)}:

> rns := {seq(x || i = a λ^i, i = 0 ..n), seq(y || j = b λ^j, j = 0 ..m)} : simplify(eval(EQ, rns))

$$\{0\} \quad (58)$$

> J := ⟨op(EQ)⟩ : HilbertDimension(J)

$$3 \quad (59)$$

> sol := solve({seq(coeffs(expand(eval(LieDerivative(X, EQ[k]), rns)), {a, b, λ}), k = 1 ..nops(EQ))}) : free := { } :**for** i **to** nops(sol) **do if** lhs(sol[i]) = rhs(sol[i]) **then** free := {op(free), lhs(sol[i])} :**fi**:**od**: d := nops(free)

$$d := 7 \quad (60)$$

> Xtmp := eval(X, sol) :**for** i **to** d **do** X || i := DGsimplify(eval(Xtmp, {seq(free[j] = 0, j = 1 ..i − 1), free[i] = 1, seq(free[j] = 0, j = i + 1 ..d)})) :**od**:

> L := LieAlgebraData([seq(X || i, i = 1 ..d)], alg) : DGsetup(L) : LD := LeviDecomposition( )

$$LD := \left[[e1, e2, e3 + e7, e5], \left[e1 + \frac{2\,e3}{3} + \frac{4\,e7}{3}, e4, e6\right]\right] \quad (61)$$

> Center( )

$$[e1 + e3 + e7] \quad (62)$$

> LieAlgebraData([e1, e2, e5]); LieAlgebraData([3 e1 + 2 e3 + 4 e7, e6, 4 e4]); LieAlgebraData([3 e1 + 2 e3 + 4 e7, e1, e2, e5])

$$[[e1, e2] = -e2, [e1, e3] = -e3]$$
$$[[e1, e2] = 2\,e2, [e1, e3] = -2\,e3, [e2, e3] = e1]$$
$$[[e1, e3] = -e3, [e1, e4] = e4, [e2, e3] = -e3, [e2, e4] = -e4] \quad (63)$$

> evalDG(3 X1 + 2 X3 + 4 X7), evalDG(4 X4), X6

$$-3\,x0\,D\_x0 - x1\,D\_x1 + x2\,D\_x2 + 3\,x3\,D\_x3 - 4\,y0\,D\_y0 - 2\,y1\,D\_y1 + 2\,y3\,D\_y3 + 4\,y4\,D\_y4, x0\,D\_x1 + 2\,x1\,D\_x2 + 3\,x2\,D\_x3 + y0\,D\_y1 + 2\,y1\,D\_y2 + 3\,y2\,D\_y3 + 4\,y3\,D\_y4, 3\,x1\,D\_x0 + 2\,x2\,D\_x1 + x3\,D\_x2 + 4\,y1\,D\_y0 + 3\,y2\,D\_y1 + 2\,y3\,D\_y2 + y4\,D\_y3 \quad (64)$$

>

> n := 4 : m := 4 :

> var := seq(x || i, i = 0 ..n), seq(y || j, j = 0 ..m) : Dvar := seq(D_x || i, i = 0 ..n), seq(D_y || j, j = 0 ..m) : dvar := seq(dx || i, i = 0 ..n), seq(dy || j, j = 0 ..m) : DGsetup([var], M) :

> X := evalDG(add(add((a || i || j) var[i] Dvar[j], j = 1 ..n + m + 2), i = 1 ..n + m + 2)) :

> $EQ := \{seq(seq((x\|i)\cdot(x\|j) - (x\|(i+1))\cdot(x\|(j-1)), j=i+2..n), i=0..n-2), seq(seq((x\|i)\cdot(y\|j) - (x\|(i+1))\cdot(y\|(j-1)), j=1..m), i=0..n-1), seq(seq((y\|i)\cdot(y\|j) - (y\|(i+1))\cdot(y\|(j-1)), j=i+2..m), i=0..m-2)\}:$

> $rns := \{seq(x\|i = a\,\lambda^i, i=0..n), seq(y\|j = b\,\lambda^j, j=0..m)\} : simplify(eval(EQ, rns))$

$$\{0\} \quad \textbf{(65)}$$

> $J := \langle op(EQ)\rangle : HilbertDimension(J)$

$$3 \quad \textbf{(66)}$$

> $sol := solve(\{seq(coeffs(expand(eval(LieDerivative(X, EQ[k]), rns)), \{a, b, \lambda\}), k=1..nops(EQ))\}) : free := \{\ \}$ :**for** $i$ **to** $nops(sol)$ **do if** $lhs(sol[i]) = rhs(sol[i])$ **then** $free := \{op(free), lhs(sol[i])\}$ :**fi**:**od**: $d := nops(free)$

$$d := 7 \quad \textbf{(67)}$$

> $Xtmp := eval(X, sol)$ :**for** $i$ **to** $d$ **do** $X\|i := DGsimplify(eval(Xtmp, \{seq(free[j]=0, j=1..i-1), free[i]=1, seq(free[j]=0, j=i+1..d)\}))$ :**od**:

> $L := LieAlgebraData([seq(X\|i, i=1..d)], alg) : DGsetup(L) : LD := LeviDecomposition(\ )$

$$LD := \left[[e2+e3+e7], \left[e1, e2+\frac{e7}{2}, e3+\frac{3\,e7}{2}, e4, e5, e6\right]\right] \quad \textbf{(68)}$$

> $Center(\ )$

$$[e2+e3+e7] \quad \textbf{(69)}$$

> $LieAlgebraData([e2-e3-e7, e1, e5, 4\,e2+2\,e7, e6, 8\,e4])$

$$[[e1, e2] = 2\,e2, [e1, e3] = -2\,e3, [e2, e3] = e1, [e4, e5] = 2\,e5, [e4, e6] = -2\,e6, [e5, e6] = e4] \quad \textbf{(70)}$$

> $evalDG(X2 - X3 - X7), X1, X5; evalDG(4\,X2 + 2\,X7), evalDG(2\,X6), evalDG(4\,X4)$

$$x0\,D\_x0 + x1\,D\_x1 + x2\,D\_x2 + x3\,D\_x3 + x4\,D\_x4 - y0\,D\_y0 - y1\,D\_y1 - y2\,D\_y2 - y3\,D\_y3 - y4\,D\_y4, x0\,D\_y0 + x1\,D\_y1 + x2\,D\_y2 + x3\,D\_y3 + x4\,D\_y4, y0\,D\_x0 + y1\,D\_x1 + y2\,D\_x2 + y3\,D\_x3 + y4\,D\_x4$$

$$-4\,x0\,D\_x0 - 2\,x1\,D\_x1 + 2\,x3\,D\_x3 + 4\,x4\,D\_x4 - 4\,y0\,D\_y0 - 2\,y1\,D\_y1 + 2\,y3\,D\_y3 + 4\,y4\,D\_y4, 4\,x1\,D\_x0 + 3\,x2\,D\_x1 + 2\,x3\,D\_x2 + x4\,D\_x3 + 4\,y1\,D\_y0 + 3\,y2\,D\_y1 + 2\,y3\,D\_y2 + y4\,D\_y3, x0\,D\_x1 + 2\,x1\,D\_x2 + 3\,x2\,D\_x3 + 4\,x3\,D\_x4 + y0\,D\_y1 + 2\,y1\,D\_y2 + 3\,y2\,D\_y3 + 4\,y3\,D\_y4 \quad \textbf{(71)}$$

>

>

Conclusion: sym(S[n,n])=sl(2)+sl(2) and for n<m sym(S[n,m])=gl(2)⋉R^{m-n+1} of dim=m-n+5 (the Abelian part is S^{m-n}(R^2) irrep).
Thus sym(RNS) differ by (ambien.dim,deg,dim.sym): for m=n we get (2n+1,2n,6) for n<m we get (n+m+1,n+m,m-n+5); the cases m=n and m=n+1 differ by the structure (semi-simple vs semi-direct)

>
